# Supplementary material for: A Complete and Natural Rule Set for Multi-Qutrit Clifford Circuits
Source: arXiv:2508.14670 ancillary file (2025-08-20)
Supplement: Supplementary file 1 [file supplement.pdf]

# A Complete and Natural Rule Set for Multi-Qutrit Clifford Circuits: Derived Relations and Supplemental Proofs

Sarah Meng Li  
sarah.li@uva.nl

Michele Mosca  
michele.mosca@uwaterloo.ca

Neil J. Ross  
neil.jr.ross@dal.ca

John van de Wetering  
john@vdwetering.name

Yuming Zhao  
yuming@math.ku.dk

We demonstrate that the 380 box relations listed in Appendix C of [1] can be derived from the 18 reduced relations shown in Figure 1 and the generators presented in Figure 2. As a byproduct of this derivation, we identify a set of *derived relations* that follow from the equations in Figures 1 and 2. They serve as a useful set of axioms for simplifying the supplemental proofs.

## Contents

|          |                                                      |           |
|----------|------------------------------------------------------|-----------|
| <b>1</b> | <b>Derived Relations</b>                             | <b>4</b>  |
| 1.1      | The Single-Qutrit Derived Relations . . . . .        | 6         |
| 1.2      | The Two-Qutrit Derived Relations . . . . .           | 7         |
| 1.3      | The Three-Qutrit Derived Relations . . . . .         | 21        |
| <b>2</b> | <b>Single-Qutrit Clifford Completeness</b>           | <b>41</b> |
| 2.1      | Reduce the Single-Qutrit Derived Relations . . . . . | 42        |
| 2.2      | Reduce the Single-Qutrit Box Relations . . . . .     | 46        |
| <b>3</b> | <b>Two-Qutrit Clifford Completeness</b>              | <b>52</b> |
| 3.1      | Reduce the Two-Qutrit Derived Relations . . . . .    | 56        |
| 3.2      | Reduce the Two-Qutrit Box Relations . . . . .        | 90        |
| <b>4</b> | <b>Three-Qutrit Clifford Completeness</b>            | <b>90</b> |
| 4.1      | Reduce the Three-Qutrit Derived Relations . . . . .  | 93        |
| 4.2      | Reduce the Three-Qutrit Box Relations . . . . .      | 166       |

Throughout this supplement, we use the same definitions and conventions as given in Section 2 and Appendix E of [1]. We begin by reducing all single-qutrit derived relations and box relations to the equations in Figures 53 and 54. This allows us to establish the completeness for single-qutrit Clifford circuits. We then use this completeness result as a lemma to prove that all two-qutrit derived relations and box relations follow from the equations in Figures 57 and 58. Similarly, after establishing the completeness for two-qutrit Clifford circuits, we use it as a lemma to prove that all three-qutrit derived relations and box relations follow from the equations in Figures 59 and 60. Thus, in Sections 2 to 4, our approach to the relation reduction is organized according to the number of qutrits in the circuit. The correctness of all proofs was verified by checking that the circuit semantics remain unchanged at various intermediate steps <sup>1</sup>.

<sup>1</sup><https://github.com/SarahMMMLi/QuTritClifford/blob/main/Verification.ipynb>

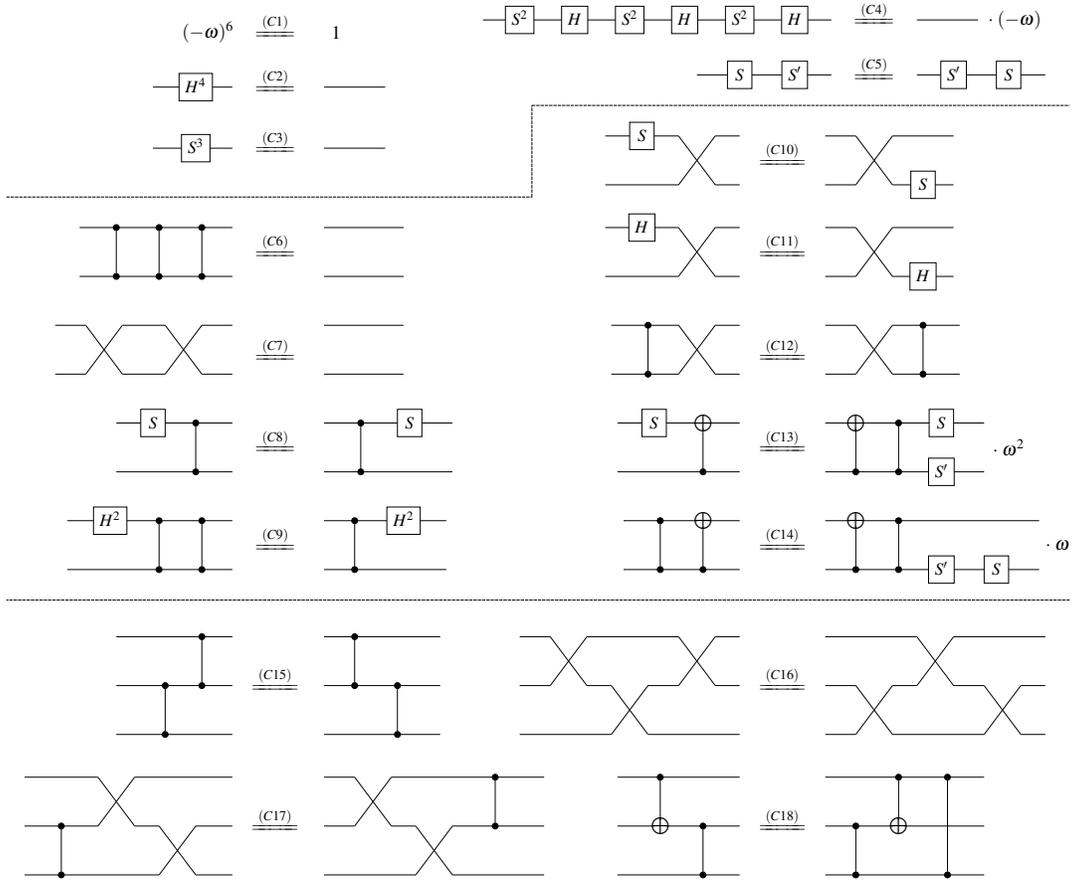

Figure 1: A complete set of rewrite rules for  $n$ -qutrit Clifford circuits. Note that  $\omega$ ,  $S'$ , SWAP, CX, XC, and the CZ acting on the first and third qutrits are derived generators defined in Figure 2. Let  $g$  be a gate and  $m$  be a natural number.  $g^m$  denotes  $m$  copies of  $g$  gate. In addition to these circuit relations, we assume the standard spatial relations which allow us to commute gates acting on disjoint subsets of qutrits. In the remainder of this paper, we use ‘relations’ and ‘(rewrite) rules’ interchangeably.

**Definition 0.1.** The equations in Figure 1 are called the reduced relations. The lefthand sides of the equations in Figure 2 are called the derived generators. The equations in Appendix C of [1] are called the box relations. The equations that follow from those in Figures 1 and 2 are called the derived relations.

**Definition 0.2.** When we say that an equation follows from the reduced relations, we mean that it can be proved using the equations from Figures 1 and 2. Then, we say that the circuits on both sides of the equation is syntactically equivalent. Each circuit represents a unitary matrix. Any equality between two circuits is a true equality if the unitary matrices are the same. Then, we say that these two circuits are semantically equivalent.

**Definition 0.3.** Let  $R : C_1 = C_2$  be an equation where  $C_1, C_2 \in \mathcal{C}_n$ .  $C_1 = C_2$  means that there exists a sequence of rules from Figure 1 to rewrite  $C_1$  into  $C_2$ .

For convenience, we use several conventions in Sections 2 to 4. They are summarized below.

- Let  $a \in \mathbb{N}$ . For  $u, v \in \mathbb{Z}$ , we use  $u \equiv_a v$  to denote  $u$  is congruent to  $v$  modulo  $a$ .

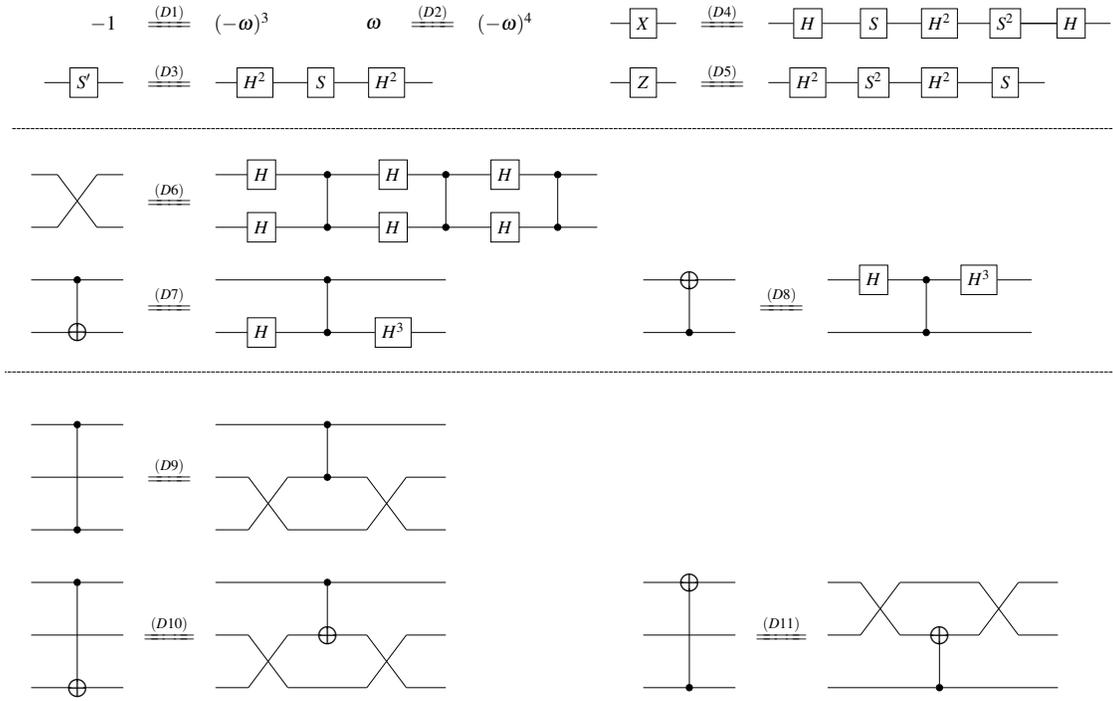

Figure 2: Derived generators of  $C_n$  that are useful for the relation reduction.

- We use *relations*, (*rewrite*) *rules*, and *equations* interchangeably.
- We use  $\stackrel{\text{(def)}}{=}$  to reference a definition from [Figure 3](#).

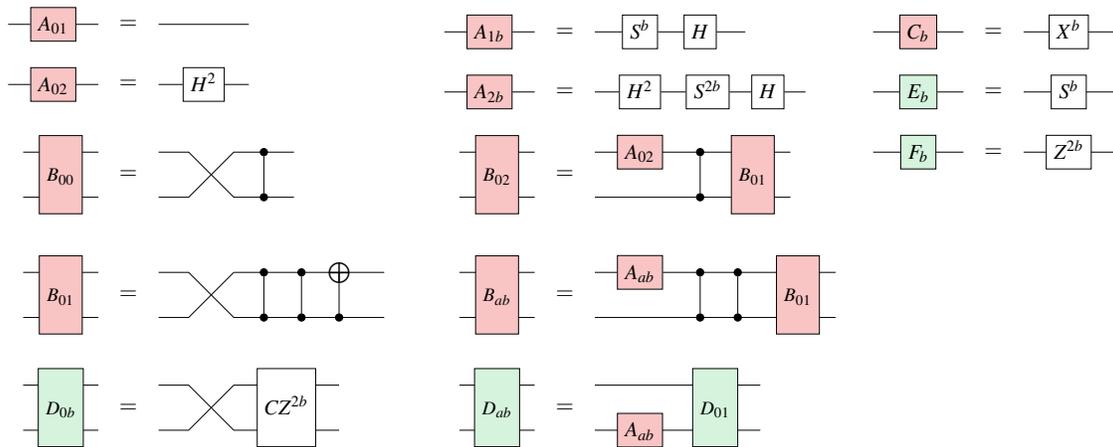

Figure 3: The concrete implementations of the Z and X normal boxes. Here  $a, b \in \mathbb{Z}_3$  and  $a \neq 0$ .

- We use  $AB$  to denote two gates  $A$  and  $B$  composed in diagrammatic order:

$$AB = \begin{array}{c} \text{---} \\ \vdots \\ \text{---} \end{array} \boxed{A} \begin{array}{c} \text{---} \\ \vdots \\ \text{---} \end{array} \boxed{B} \begin{array}{c} \text{---} \\ \vdots \\ \text{---} \end{array}$$

- Let  $C, C' \in \mathcal{C}_n$  and  $R$  be a rewrite rule. We write  $C \stackrel{R}{=} C'$  to denote that after applying  $R$  to  $C$ , we get  $C'$ , which is semantically equivalent to  $C$ .
- Let  $R: A = B$  and  $R': A' = B'$ . We write  $R \iff R'$  to denote that the equation  $R$  can be *equivalently expressed* as the equation  $R'$  after applying certain rewrite rules.
- We use an orange dashed box to denote where a rewrite rule has been applied to a circuit. An example is below.

$$\begin{array}{c} (C_6^1).\text{LHS} = \\ \text{---} \oplus \oplus \oplus \text{---} \\ \bullet \bullet \bullet \\ \text{---} \end{array} \stackrel{(D8)}{=} \begin{array}{c} \text{---} \boxed{H} \bullet \text{---} \boxed{H^3} \text{---} \boxed{H} \bullet \text{---} \boxed{H^3} \text{---} \boxed{H} \bullet \text{---} \boxed{H^3} \text{---} \\ \bullet \bullet \bullet \\ \text{---} \end{array} \\ \stackrel{(C2)}{=} \begin{array}{c} \text{---} \boxed{H} \bullet \bullet \bullet \text{---} \boxed{H^3} \\ \bullet \bullet \bullet \\ \text{---} \end{array} \stackrel{(C6)}{=} \begin{array}{c} \text{---} \boxed{H} \text{---} \boxed{H^3} \text{---} \\ \text{---} \end{array} \stackrel{(C2)}{=} \text{---} = (C_6^1).\text{RHS}$$

- We use a few abbreviations in the proofs. WTS is short for *Want To Show*. LHS is short for *the lefthand side*. RHS is short for *the righthand side*. Given a rewrite rule  $R$ ,  $R.\text{LHS}$  refers to the lefthand side of  $R$ , and  $R.\text{RHS}$  refers to the righthand side of  $R$ .

## 1 Derived Relations

Before reducing all box relations to a smaller set of rewrite rules, it is helpful to first obtain an expanded rule set that serves as a ‘halfway point’. For this, we introduce the notion of *derived relations*, which are the relations implied by the 18 reduced relations in [Figure 1](#) and the 9 derived generators in [Figure 2](#). According to the number of qutrits being involved, we list these derived relations in [Sections 1.1 to 1.3](#). We came to these relations as they either express canonical relations about pushing one gate across the other or they follow from the property of a SWAP gate. On the other hand, we found that many box relations were reducible to simpler forms, which are then added as a derived relation.

Let  $R$  be some relation that we have shown to be derivable from [Figure 1](#). Then the following rules based on modifying  $R$  are also derivable. We use a superscript to denote such a relation (e.g.,  $R^k$ ). Since these techniques are frequently used, we call them *meta rules* and describe how they work below.

**Meta Rule 1:** The relation where we take any permutation of the qutrit wires on both sides of  $R$ . This follows after we have proven properties regarding the SWAP gate. For example, in [Figure 9](#),  $(C_6^2)$  can be derived from  $(C_6^1)$  by permuting the first and the second qutrit wires.

**Meta Rule 2:** The relation where we take the inverse of both sides of  $R$ . This follows from the order of  $-\omega, S, H$  and CZ being axioms of [Figure 1](#). For example, in [Figure 11](#),  $(C_9^4)$  can be derived from  $(C_9)$  by leveraging  $(C_2)$ :  $H^4 = I$ .

**Meta Rule 3:** The relation where we append or prepend both the left- and righthand sides of  $R$  with the same gates. In particular, doing this with powers of  $H$  gates allows us to exchange the CZ gate with the CX (or XC) gate. For example, in [Figure 9](#),  $(C_6^1)$  can be derived from  $(C6)$  by leveraging  $(D8)$  and  $(C2)$ .

**Meta Rule 4:** The relation that follows from applying a rule a couple of times. Summarizing them into axioms allows us to shorten the proofs of relation reduction. For example, in [Figure 11](#),  $(C_9^2)$  can be derived by applying  $(C9)$  twice.

In [Sections 1.1 to 1.3](#), we present the derived relations for one-, two-, and three-qutrit Clifford circuits. The labelling of these relations matches the order of the proofs in [Sections 2.1, 3.1 and 4.1](#). This is intentionally arranged to prevent circular reasoning in the proofs of relation reduction.

## 1.1 The Single-Qutrit Derived Relations

$$S'^3 = 1 \quad (R1)$$

$$X^2 = HS^2H^2SH \quad (R2)$$

$$X^3 = 1 \quad (R3)$$

$$Z = S'^2S \quad (R4)$$

$$Z^2 = S'S^2 \quad (R5)$$

$$Z^3 = 1 \quad (R6)$$

$$HSH = S^2HS^2X^2 \cdot (-\omega^2) \quad (R7)$$

$$SH^2 = H^2SZ^2 \quad (R8)$$

$$SZ = ZS \quad (R9)$$

$$Z^2H = HX \quad (R10)$$

$$SX = XZS \cdot \omega^2 \quad (R11)$$

$$ZX = XZ \cdot \omega^2 \quad (R12)$$

Figure 4: Single-qutrit derived relations.

$$S^2HS^2HS^2H = -\omega \quad (C4)$$

$$S^2HS^2 = H^3SH^3 \cdot (-\omega) \quad (C_4^1)$$

$$SH^3S = HS^2H \cdot (-\omega^2) \quad (C_4^2)$$

$$S'H^3S' = HS'^2H \cdot (-\omega^2) \quad (C_4^3)$$

$$H^3S = S^2HS^2H \cdot (-\omega^2) \quad (C_4^4)$$

$$SH^2SH^2 = H^2SH^2S \quad (C5)$$

$$SH^2S = H^2SH^2SH^2 \quad (C_5^1)$$

Figure 5: Variants of (C4) and (C5).

$$HSH = S^2HS^2X^2 \cdot (-\omega^2) \quad (R7)$$

$$HS^2H = H^2SHXS \cdot (-\omega) \quad (R_7^1)$$

Figure 6: An alternative expression of (R7).

$$Z^2H = HX \quad (R10)$$

$$HZH^3 = X \quad (R_{10}^1)$$

$$HZ^2H^3 = X^2 \quad (R_{10}^2)$$

Figure 7: Interchanging between Pauli  $X$  and  $Z$  gates using the  $H$  gate.

### 1.2 The Two-Qutrit Derived Relations

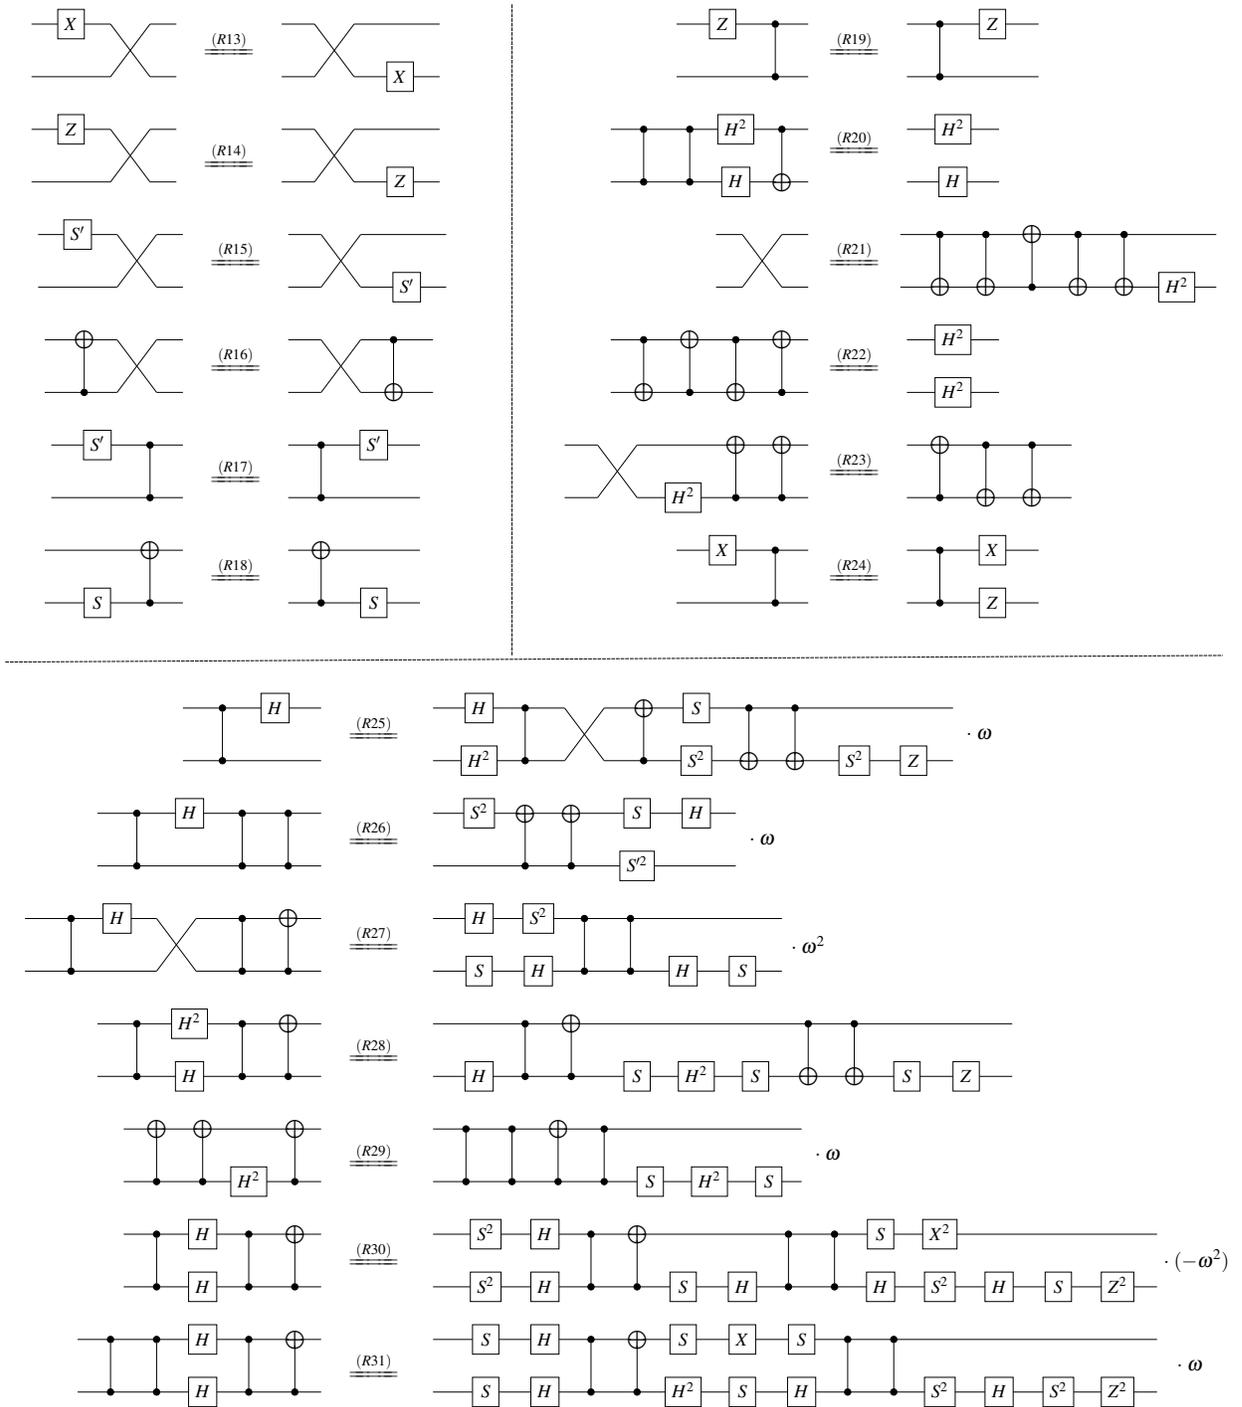

Figure 8: Two-qutrit derived relations.

(C6)

(C6<sup>1</sup>)

(C6<sup>2</sup>)

Figure 9: Equations that follow from the order of a CZ gate:  $CZ^3 = 1$ .

(C8)

(C8<sup>1</sup>)

Figure 10: Pushing an  $S$  gate through a CZ gate and its vertically symmetrical variant.

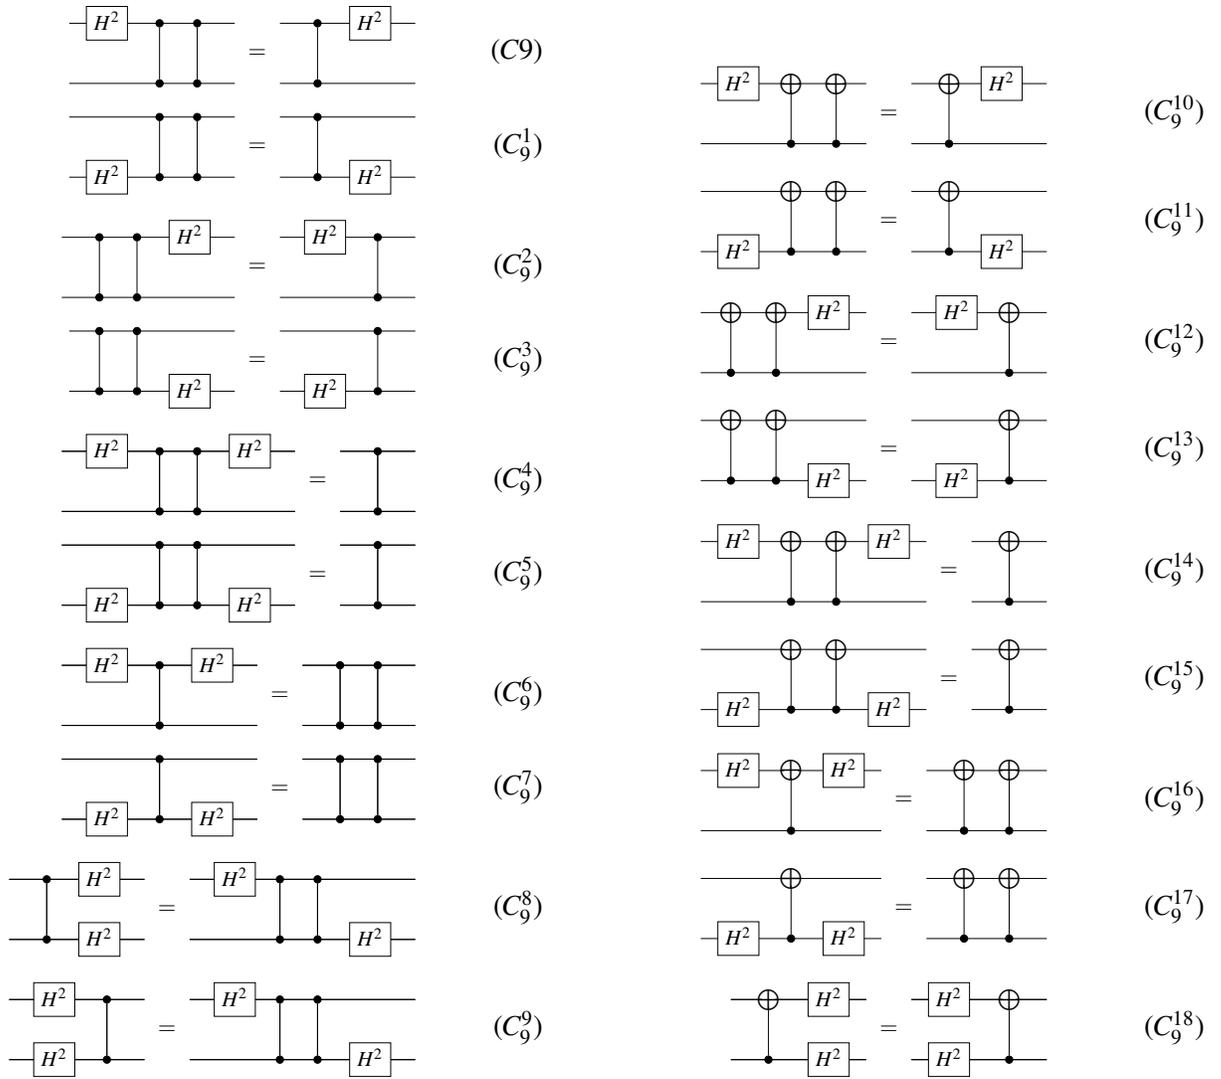

Figure 11: Pushing  $H^2$  through a CZ gate and its variants.

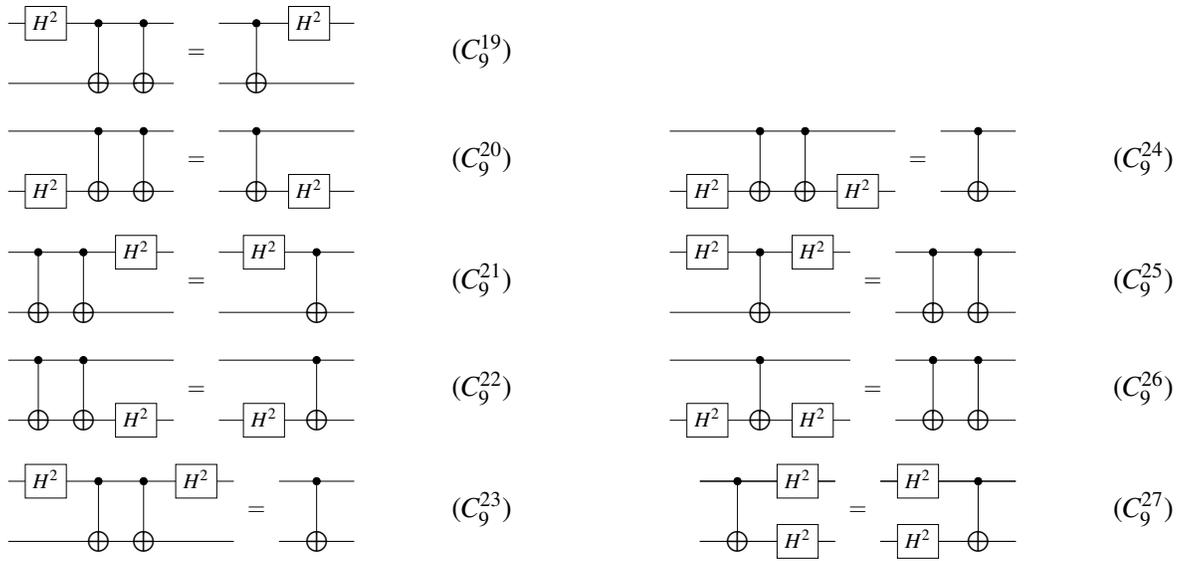

Figure 12: The vertically symmetrical variants of the equations in Figure 11.

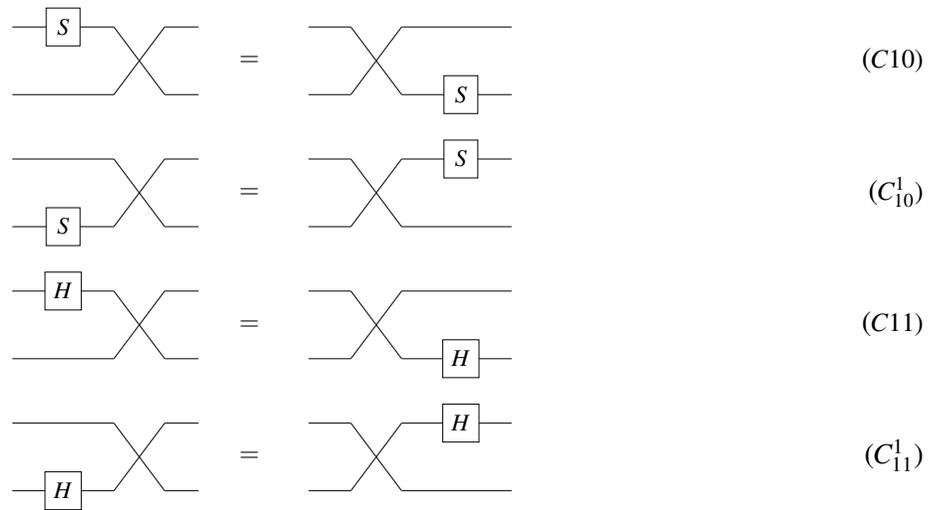

Figure 13: Pushing an  $H$  or  $S$  gate through a SWAP gate and their vertically symmetrical variants.

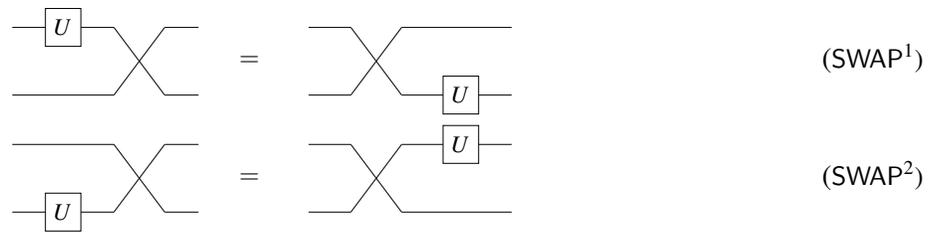

Figure 14: Pushing single-qutrit Clifford unitaries through a SWAP gate.

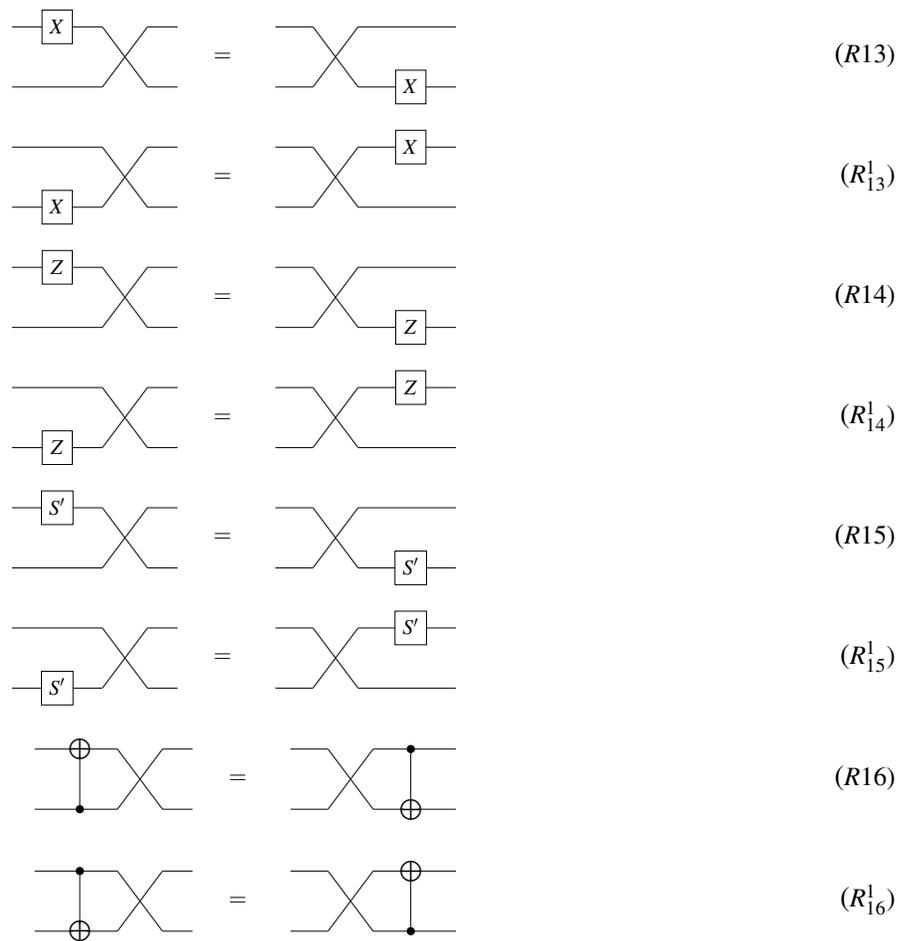

Figure 15: Pushing an  $X$ ,  $Z$ ,  $S'$ ,  $CX$ , or  $XC$  gate through a SWAP gate and their vertically symmetrical variants.

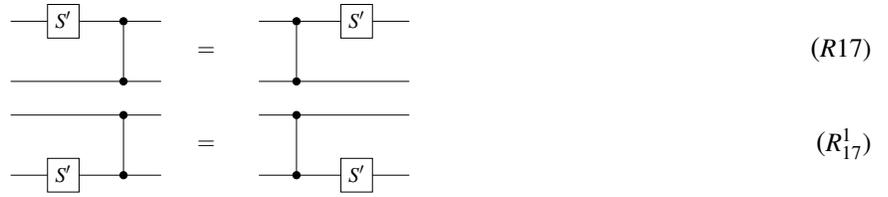

Figure 16: Pushing an  $S'$  gate through a CZ gate and its vertically symmetrical variant.

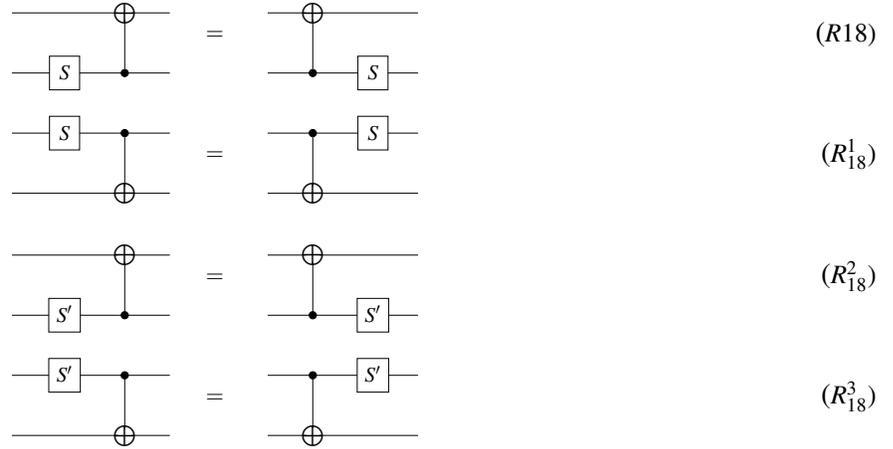

Figure 17: When an  $S$  or  $S'$  gate commutes with a CX or XC gate.

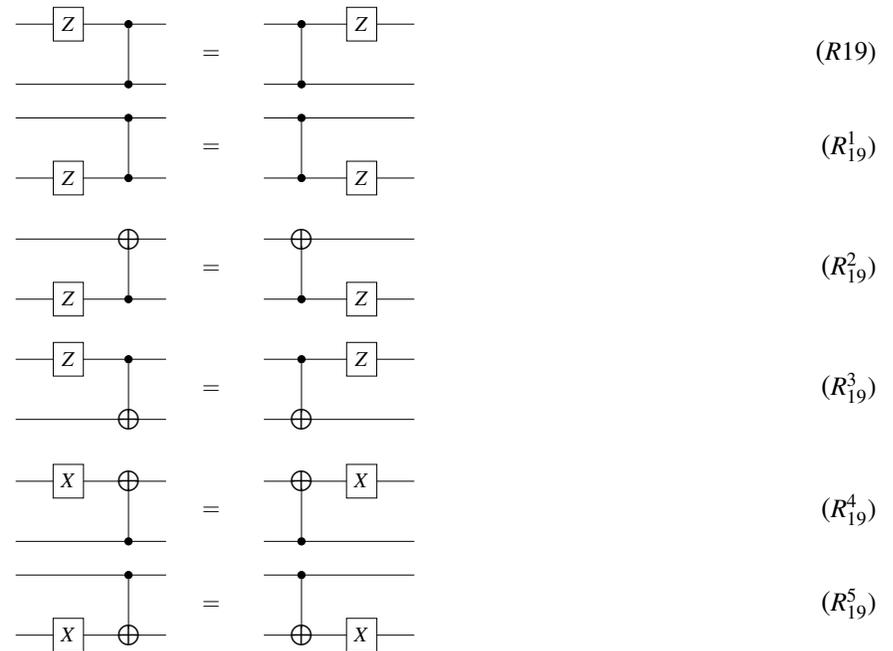

Figure 18: When a Pauli  $X$  or  $Z$  gate commutes with a CZ, CX, or XC gate.

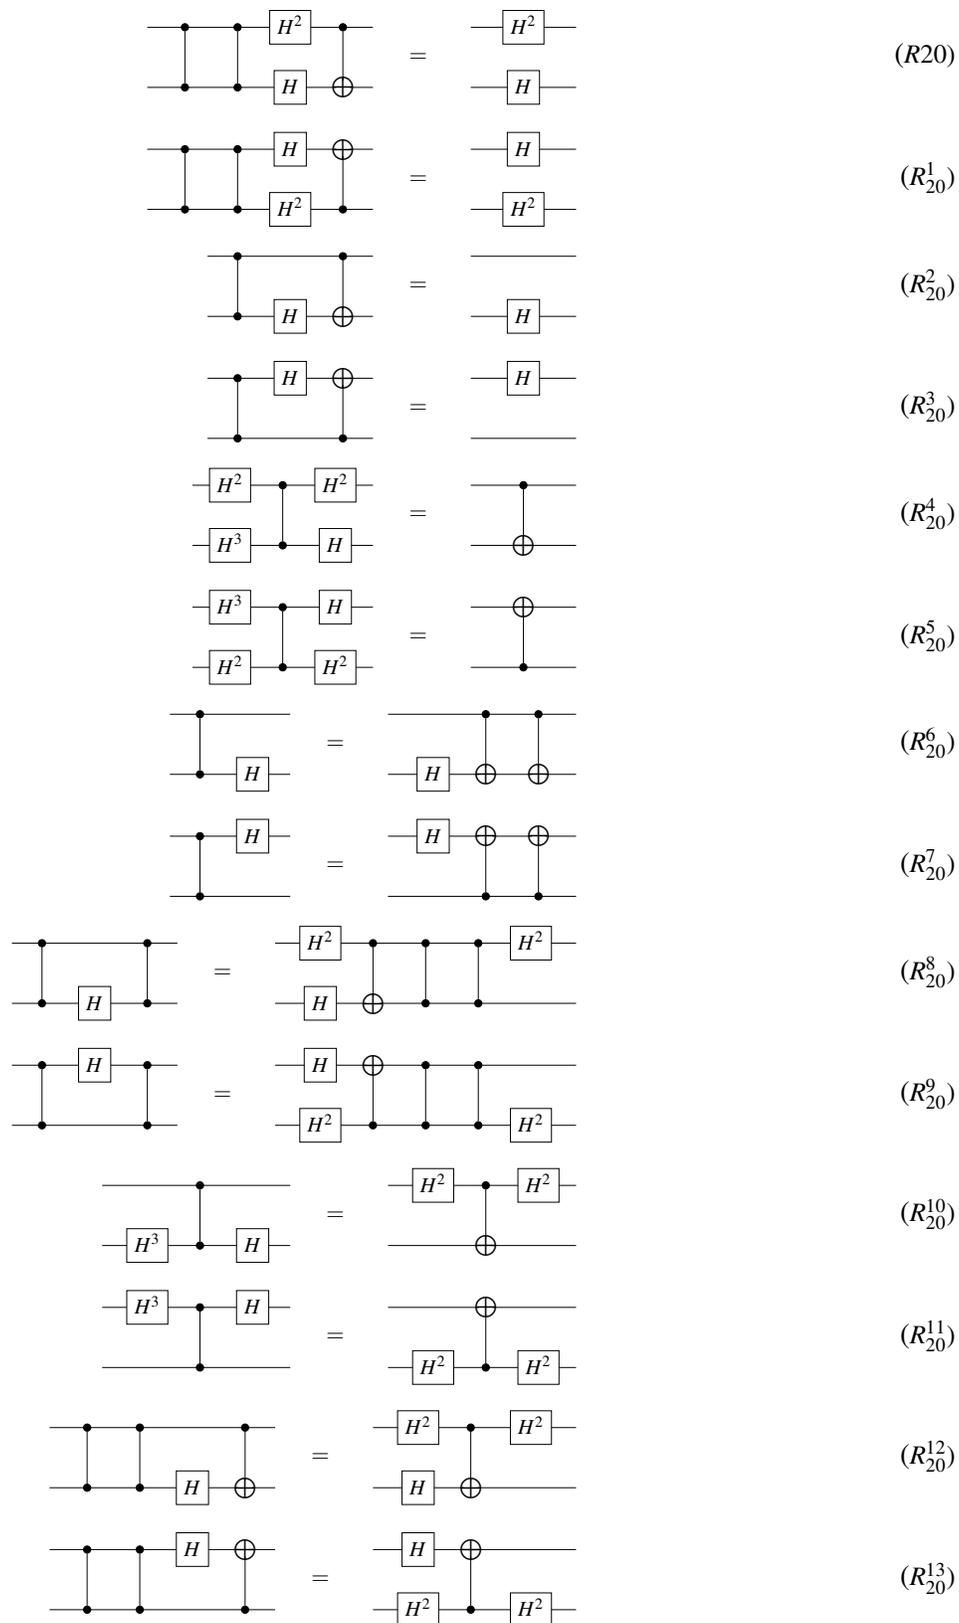

Figure 19:  $(R_{20}^1)$  to  $(R_{20}^{13})$  can be derived from  $(R_{20})$ . They are useful for deriving some other two-qutrit Clifford relations.

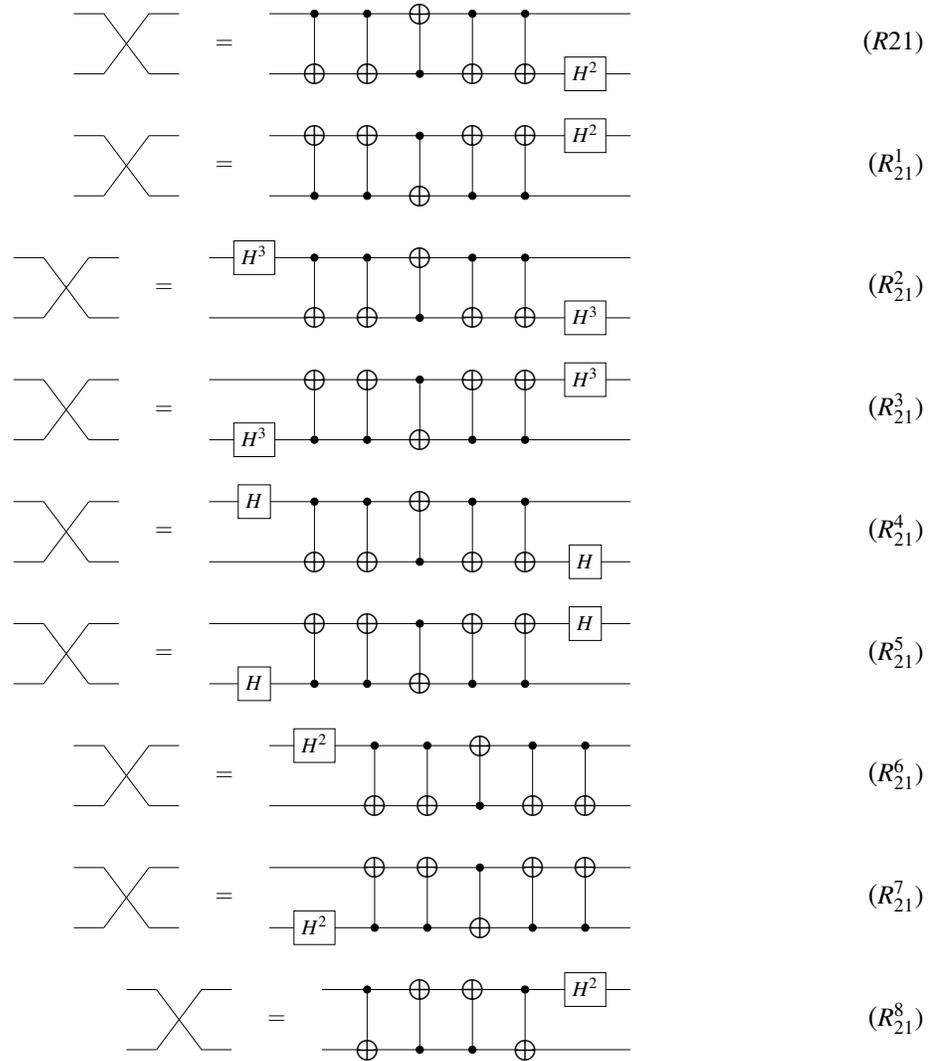

Figure 20: Different implementations of a SWAP gate.

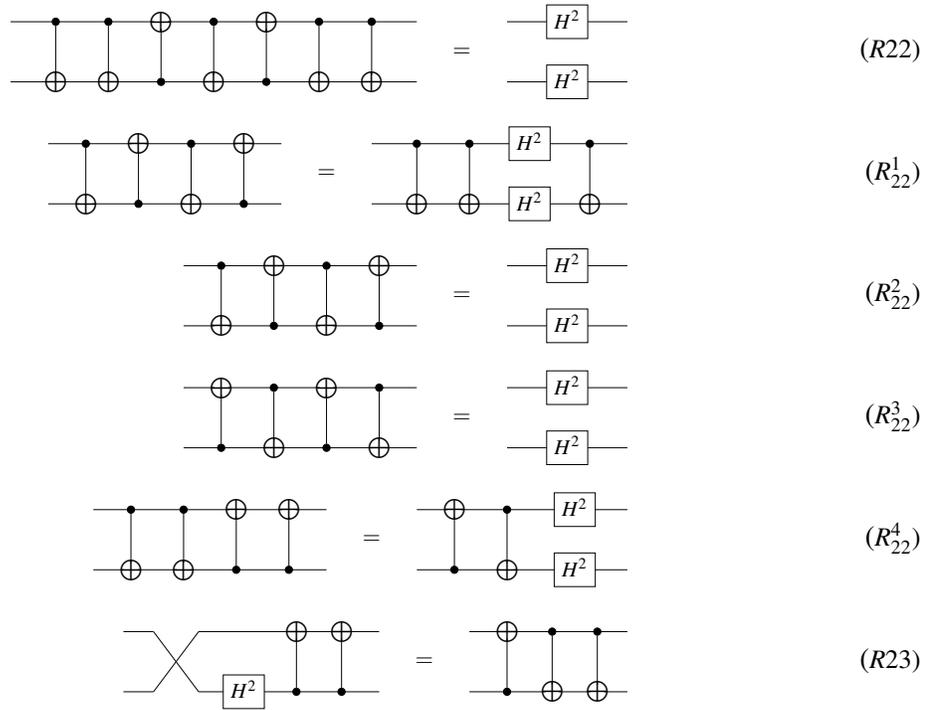

Figure 21: (R22) to (R23) can be derived using the equations in Figure 20.

(C<sub>13</sub>)

(C<sub>13</sub><sup>1</sup>)

(C<sub>13</sub><sup>2</sup>)

(C<sub>13</sub><sup>3</sup>)

(C<sub>13</sub><sup>4</sup>)

(C<sub>13</sub><sup>5</sup>)

(C<sub>13</sub><sup>6</sup>)

Figure 22: When an  $S$  gate does not commute with an XC gate, it can be pushed through the target of XC and produce some single-qutrit gates.

(C<sub>13</sub><sup>7</sup>)

(C<sub>13</sub><sup>8</sup>)

(C<sub>13</sub><sup>9</sup>)

(C<sub>13</sub><sup>10</sup>)

(C<sub>13</sub><sup>11</sup>)

(C<sub>13</sub><sup>12</sup>)

Figure 23: The vertically symmetrical variants of the equations in [Figure 22](#).

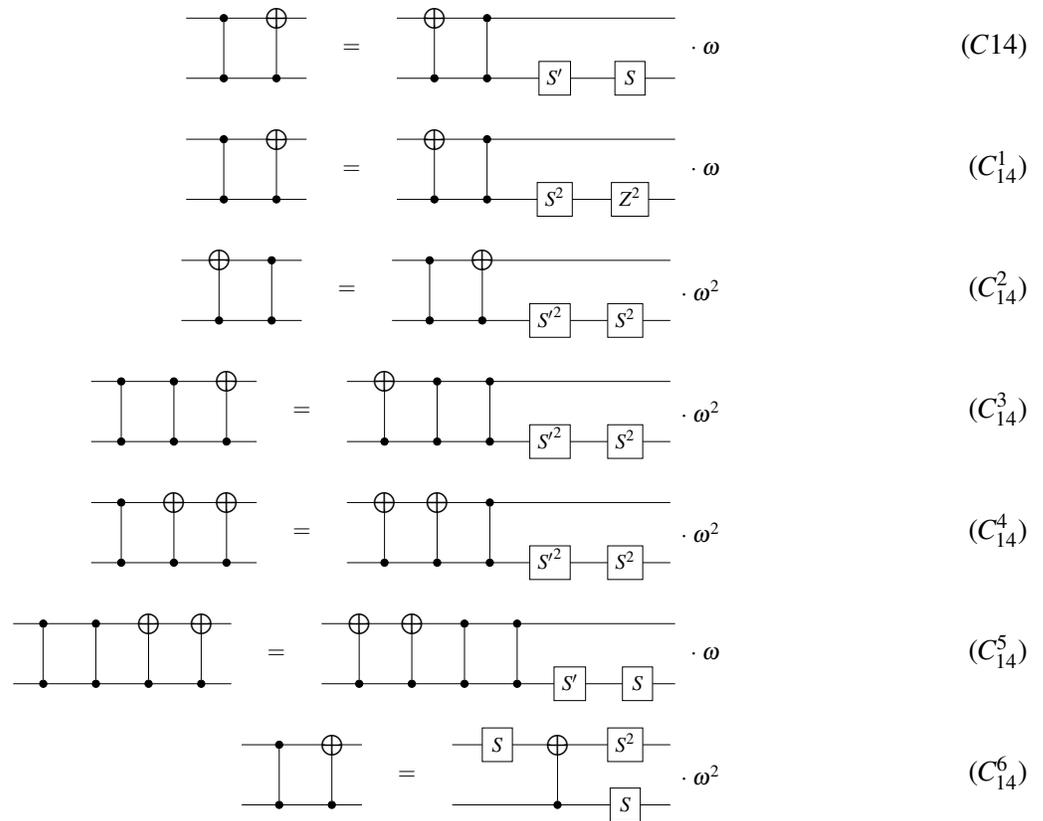

Figure 24: Different cases of pushing a CZ gate through an XC gate.

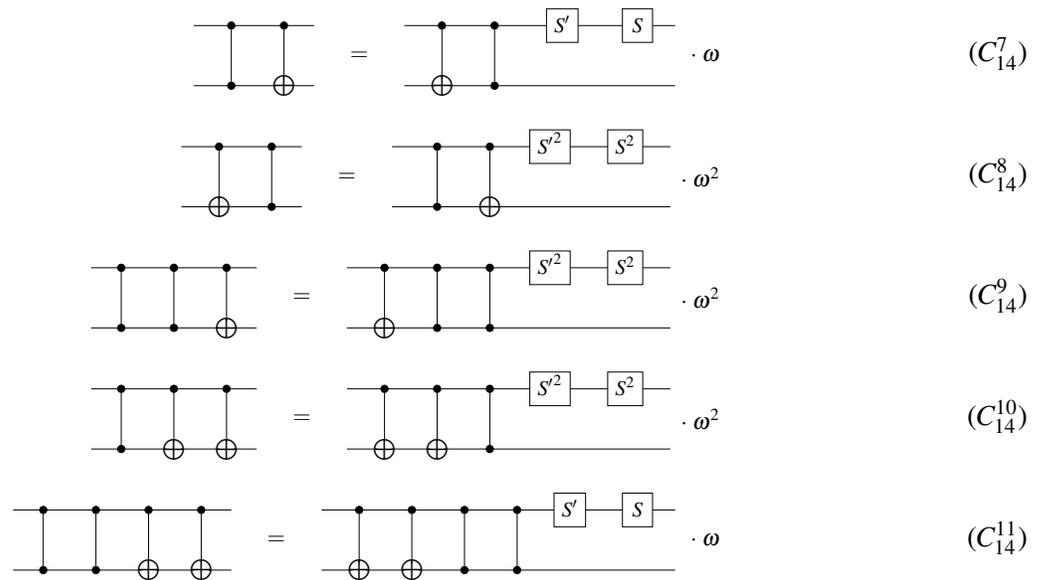

Figure 25: The vertically symmetrical variants of the equations in [Figure 24](#).

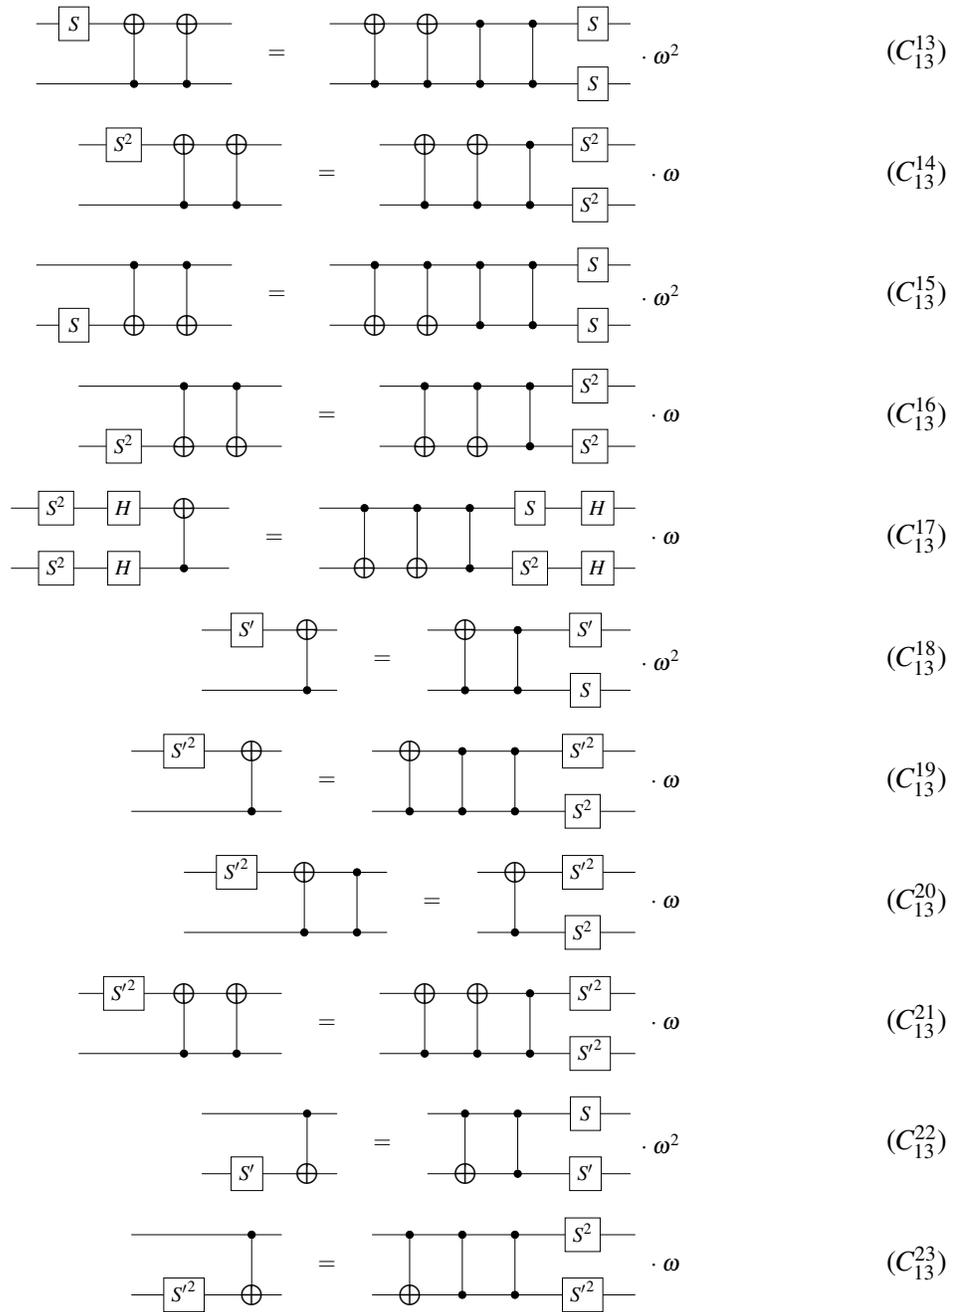

Figure 26: Different cases of pushing an  $S$  or  $S'$  gate through an XC gate. They can be derived using the equations in [Figures 22 to 25](#).

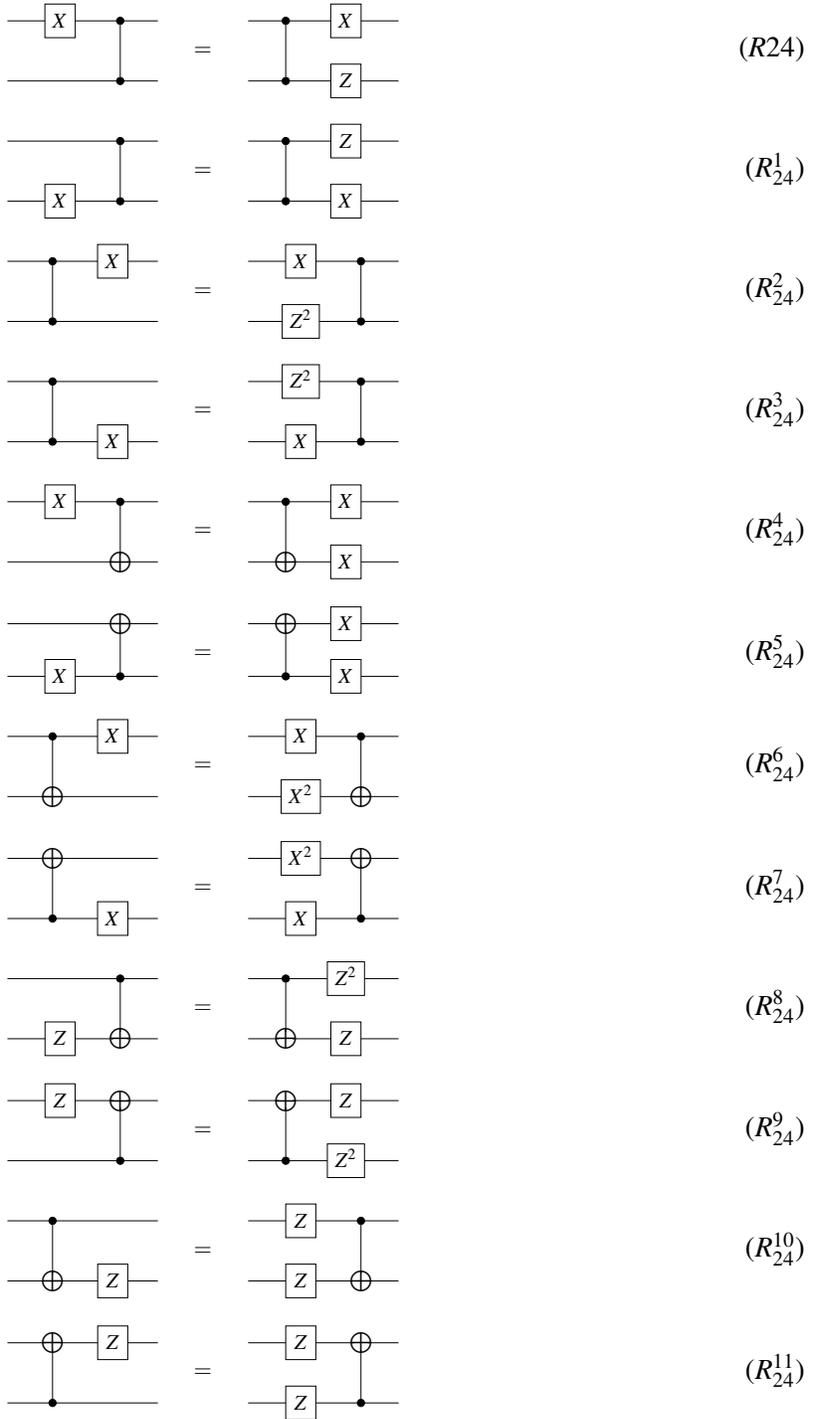

Figure 27: When a Pauli  $X$  or  $Z$  gate does not commute with a  $CZ$ ,  $CX$ , or  $XC$  gate.

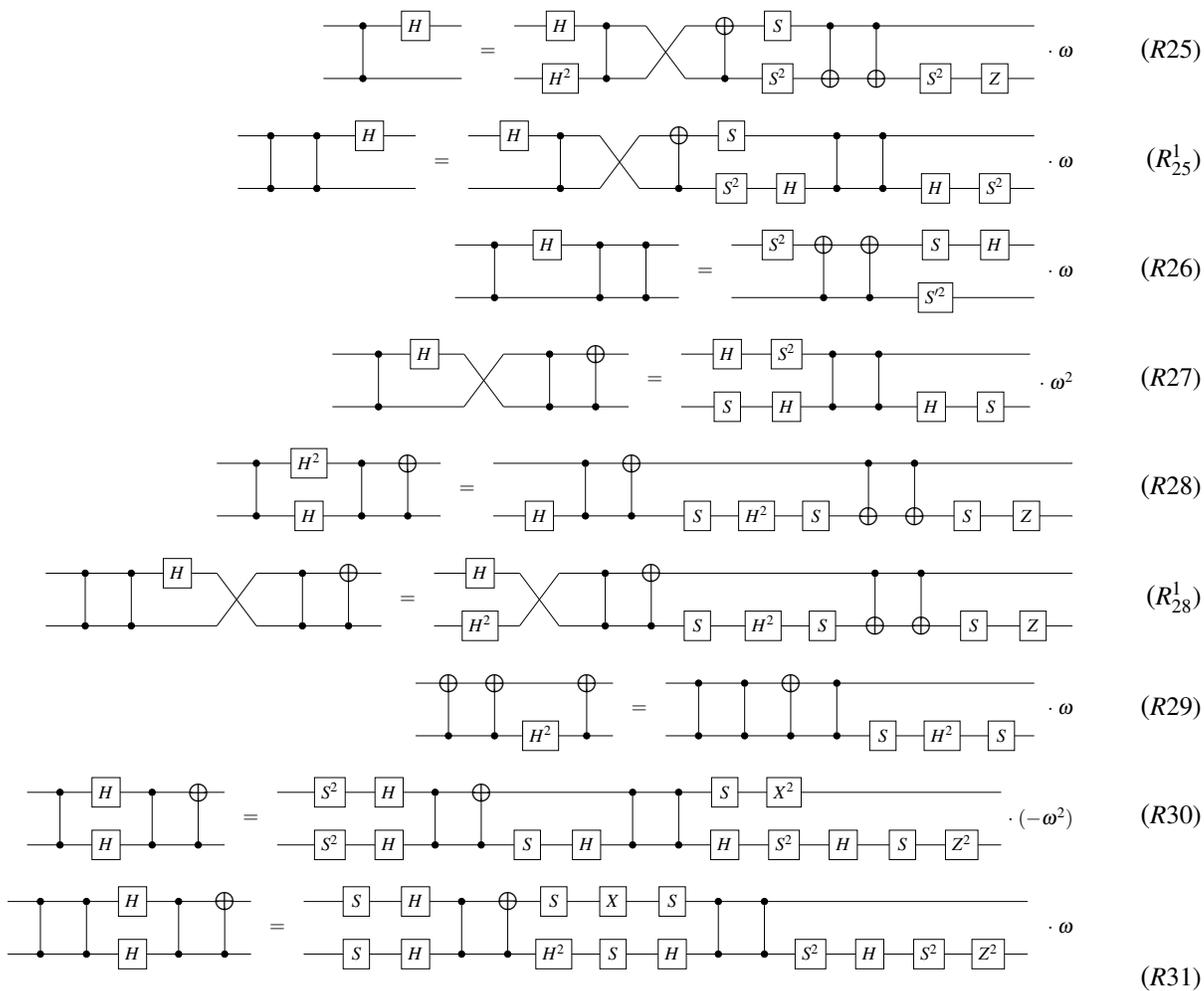

Figure 28: Other derived relations that are used to reduce the two-qutrit box relations.

### 1.3 The Three-Qutrit Derived Relations

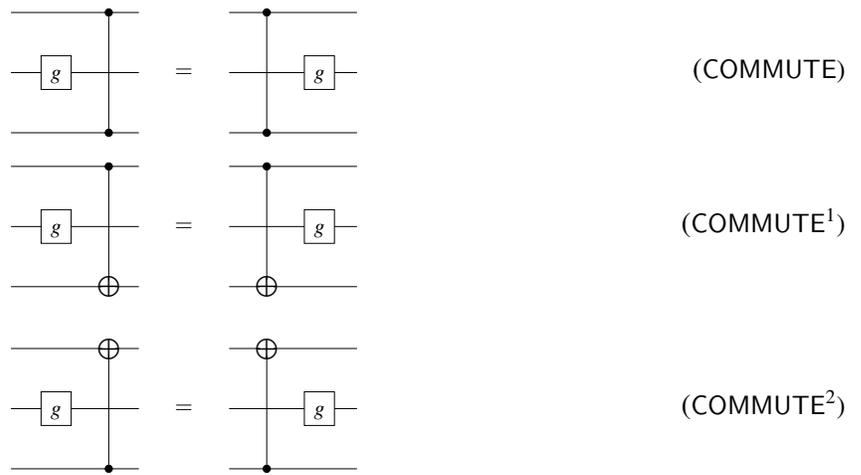

Figure 29: A single-qutrit gate  $g$  on wire 2 can be moved past a two-qutrit gate on wires 1 and 3.

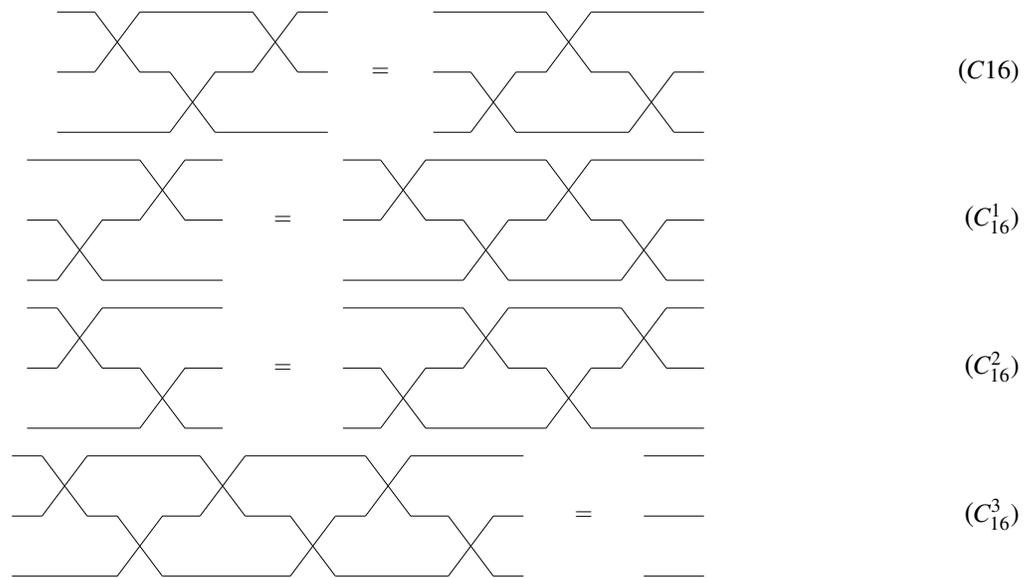

Figure 30: Different ways of presenting the Yang–Baxter equation.

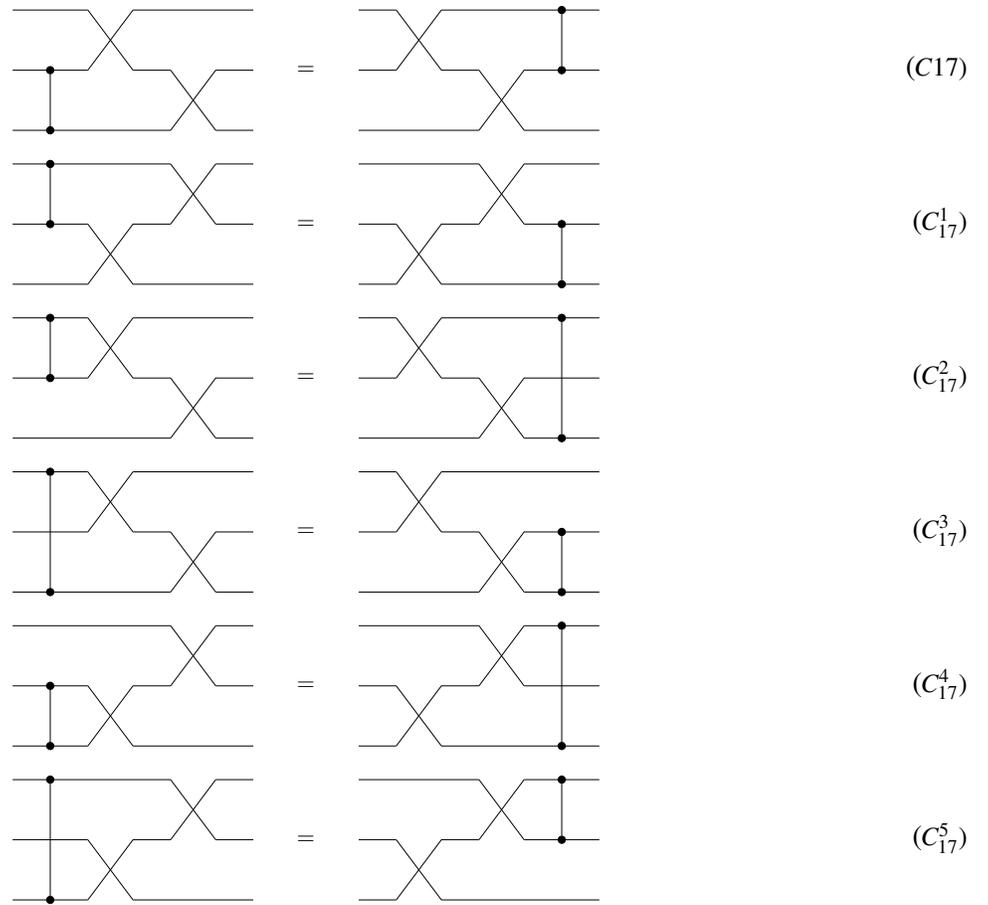

Figure 31: Pushing a CZ gate through two stacked SWAP gates.

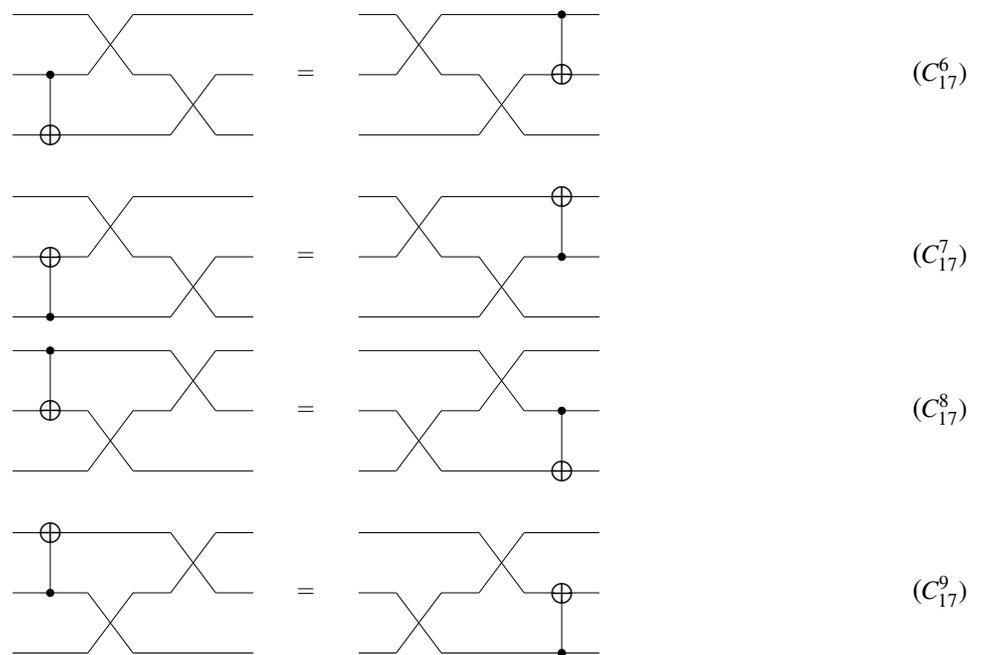

Figure 32: Pushing a CX or XC gate through two stacked SWAP gates, part 1.

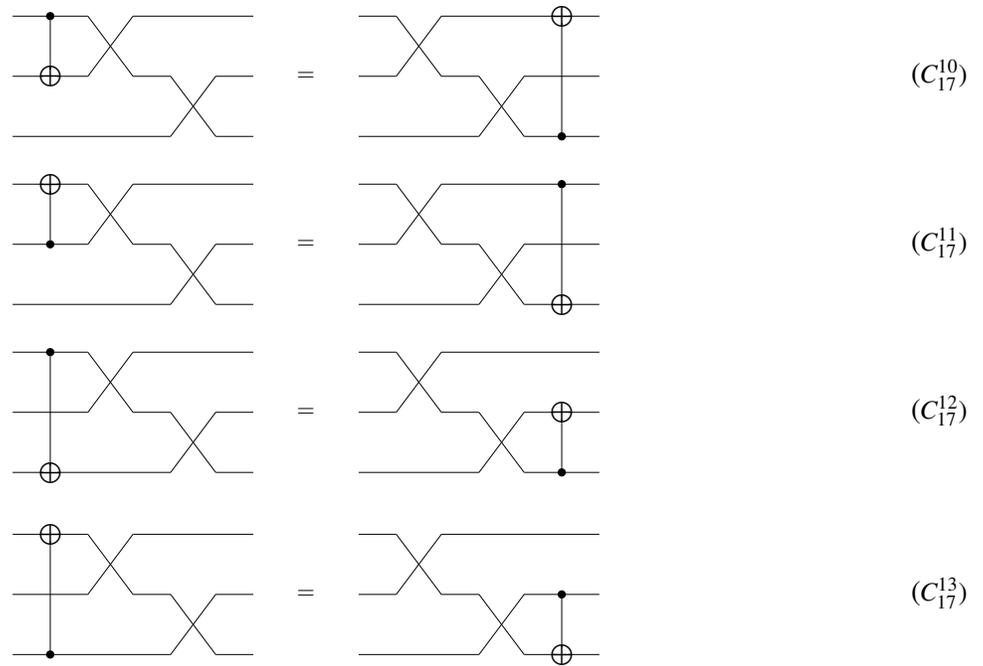

Figure 33: Pushing a CX or XC gate through two stacked SWAP gates, part 2.

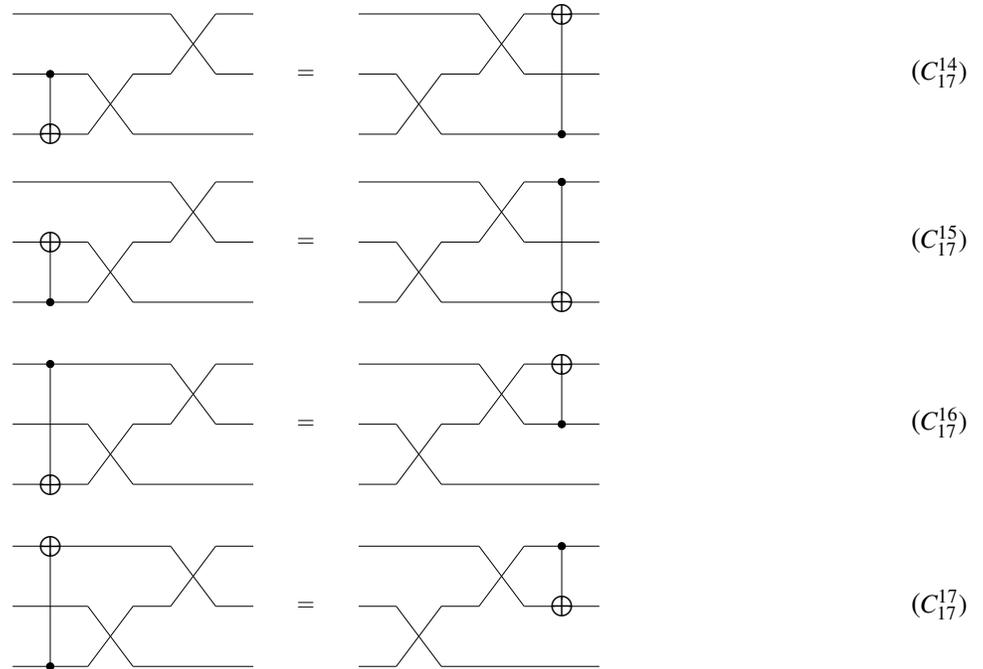

Figure 34: Pushing a CX or XC gate through two stacked SWAP gates, part 3.

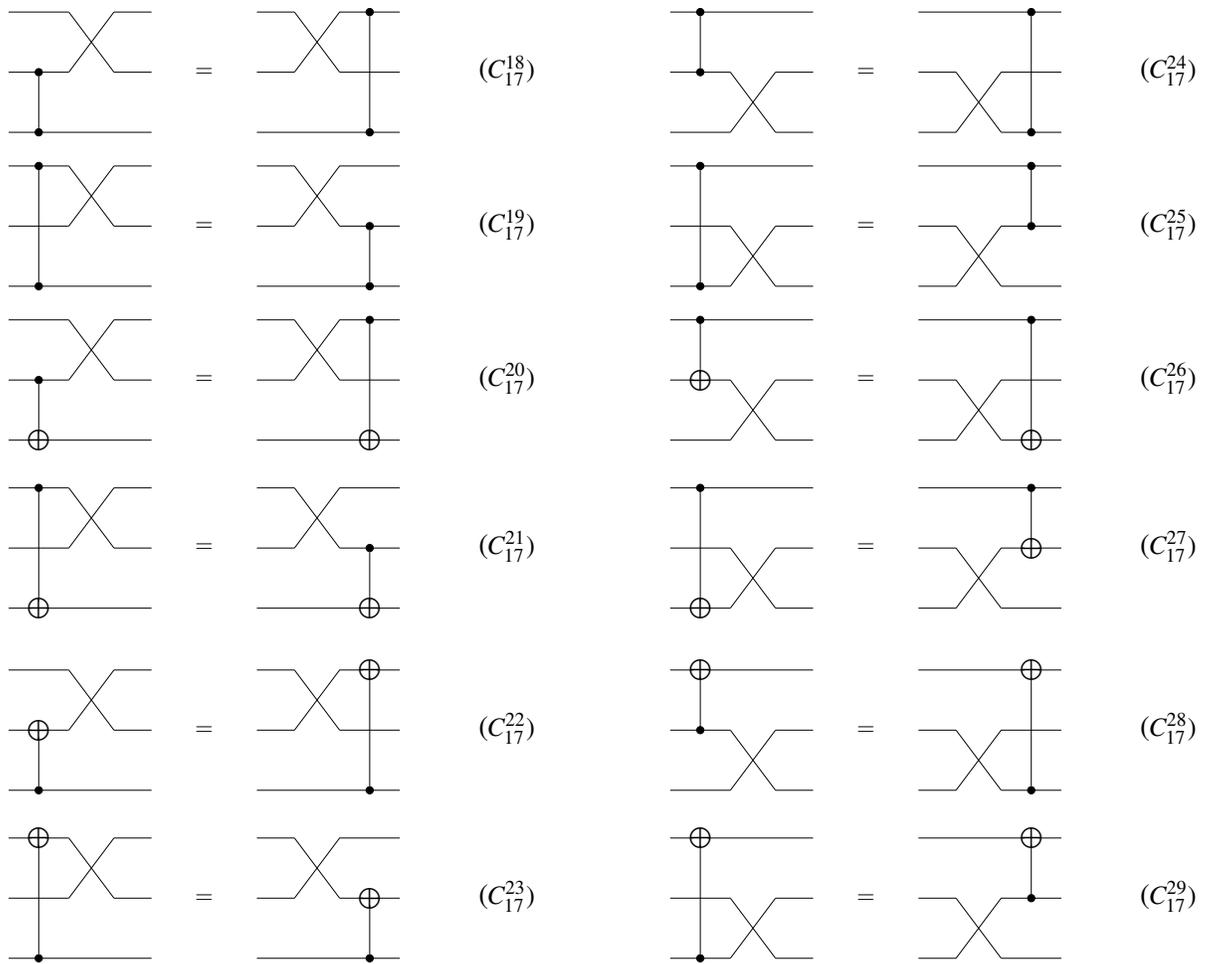

Figure 35: Pushing a CZ, CX or XC gate through a local SWAP gate.

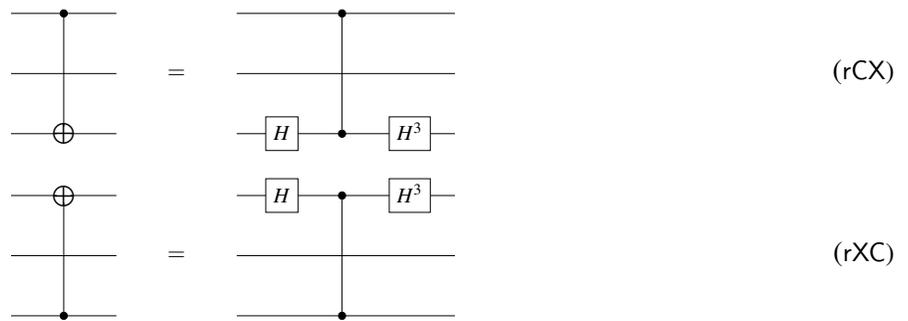

Figure 36: An alternative way to define the remote CX and XC gates.

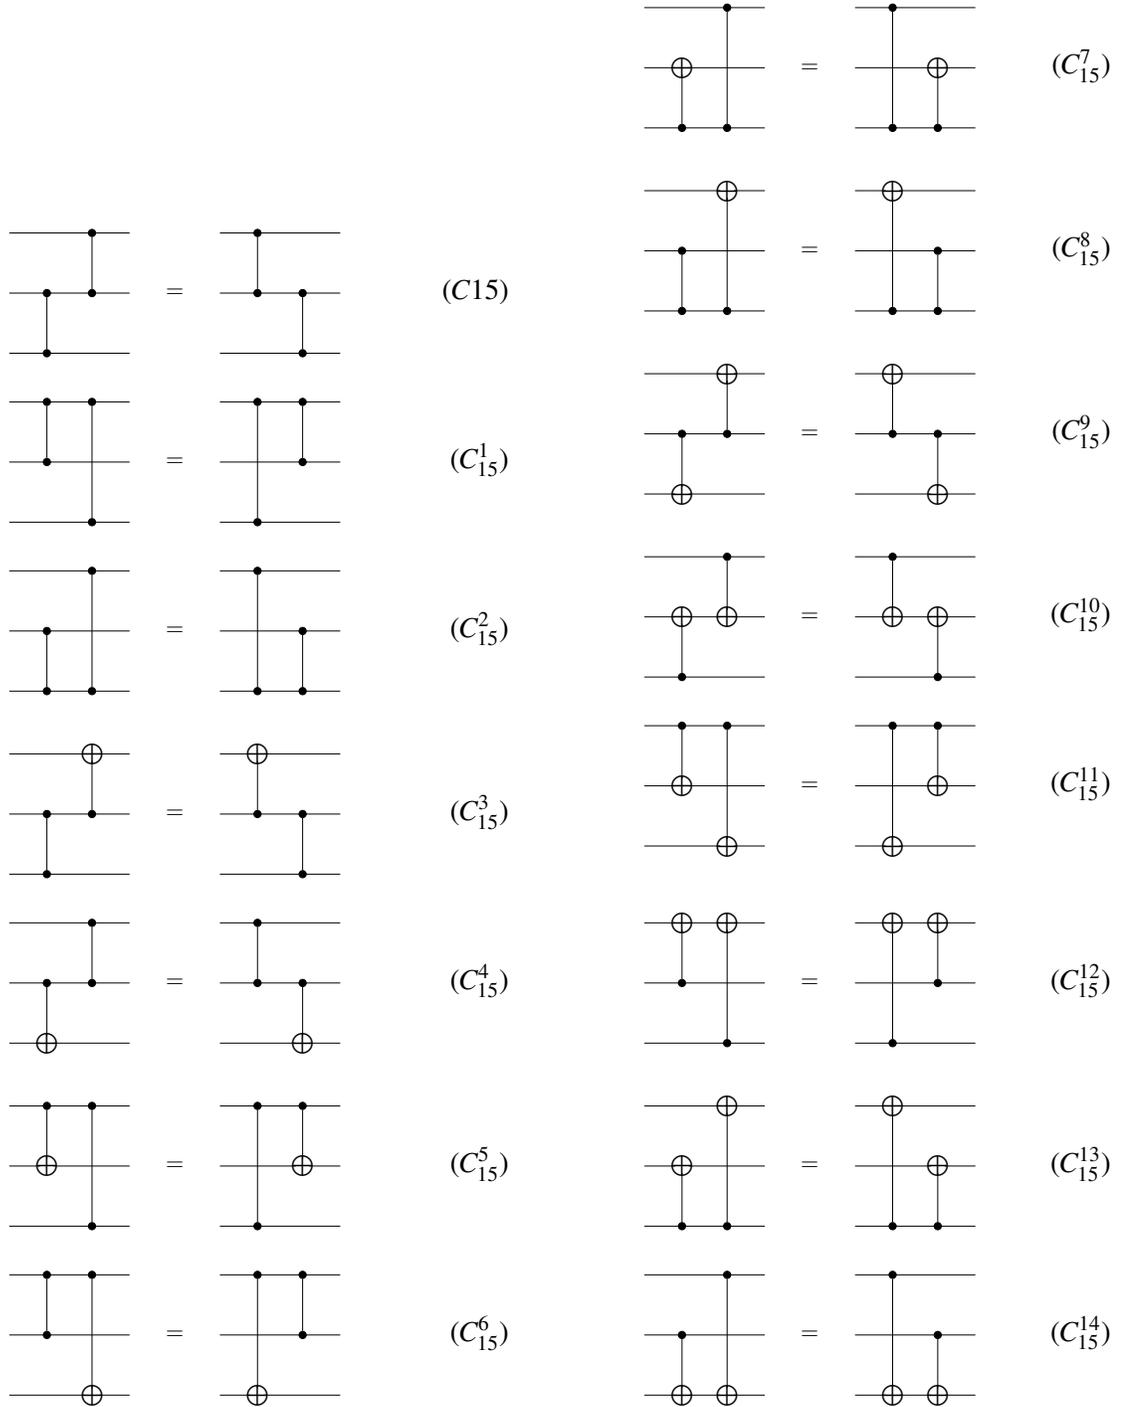

Figure 37: When CZ, CX, and XC commute with each other.

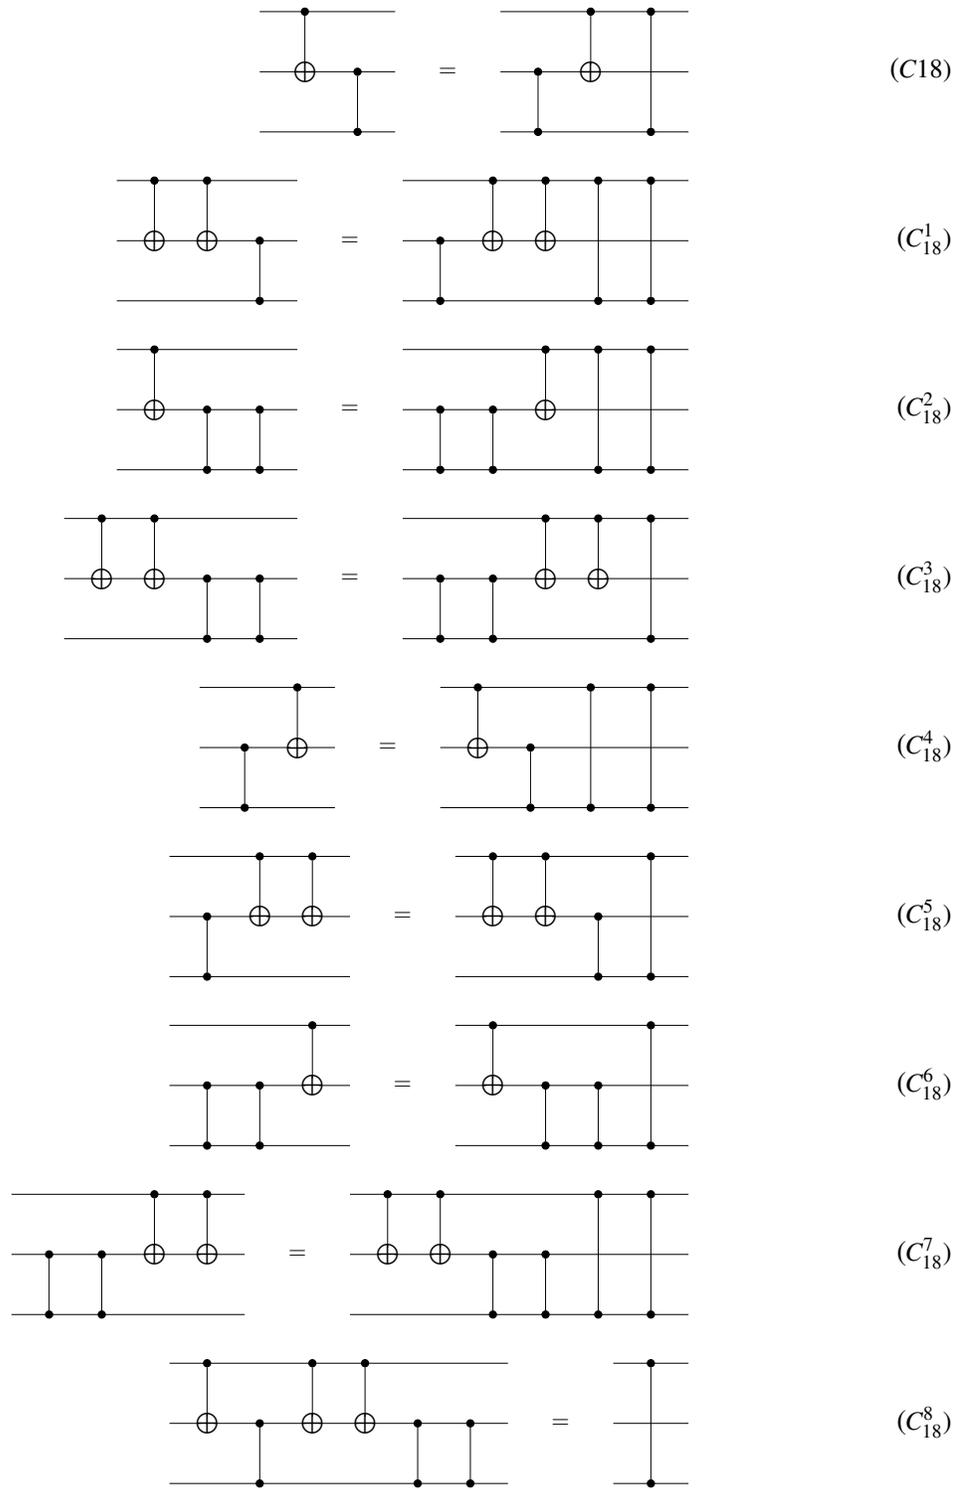

Figure 38: When CX and CZ gates do not commute.

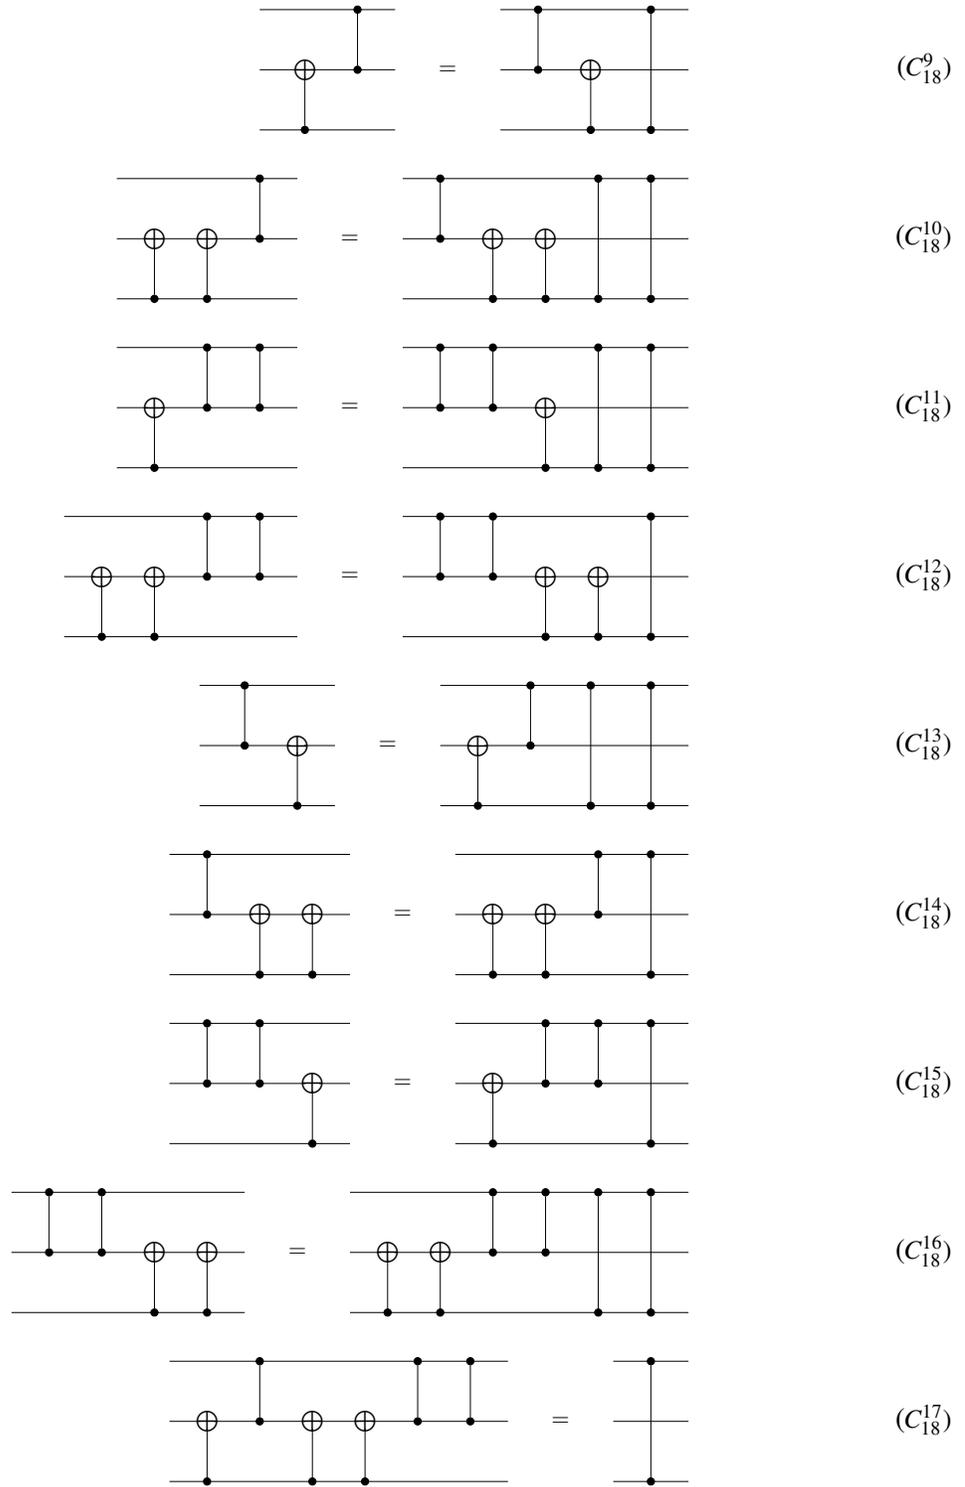

Figure 39: This is the qutrit-permuted variant of [Figure 38](#), corresponding to the case where the XC and CZ gates do not commute. In this variant, qutrit 2 remains unchanged, while the positions of qutrits 1 and 3 are exchanged.

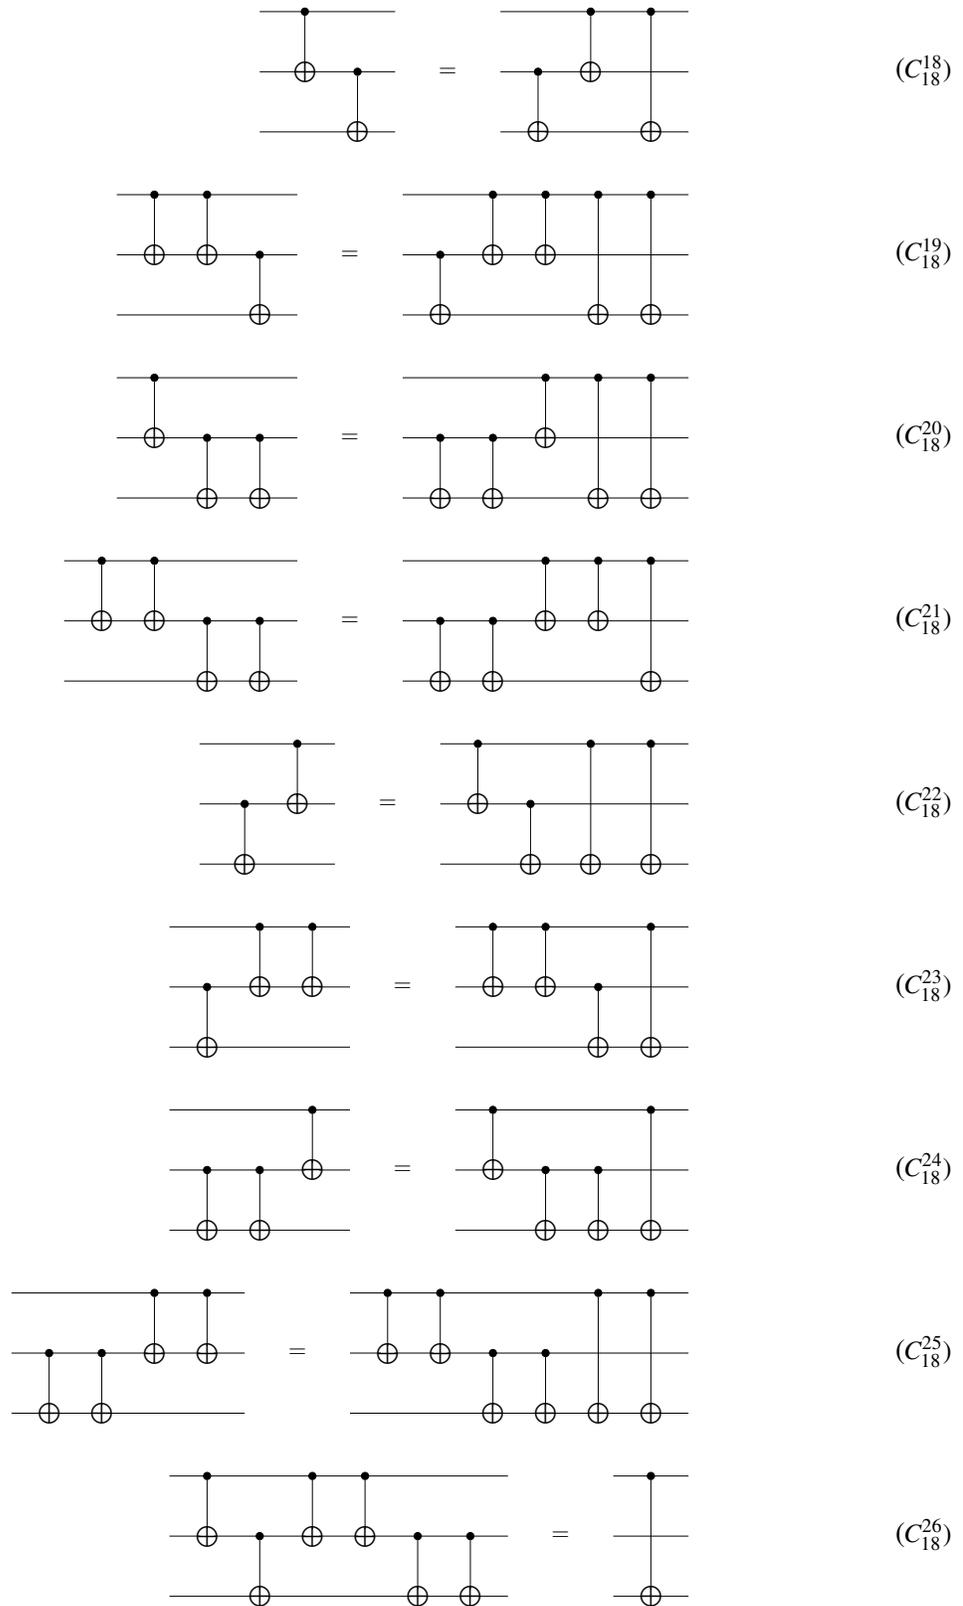

Figure 40: This Hadamard-conjugated variant of [Figure 38](#) corresponds to the case where the CX gates do not commute. Each equation is obtained by conjugating the corresponding equation in [Figure 38](#) with  $I \otimes I \otimes H$ .

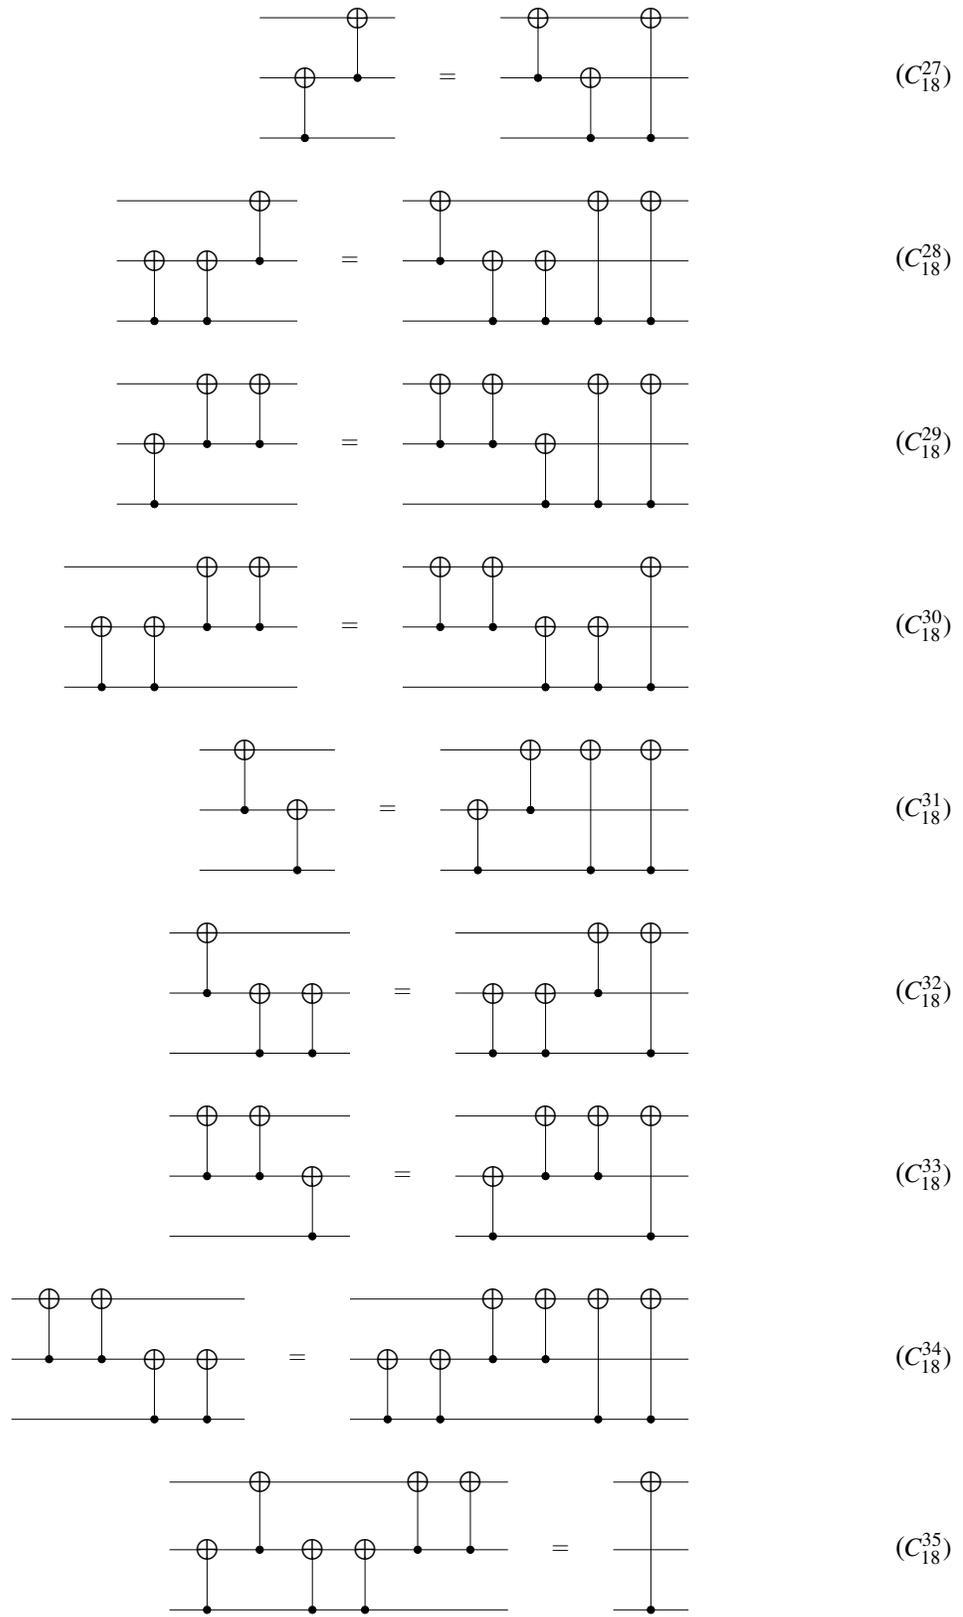

Figure 41: This Hadamard-conjugated variant of Figure 39 corresponds to the case where the XC gates do not commute. Each equation is obtained by conjugating the corresponding equation in Figure 39 with  $H \otimes I \otimes I$ .

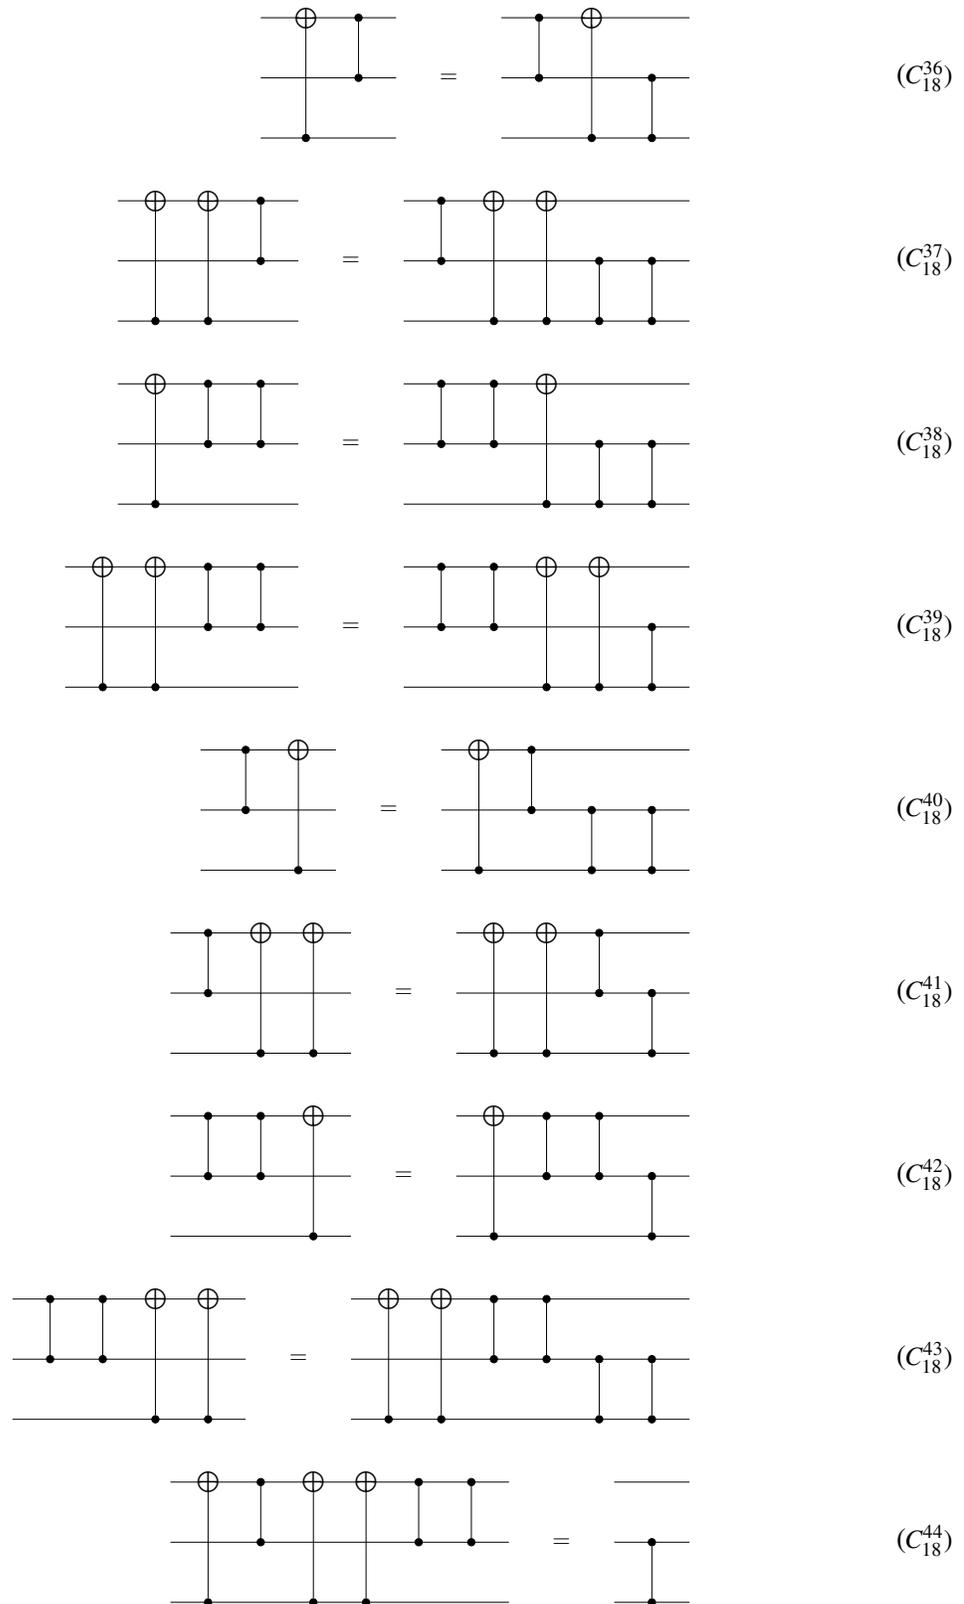

Figure 42: This is the qutrit-permuted variant of [Figure 38](#), corresponding to the case where the XC and CZ gates do not commute. All the qutrits are shifted by one position counter-clockwise (i.e., upward). That is, qutrit 1 is shifted to the position 3, qutrit 2 is shifted to the position 1, and qutrit 3 is shifted to the position 2.

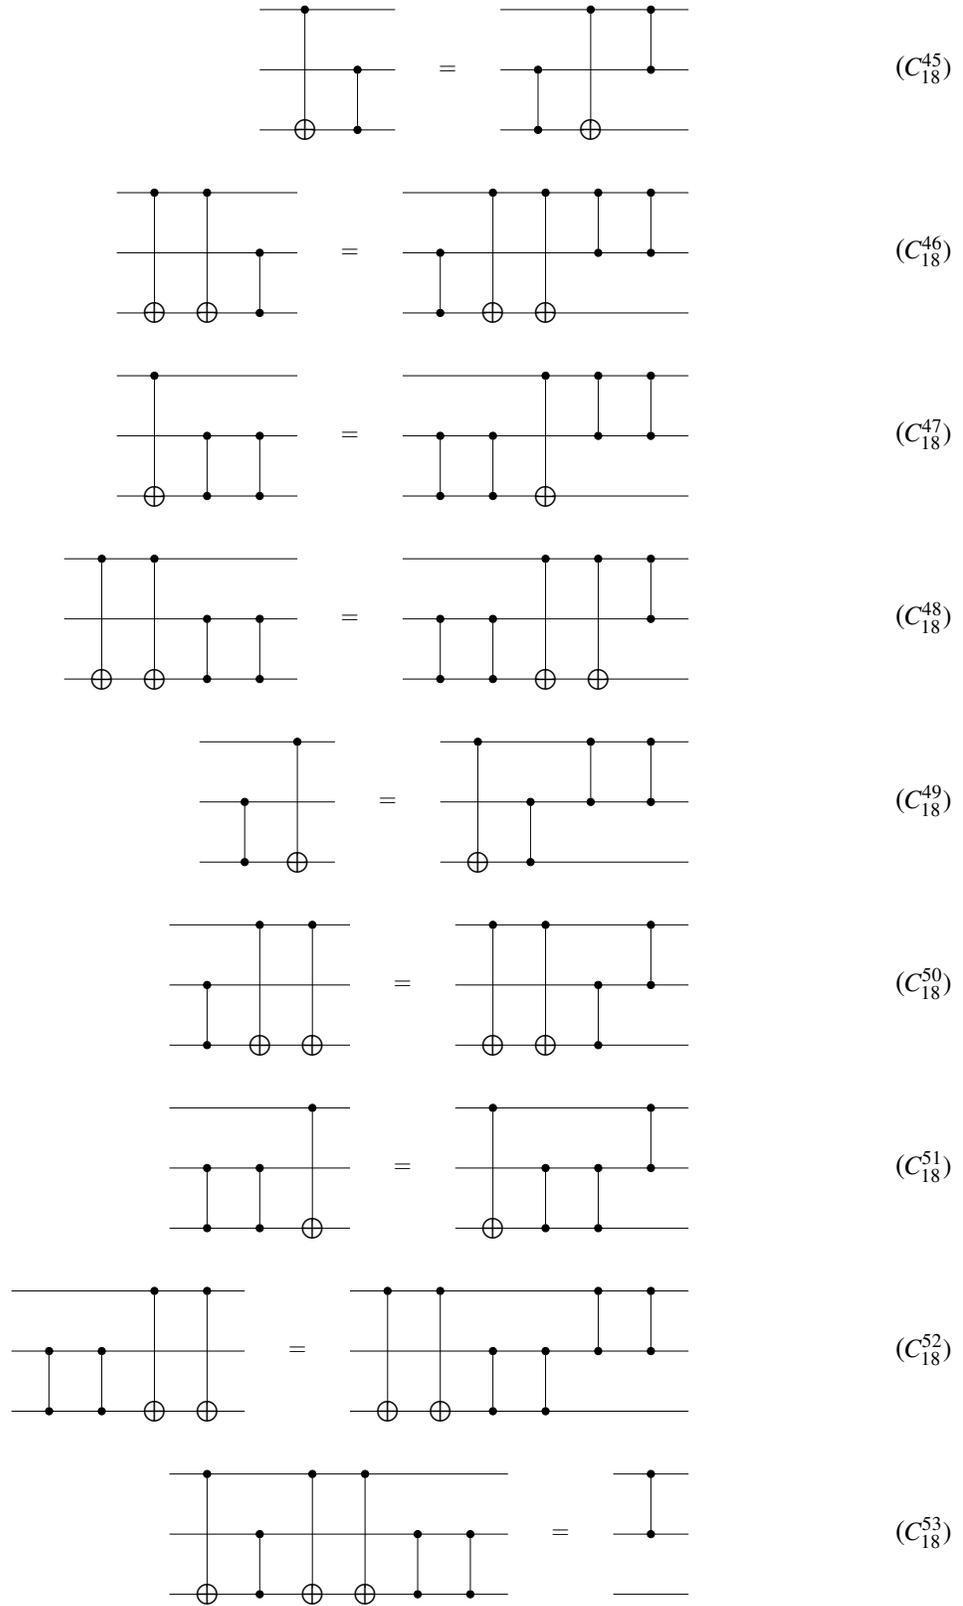

Figure 43: This is the qutrit-permuted variant of Figure 42, corresponding to the case where the CX and CZ gates do not commute. In this variant, qutrit 2 remains unchanged, while the positions of qutrits 1 and 3 are exchanged.

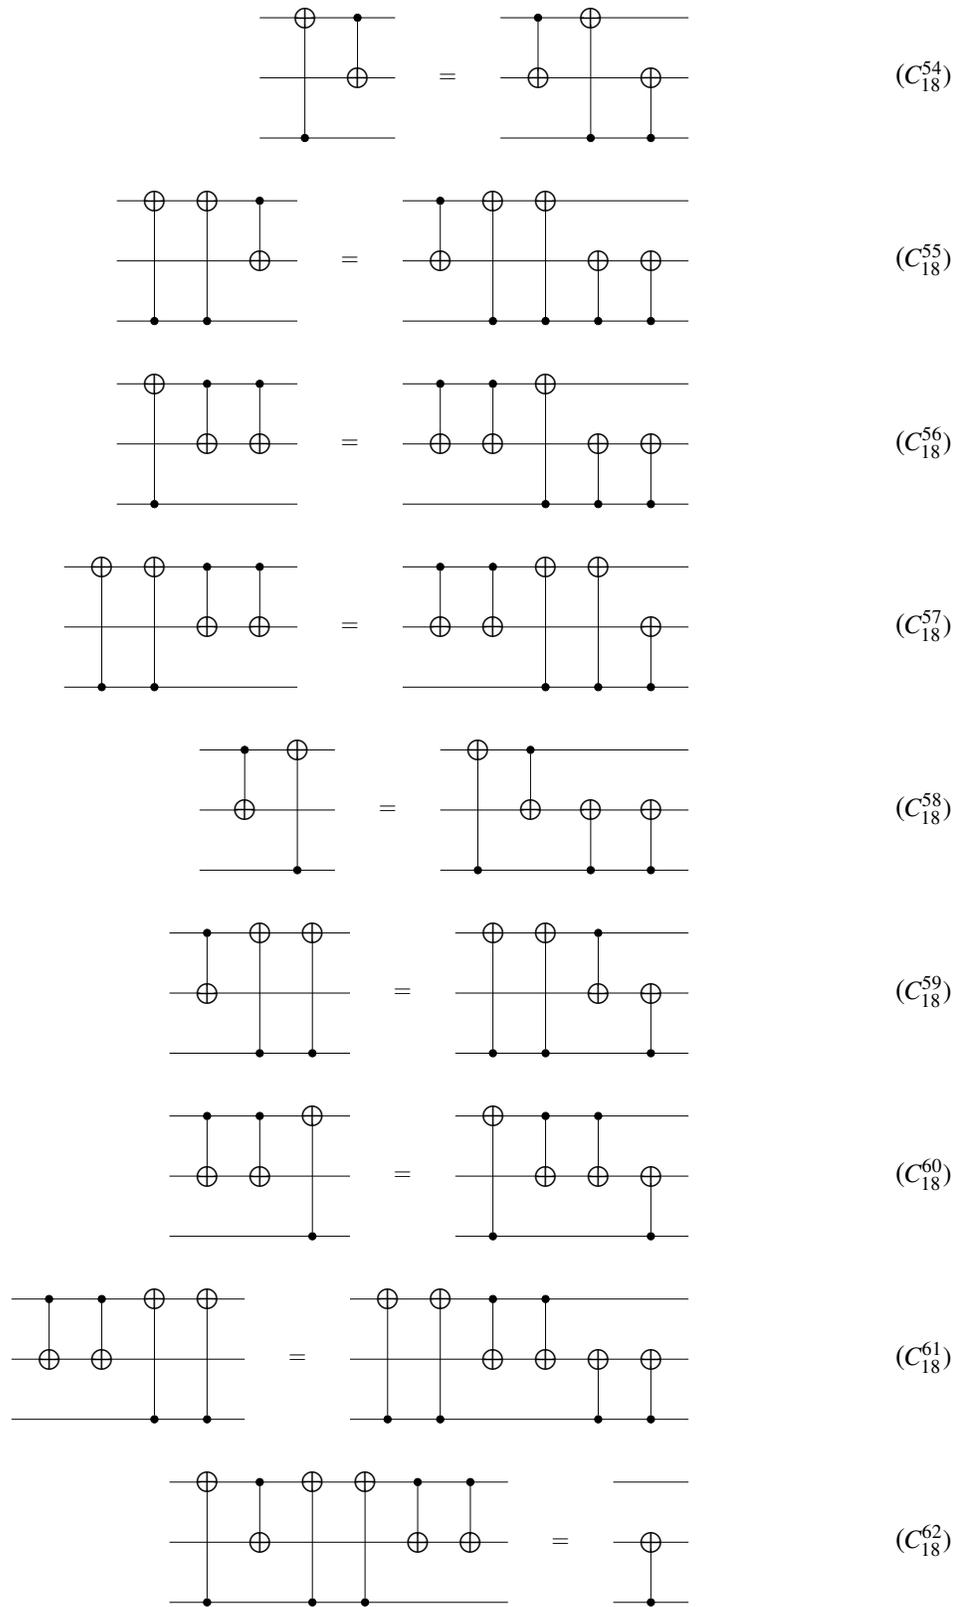

Figure 44: This Hadamard-conjugated variant of [Figure 42](#) corresponds to the case where the CX and XC gates do not commute. Each equation is obtained by conjugating the corresponding equation in [Figure 42](#) with  $I \otimes H \otimes I$ .

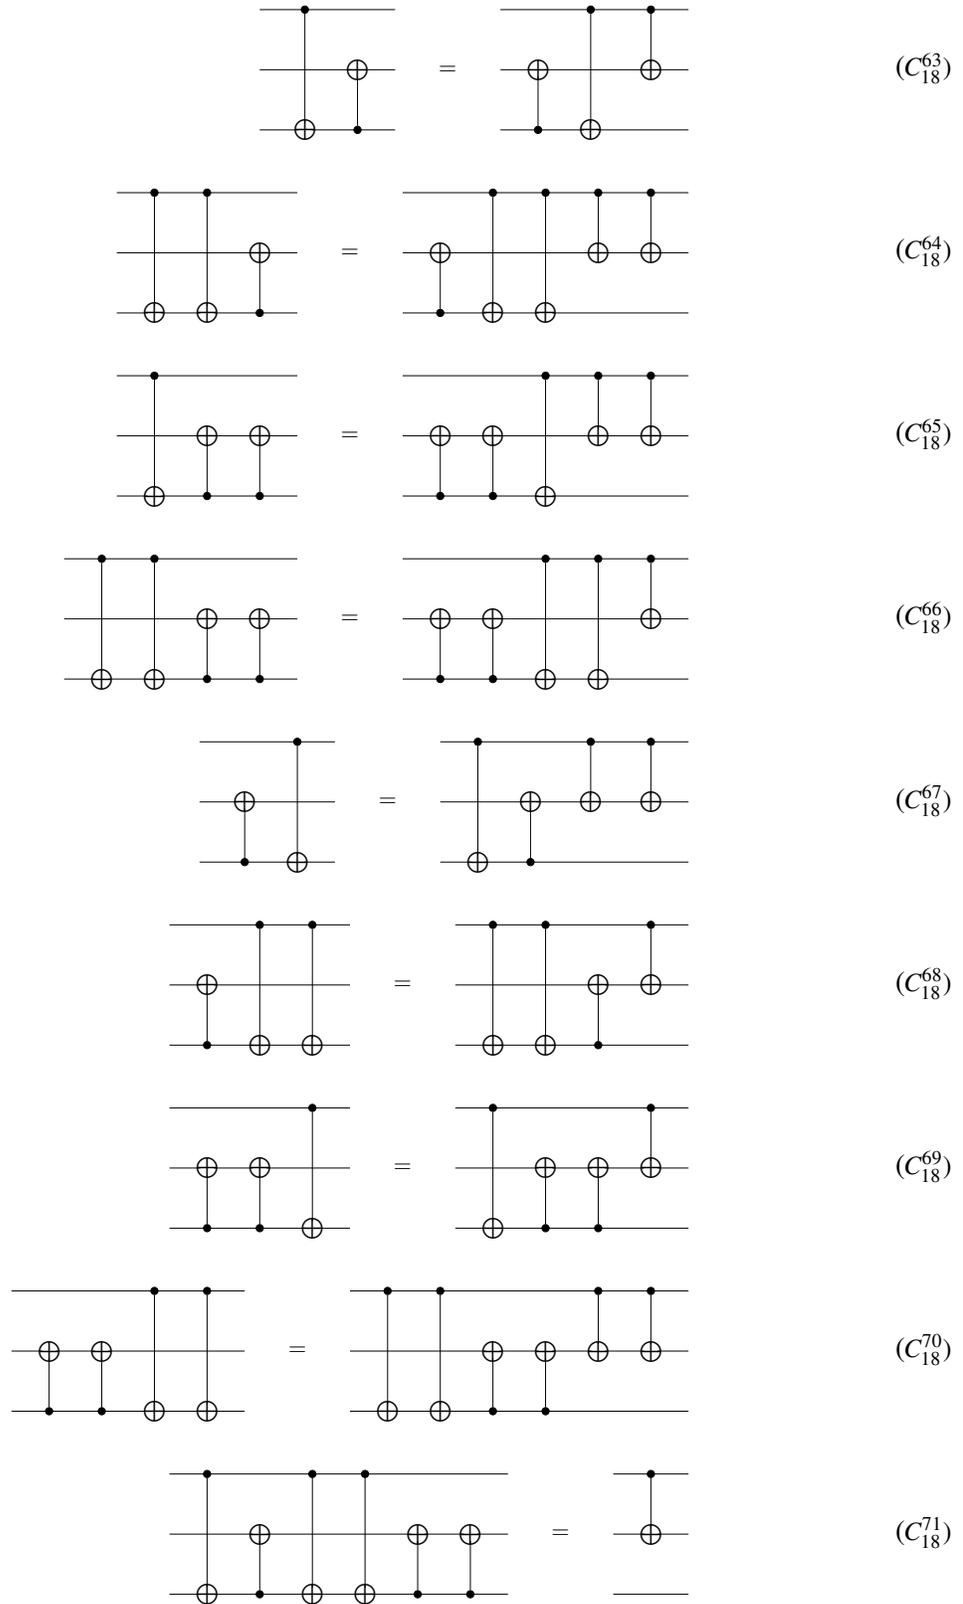

Figure 45: This Hadamard-conjugated variant of [Figure 43](#) corresponds to the case where the CX and XC gates do not commute. Each equation is obtained by conjugating the corresponding equation in [Figure 43](#) with  $I \otimes H \otimes I$ .

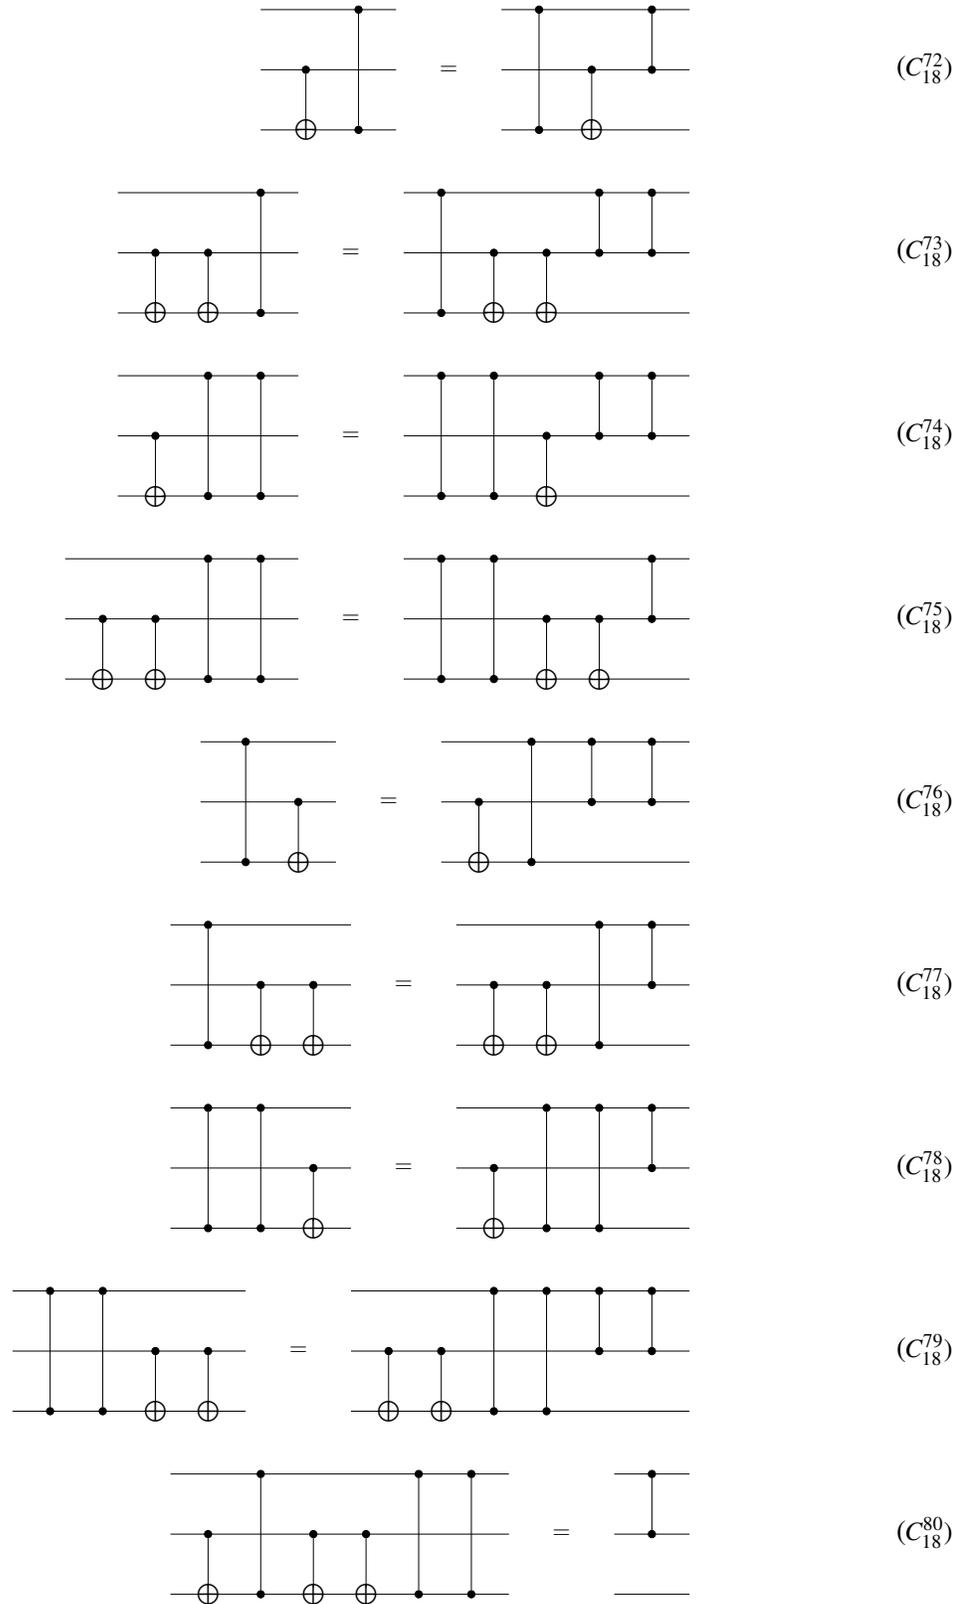

Figure 46: This is the qutrit-permuted variant of [Figure 38](#), corresponding to the case where the CX and CZ gates do not commute. All the qutrits are shifted by one position clockwise (i.e., downward). That is, qutrit 1 is shifted to the position 2, qutrit 2 is shifted to the position 3, and qutrit 3 is shifted to the position 1.

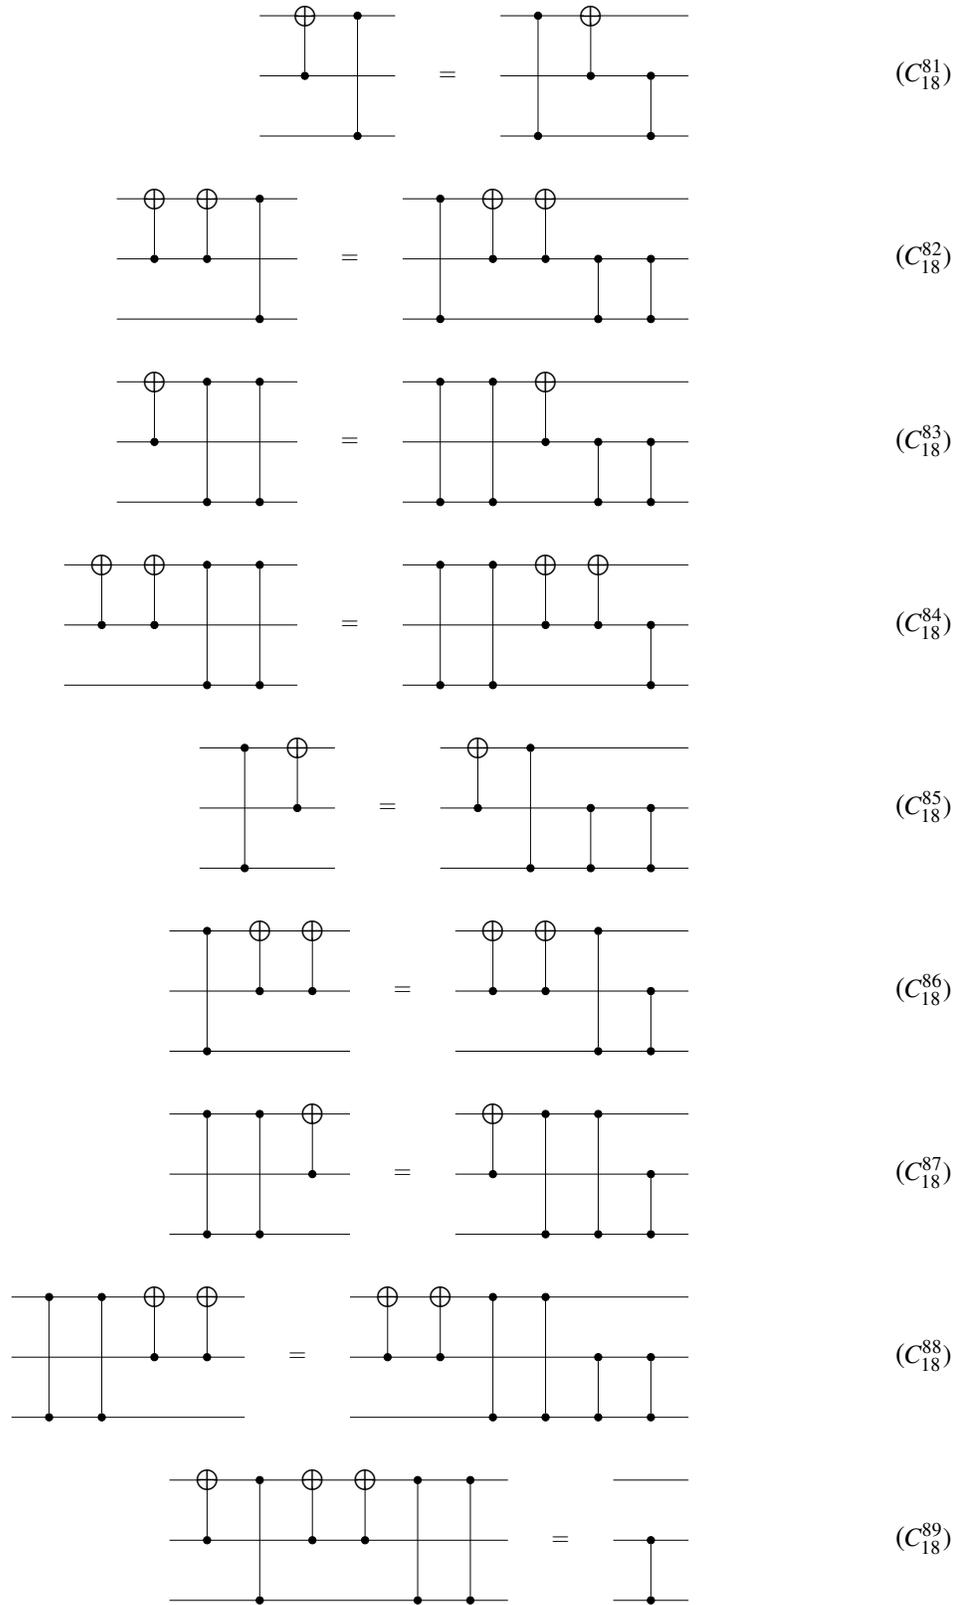

Figure 47: This is the qutrit-permuted variant of Figure 46, corresponding to the case where the XC and CZ gates do not commute. In this variant, qutrit 2 remains unchanged, while the positions of qutrits 1 and 3 are exchanged.

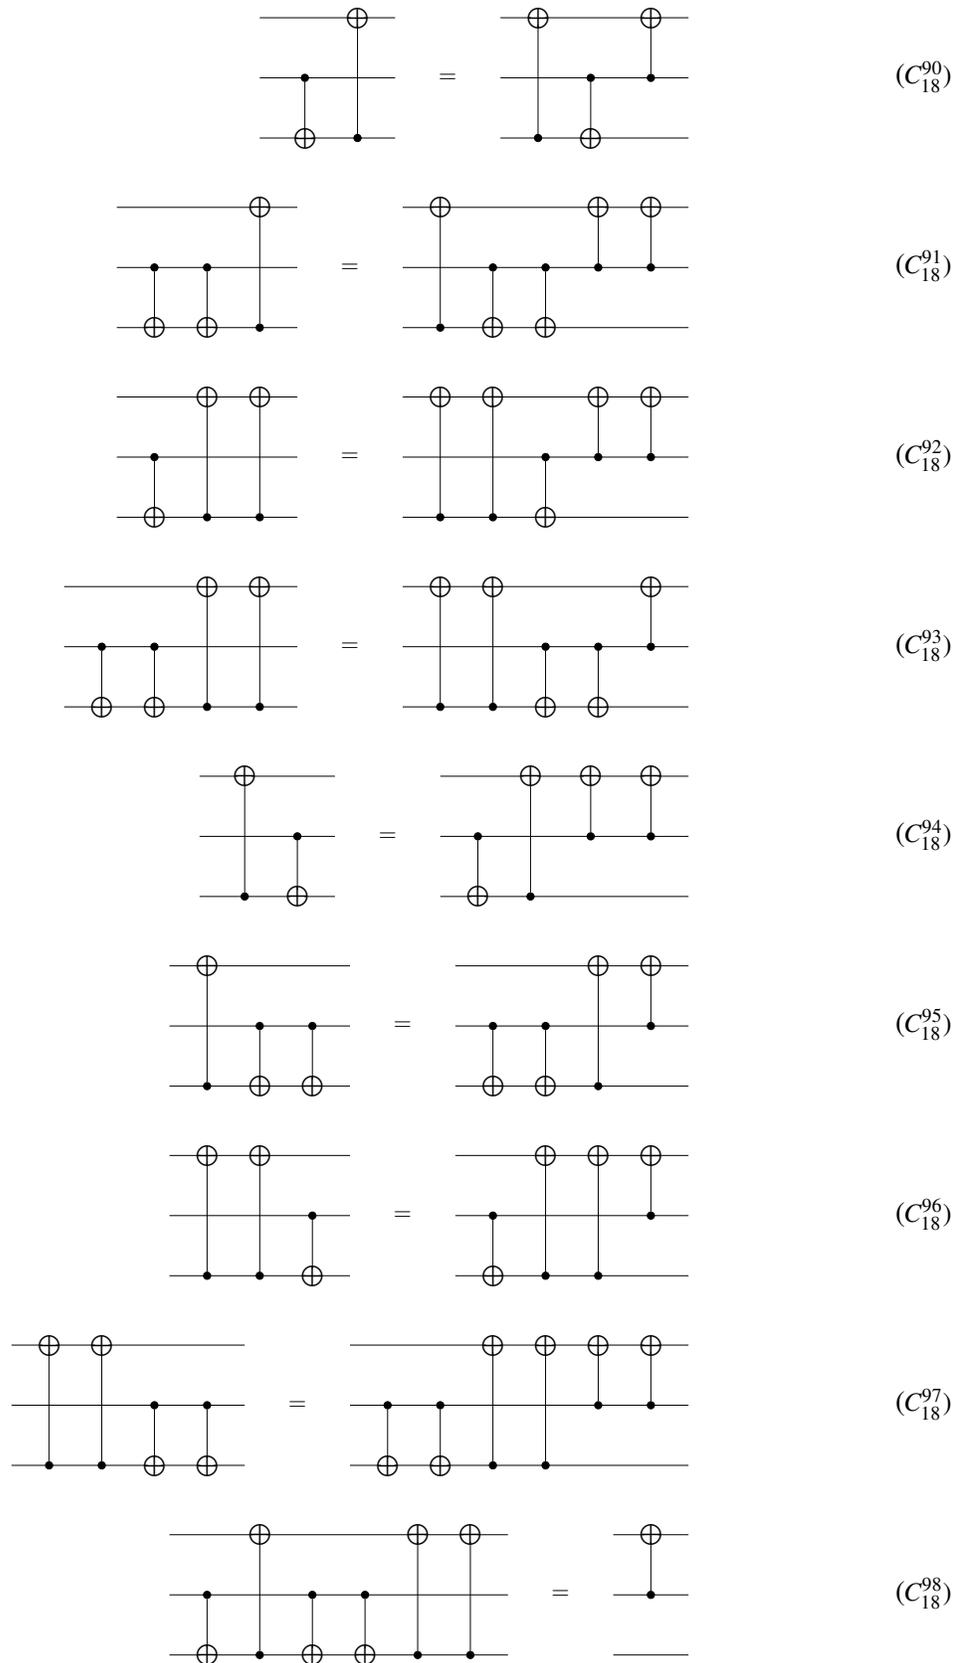

Figure 48: This Hadamard-conjugated variant of [Figure 46](#) corresponds to the case where the CX and XC gates do not commute. Each equation is obtained by conjugating the corresponding equation in [Figure 46](#) with  $H \otimes I \otimes I$ .

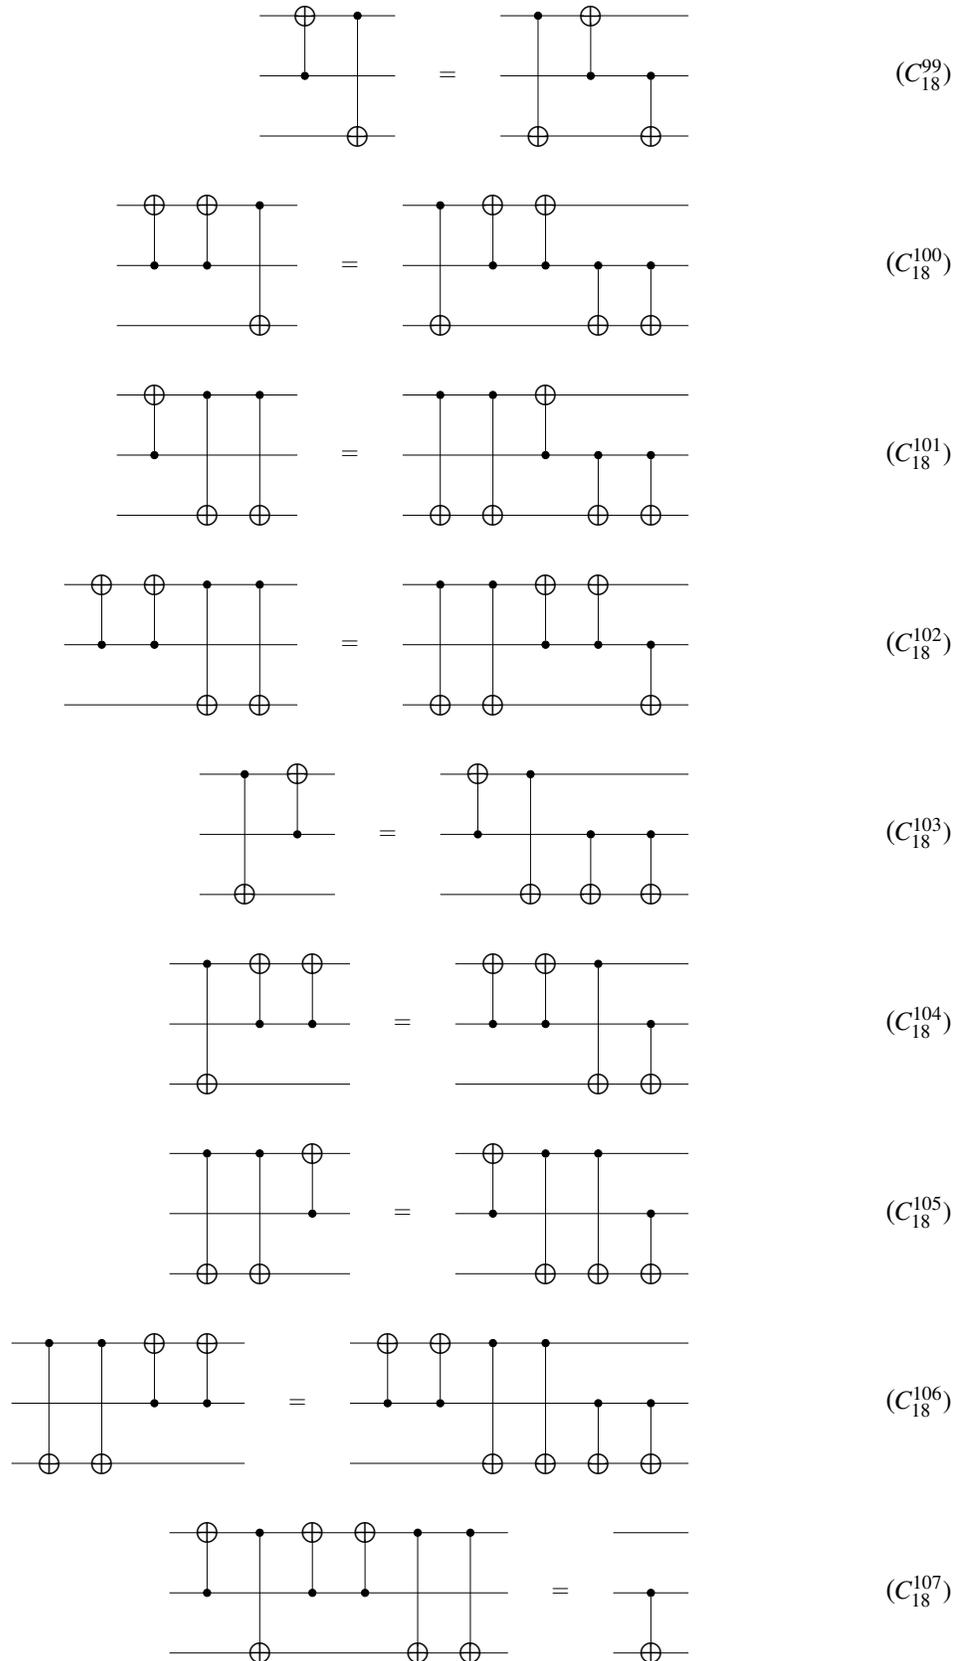

Figure 49: This Hadamard-conjugated variant of [Figure 47](#) corresponds to the case where the CX and XC gates do not commute. Each equation is obtained by conjugating the corresponding equation in [Figure 47](#) with  $I \otimes I \otimes H$ .

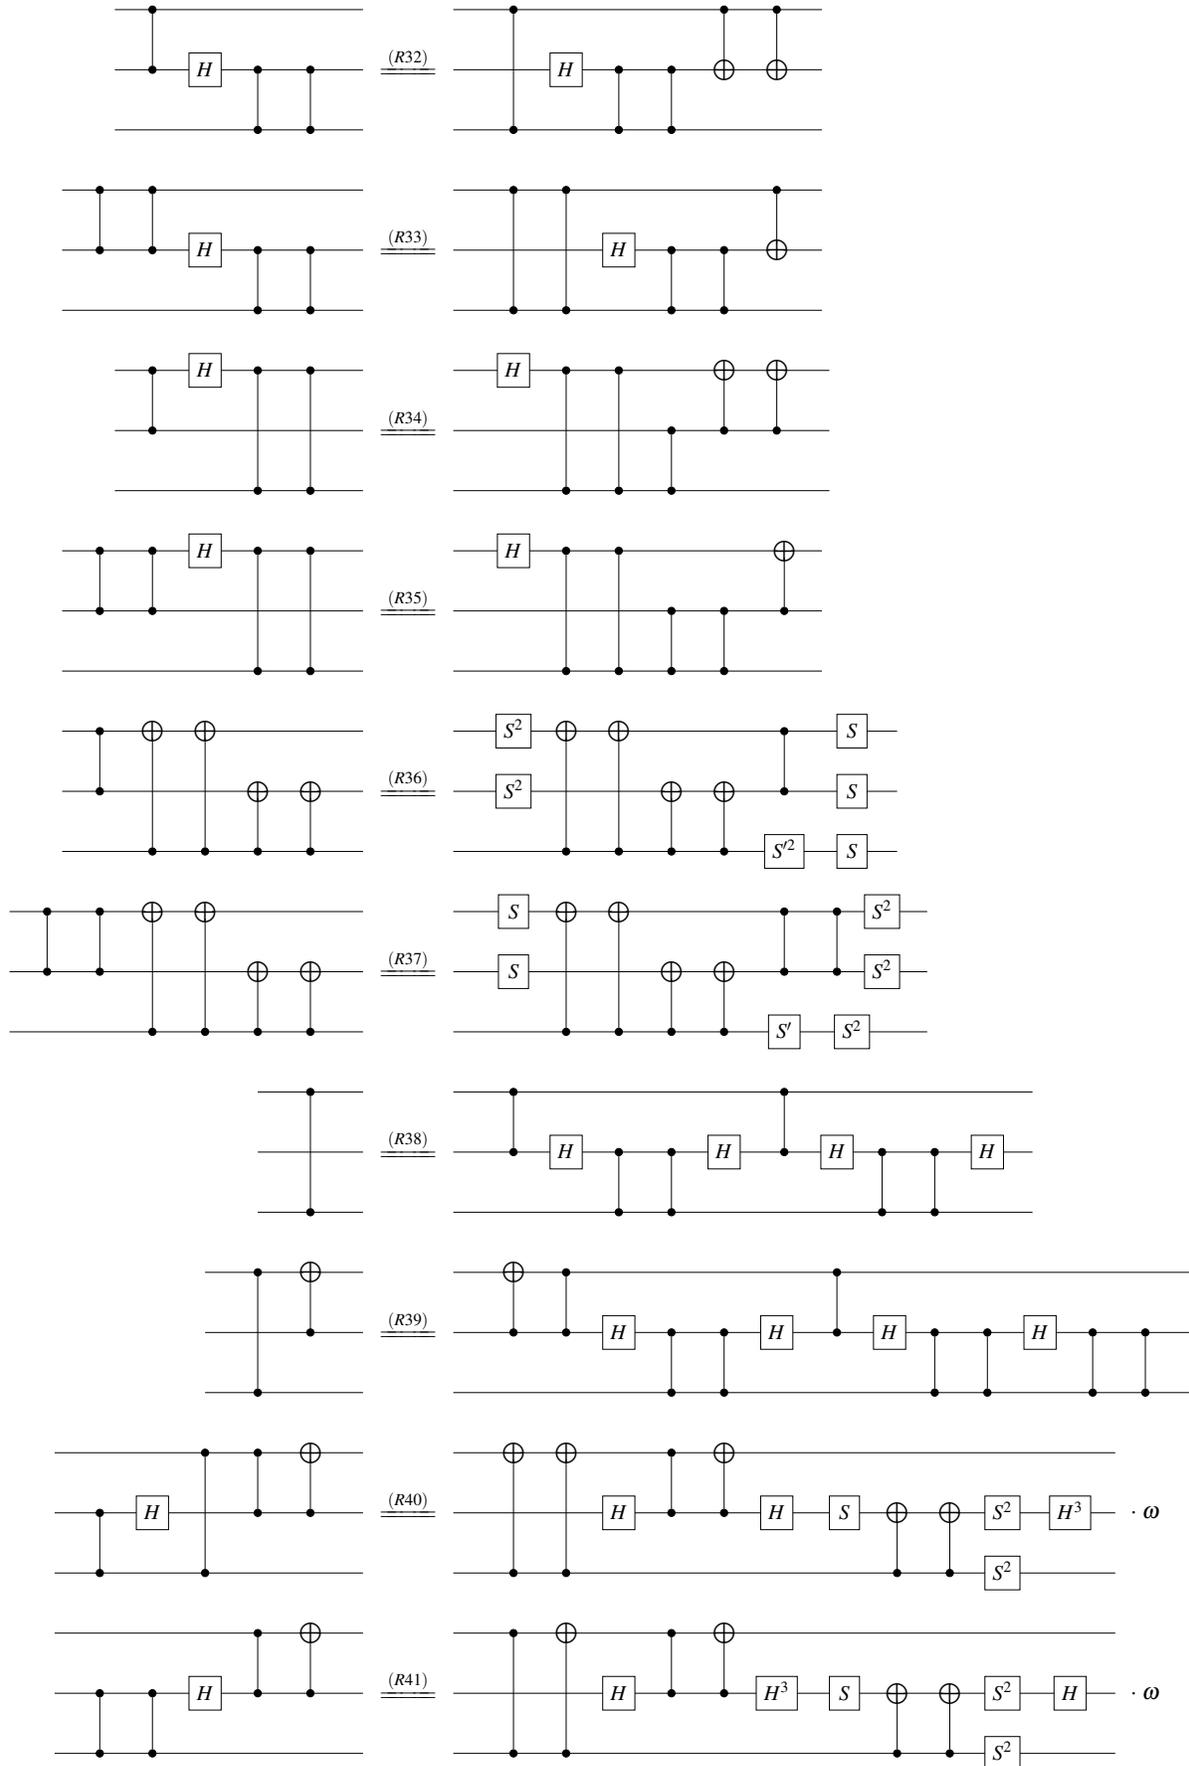

Figure 50: The other three-qutrit derived relations, part 1.

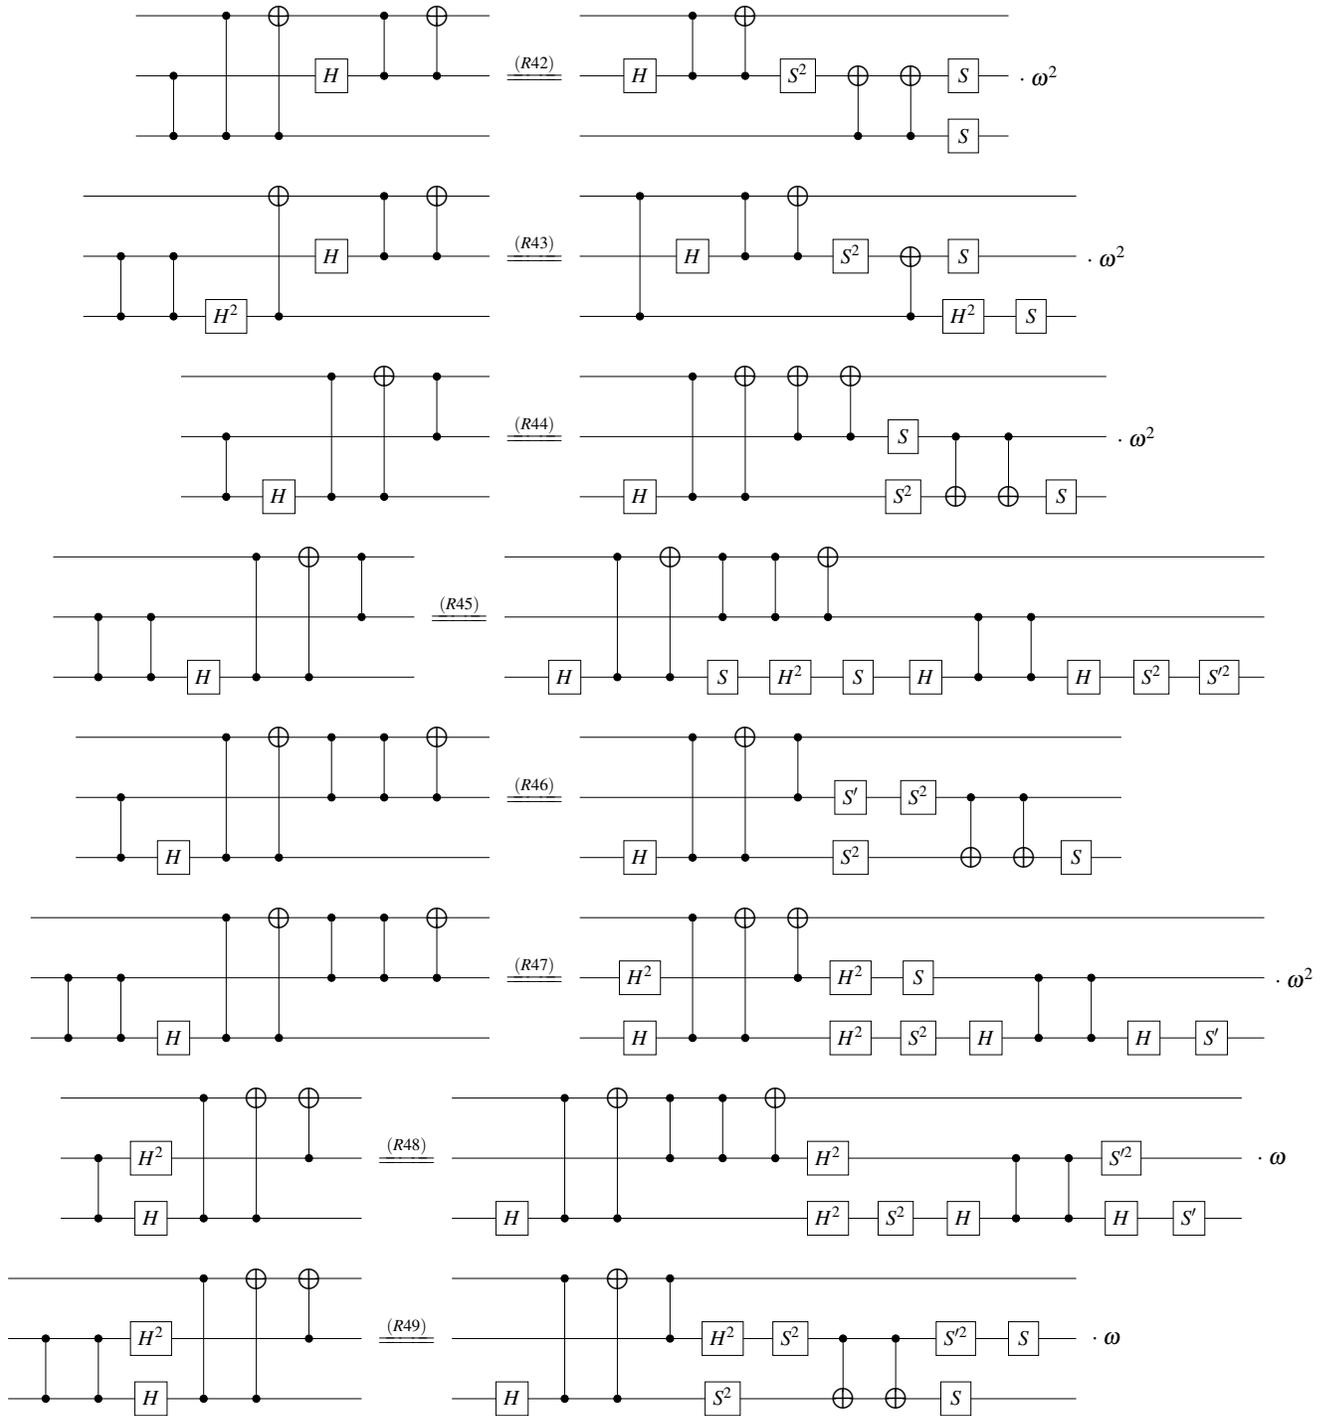

Figure 51: The other three-qutrit derived relations, part 2.

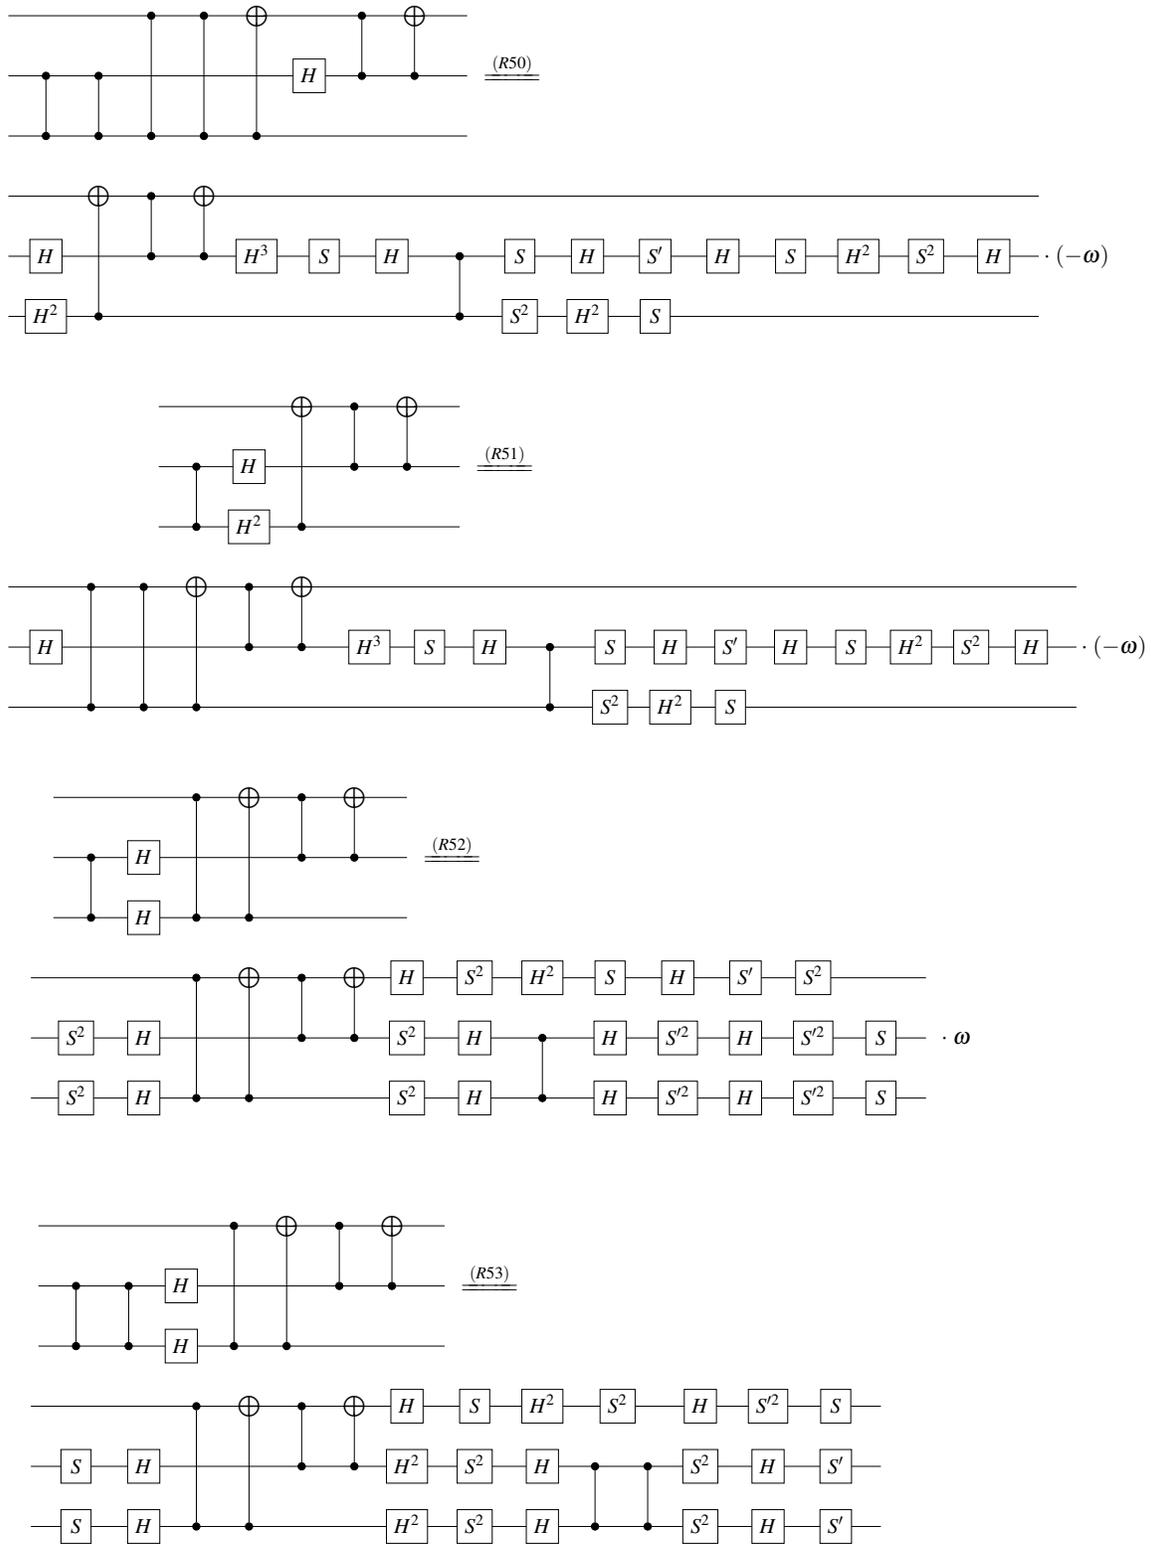

Figure 52: The other three-qutrit derived relations, part 3.

## 2 Single-Qutrit Clifford Completeness

The zero-qutrit box relations in Appendix C.1 follow from (C1) in Figure 54, with (D1) and (D2) in Figure 53.

$$(-1)^2 = 1, \quad \omega^3 = 1. \quad (1)$$

To prove the single-qutrit Clifford completeness, we need to show that the 34 single-qutrit box relations in Appendix C.2 are consequences of the reduced relations in Figure 54 and the derived generator in Figure 53. We proceed in two steps. In Section 2.1, we show that the 12 derived relations in Figure 4 are consequences of the reduced relations in Figure 54 and the derived generators in Figure 53. In Section 2.2, we show that the 34 box relations in Appendix C.2 are consequences of the equations in Figures 4, 53 and 54. The proofs of box relation reductions are summarized in Figure 56. Together, we prove the single-qutrit Clifford completeness, as stated below. Its proof will be presented at the end of this section.

**Theorem 2.1.** *Any true equality between single-qutrit Clifford circuits is provable using the rules in Figure 54 with the derived generators in Figure 53.*

$$-1 = (-\omega)^3 \quad (D1)$$

$$\omega = (-\omega)^4 \quad (D2)$$

$$S' = H^2 S H^2 \quad (D3)$$

$$X = H S H^2 S^2 H \quad (D4)$$

$$Z = H^2 S^2 H^2 S \quad (D5)$$

Figure 53: The single-qutrit derived generators from Figure 2.

$$(-\omega)^6 = 1 \quad (C1)$$

$$H^4 = 1 \quad (C2)$$

$$S^3 = 1 \quad (C3)$$

$$(S^2 H)^3 = -\omega \quad (C4)$$

$$S' S = S S' \quad (C5)$$

Figure 54: The zero- and single-qutrit reduced relations from Figure 1.

In Figures 5 to 7, we derive some useful equations that follow from the equations in Figures 4 and 54. They will be used in Sections 2.1 and 2.2.

**Lemma 2.2.** *The equations in Figure 5 follow from the reduced relations.*

*Proof.* We derive all equations in Figure 5 in order. Recall that

$$(S^2 H)^3 = -\omega \quad (C4)$$

- Right-appending both sides of (C4) by  $H^3SH^3$  yields (C<sub>4</sub><sup>1</sup>):

$$(S^2HS^2HS^2H)(H^3SH^3) = (H^3SH^3) \cdot (-\omega) \xleftrightarrow[(C3)]{(C2)} S^2HS^2 = H^3SH^3 \cdot (-\omega).$$

- Left-appending both sides of (C<sub>4</sub><sup>1</sup>) by  $S$  and right-appending both sides of (C<sub>4</sub><sup>1</sup>) by  $H$  yields:

$$S(S^2HS^2)H = S(H^3SH^3)H \cdot (-\omega) \xleftrightarrow[(C3)]{(C2)} HS^2H = SH^3S \cdot (-\omega). \quad (2)$$

Multiplying both sides of (2) by  $-\omega^2$  yields (C<sub>4</sub><sup>2</sup>):

$$HS^2H \cdot (-\omega^2) = SH^3S \cdot (-\omega) \cdot (-\omega^2) \xleftrightarrow[(D1),(D2)]{((C1))} HS^2H \cdot (-\omega^2) = SH^3S.$$

- Left- and right-appending both sides of (C<sub>4</sub><sup>2</sup>) by  $H^2$  yields (C<sub>4</sub><sup>3</sup>):

$$\begin{aligned} H^2(SH^3S)H^2 &= H^2(HS^2H)H^2 \cdot (-\omega^2) \xleftrightarrow{(C2)} (H^2SH^2)H^3(H^2SH^2) = H(H^2S^2H^2)H \cdot (-\omega^2) \\ &\xleftrightarrow[(D3)]{(C2)} S'H^3S' = HS'^2H \cdot (-\omega^2). \end{aligned}$$

- Left-appending both sides of (C<sub>4</sub><sup>3</sup>) by  $S^2$  yields (C<sub>4</sub><sup>4</sup>):

$$S^2(SH^3S) = S^2(HS^2H) \cdot (-\omega^2) \xleftrightarrow{(C3)} H^3S = S^2HS^2H \cdot (-\omega^2).$$

Recall that

$$S'S = SS' \quad (C5)$$

Left-appending both sides of (C5) by  $H^2$  yields (C<sub>5</sub><sup>1</sup>):

$$H^2(S'S) = H^2(SS') \xleftrightarrow{(D3)} H^2(H^2SH^2)S = H^2S(H^2SH^2) \xleftrightarrow{(C2)} SH^2S = H^2SH^2SH^2. \quad \square$$

## 2.1 Reduce the Single-Qutrit Derived Relations

Here, we show that the 12 derived relations in Figure 4 follow from the reduced relations in Figure 54 and the derived generators in Figure 53.

**Lemma 2.3.** (R1) to (R10) in Figure 4 follow from the reduced relations.

*Proof.* We derive (R1) to (R10) from equations in Figures 53 and 54 one after the other.

$$(R1).LHS = S'^3 \xleftrightarrow[(C3)]{(D3)} (H^2SH^2)(H^2SH^2)(H^2SH^2) \xleftrightarrow{(C2)} 1 = (R1).RHS.$$

$$\begin{aligned} (R2).LHS &= X^2 \xleftrightarrow{(D4)} (HSH^2S^2H)(HSH^2S^2H) = HSH^2S^2(H^2SH^2)S^2H \xleftrightarrow{(D3)} HSH^2S^2(S')S^2H \\ &\xleftrightarrow[(C3)]{(C5)} HSH^2S'SH \xleftrightarrow{(D3)} HSH^2(H^2SH^2)SH \xleftrightarrow{(C2)} HS^2H^2SH = (R2).RHS. \end{aligned}$$

$$(R3).LHS = X^3 \xrightarrow[(R2)]{(D4)} (HS^2H^2SH)(HSH^2S^2H) = HS^2H^2SH^2S^2H \xrightarrow{(D3)} HS^2H^2S(S')S^2H \\ \xrightarrow[(C3)]{(C5)} HS^2H^2S'H \xrightarrow{(D3)} HS^2H^2(H^2SH^2)H \xrightarrow[(C3)]{(C2)} HS^2SH^3 \xrightarrow{(C3)} 1 = (R3).RHS.$$

$$(R4).LHS = Z \xrightarrow{(D5)} H^2S^2H^2S \xrightarrow[(C2)]{(D3)} S'^2S = (R4).RHS.$$

$$(R5).LHS = Z^2 \xrightarrow{(R4)} (S'^2S)(S'^2S) \xrightarrow[(R1)]{(C5)} S'S^2 = (R5).RHS.$$

$$(R6).LHS = Z^3 \xrightarrow[(R5)]{(R4)} (S'^2S)(S'^2S) \xrightarrow[(R1)]{(C5)} (S'^3)(S^3) \xrightarrow{(C3)} 1 = (R6).RHS.$$

$$(R7).RHS = S^2HS^2X^2 \cdot (-\omega^2) \xrightarrow{(R2)} S^2HS^2(HS^2H^2SH) \cdot (-\omega^2) \xrightarrow{(C_4^1)} (H^3SH^3)(HS^2H^2SH) \cdot (-\omega^2) \cdot (-\omega) \\ \xrightarrow[(C1),(C2)]{(D1),(D2)} H^3SS^2H^2SH \xrightarrow[(C3)]{(C2)} HSH = (R7).LHS.$$

$$(R8).RHS = H^2SZ^2 \xrightarrow{(R5)} H^2S(S'^2S) \xrightarrow[(D3)]{(C5)} H^2(SS^2)S' \xrightarrow[(D3)]{(C3)} H^2(H^2SH^2) \xrightarrow{(C2)} SH^2 = (R8).LHS.$$

$$(R9).LHS = SZ \xrightarrow{(R4)} S(S'^2S) \xrightarrow[(C5)]{(C5)} (S'^2S)S \xrightarrow{(R4)} ZS = (R9).RHS.$$

$$(R10).LHS = Z^2H \xrightarrow{(R5)} S'S^2H \xrightarrow[(D3)]{(C5)} SS'SH \xrightarrow[(D3)]{(C2)} H^2H^2S(H^2SH^2)SH \xrightarrow{(C_5^1)} H^2(SH^2S)SH \\ \xrightarrow{(D4)} HX = (R10).RHS. \quad \square$$

Next, we show that the equations in [Figures 6](#) and [7](#) follow from the equations in [Figures 53](#) and [54](#). These derived relations will be used in [Lemmas 2.6](#) and [2.7](#).

**Lemma 2.4.** *The equation in [Figure 6](#) follows from the reduced relations.*

*Proof.* Recall that

$$HSH = S^2HS^2X^2 \cdot (-\omega^2) \quad (R7)$$

Left-appending both sides of [\(R7\)](#) by H yields:

$$H^2SH = HS^2HS^2X^2 \cdot (-\omega^2). \quad (3)$$

Right-appending both sides of [\(3\)](#) by XS yields:

$$(H^2SH)XS = (HS^2HS^2X^2)XS \cdot (-\omega^2) \xrightarrow[(C3)]{(R3)} H^2SHXS = HS^2H \cdot (-\omega^2). \quad (4)$$

Multiplying both sides of [\(4\)](#) by  $-\omega$  yields [\(R\\_7^1\)](#):

$$H^2SHXS \cdot (-\omega) = HS^2H \cdot (-\omega^2) \cdot (-\omega) \xrightarrow[(C1)]{(D1),(D2)} H^2SHXS \cdot (-\omega) = HS^2H. \quad \square$$

**Lemma 2.5.** *The equations in Figure 7 follow from the reduced relations.*

*Proof.* We derive  $(R_{10}^1)$  and  $(R_{10}^2)$  from equations in Figures 53 and 54 one after the other. Recall that

$$Z^2H = HX \quad (R10)$$

- To show that  $(R_{10}^1)$  is a consequence of  $(R10)$ , by  $(C2)$ , it suffices to show

$$XH = HZ. \quad (5)$$

$$(5).\text{LHS} = XH \xrightarrow{(D4)} (HSH^2S^2H)H \xrightarrow[(C2)]{(D3)} HSS'^2 \xrightarrow[(C5)]{(R4)} HZ = (5).\text{RHS}.$$

- $(R_{10}^2).\text{LHS} = HZ^2H^3 \xrightarrow{(C2)} (HZH^3)(HZH^3) \xrightarrow{(R_{10}^1)} X^2 = (R_{10}^2).\text{RHS}$ .  $\square$

Finally, we show that  $(R11)$  and  $(R12)$  follow from the reduced relations.

**Lemma 2.6.**  $(R11)$  follows from the reduced relations.

*Proof.* Note that

$$SX \xrightarrow{\text{WTS}} XZS \cdot \omega^2 \quad (R11)$$

By the equations in Figures 53 and 54, it suffices to show

$$SXZ^2S^2X^2 \cdot \omega \xrightarrow{\text{WTS}} 1. \quad (6)$$

$$(6).\text{LHS} = SXZ^2S^2X^2 \cdot \omega$$

$$\begin{aligned} & \xrightarrow[(R_{10}^2)]{(R_{10}^1)} S(HZH^3)Z^2S^2(HZ^2H^3) \cdot \omega \\ & \xrightarrow[(R5)]{(R4)} SH(S'^2S)H^3(S'S^2)S^2H(S'S^2)H^3 \cdot \omega \\ & \xrightarrow[(C5)]{(C3)} SHS'^2(SH^3S)S'HS'S^2H^3 \cdot \omega \\ & \xrightarrow{(C_4^2)} SHS'^2(HS^2H)S'HS'S^2H^3 \cdot \omega \cdot (-\omega^2) \\ & \xrightarrow[(D2),(D3)]{(C1),(D1)} SH(H^2S^2H^2)(HS^2H)(H^2SH^2)H(H^2SH^2)S^2H^3 \cdot (-1) \\ & \xrightarrow{(C2)} SH^3S^2H^3S^2H^3SHSH^2S^2H^3 \cdot (-1) = S(H^3S)S(H^3S)S(H^3S)HSH^2S^2H^3 \cdot (-1) \\ & \xrightarrow{(C_4^1)} S(S^2HS^2H)S(S^2HS^2H)S(S^2HS^2H)(HSH^2S^2H^3) \cdot (-1) \cdot (-\omega^2)^3 \\ & \xrightarrow[(C1),(C3)]{(D1),(D2)} (HS^2H)(HS^2H)(HS^2H)(HSH^2S^2H^3) = HS^2(H^2S^2H^2)S^2(H^2SH^2)S^2H^3 \\ & \xrightarrow[(D3)]{(C2)} HS^2S'^2S^2S'S^2H^3 \xrightarrow[(C3)]{(C5)} H(S^2S^2S^2)(S'^2S')H^3 \xrightarrow{(R1)} HH^3 \xrightarrow{(C2)} 1 = (6).\text{RHS}. \quad \square \end{aligned}$$

**Lemma 2.7.**  $(R12)$  follows from the reduced relations.

*Proof.* Note that

$$ZX \stackrel{\text{WTS}}{=} XZ \cdot \omega^2 \quad (\text{R12})$$

By (R3) and (R6), it suffices to show

$$XZX^2Z^2 \cdot \omega^2 \stackrel{\text{WTS}}{=} 1. \quad (7)$$

$$\begin{aligned} (7).\text{LHS} &= XZX^2Z^2 \cdot \omega^2 \\ &\stackrel{(R_{10}^1)}{\stackrel{(R_{10}^2)}{=}} (HZH^3)Z(HZ^2H^3)Z^2 \cdot \omega^2 \\ &\stackrel{(R4)}{\stackrel{(R5)}{=}} H(S'^2S)H^3(S'^2S)H(S'S^2)H^3(S'S^2) \cdot \omega^2 \\ &\stackrel{(C5)}{=} HS'^2(SH^3S)S'^2H(S'S^2)H^3(S'S^2) \cdot \omega^2 \\ &\stackrel{(C_4^2)}{=} HS'^2(HS^2H)S'^2H(S'S^2)H^3(S'S^2) \cdot \omega^2 \cdot (-\omega^2) \\ &\stackrel{(D1),(D2)}{\stackrel{(C1),(C5)}{=}} HS'^2(HS^2H)S'^2HS^2(S'H^3S')S^2 \cdot (-\omega) \\ &\stackrel{(C_4^3)}{=} HS'^2(HS^2H)S'^2HS^2(HS'^2H)S^2 \cdot (-\omega) \cdot (-\omega^2) \\ &\stackrel{(D1),(D2)}{\stackrel{(C1)}{=}} HS'^2HS^2HS'^2HS^2HS'^2HS^2. \end{aligned}$$

Then, our problem is reduced to showing

$$HS'^2HS^2HS'^2HS^2HS'^2HS^2 \stackrel{\text{WTS}}{=} 1. \quad (8)$$

Conjugating both sides of (8) by  $H^3$  yields:

$$H^3(HS'^2HS^2HS'^2HS^2HS'^2HS^2)H \stackrel{\text{WTS}}{=} H^3H \stackrel{(C2)}{\iff} S'^2HS^2HS'^2HS^2HS'^2HS^2H \stackrel{\text{WTS}}{=} 1. \quad (9)$$

Then we have

$$\begin{aligned} (9).\text{LHS} &= S'^2HS^2HS'^2HS^2HS'^2HS^2H = (S'^2(HS^2H))^3 \\ &\stackrel{(C1),(C_4^3)}{\stackrel{(D1),(D2)}{=}} (S'^2(SH^3S))^3 \cdot (-\omega)^3 \stackrel{(D1)}{=} (S'^2(SH^3S))^3 \cdot (-1). \end{aligned}$$

It follows that we need to show

$$(S'^2(SH^3S))^3 \cdot (-1) \stackrel{\text{WTS}}{=} 1. \quad (10)$$

Conjugating both sides of (10) by  $S$  yields

$$\begin{aligned} S(S'^2(SH^3S))^3S^2 \cdot (-1) &\stackrel{\text{WTS}}{=} SS^2 \stackrel{(C3)}{\iff} S(S'^2(SH^3S))S^2S(S'^2(SH^3S))S^2S(S'^2(SH^3S))S^2 \cdot (-1) \stackrel{\text{WTS}}{=} 1 \\ &\stackrel{(C3)}{\iff} S(S'^2(SH^3S))S(S'^2(SH^3S))S(S'^2(SH^3S)) \cdot (-1) \stackrel{\text{WTS}}{=} 1 \end{aligned}$$

$$\stackrel{(C5)}{\iff} (S^2 S^2 H^3)^3 \cdot (-1) \stackrel{WTS}{=} 1.$$

By (D3) and (C2), we need to show

$$(H^2 S^2 H^2 S^2 H^3)^3 \cdot (-1) \stackrel{WTS}{=} 1. \quad (11)$$

Conjugating both sides of (11) by  $H^2$  yields

$$\begin{aligned} & H^2 (H^2 S^2 H^2 S^2 H^3)^3 H^2 \cdot (-1) \stackrel{WTS}{=} H^2 H^2 \\ & \stackrel{(C2)}{\iff} H^2 (H^2 S^2 H^2 S^2 H^3) H^2 H^2 (H^2 S^2 H^2 S^2 H^3) H^2 H^2 (H^2 S^2 H^2 S^2 H^3) H^2 \cdot (-1) \stackrel{WTS}{=} 1 \\ & \stackrel{(C2)}{\iff} S^2 H^2 (S^2 H S^2) H^2 (S^2 H S^2) H^2 S^2 H \cdot (-1) \stackrel{WTS}{=} 1 \\ & \stackrel{(C4)}{\iff} S^2 H^2 (H^3 S H^3) H^2 (H^3 S H^3) H^2 S^2 H \cdot (-1) \cdot (-\omega)^2 \stackrel{WTS}{=} 1 \\ & \stackrel{(D1)}{\iff} \stackrel{(C1),(C2)}{\iff} S^2 H S^2 H S^2 H \cdot (-\omega^2) \stackrel{WTS}{=} 1 \end{aligned} \quad (12)$$

By (D1), (D2), (C1), and (C4), (12).LHS =  $(S^2 H S^2 H S^2 H) \cdot (-\omega^2) = (-\omega) \cdot (-\omega^2) = 1$ . This completes the proof.  $\square$

**Proposition 2.8.** *The equations in Figures 53 and 54 imply the equations in Figure 4.*

*Proof.* By Lemmas 2.2 to 2.7, we complete the proof.  $\square$

## 2.2 Reduce the Single-Qutrit Box Relations

In Proposition 4.1 of [1], we showed that the 34 single-qutrit box relations in Appendix C.2 suffice to convert any single-qutrit Clifford circuit to its normal form. These box relations describe how to push single-qutrit Clifford gates through the  $A$ ,  $C$ ,  $E$ , and  $F$  boxes, whose constructions are specified in Figure 55. In what follows, we show that these box relations are consequences of the relations in Figures 4 and 54 and the derived generators in Figure 53.

$$\begin{array}{lcl} \text{---} \boxed{A_{01}} \text{---} = \text{---} & \text{---} \boxed{A_{02}} \text{---} = \text{---} \boxed{H^2} \text{---} & \text{---} \boxed{C_b} \text{---} = \text{---} \boxed{X^b} \text{---} \\ \text{---} \boxed{A_{ab}} \text{---} = \text{---} \boxed{H^{a(a-1)}} \text{---} \boxed{S^{ab}} \text{---} \boxed{H} \text{---} & \text{---} \boxed{E_b} \text{---} = \text{---} \boxed{S^b} \text{---} & \text{---} \boxed{F_b} \text{---} = \text{---} \boxed{Z^{2b}} \text{---} \end{array}$$

Figure 55: The concrete implementations of  $A$ ,  $C$ ,  $E$ , and  $F$  boxes. Here  $a, b \in \mathbb{Z}_3$  and  $a \neq 0$ .

### 2.2.1 Equation

$$\text{---} = \text{---} \boxed{A_{01}} \text{---} \boxed{C_0} \text{---} \boxed{E_0} \text{---} \boxed{F_0} \text{---}$$

*Proof.* By the definitions of  $A_{01}$ ,  $C_0$ ,  $E_0$ , and  $F_0$  in Figure 55.  $\square$

| Class                                                                                                                                                                                                                                                                               | Count       | Box relations in Appendix C                     | Reduce the box relations to the equations in Figures 53 and 54 |
|-------------------------------------------------------------------------------------------------------------------------------------------------------------------------------------------------------------------------------------------------------------------------------------|-------------|-------------------------------------------------|----------------------------------------------------------------|
| 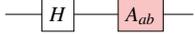<br>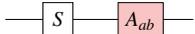<br>$(a, b) \in \mathbb{Z}_3 \times \mathbb{Z}_3 \setminus \{(0, 0)\}$                                        | 8<br>8      | Figure 16<br>Figure 17                          | Equation 2.2.2 to 2.2.4<br>Equation 2.2.5 to 2.2.8             |
| 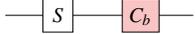<br>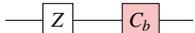<br>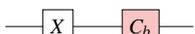<br>$b \in \mathbb{Z}_3$ | 3<br>3<br>3 | Figure 18.(1)<br>Figure 18.(2)<br>Figure 18.(3) | Equation 2.2.9<br>Equation 2.2.10<br>Equation 2.2.11           |
| 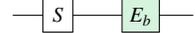<br>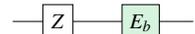<br>$b \in \mathbb{Z}_3$                                                                                      | 3<br>3      | Figure 19.(1)<br>Figure 19.(2)                  | Equation 2.2.12<br>Equation 2.2.13                             |
| 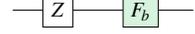<br>$b \in \mathbb{Z}_3$                                                                                                                                                                           | 3           | Figure 20                                       | Equation 2.2.14                                                |
| Total number of single-qutrit box relations                                                                                                                                                                                                                                         | 34          | Appendix C.2 of [1]                             | Section 2.2                                                    |

Figure 56: Overview of the proofs for reducing the single-qutrit box relations to the equations in Figures 53 and 54. ‘Class’ summarizes all possible cases of box relations. ‘Count’ keeps track of the number of distinct rules in each class. The third and fourth columns denote which figure in [1] expresses the box relations and where the proofs of relation reduction can be found in this document, respectively.

## 2.2.2 Equation

$$\text{---} \boxed{H} \text{---} \boxed{A_{ab}} \text{---} = \text{---} \boxed{A_{b,2a}} \text{---} \quad ab = 0$$

*Proof.* By Figure 55, for  $ab = 0$ ,  $A_{ab} = H^{\frac{a(a+1)}{2} + b^2 - b}$ . Then

$$\text{Equation 2.2.2.LHS} = HA_{ab} \stackrel{(\text{def})}{=} HH^{\frac{a(a+1)}{2} + b^2 - b} = H^{\frac{a(a+1)}{2} + b^2 - b + 1}.$$

$$\text{Equation 2.2.2.RHS} = A_{b,2a} \stackrel{(\text{def})}{=} H^{\frac{b(b+1)}{2} + (2a)^2 - 2a} = H^{\frac{b(b+1)}{2} + 2a}.$$

It suffices to show

$$\frac{a(a+1)}{2} + b^2 - b + 1 \equiv_4 \frac{b(b+1)}{2} + 2a. \quad (13)$$

Multiplying both sides of (13) by 2 yields

$$a^2 + a + 2b^2 - 2b + 2 \stackrel{\text{WTS}}{\equiv_4} b^2 + b.$$

Equivalently, we have

$$a^2 + a + b^2 + b \stackrel{\text{WTS}}{\equiv_4} 2. \quad (14)$$

To prove (14), we proceed by case distinctions on  $a$  and  $b$ . Since  $ab = 0$  and  $(a, b) \neq (0, 0)$ , we have:

**Case 1:**  $a = 0$  and  $b \in \{1, 2\}$ . By direct computation,  $b^2 + b \equiv_4 2$ . Hence

$$(14).\text{LHS} = 0 + 2 \equiv_4 2 = (14).\text{RHS}.$$

**Case 2:**  $b = 0$  and  $a \in \{1, 2\}$ . By symmetry,

$$(14).\text{LHS} = 2 + 0 \equiv_4 2 = (14).\text{RHS}.$$

This shows that Equation 2.2.2 is a consequence of (C2), since this rule is used throughout the derivation.  $\square$

### 2.2.3 Equation

$$\text{---} \boxed{H} \text{---} \boxed{A_{ab}} \text{---} = \text{---} \boxed{A_{b,2a}} \text{---} \boxed{S^2} \text{---} \boxed{X^2} \text{---} \cdot (-\omega^2) \quad a = b \in \{1, 2\}$$

*Proof.* By Figure 55, for  $ab \neq 0$  and  $a \equiv_3 b \in \{1, 2\}$ ,  $ab = a^2 \equiv_3 1$  and  $2ab \equiv_3 2$ . Hence,

$$A_{ab} = H^{a(a-1)}SH \quad \text{and} \quad A_{b,2a} = H^{b(b-1)}S^2H.$$

Then

$$\text{Equation 2.2.3.LHS} = HA_{ab} \stackrel{(\text{def})}{=} HH^{a(a-1)}SH = H^{a(a-1)+1}SH.$$

$$\text{Equation 2.2.3.RHS} = A_{b,2a}S^2X^2 \cdot (-\omega^2) \stackrel{(\text{def})}{=} H^{b(b-1)}S^2HS^2X^2 \cdot (-\omega^2) \stackrel{b=a}{=} H^{a(a-1)}S^2HS^2X^2 \cdot (-\omega^2).$$

It suffices to show

$$H^{a(a-1)+1}SH = H^{a(a-1)}S^2HS^2X^2 \cdot (-\omega^2). \quad (15)$$

Multiplying both sides of (15) by  $H^{-a(a-1)}$  yields

$$H^{-a(a-1)}H^{a(a-1)+1}SH = H^{-a(a-1)}H^{a(a-1)}S^2HS^2X^2 \cdot (-\omega^2) \stackrel{(C2)}{\iff} HSH \stackrel{\text{WTS}}{=} S^2HS^2X^2 \cdot (-\omega^2). \quad (16)$$

According to (16), Equation 2.2.3 is indeed a consequence of (R7). This completes the proof.  $\square$

### 2.2.4 Equation

$$\boxed{H} \boxed{A_{ab}} = \boxed{A_{b,2a}} \boxed{X} \boxed{S} \cdot (-\omega) \quad a \neq b \in \{1,2\}$$

*Proof.* By [Figure 55](#), for  $ab \neq 0$  and  $a \neq b \in \{1,2\}$ ,  $b \equiv_3 2a$ . Then  $ab = 2a^2 \equiv_3 2$  and  $2ab \equiv_3 1$ . Hence,

$$A_{ab} = H^{a(a-1)} S^2 H \quad \text{and} \quad A_{b,2a} = H^{b(b-1)} S H.$$

Then

$$\text{Equation 2.2.4.LHS} = H A_{ab} \stackrel{(\text{def})}{=} H H^{a(a-1)} S^2 H = H^{a(a-1)+1} S^2 H.$$

$$\begin{aligned} \text{Equation 2.2.4.RHS} &= A_{b,2a} X S \cdot (-\omega) \stackrel{(\text{def})}{=} H^{b(b-1)} S H X S \cdot (-\omega) \stackrel{b=2a}{=} H^{2a(2a-1)} S H X S \cdot (-\omega) \\ &\stackrel{(\text{C2})}{=} H^{2a} S H X S \cdot (-\omega). \end{aligned}$$

It suffices to show

$$H^{a^2-a+1} S^2 H = H^{2a} S H X S \cdot (-\omega). \quad (17)$$

Multiplying both sides of (17) by  $H^{2a}$  yields

$$H^{2a} H^{a^2-a+1} S^2 H \stackrel{\text{WTS}}{=} S H X S \cdot (-\omega) \stackrel{(\text{C2})}{\iff} H^{a^2+a+1} S^2 H \stackrel{\text{WTS}}{=} S H X S \cdot (-\omega) \quad (18)$$

Since  $a \in \{1,2\}$ ,  $a^2 + a = 2$ . (18) can be simplified to

$$H^3 S^2 H \stackrel{\text{WTS}}{=} S H X S \cdot (-\omega) \stackrel{(\text{C2})}{\iff} H S^2 H \stackrel{\text{WTS}}{=} H^2 S H X S \cdot (-\omega). \quad (19)$$

By [Lemma 2.4](#), [Equation 2.2.4](#) is indeed a consequence of (R7). This completes the proof.  $\square$

### 2.2.5 Equation

$$\boxed{S} \boxed{A_{01}} = \boxed{A_{01}} \boxed{S}$$

*Proof.* By [Figure 55](#),  $A_{01} = I$ . Then

$$\text{Equation 2.2.5.LHS} = S A_{01} \stackrel{(\text{def})}{=} S \stackrel{(\text{def})}{=} A_{01} S = \text{Equation 2.2.5.RHS}. \quad \square$$

### 2.2.6 Equation

$$\boxed{S} \boxed{A_{02}} = \boxed{A_{02}} \boxed{S} \boxed{Z^2}$$

*Proof.* By [Figure 55](#),  $A_{02} = H^2$ . Then

$$\text{Equation 2.2.6.LHS} = S A_{02} \stackrel{(\text{def})}{=} S H^2 \stackrel{(\text{R8})}{=} H^2 S Z^2 \stackrel{(\text{def})}{=} A_{02} S Z^2 = \text{Equation 2.2.6.RHS}. \quad \square$$

## 2.2.7 Equation

$$\text{---} \boxed{S} \text{---} \boxed{A_{1b}} \text{---} = \text{---} \boxed{A_{1,b+1}} \text{---} \quad b \in \mathbb{Z}_3$$

*Proof.* By Figure 55, for  $b \in \mathbb{Z}_3$ ,  $A_{1b} = S^b H$ . Then

$$\text{Equation 2.2.7.LHS} = SA_{1b} \stackrel{(\text{def})}{=} SS^b H = S^{b+1} H \stackrel{(\text{C3})}{=} A_{1,b+1} = \text{Equation 2.2.7.RHS.} \quad \square$$

## 2.2.8 Equation

$$\text{---} \boxed{S} \text{---} \boxed{A_{2b}} \text{---} = \text{---} \boxed{A_{2,b+2}} \text{---} \boxed{X} \text{---} \quad b \in \mathbb{Z}_3$$

*Proof.* By Figure 55, for  $b \in \mathbb{Z}_3$ ,  $A_{2b} = H^2 S^{2b} H$ . Then

$$\begin{aligned} \text{Equation 2.2.8.LHS} &= SA_{2b} \stackrel{(\text{def})}{=} SH^2 S^{2b} H \stackrel{(\text{R8})}{=} H^2 SZ^2 S^{2b} H \stackrel{(\text{R9})}{=} H^2 SS^{2b} Z^2 H \\ &= H^2 S^{2b+1} Z^2 H \stackrel{(\text{C3})}{=} H^2 S^{2(b+2)} HX \stackrel{(\text{def})}{=} A_{2,b+2} X = \text{Equation 2.2.8.RHS.} \quad \square \end{aligned}$$

## 2.2.9 Equation

$$\text{---} \boxed{S} \text{---} \boxed{C_b} \text{---} = \text{---} \boxed{C_b} \text{---} \boxed{S} \text{---} \boxed{Z^b} \text{---} \cdot \omega^{b(b+1)} \quad b \in \mathbb{Z}_3$$

*Proof.* By Figure 55, for  $b \in \mathbb{Z}_3$ ,  $C_b = X^b$ . Then

$$\text{Equation 2.2.9.LHS} = SC_b \stackrel{(\text{def})}{=} SX^b. \quad (20)$$

We proceed by case distinctions on  $b \in \mathbb{Z}_3$ .

**Case 1:**  $b = 0$ . (20) =  $S \stackrel{(\text{def})}{=} C_0 S = \text{Equation 2.2.9.RHS.}$

**Case 2:**  $b = 1$ . (20) =  $SX \stackrel{(\text{R11})}{=} XZS \cdot \omega^2 \stackrel{(\text{R9})}{=} XSZ \cdot \omega^2 \stackrel{(\text{def})}{=} C_1 SZ \cdot \omega^2 = \text{Equation 2.2.9.RHS.}$

**Case 3:**  $b = 2$ . (20) =  $SX^2 \stackrel{(\text{R11})}{=} XZSX \cdot \omega^2 \stackrel{(\text{R11})}{=} XZXZS \cdot \omega^2 \cdot \omega^2 \stackrel{(\text{D2})}{=} X^2 Z^2 S \cdot \omega \cdot \omega^2 \stackrel{(\text{D2})}{=} X^2 SZ^2 \stackrel{(\text{def})}{=} C_2 SZ^2 = \text{Equation 2.2.9.RHS.} \quad \square$

## 2.2.10 Equation

$$\text{---} \boxed{Z} \text{---} \boxed{C_b} \text{---} = \text{---} \boxed{C_b} \text{---} \boxed{Z} \text{---} \cdot \omega^{2b} \quad b \in \mathbb{Z}_3$$

*Proof.* By Figure 55, for  $b \in \mathbb{Z}_3$ ,  $C_b = X^b$ . Then

$$\text{Equation 2.2.10.LHS} = ZC_b \stackrel{(\text{def})}{=} ZX^b. \quad (21)$$

We proceed by case distinctions on  $b \in \mathbb{Z}_3$ .

**Case 1:**  $b = 0$ . (21) =  $Z \stackrel{(\text{def})}{=} C_0 Z = \text{Equation 2.2.10.RHS.}$

**Case 2:**  $b = 1$ . (21) =  $ZX \stackrel{(\text{R12})}{=} XZ \cdot \omega^2 \stackrel{(\text{def})}{=} C_1 Z \cdot \omega^2 = \text{Equation 2.2.10.RHS.}$

**Case 3:**  $b = 2$ . (21) =  $ZX^2 \stackrel{(\text{R12})}{=} XZX \cdot \omega^2 \stackrel{(\text{R12})}{=} X^2 Z \cdot \omega^2 \cdot \omega^2 \stackrel{(\text{C1})}{=} X^2 Z \cdot \omega \stackrel{(\text{def})}{=} C_2 Z \cdot \omega = \text{Equation 2.2.10.RHS.} \quad \square$

### 2.2.11 Equation

$$\text{---} \boxed{X} \text{---} \boxed{C_b} \text{---} = \text{---} \boxed{C_{b+1}} \text{---} \quad b \in \mathbb{Z}_3$$

*Proof.* By Figure 55, for  $b \in \mathbb{Z}_3$ ,  $C_b = X^b$ . Then

$$\text{Equation 2.2.11.LHS} = XC_b \stackrel{(\text{def})}{=} XX^b = X^{b+1} \stackrel{(\text{def})}{\stackrel{(R3)}{=}} C_{b+1} = \text{Equation 2.2.11.RHS.} \quad \square$$

### 2.2.12 Equation

$$\text{---} \boxed{S} \text{---} \boxed{E_b} \text{---} = \text{---} \boxed{E_{b+1}} \text{---} \quad b \in \mathbb{Z}_3$$

*Proof.* By Figure 55, for  $b \in \mathbb{Z}_3$ ,  $E_b = S^b$ . Then

$$\text{Equation 2.2.12.LHS} = SE_b \stackrel{(\text{def})}{=} SS^b = S^{b+1} \stackrel{(\text{def})}{\stackrel{(C3)}{=}} E_{b+1} = \text{Equation 2.2.12.RHS.} \quad \square$$

### 2.2.13 Equation

$$\text{---} \boxed{Z} \text{---} \boxed{E_b} \text{---} = \text{---} \boxed{E_b} \text{---} \boxed{Z} \text{---} \quad b \in \mathbb{Z}_3$$

*Proof.* By Figure 55, for  $b \in \mathbb{Z}_3$ ,  $E_b = S^b$ . Then

$$\text{Equation 2.2.13.LHS} = ZE_b \stackrel{(\text{def})}{=} ZS^b \stackrel{(R9)}{=} S^bZ \stackrel{(\text{def})}{=} E_bZ = \text{Equation 2.2.13.RHS.} \quad \square$$

### 2.2.14 Equation

$$\text{---} \boxed{Z} \text{---} \boxed{F_b} \text{---} = \text{---} \boxed{F_{b+2}} \text{---} \quad b \in \mathbb{Z}_3$$

*Proof.* By Figure 55, for  $b \in \mathbb{Z}_3$ ,  $F_b = Z^{2b}$ . Then

$$\text{Equation 2.2.14.LHS} = ZF_b \stackrel{(\text{def})}{=} ZZ^{2b} = Z^{2(b+2)} \stackrel{(\text{def})}{\stackrel{(R6)}{=}} F_{b+2} = \text{Equation 2.2.14.RHS.} \quad \square$$

**Theorem 2.1.** Any true equality between single-qutrit Clifford circuits is provable using the rules in Figure 54 with the derived generators in Figure 53.

*Proof.* By Proposition 4.3 in [1], the zero- and single-qutrit box relations in Appendices C.1 and C.2 are complete for the single-qutrit Clifford group. Based on the derivations in Section 2.2, the rules in Figures 4 and 54 with the derived generators in Figure 53 suffice to prove all relations in Appendix C.2. By Proposition 2.8, the equations in Figure 4 follow from the equations in Figures 53 and 54. This implies that we can prove any true equality between single-qutrit Clifford circuits using the rules in Figure 54 with the derived generators in Figure 53.  $\square$



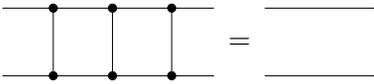

(C6)

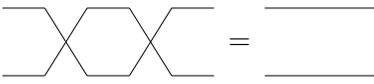

(C7)

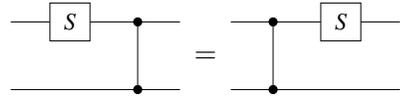

(C8)

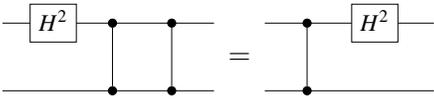

(C9)

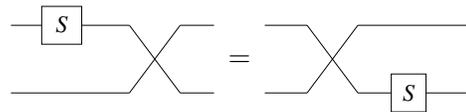

(C10)

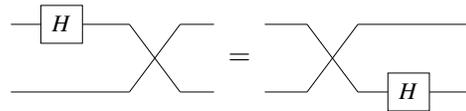

(C11)

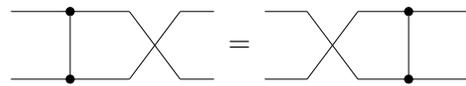

(C12)

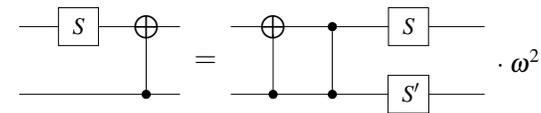

(C13)

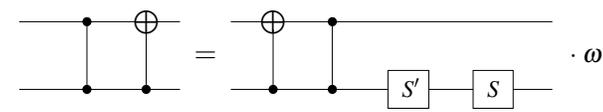

(C14)

Figure 58: The two-qutrit reduced relations from Figure 1.

*Proof.*

(C<sub>8</sub><sup>1</sup>).LHS = 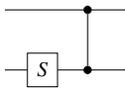  $\stackrel{(C7)}{=}$  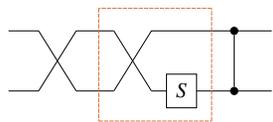  $\stackrel{(C10)}{=}$  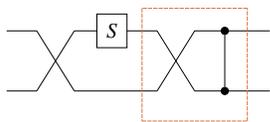

$\stackrel{(C12)}{=}$  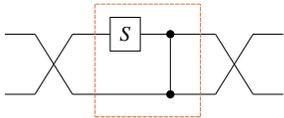  $\stackrel{(C8)}{=}$  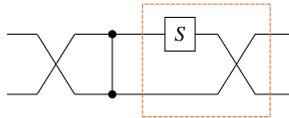

$\stackrel{(C10)}{=}$  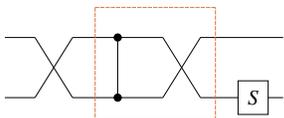  $\stackrel{(C12)}{=}$  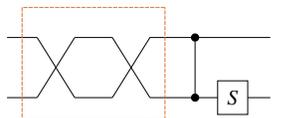

$\stackrel{(C7)}{=}$  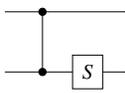 = (C<sub>8</sub><sup>1</sup>).RHS

□

**Lemma 3.4.** *The equations in Figure 11 follow from the reduced relations.*

*Proof.* We derive  $(C_9^1)$  to  $(C_9^{11})$  from Figures 1 and 2 one after the other.

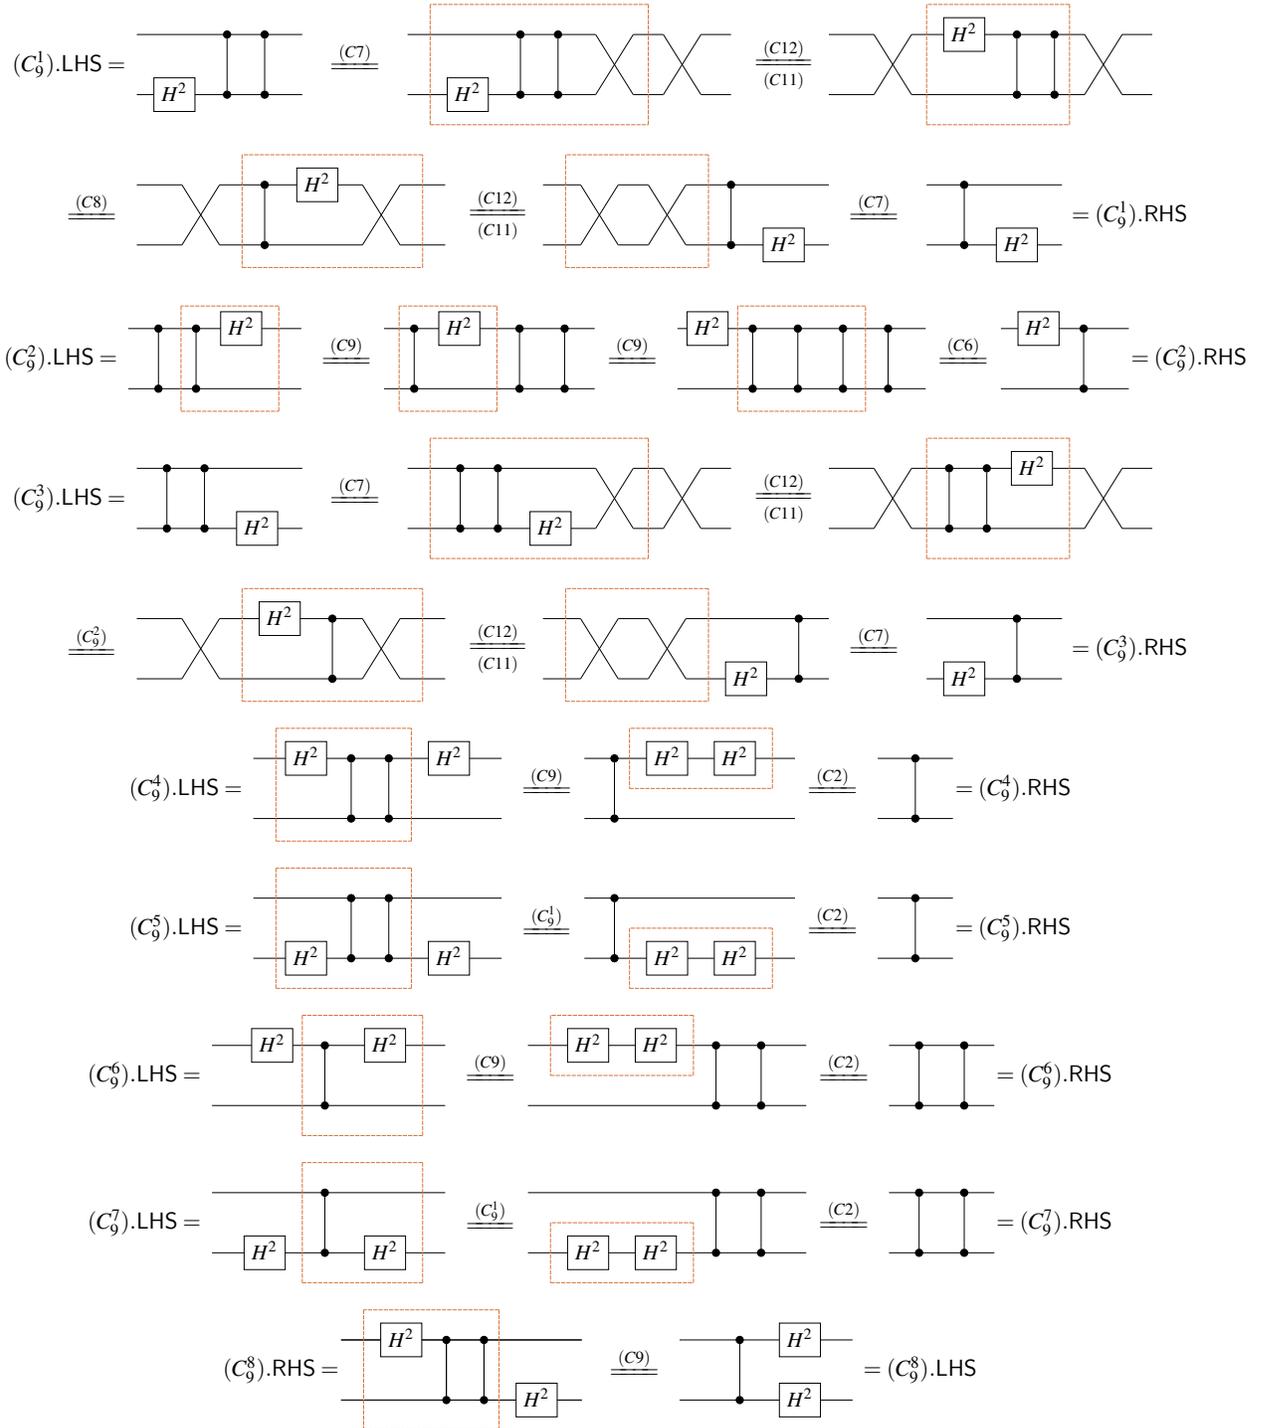

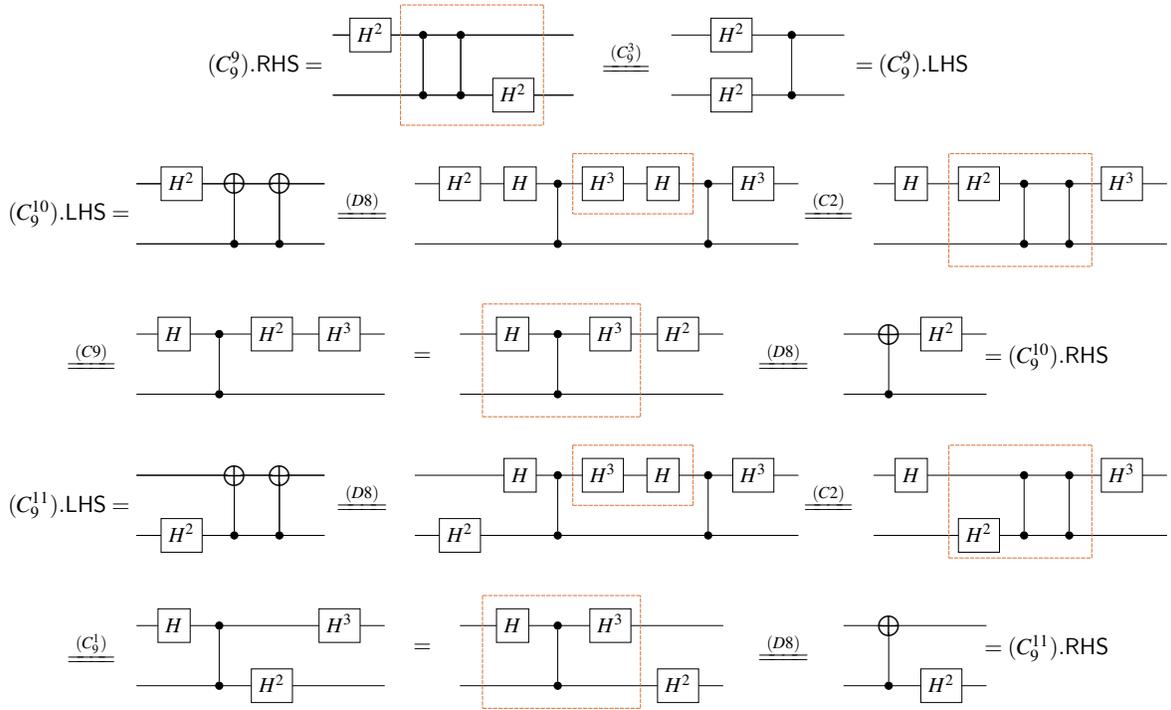

Reasoning analogously as above, we can show that  $(C_9^{12})$  to  $(C_9^{18})$  follow from  $(D6)$ ,  $(D8)$ ,  $(C2)$ ,  $(C6)$ ,  $(C7)$ ,  $(C9)$ ,  $(C11)$ , and  $(C12)$   $\square$ .

**Corollary 3.5.** *The equations in Figure 12 follow from the reduced relations.*

**Lemma 3.6.** *The equations in Figure 13 follow from the reduced relations.*

*Proof.*

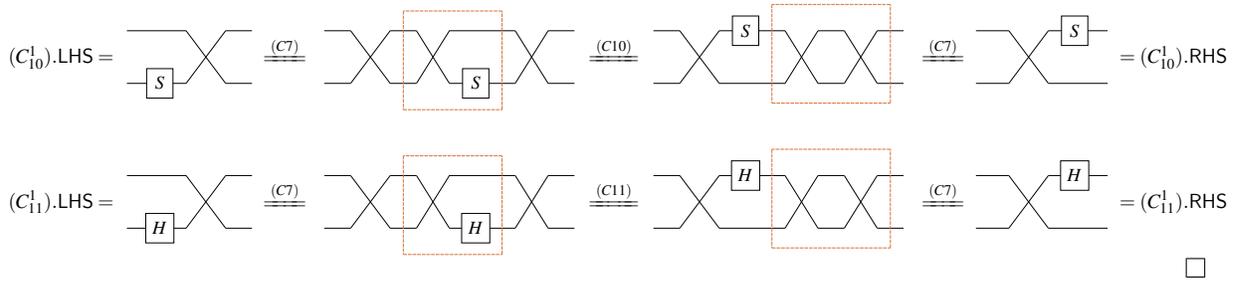

**Proposition 3.7.** *Let  $A = \{H, S\}$ . For all  $U \in A^*$ , the equations in Figure 14 follow from the reduced relations.*

*Proof.* We first prove  $(SWAP^1)$ . Let  $U \in A^*$  be an arbitrary single-qutrit Clifford word. Then  $U = S^{a_1} H^{b_1} \dots S^{a_m} H^{b_m}$ ,  $m \in \mathbb{N}^{>0}$ ,  $a_j \in \mathbb{Z}_3$ ,  $b_j \in \mathbb{Z}_4$ , for all  $1 \leq j \leq m$ . We proceed by induction on  $m$ . Consider the base case when  $m = 1$ . There are two scenarios. When  $a_1 = 1$  and  $b_1 = 0$ ,  $U = S$ . When  $a_1 = 0$  and  $b_1 = 1$ ,  $U = H$ . By  $(C10)$  and  $(C11)$ ,  $(SWAP^1)$  holds.

By the induction hypothesis (IH),  $(SWAP^1)$  holds for  $U = S^{a_1} H^{b_1} \dots S^{a_m} H^{b_m}$ ,  $m \geq 1$ . For the induction step, consider  $U' = US^{a_{m+1}} H^{b_{m+1}}$ ,  $a_{m+1} \in \mathbb{Z}_3$  and  $b_{m+1} \in \mathbb{Z}_4$ . Then, we have

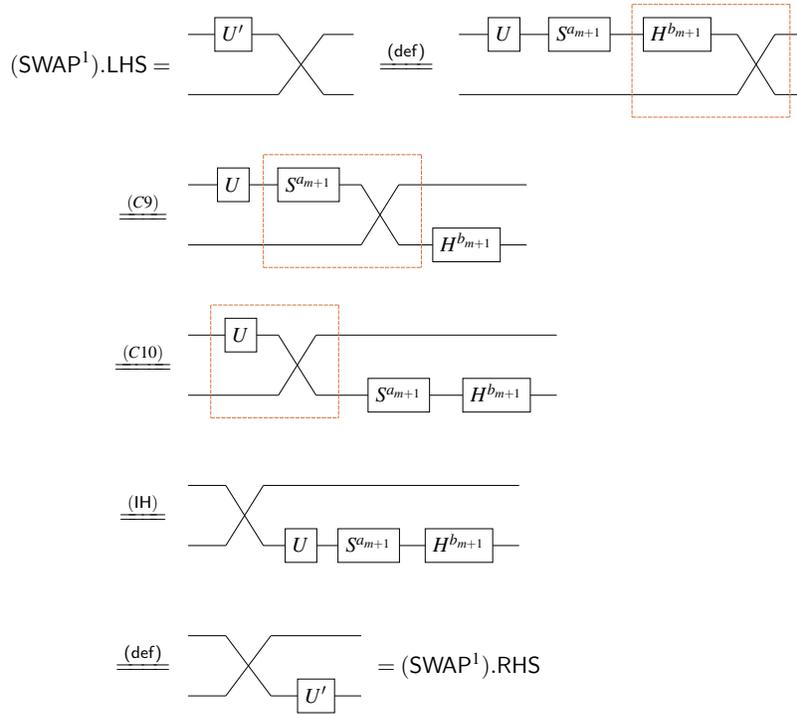

Therefore, (SWAP<sup>1</sup>) holds for all  $U \in A^*$ . Since (SWAP<sup>2</sup>) follows from (D6), (C7), and (SWAP<sup>1</sup>), this completes the proof. □

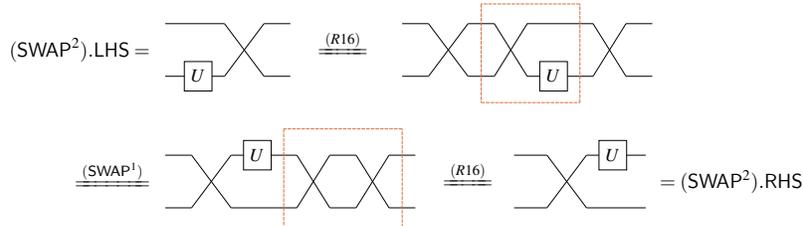

### 3.1 Reduce the Two-Qutrit Derived Relations

Up to single-qutrit Clifford completeness, we show that the derived relations in Figure 8 are consequences of the reduced relations in Figure 58 and the derived generators in Figure 57.

**Corollary 3.8.** *The equations in Figure 15 follow from the reduced relations.*

*Proof.* According to (D3), (D4), and (D5) in Figure 2, write  $X$ ,  $Z$ , and  $S'$  in terms of  $H$  and  $S$  gates. Then apply Proposition 3.7 to complete the proof. To show (R16) and (R<sub>16</sub><sup>1</sup>) follow from (D6), (D7), (D8) in Figure 2, and the equations in Figure 1, it suffices to derive (R16), since the proof of deriving (R<sub>16</sub><sup>1</sup>) proceeds analogously. □

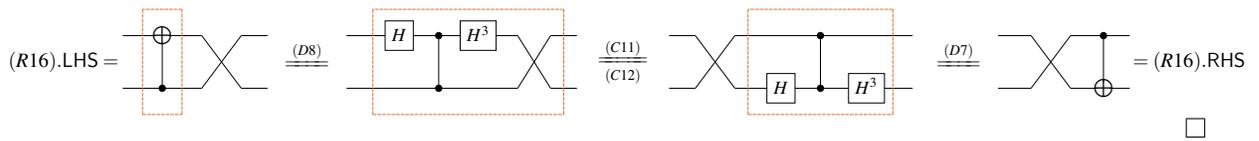

**Lemma 3.9.** *The equations in Figure 16 follow from the reduced relations.*

*Proof.* By symmetry, it suffices to derive (R17) from the equations in Figures 1 and 2.

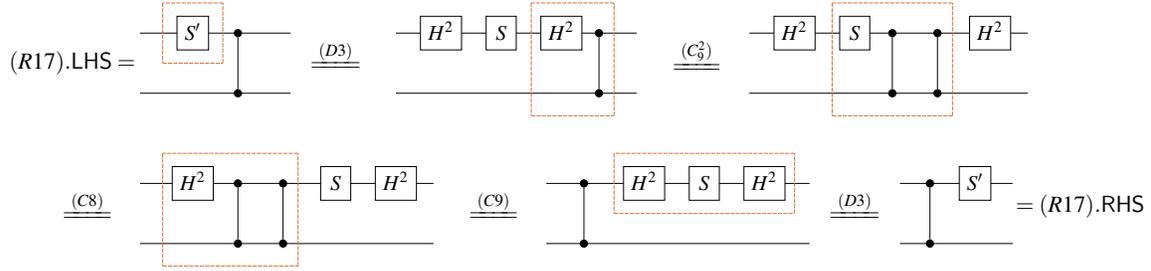

□

**Lemma 3.10.** *The equations in Figure 17 follow from the reduced relations.*

*Proof.* By symmetry, it suffices to derive (R18) and (R<sub>18</sub><sup>2</sup>) from the equations in Figures 1 and 2.

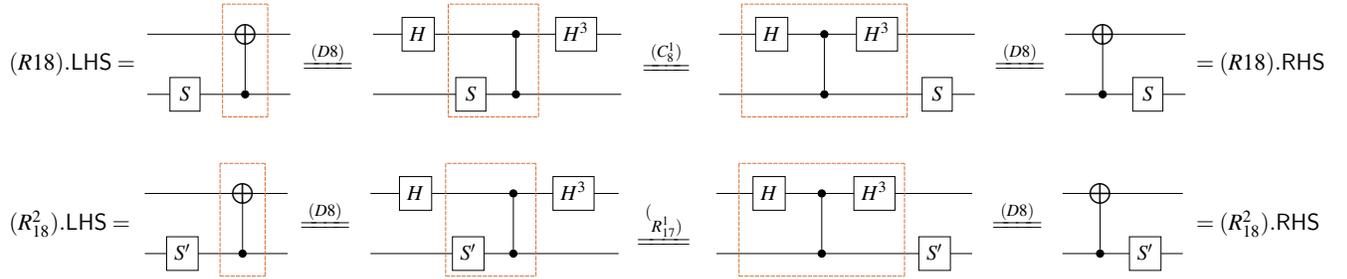

By Lemma 3.9, (R17) follows from the equations in Figures 1 and 2. This completes the proof. □

**Lemma 3.11.** *The equations in Figure 18 follow from the reduced relations.*

*Proof.* By symmetry, it suffices to derive (R19), (R<sub>19</sub><sup>2</sup>), and (R<sub>19</sub><sup>4</sup>) from the equations in Figures 1 and 2.

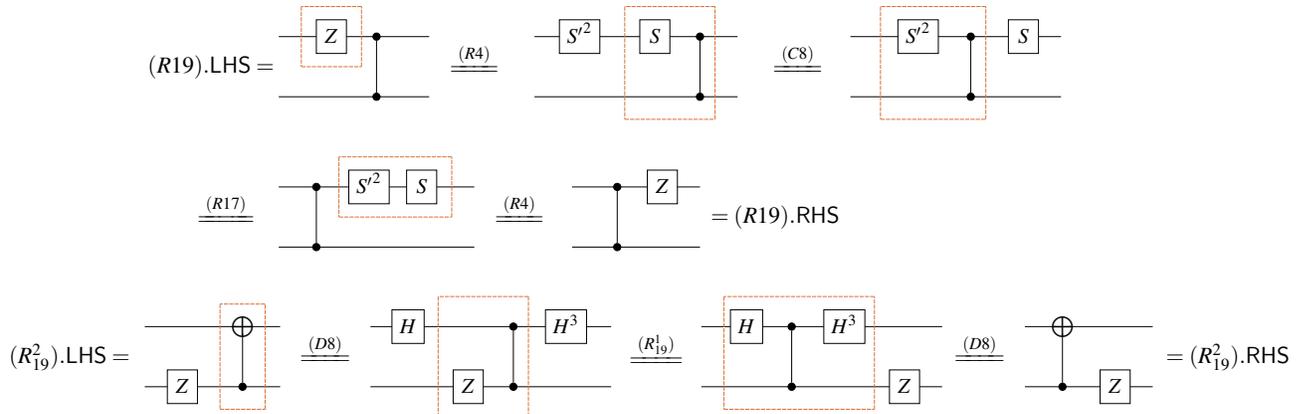

$$\begin{aligned}
(R_{19}^4).\text{LHS} &= \text{Circuit 1} \stackrel{(D8)}{=} \text{Circuit 2} \stackrel{\substack{(R_{10}^1) \\ (C2)}}{=} \text{Circuit 3} \\
&\stackrel{(R19)}{=} \text{Circuit 4} \stackrel{\substack{(R_{10}^1) \\ (C2)}}{=} \text{Circuit 5} \stackrel{(D8)}{=} \text{Circuit 6} = (R_{19}^4).\text{RHS}
\end{aligned}$$

By **Lemmas 2.3** and **3.9**, **(R10)** and **(R17)** follow from the equations in **Figures 1** and **2**. This completes the proof.  $\square$

**Lemma 3.12.** *The equations in Figure 19 follow from the reduced relations.*

*Proof.* By symmetry, it suffices to prove that **(R20)**, **(R<sub>20</sub><sup>1</sup>)**, **(R<sub>20</sub><sup>2</sup>)**, **(R<sub>20</sub><sup>4</sup>)**, **(R<sub>20</sub><sup>6</sup>)**, **(R<sub>20</sub><sup>8</sup>)**, **(R<sub>20</sub><sup>10</sup>)**, and **(R<sub>20</sub><sup>12</sup>)** follow from the equations in **Figures 1** and **2**.

$$\begin{aligned}
(R_{20}).\text{LHS} &= \text{Circuit 1} \stackrel{(D7)}{=} \text{Circuit 2} \stackrel{\substack{(C_8^8) \\ (C_9^9)}}{=} \text{Circuit 3} \\
&\stackrel{(C6)}{=} \text{Circuit 4} \stackrel{(C2)}{=} \text{Circuit 5} = (R_{20}).\text{RHS} \\
(R_{20}^1).\text{LHS} &= \text{Circuit 6} \stackrel{(C7)}{=} \text{Circuit 7} \stackrel{\substack{(R16),(C12) \\ (C_{11}), (C_{11}')}}{=} \text{Circuit 8} \\
&\stackrel{(R20)}{=} \text{Circuit 9} \stackrel{\substack{(C11) \\ (C_{11}')}}{=} \text{Circuit 10} \stackrel{(C7)}{=} \text{Circuit 11} = (R_{20}^1).\text{RHS} \\
(R_{20}^2).\text{RHS} &= \text{Circuit 12} \stackrel{(C2)}{=} \text{Circuit 13} \stackrel{(R20)}{=} \text{Circuit 14} \\
&\stackrel{(C8)}{=} \text{Circuit 15} \stackrel{(C2)}{=} \text{Circuit 16} = (R_{20}^2).\text{RHS} \\
(R_{20}^4).\text{LHS} &= \text{Circuit 17} \stackrel{(C2)}{=} \text{Circuit 18} \stackrel{\substack{(C_8^8) \\ (C_9^9)}}{=} \text{Circuit 19} \stackrel{(C2)}{=} \text{Circuit 20} \stackrel{(D7)}{=} \text{Circuit 21} = (R_{20}^4).\text{RHS} \\
(R_{20}^6).\text{LHS} &= \text{Circuit 22} \stackrel{(C_6^6)}{=} \text{Circuit 23} \stackrel{(R_{20}^2)}{=} \text{Circuit 24} = (R_{20}^6).\text{RHS}
\end{aligned}$$

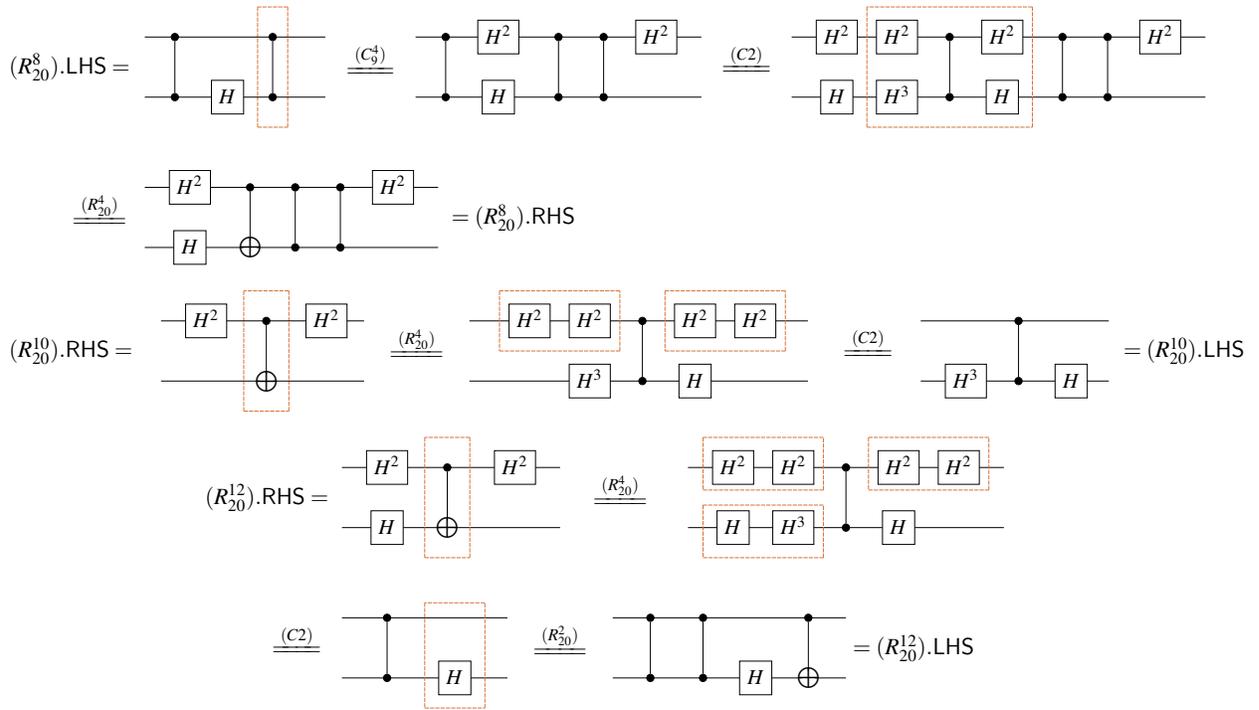

□

**Lemma 3.13.** *The equations in Figure 20 follow from the reduced relations.*

*Proof.* By symmetry, it suffices to prove that  $(R_{21})$ ,  $(R_{21}^2)$ ,  $(R_{21}^4)$ ,  $(R_{21}^6)$ , and  $(R_{21}^8)$  follow from the equations in Figures 1 and 2.

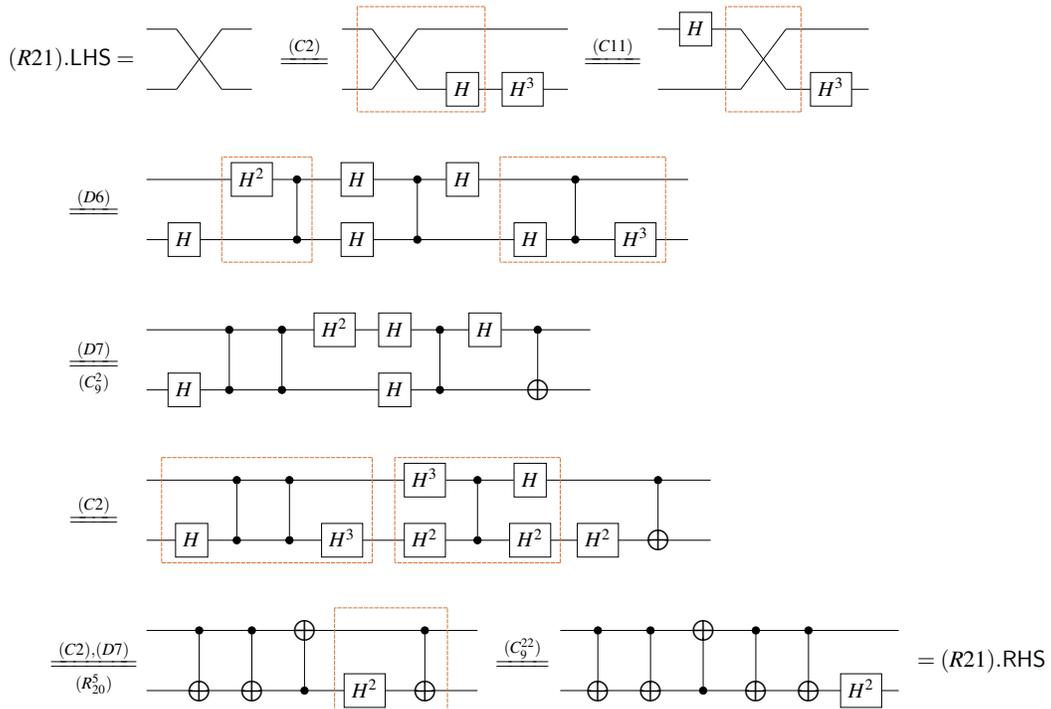

$$\begin{aligned}
 (R_{21}^2).LHS &= \text{CNOT} \stackrel{(C2)}{=} \boxed{\text{CNOT}} \text{ } \stackrel{(C11)}{=} \boxed{H^3} \text{CNOT} \\
 &\stackrel{(R21)}{=} \begin{array}{c} \text{---} H^3 \text{---} \bullet \text{---} \bullet \text{---} \oplus \text{---} \bullet \text{---} \bullet \text{---} \\ | \quad | \quad | \quad | \quad | \\ \oplus \quad \oplus \quad \bullet \quad \oplus \quad \oplus \end{array} H^2 H \\
 &= \begin{array}{c} \text{---} H^3 \text{---} \bullet \text{---} \bullet \text{---} \oplus \text{---} \bullet \text{---} \bullet \text{---} \\ | \quad | \quad | \quad | \quad | \\ \oplus \quad \oplus \quad \bullet \quad \oplus \quad \oplus \end{array} H^3 = (R_{21}^2).RHS
 \end{aligned}$$

$$\begin{aligned}
 (R_{21}^4).LHS &= \text{CNOT} \stackrel{(C2)}{=} \boxed{\text{CNOT}} \text{ } \stackrel{(C11)}{=} \boxed{H} \text{CNOT} \\
 &\stackrel{(R21)}{=} \begin{array}{c} \text{---} H \text{---} \bullet \text{---} \bullet \text{---} \oplus \text{---} \bullet \text{---} \bullet \text{---} \\ | \quad | \quad | \quad | \quad | \\ \oplus \quad \oplus \quad \bullet \quad \oplus \quad \oplus \end{array} \boxed{H^2 H^3} \\
 &\stackrel{(C2)}{=} \begin{array}{c} \text{---} H \text{---} \bullet \text{---} \bullet \text{---} \oplus \text{---} \bullet \text{---} \bullet \text{---} \\ | \quad | \quad | \quad | \quad | \\ \oplus \quad \oplus \quad \bullet \quad \oplus \quad \oplus \end{array} H = (R_{21}^4).RHS
 \end{aligned}$$

$$\begin{aligned}
 (R_{21}^6).LHS &= \text{CNOT} \stackrel{(C2)}{=} \boxed{\text{CNOT}} \text{ } \stackrel{(C11)}{=} \boxed{H^2} \text{CNOT} \\
 &\stackrel{(R21)}{=} \begin{array}{c} \text{---} H^2 \text{---} \bullet \text{---} \bullet \text{---} \oplus \text{---} \bullet \text{---} \bullet \text{---} \\ | \quad | \quad | \quad | \quad | \\ \oplus \quad \oplus \quad \bullet \quad \oplus \quad \oplus \end{array} \boxed{H^2 H^2} \\
 &\stackrel{(C2)}{=} \begin{array}{c} \text{---} H^2 \text{---} \bullet \text{---} \bullet \text{---} \oplus \text{---} \bullet \text{---} \bullet \text{---} \\ | \quad | \quad | \quad | \quad | \\ \oplus \quad \oplus \quad \bullet \quad \oplus \quad \oplus \end{array} = (R_{21}^6).RHS
 \end{aligned}$$

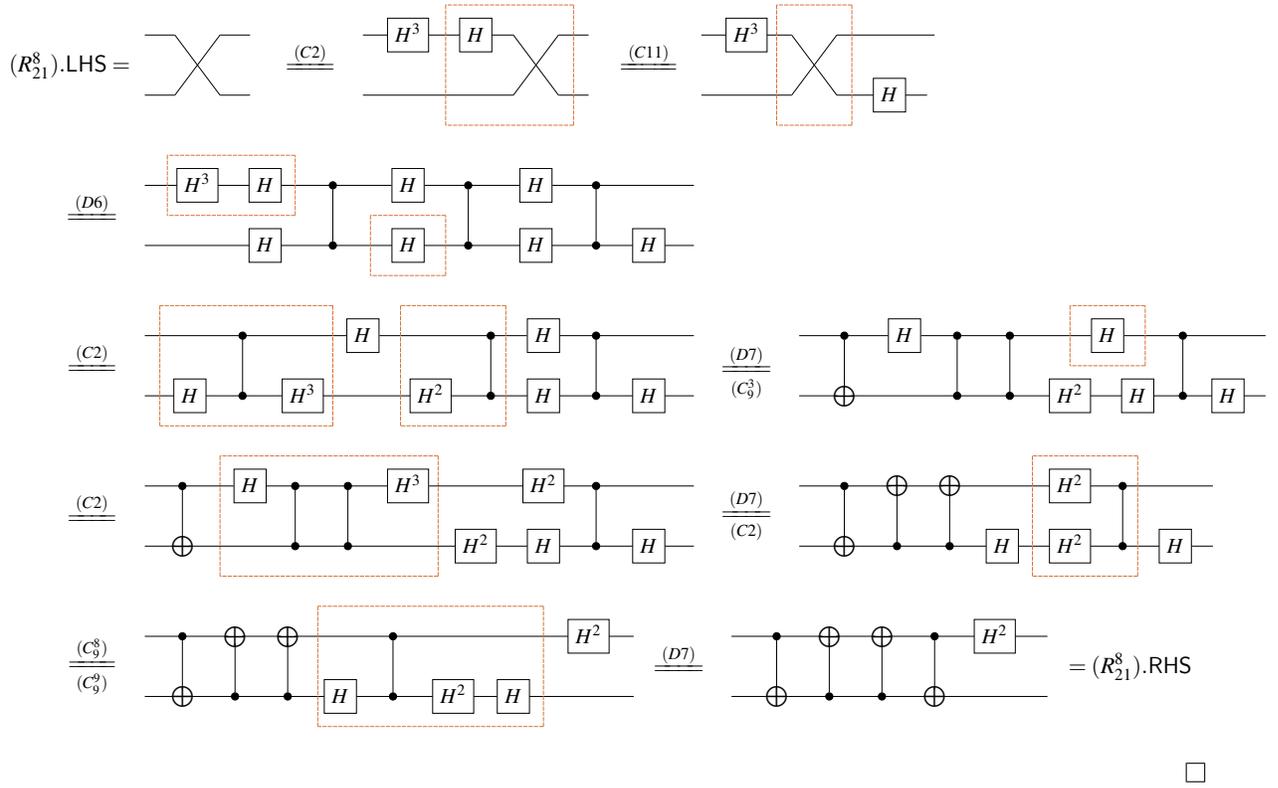

**Lemma 3.14.** *The equations in Figure 21 follow from the reduced relations.*

*Proof.* We derive equations in Figure 21 one after the other. Right-appending both sides of  $(R_{21}^8)$  by  $H^2 \otimes H^2$  yields

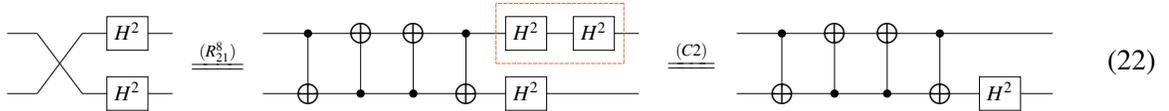

Moreover, we have

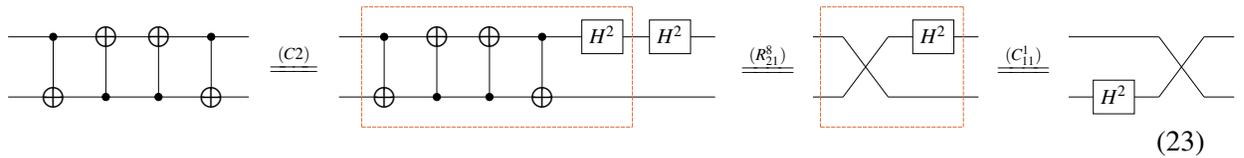

Left-appending the left-most and right-most sides of (23) by  $H^2 \otimes I$  yields

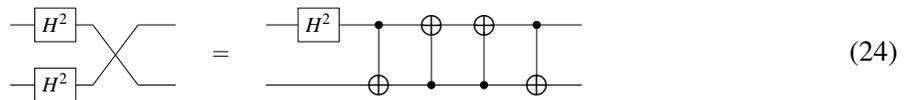

It follows that

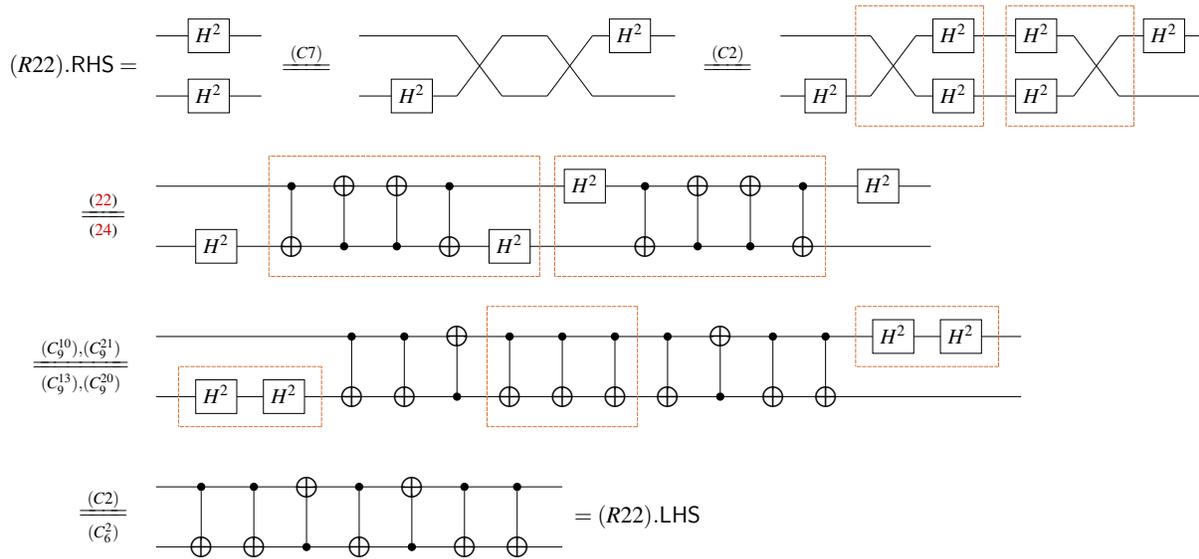

For both sides of  $(R22)$ , left-appending them by  $CX^2$  and right-appending them by  $CX$  yields

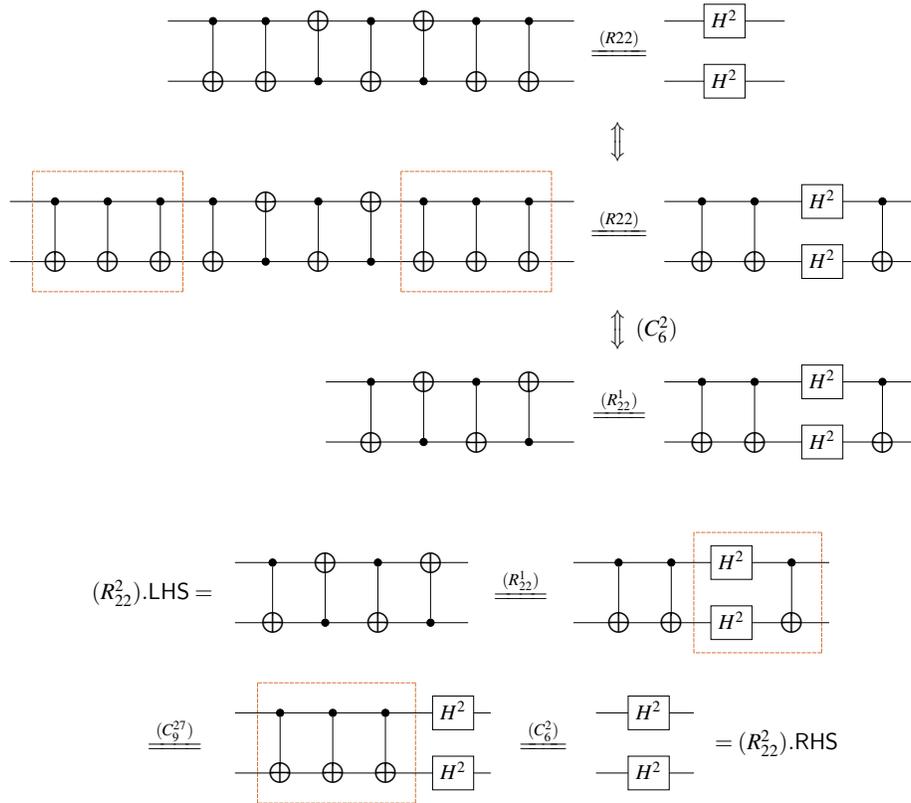

By symmetry,  $(R22^2)$  implies  $(R22^3)$ . For both sides of  $(R22^3)$ , left-appending them by  $(CX^2)(XC^2)$  and

right-appending them by  $H^2 \otimes H^2$  yields

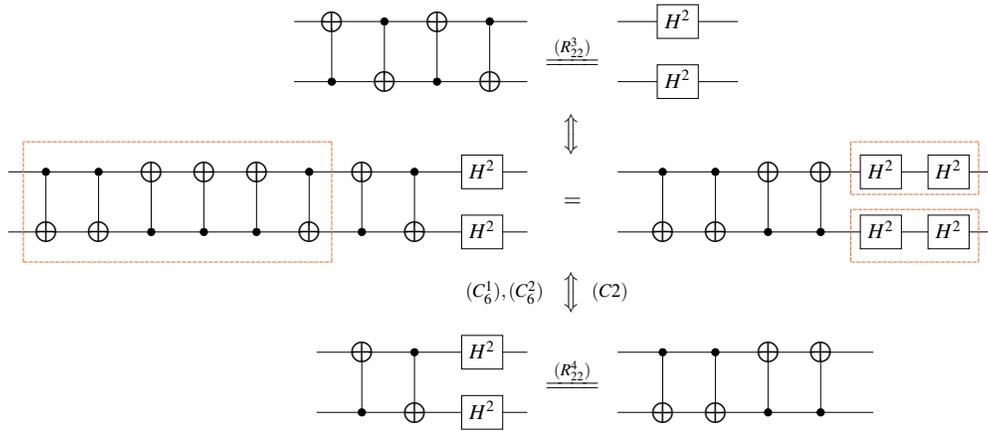

**Lemma 3.15.**  $(R23)$  in Figure 21 follows from the equations in Figure 1.

*Proof.*

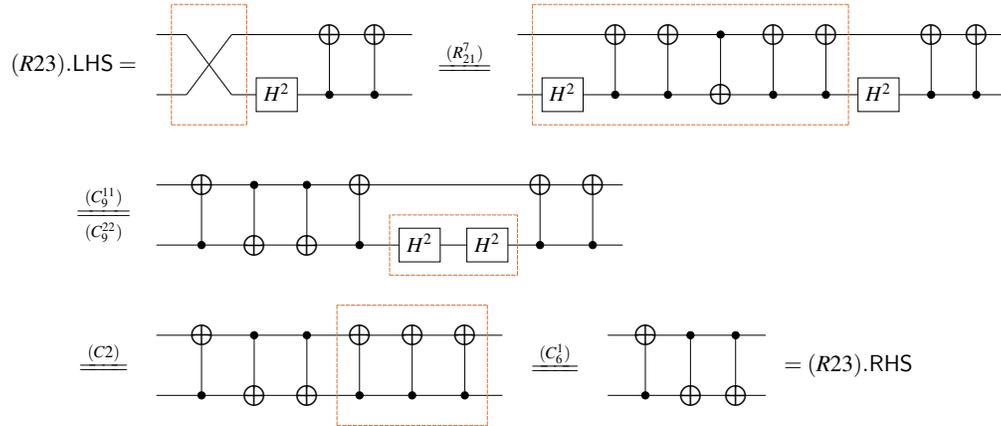

**Lemma 3.16.** The equations in Figure 22 follow from the reduced relations.

*Proof.* We derive equations in Figure 22 one after the other.

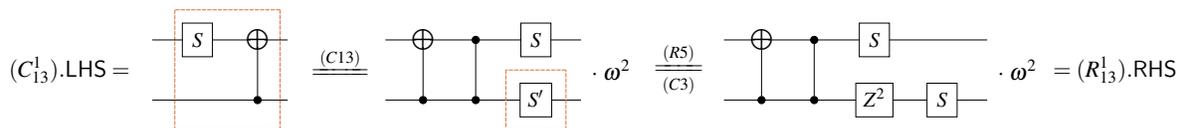

For both sides of (C13), left-appending them by  $S^2 \otimes I$  and right-appending them by  $S \otimes I$  yields

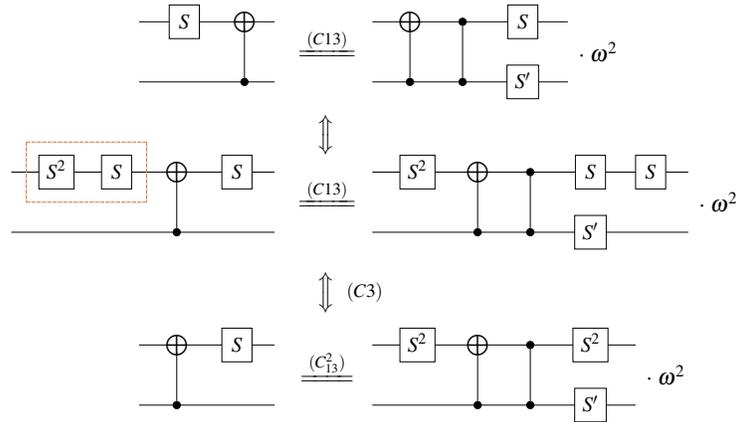

For both sides of (C13), right-appending them by  $S^2 \otimes S'^2$  and multiplying them by  $\omega$  yields

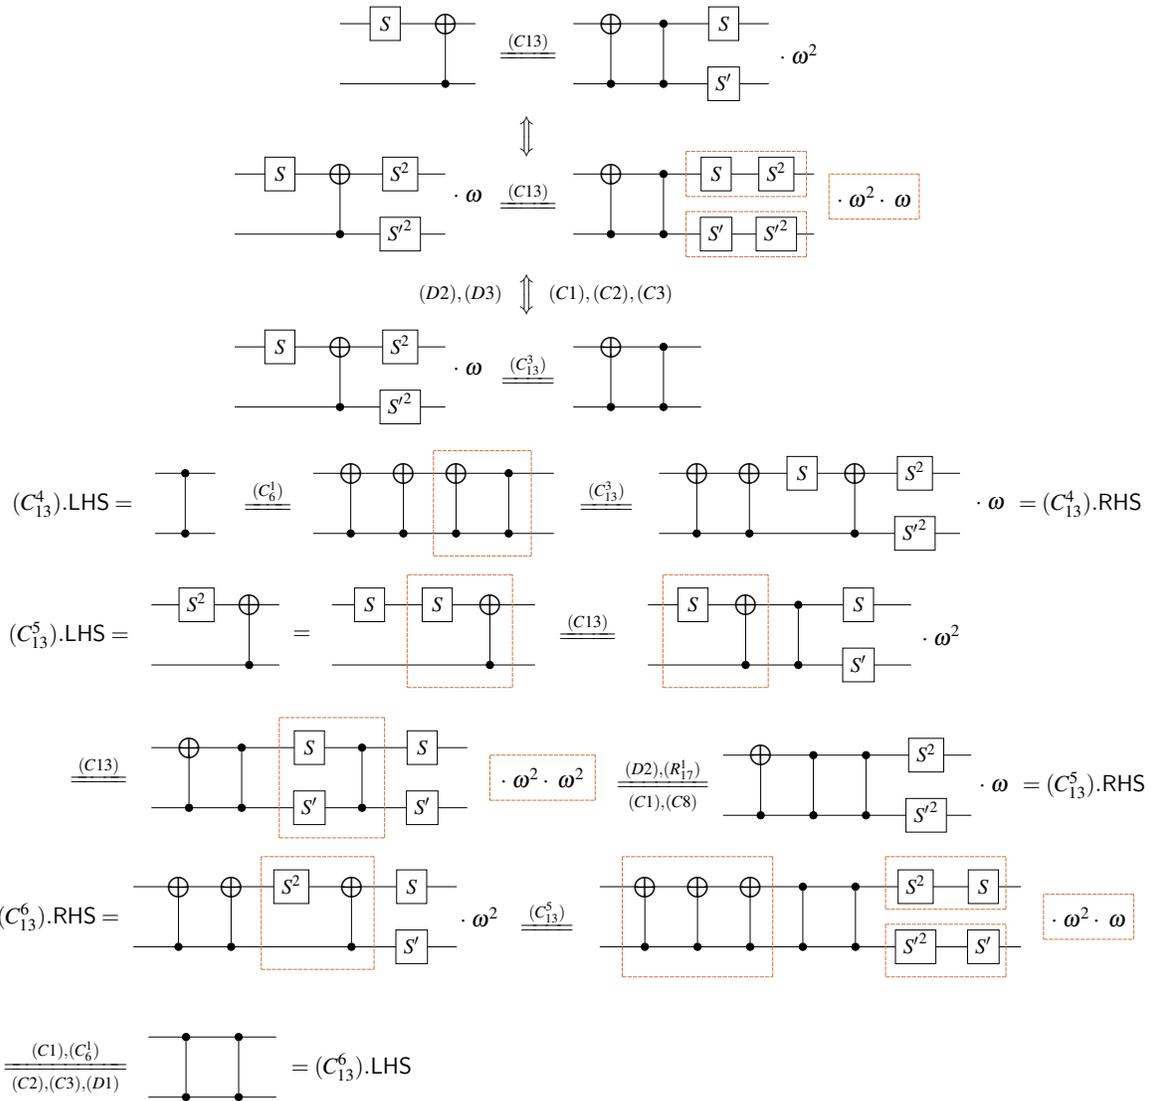

□

**Corollary 3.17.** *The equations in Figure 23 follow from the reduced relations.*

**Lemma 3.18.** *The equations in Figure 24 follow from the reduced relations.*

*Proof.* We derive equations in Figure 24 one after the other.

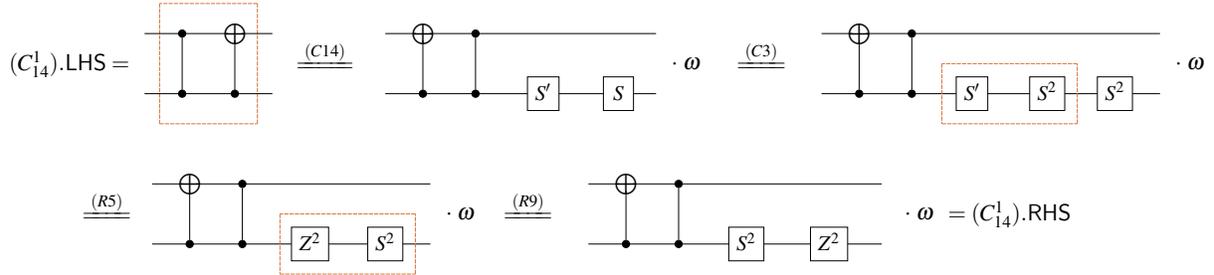

Right-appending both sides of (C14) by  $I \otimes S^2 S'^2$  yields

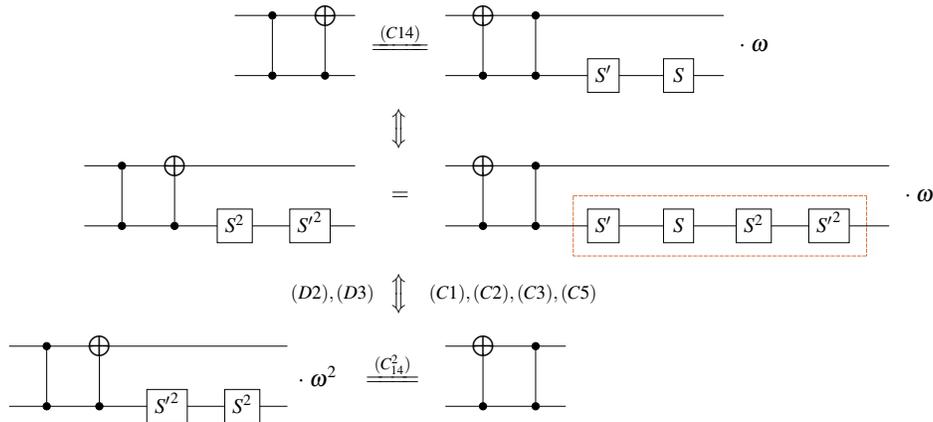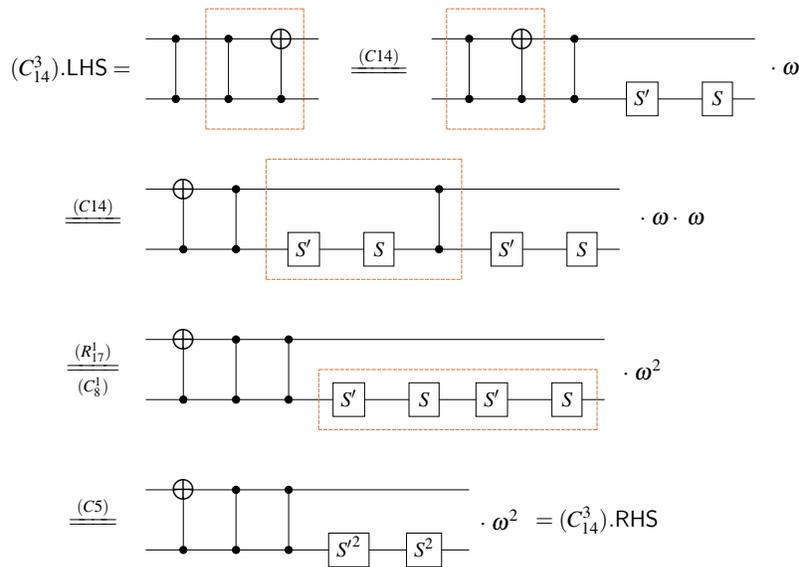



*Proof.*

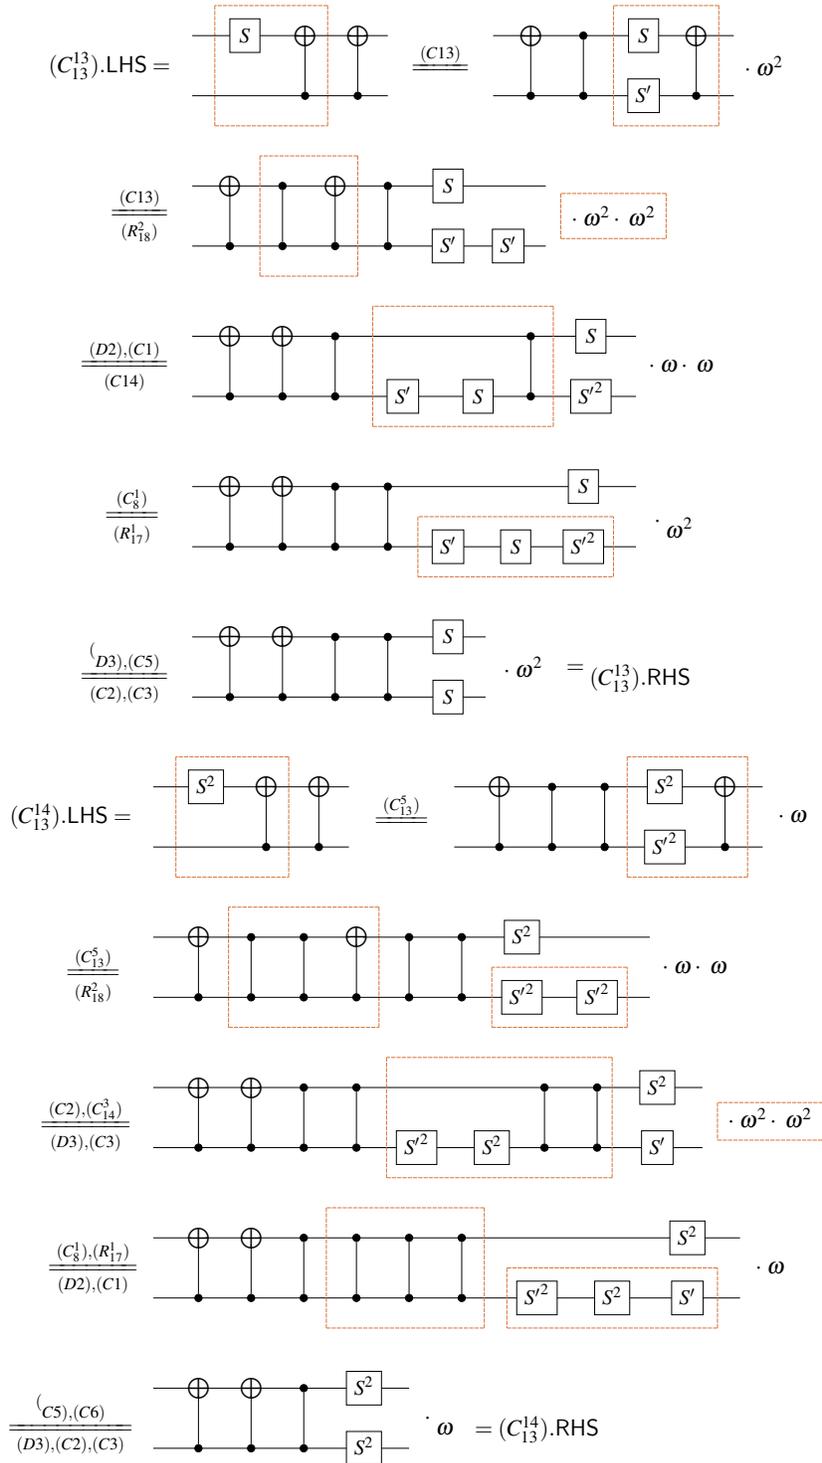

□

**Corollary 3.21.**  $(C_{13}^{15})$  and  $(C_{13}^{16})$  in Figure 26 follow from the reduced relations.

**Lemma 3.22.**  $(C_{13}^{17})$  to  $(C_{13}^{21})$  in Figure 26 follow from the reduced relations.

Proof.

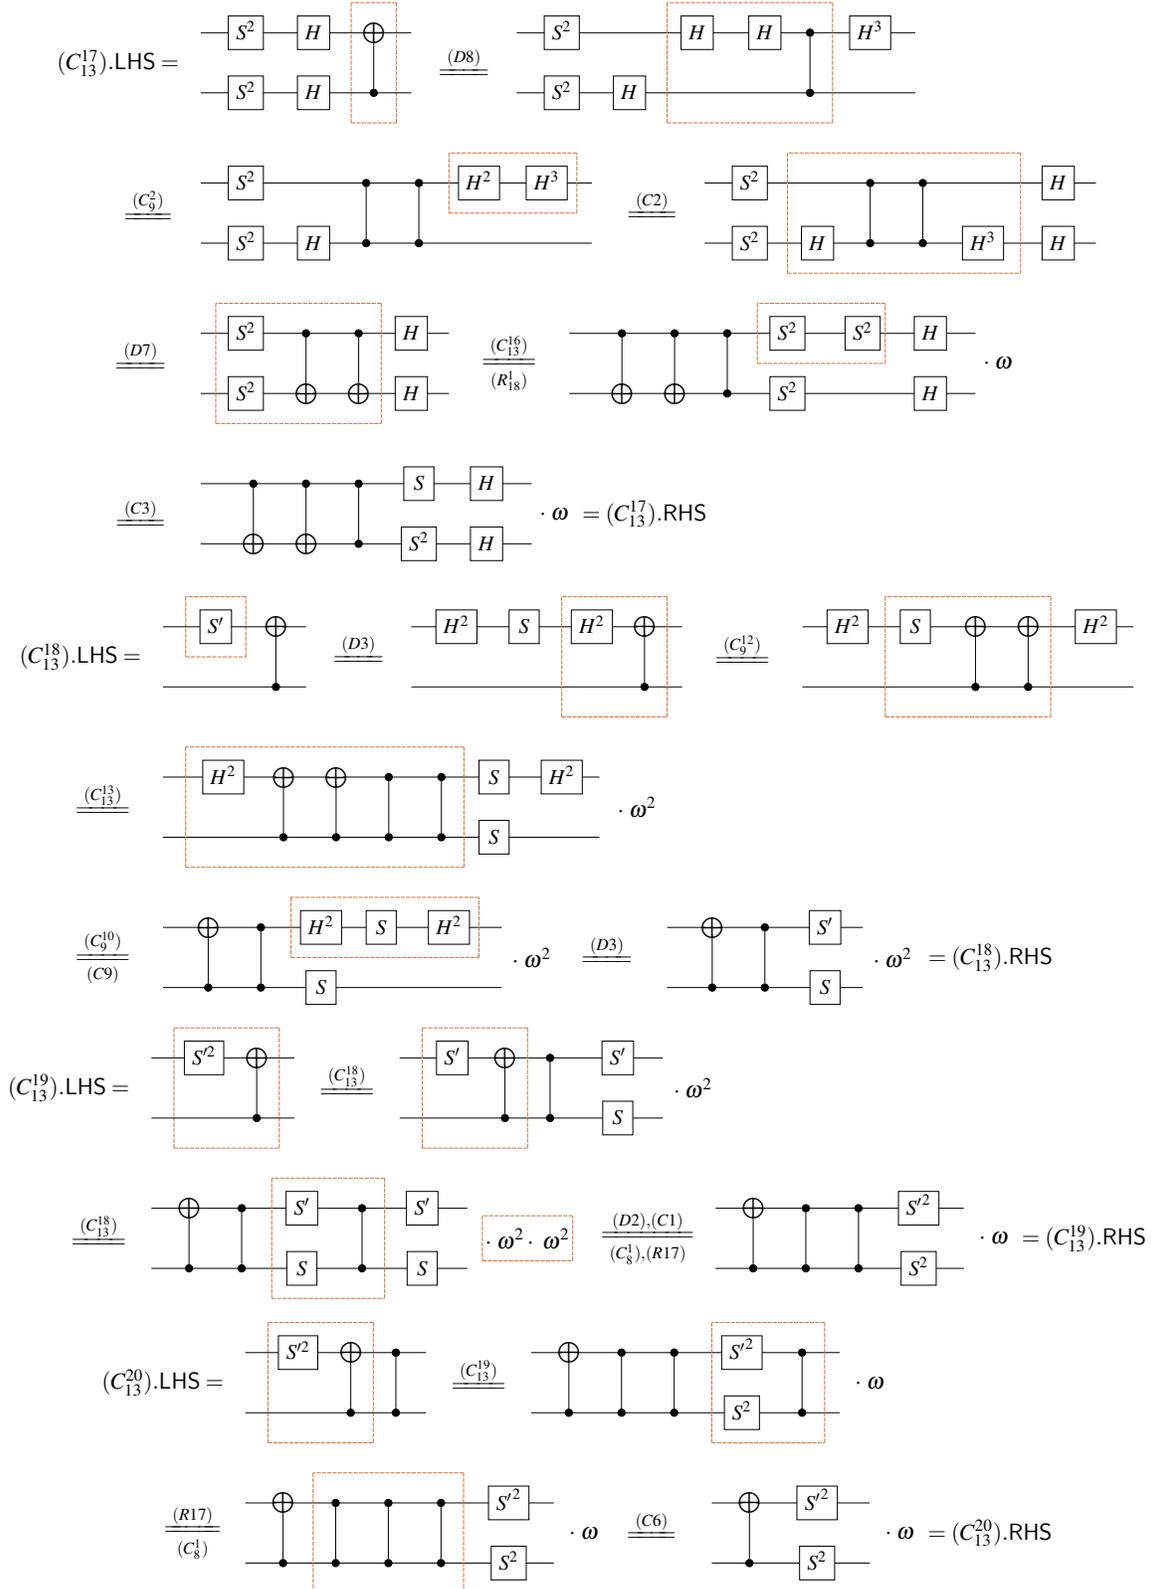

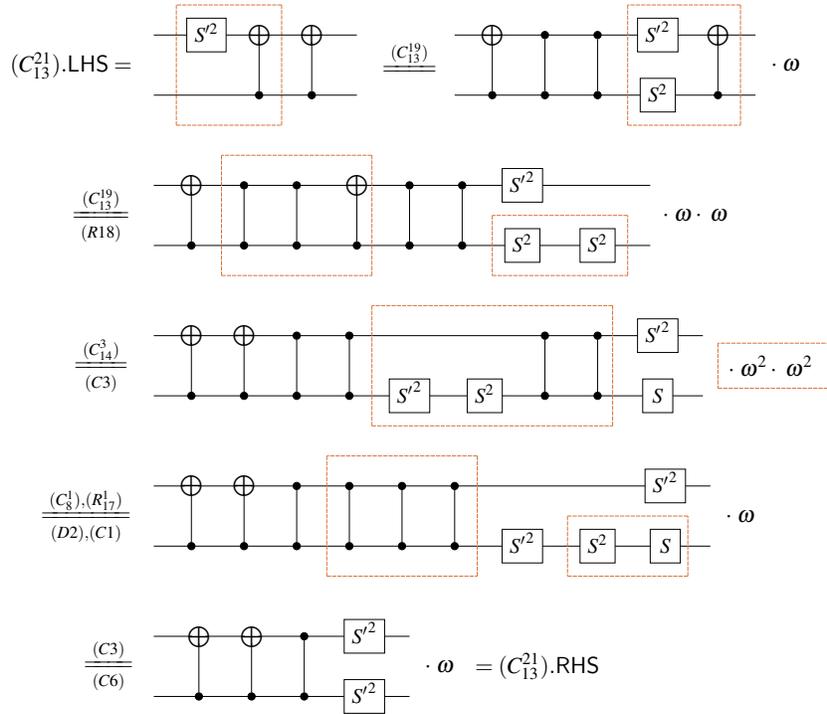

□

**Corollary 3.23.**  $(C_{13}^{22})$  and  $(C_{13}^{23})$  in Figure 26 follow from the reduced relations.

**Lemma 3.24.**  $(R_{24})$  to  $(R_{24}^{11})$  in Figure 27 follow from the equations in Figure 1.

*Proof.* By symmetry, it suffices to prove that  $(R_{24})$ ,  $(R_{24}^2)$ ,  $(R_{24}^4)$ ,  $(R_{24}^6)$ ,  $(R_{24}^8)$ , and  $(R_{24}^{10})$  follow from the

equations in **Figures 1 and 2**.

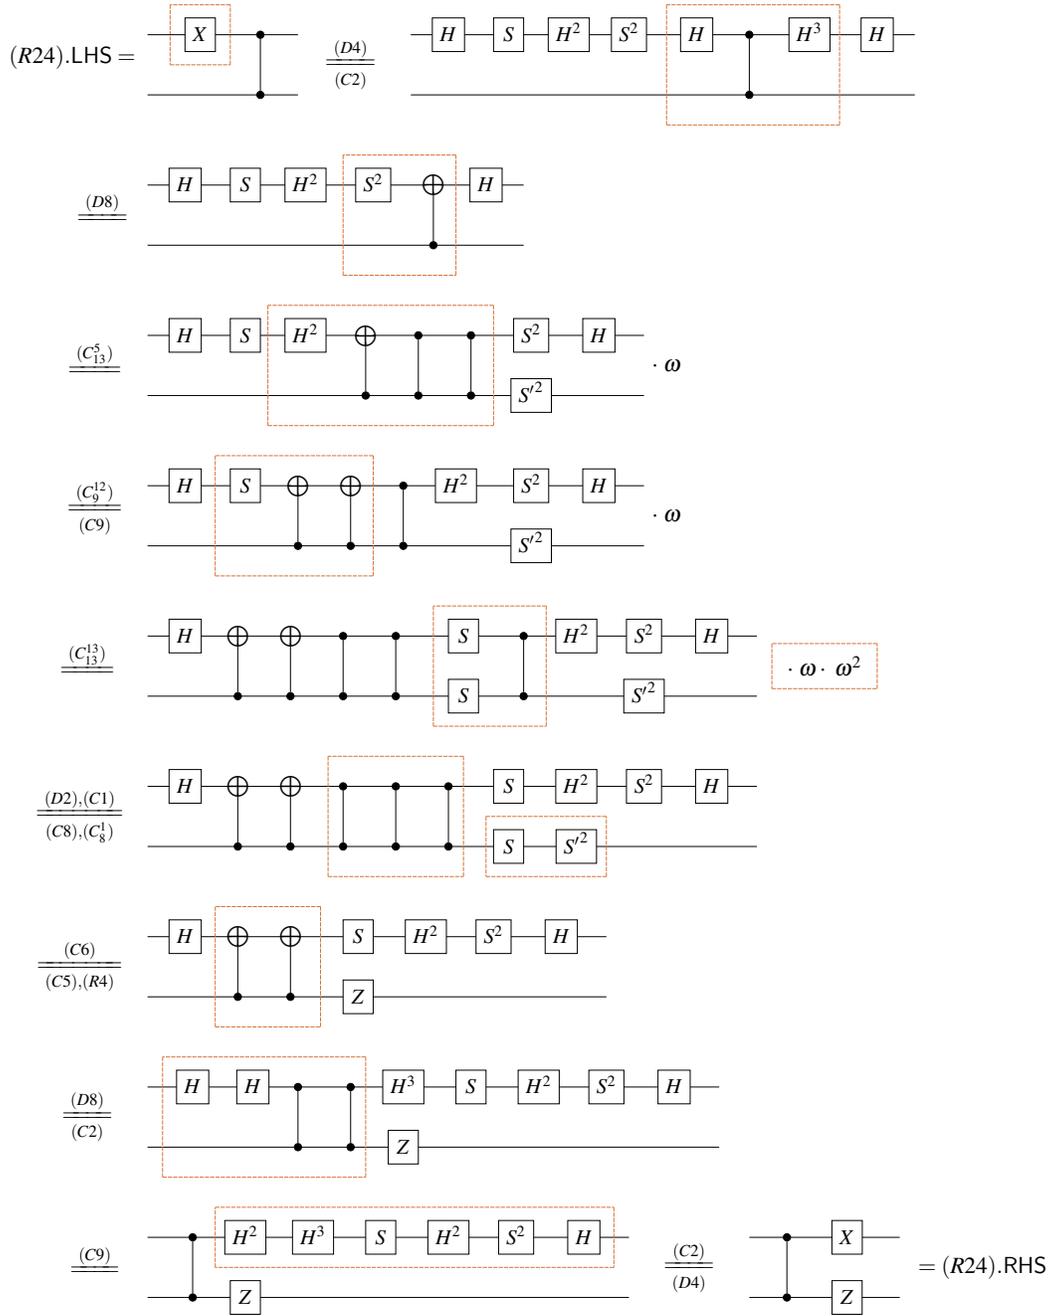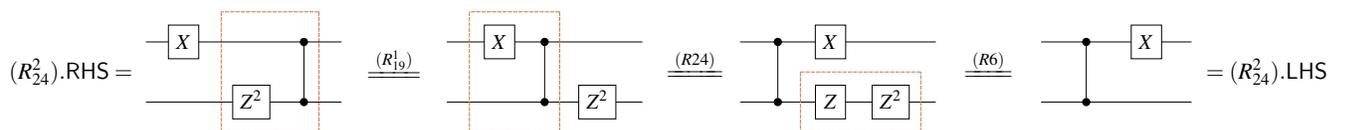

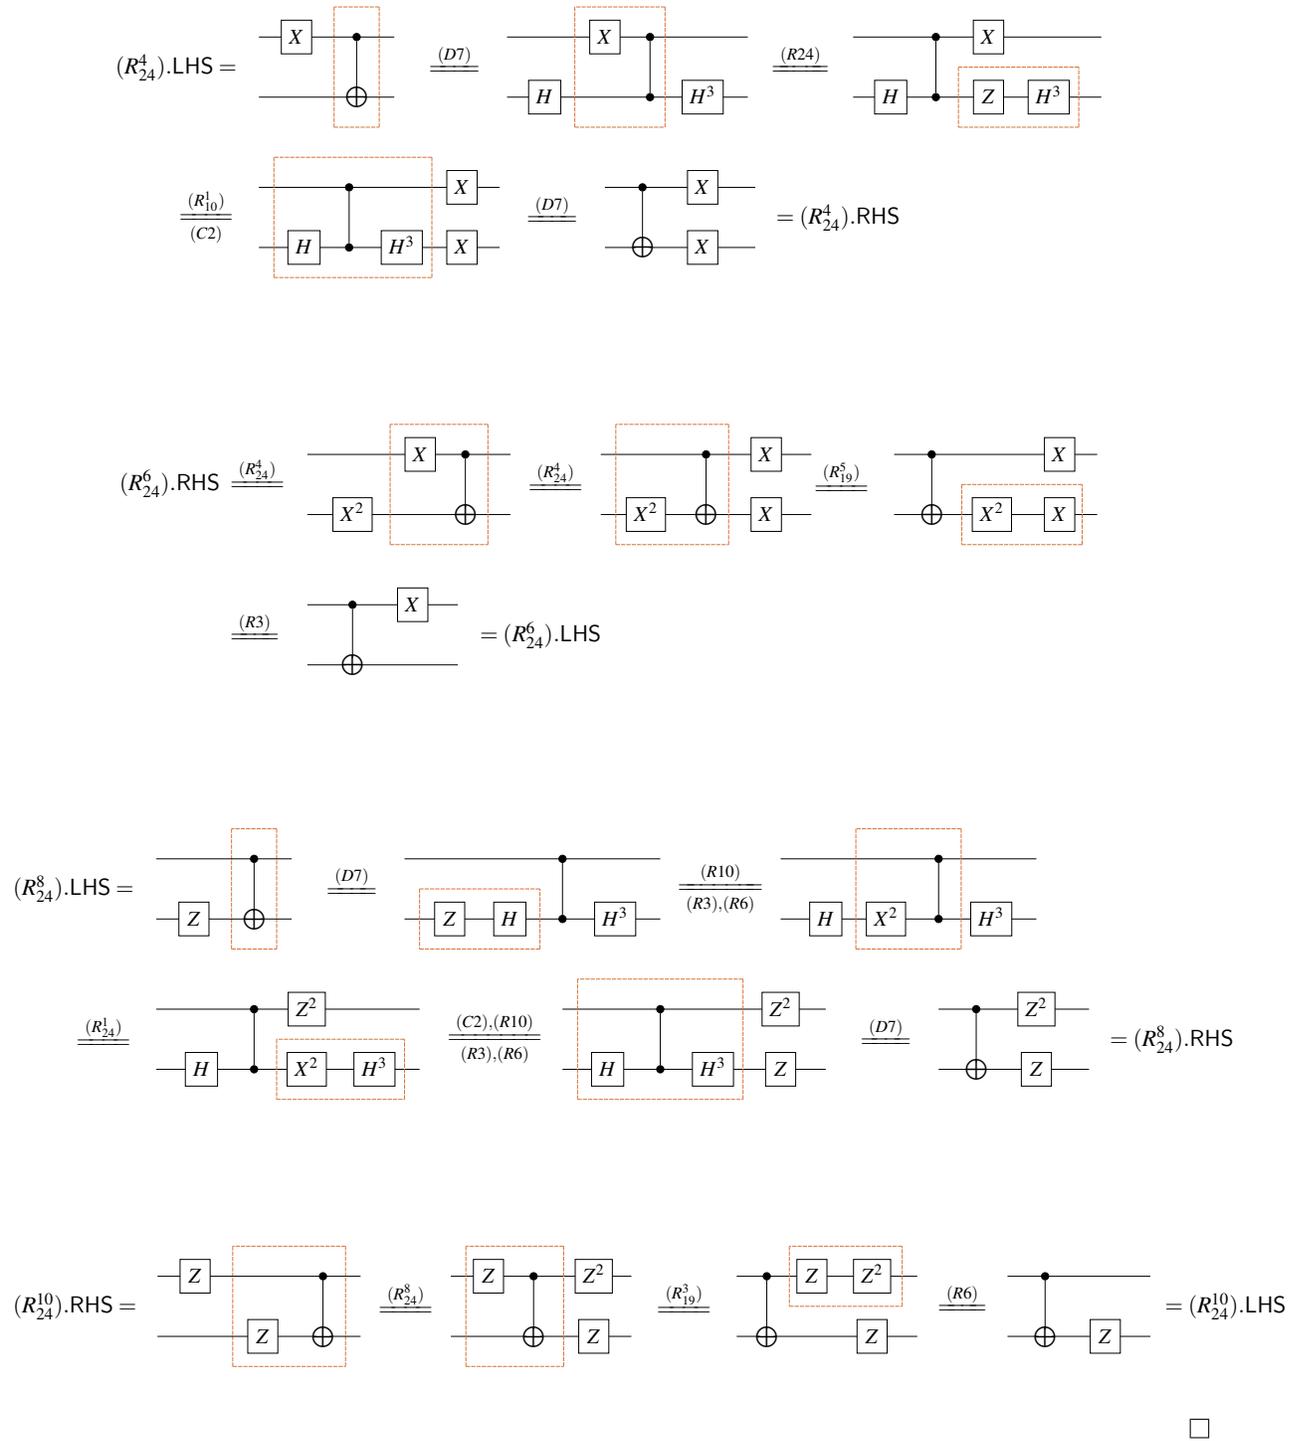

**Lemma 3.25.** The equations in *Figure 28* follow from the equations in *Figure 1*.

$(R25)$  and  $(R_{25}^1)$  follow from the reduced relations.

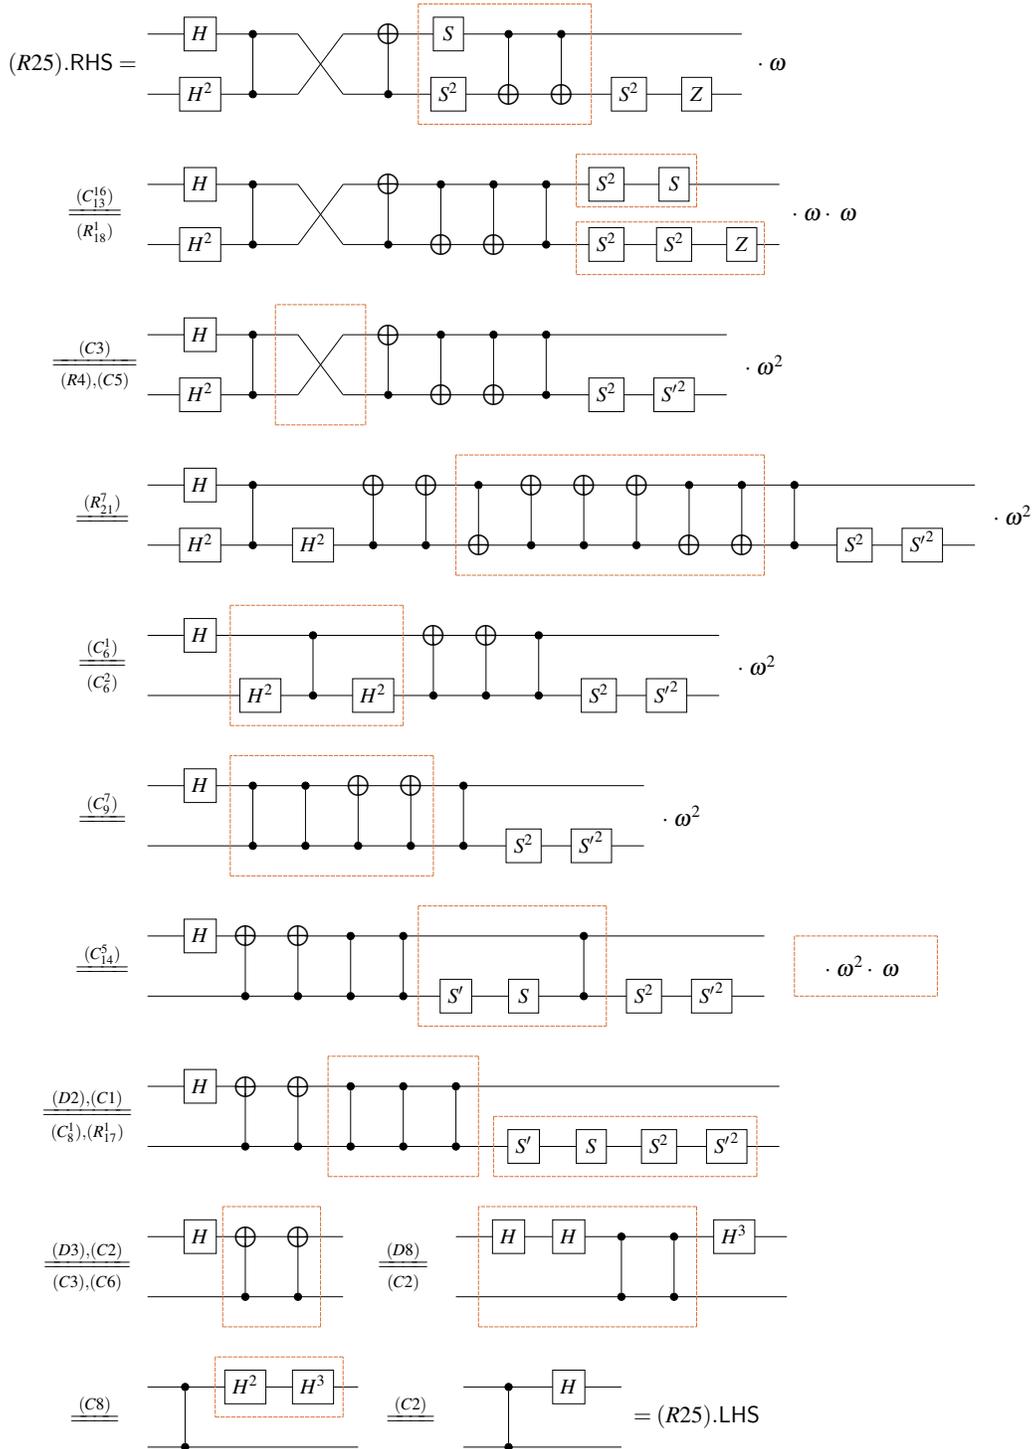

Note that

$$H^3 S^2 Z \stackrel{(R10)}{=} H^3 S^2 (S'^2 S) \stackrel{(C5)}{(C3)} H^3 S'^2 \stackrel{(D3)}{(C2)} H^3 (H^2 S^2 H^2) \stackrel{(C2)}{=} H S^2 H^2. \quad (25)$$

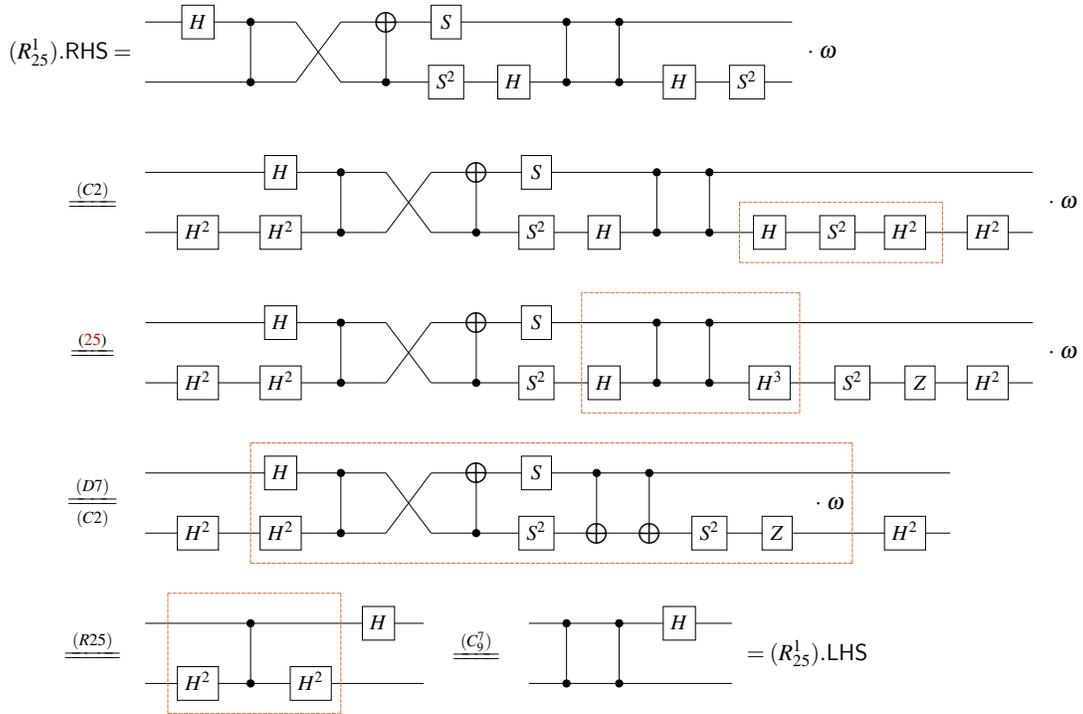

**(R26)** follows from the reduced relations.

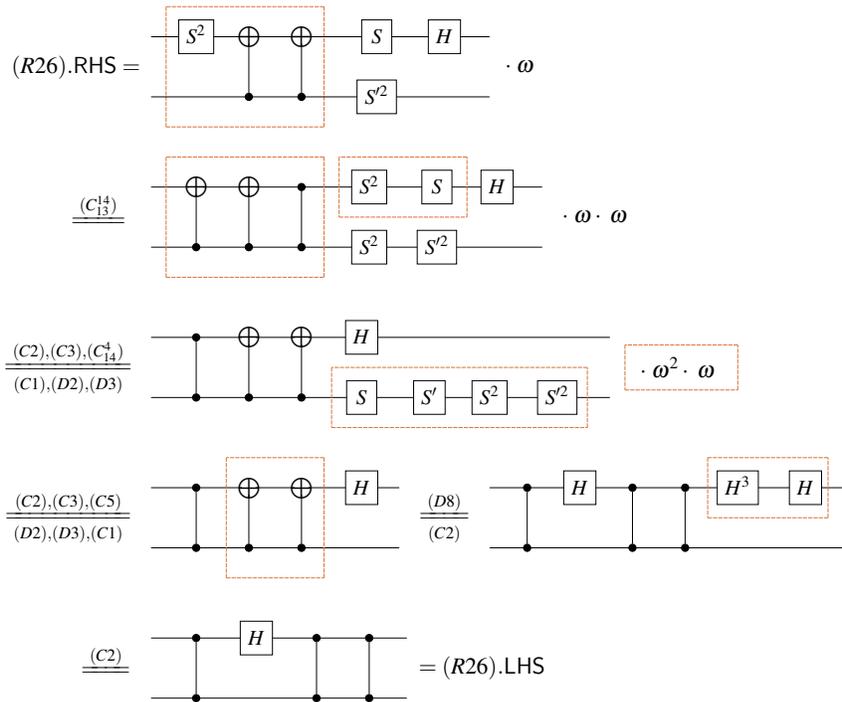

(R27) follows from the reduced relations.

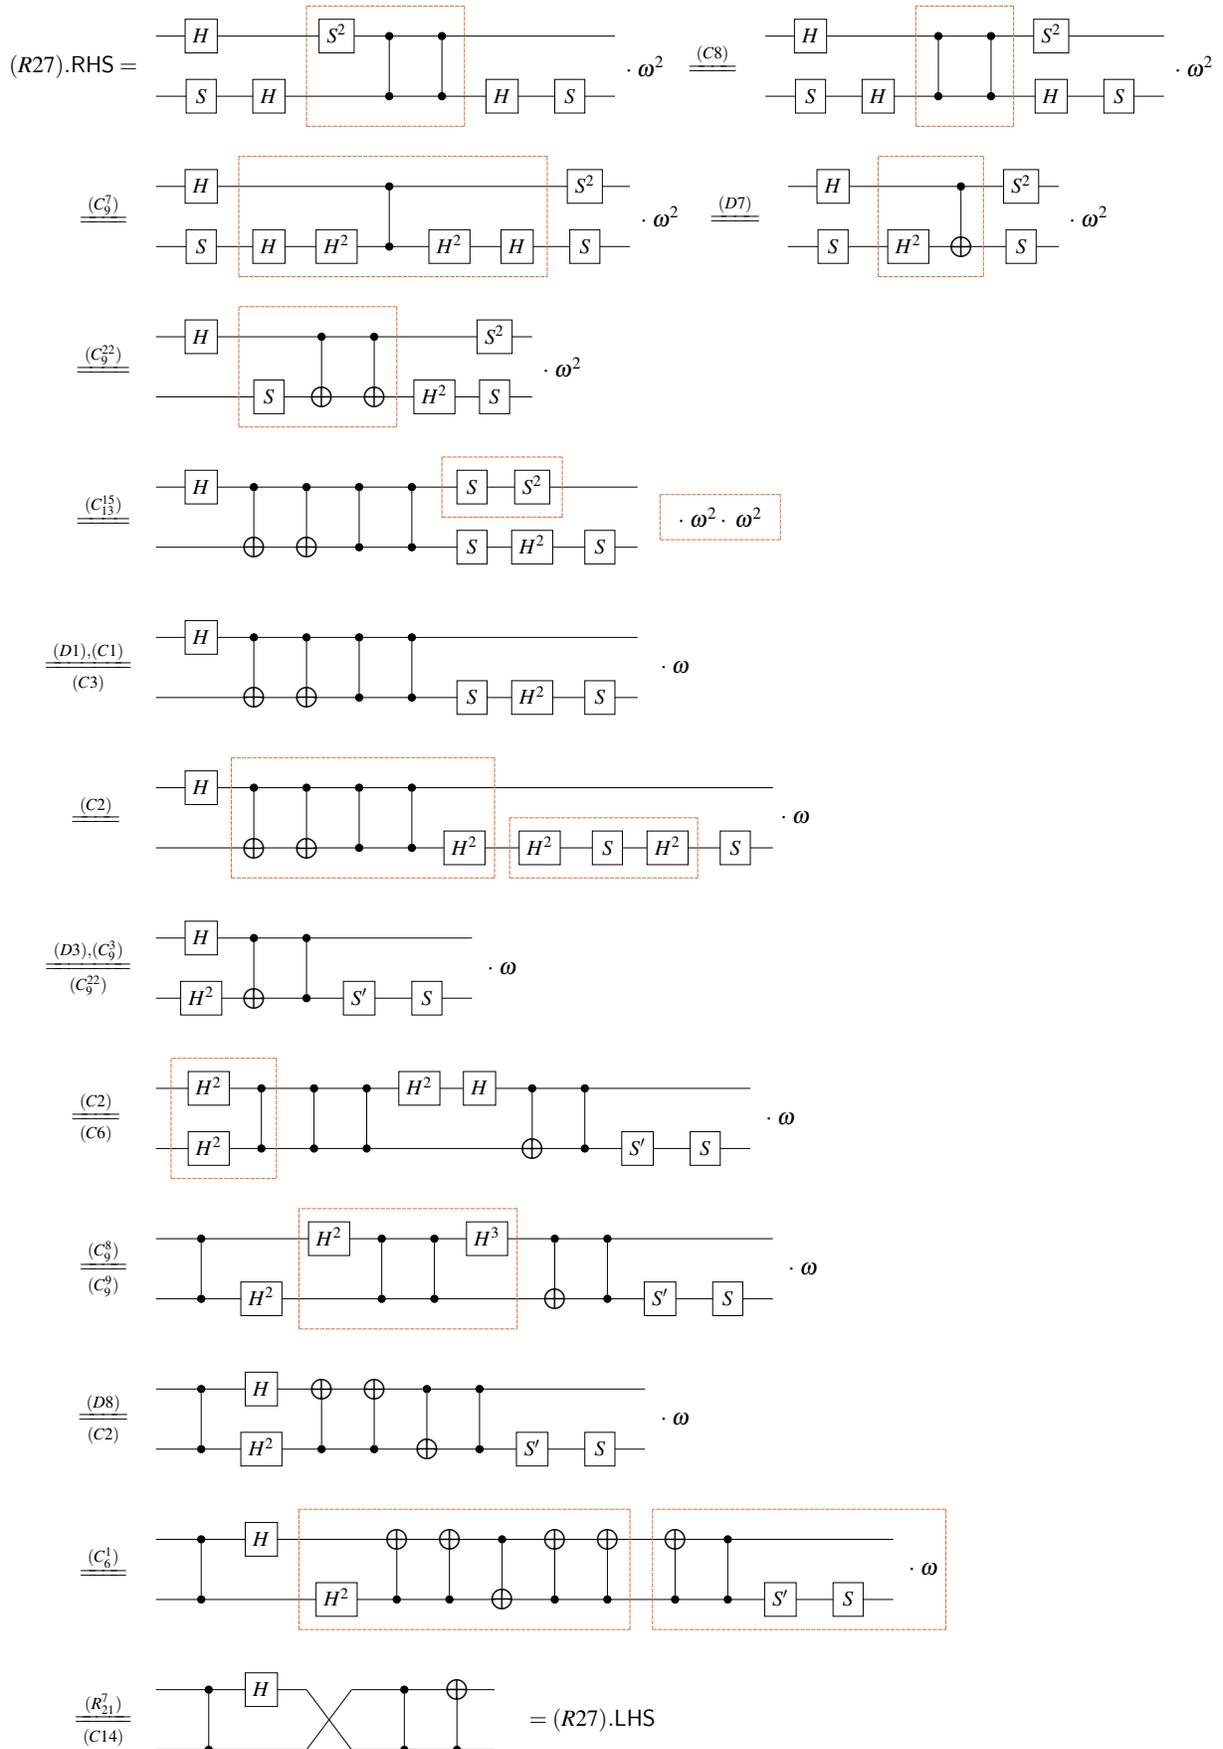



Left-appepending both sides of (26) by  $I \otimes H^3$  yields

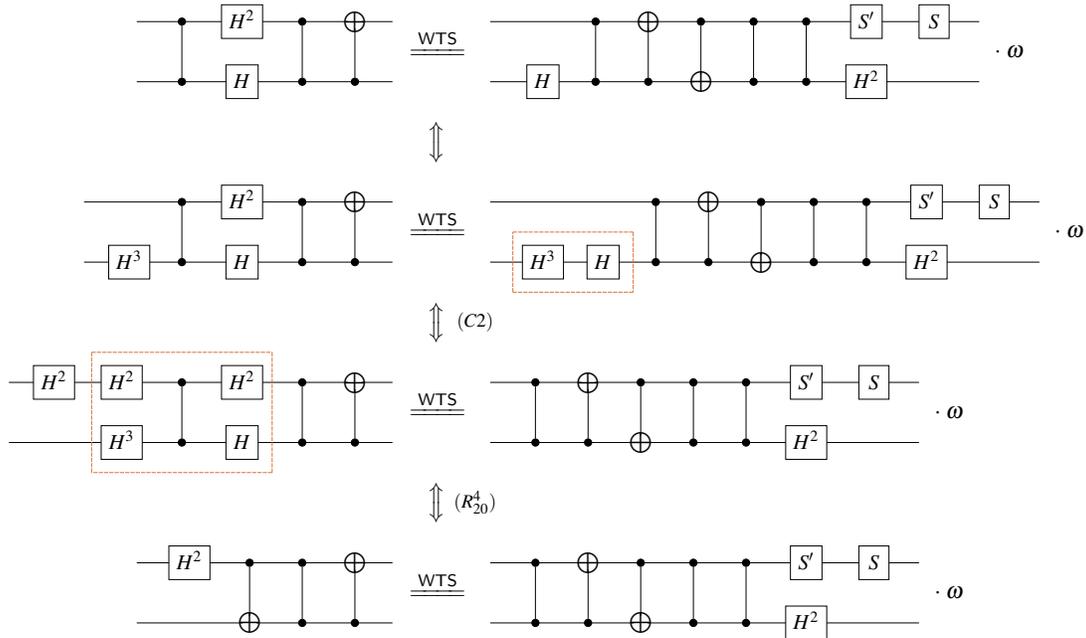

Hence, it suffices to show that (27) follows from the reduced relations.

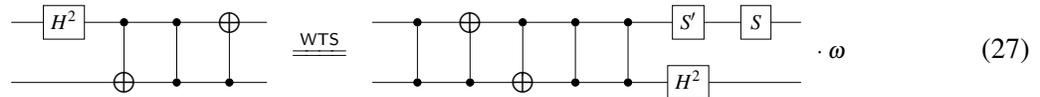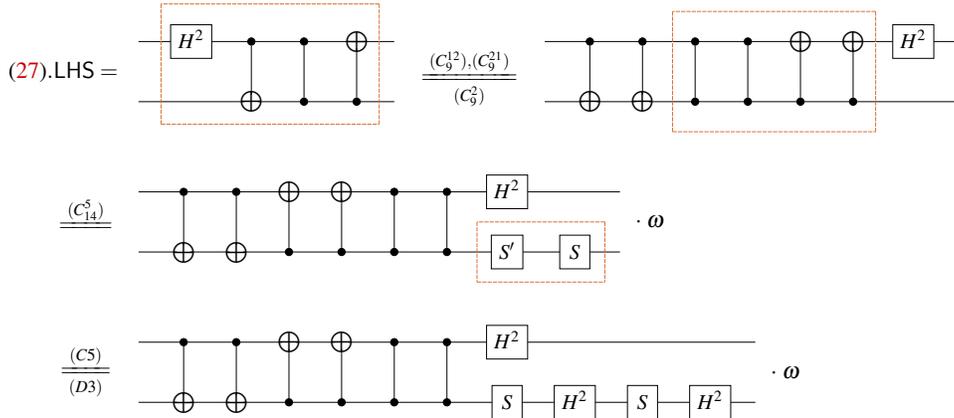

This implies that

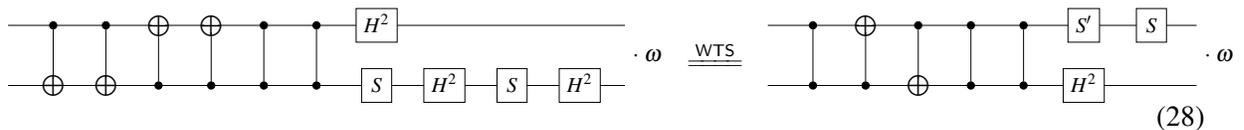

(28) can be further simplified as follows.

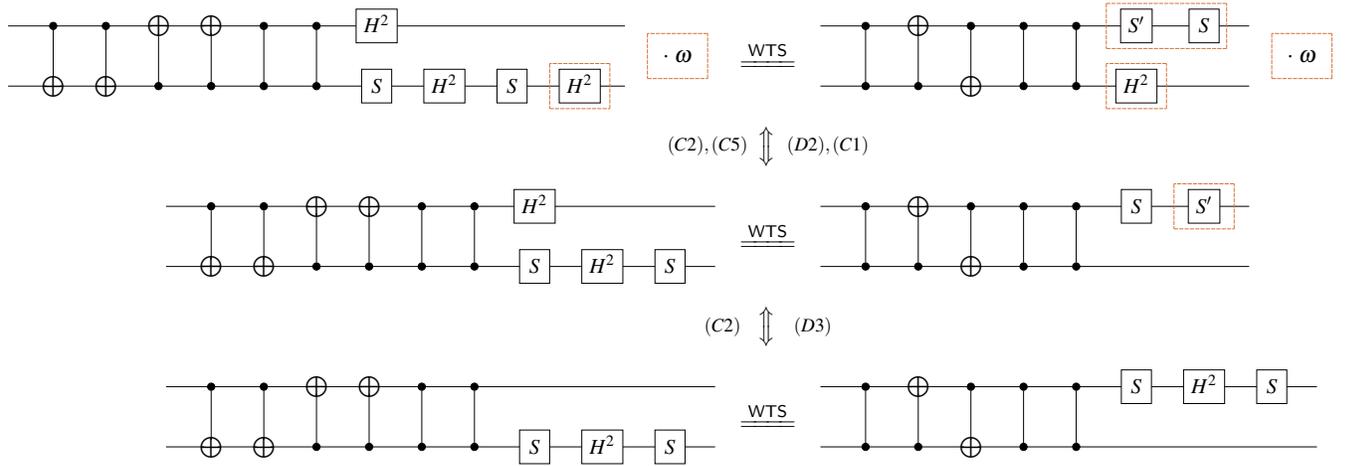

This means our problem is reduced to showing (29), whose RHS can be simplified as shown in (30).

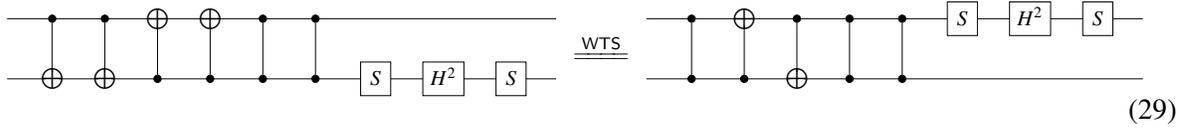

By  $(R_{22}^4)$  and the rewrites below, we complete the proof.

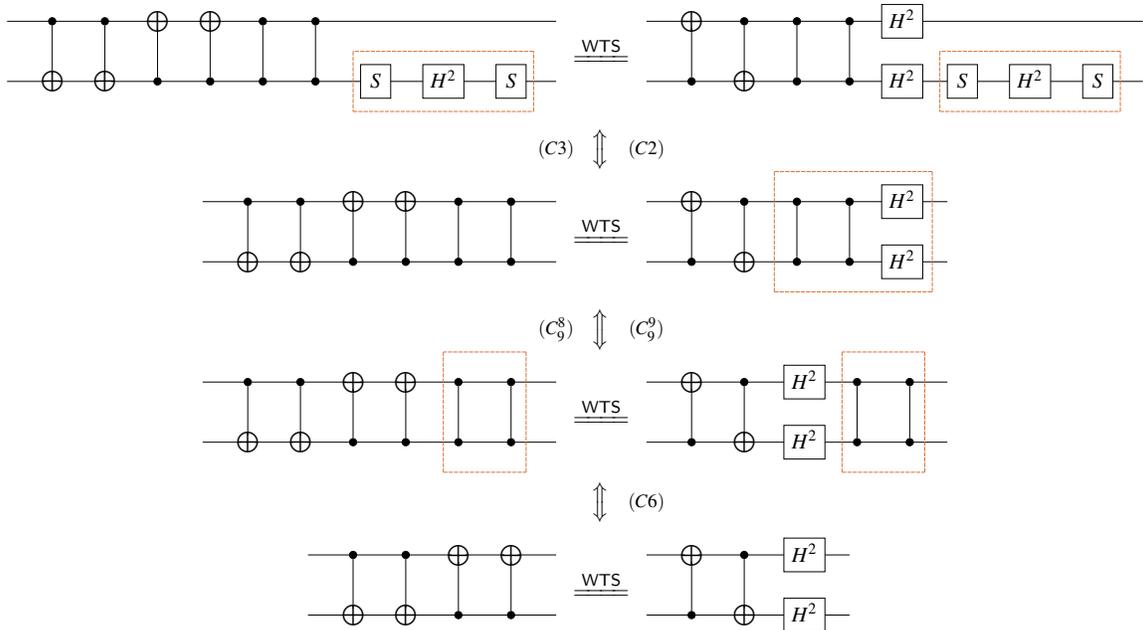

(16).RHS = 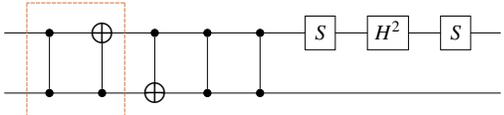

(C14) 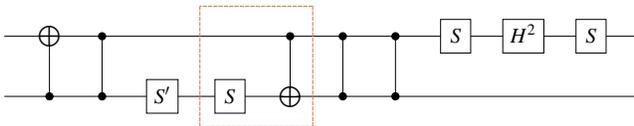 ·  $\omega$

(C'13) 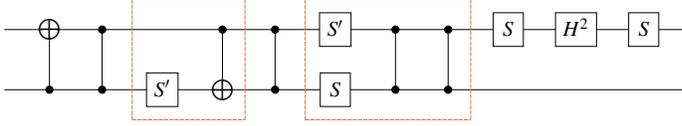 ·  $\omega \cdot \omega^2$

(D2),(C1),(C'8)  
(R17),(C'13) 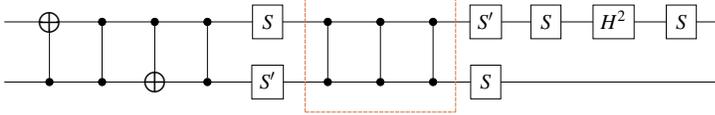 ·  $\omega^2$

(C6) 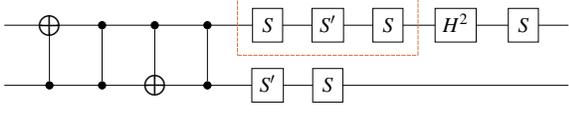 ·  $\omega^2$

(C5)  
(D3) 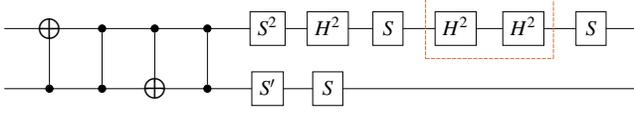 ·  $\omega^2$

(C2) 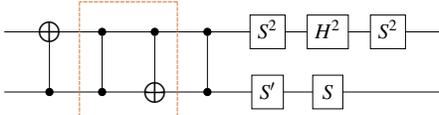 ·  $\omega^2$

(C'14) 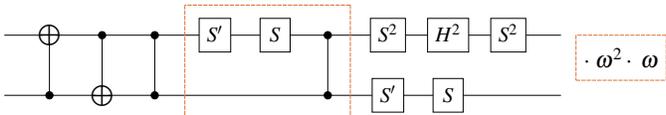 ·  $\omega^2 \cdot \omega$

(D2),(C1)  
(C8),(R17) 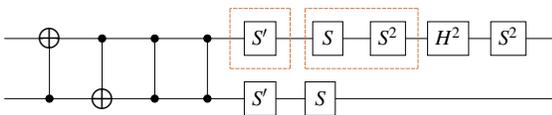

(D3)  
(C3) 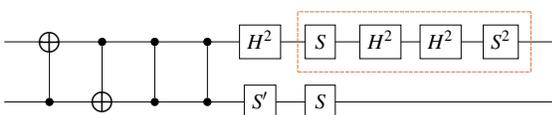

(C2)  
(C3) 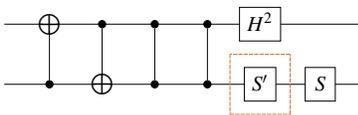 (D3) 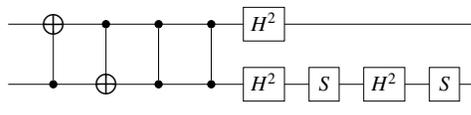

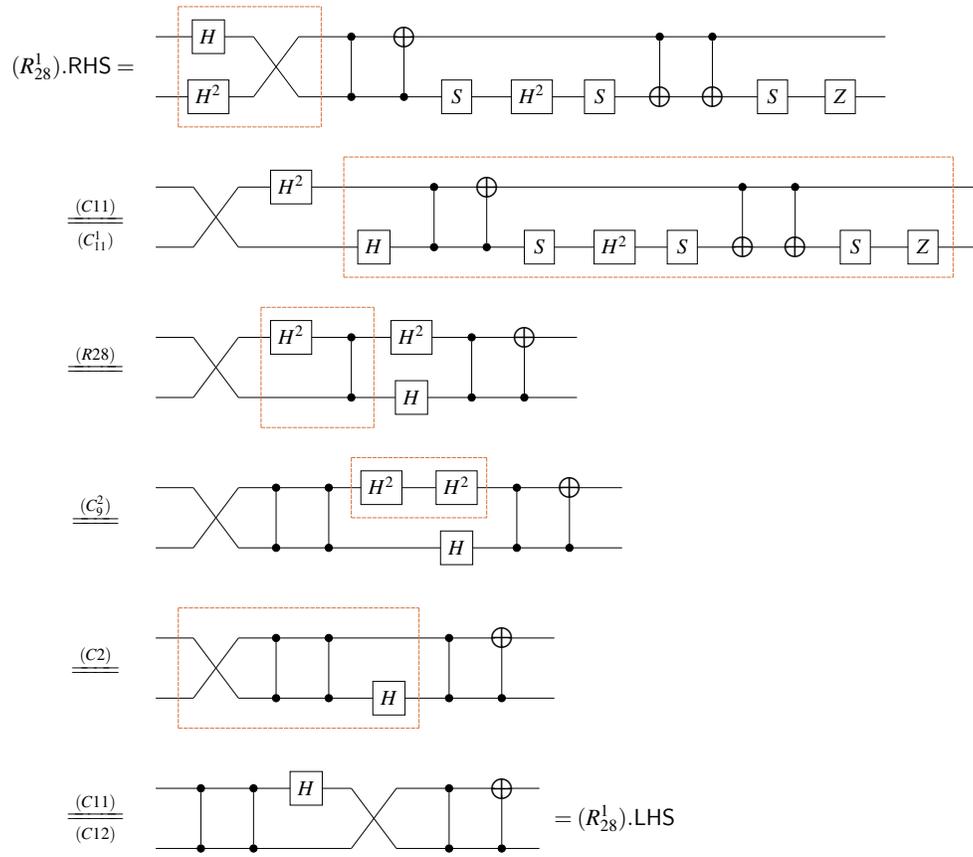

(R29) follows from the reduced relations.

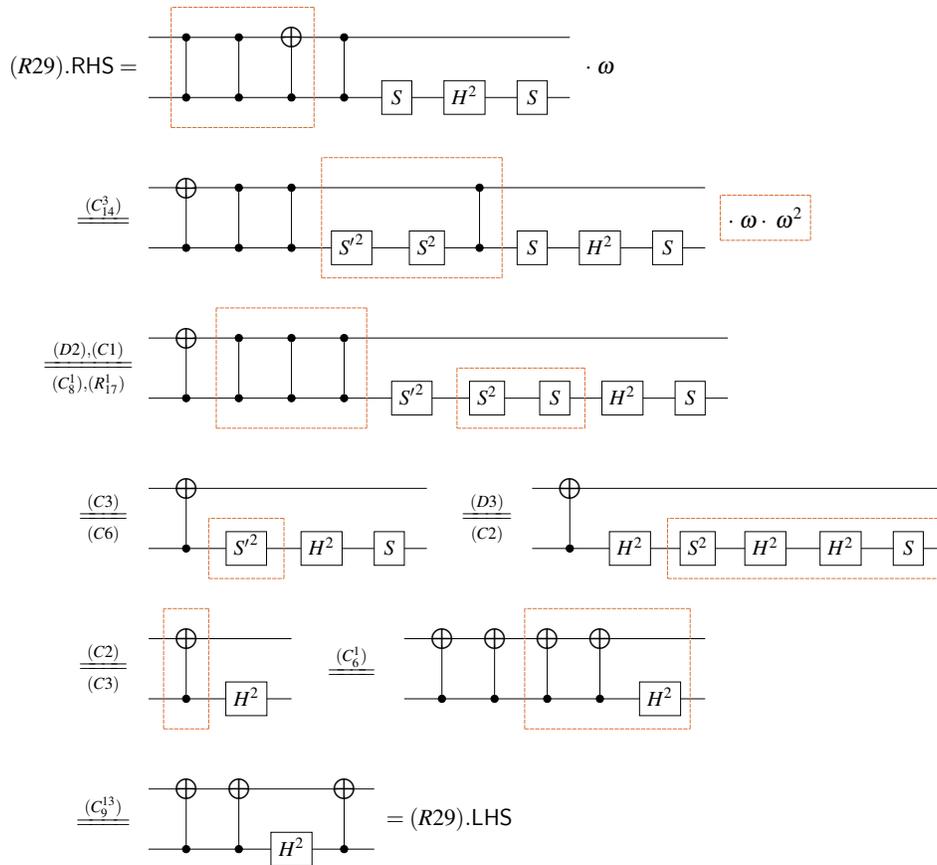

(R30) follows from the reduced relations.

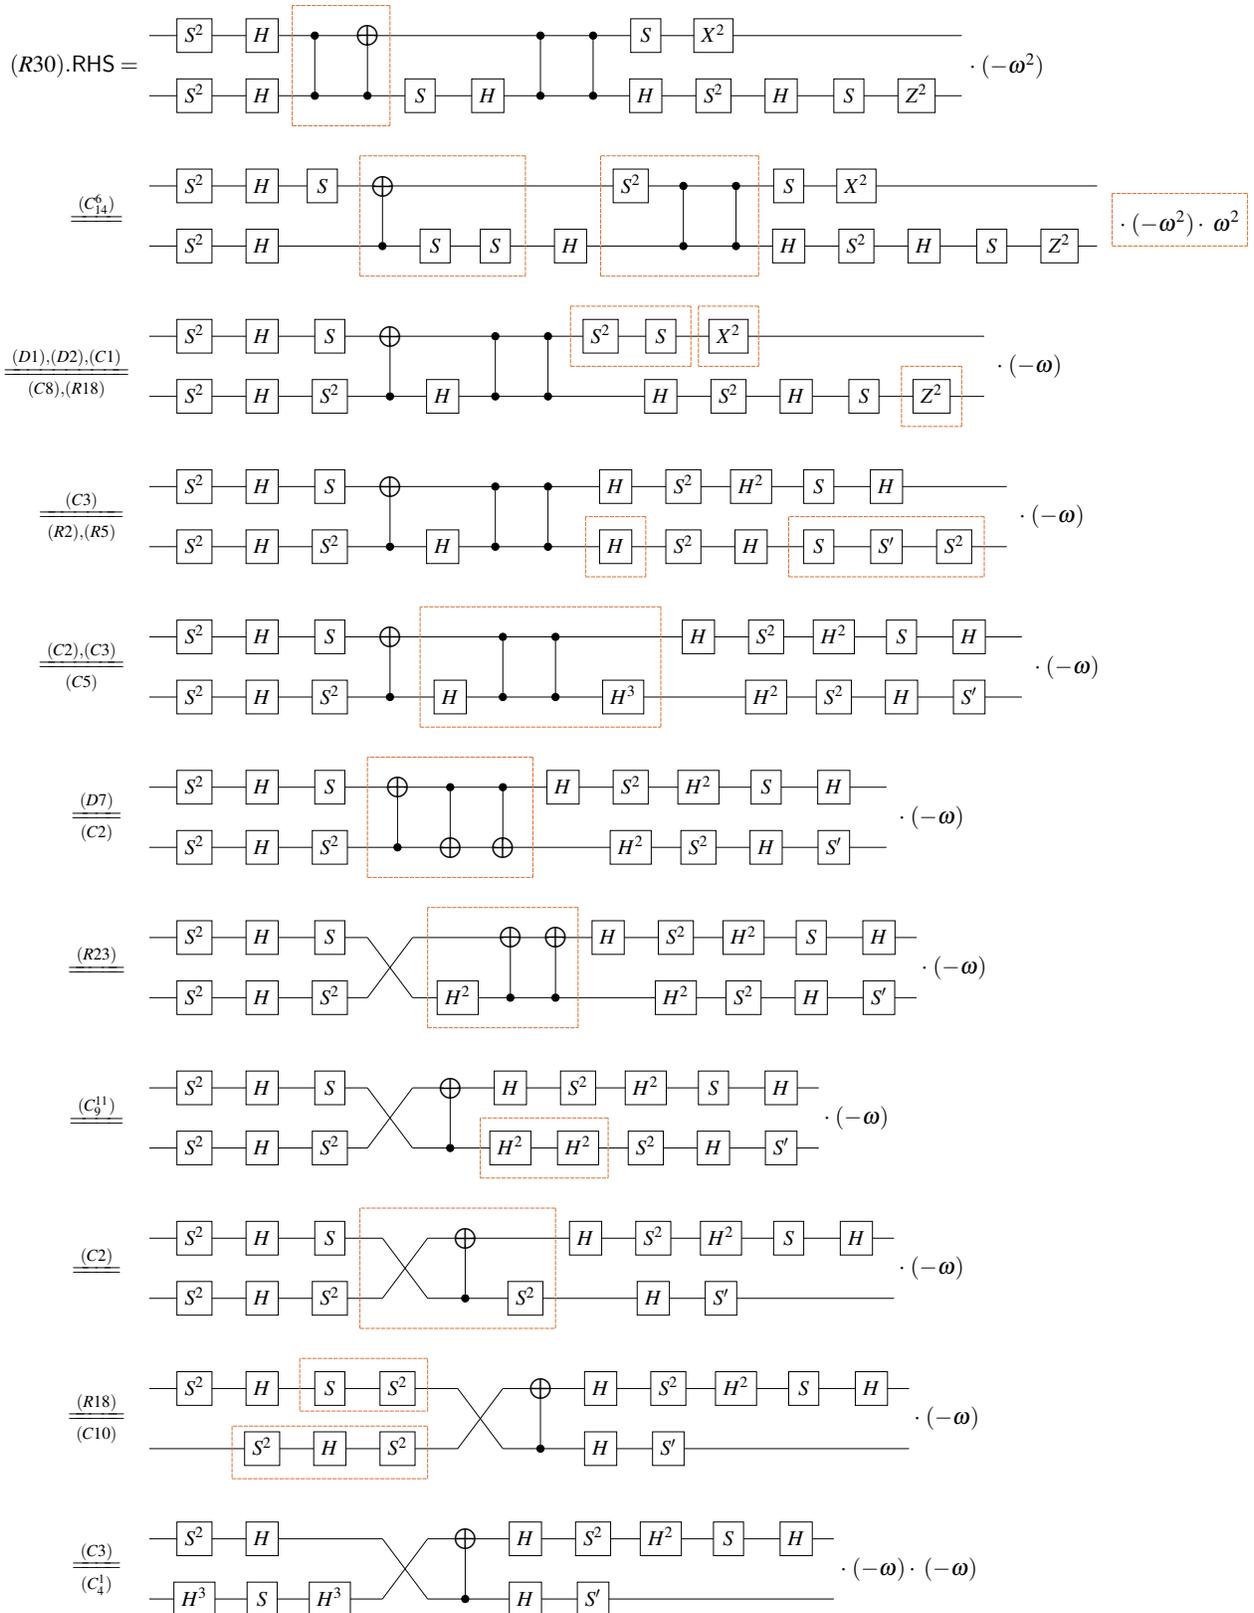

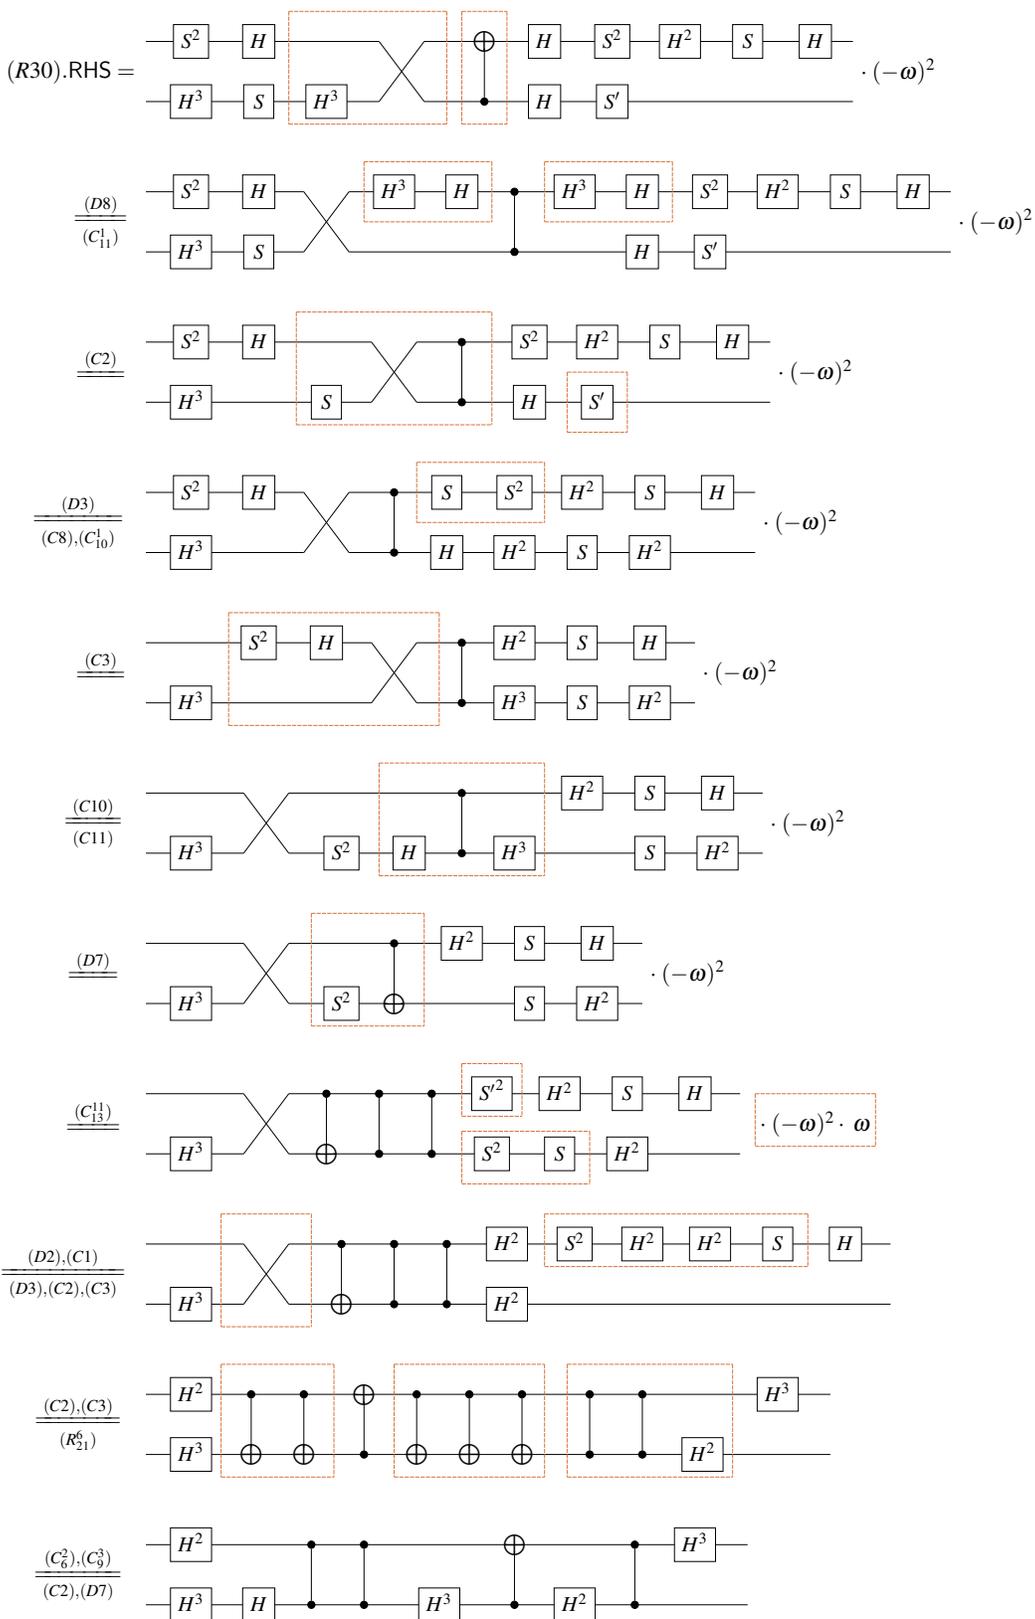

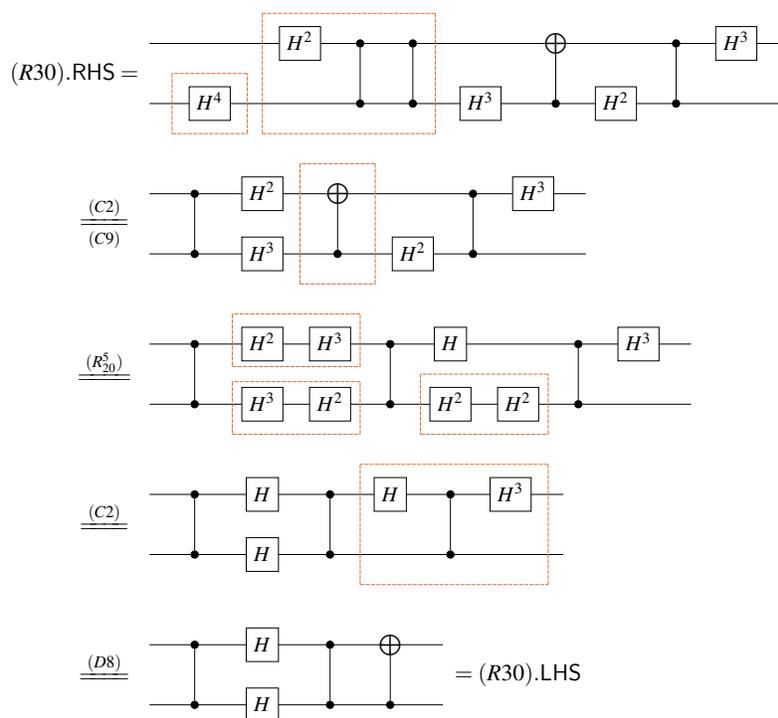

(R31) follows from the reduced relations. Note that

$$Z^2 S^2 H S^2 Z^2 \stackrel{(R11)}{=} (S' S^2) S^2 H S^2 (S' S^2) \stackrel{(C3)}{\stackrel{(C5)}}{=} S' S H S S' \quad (31)$$

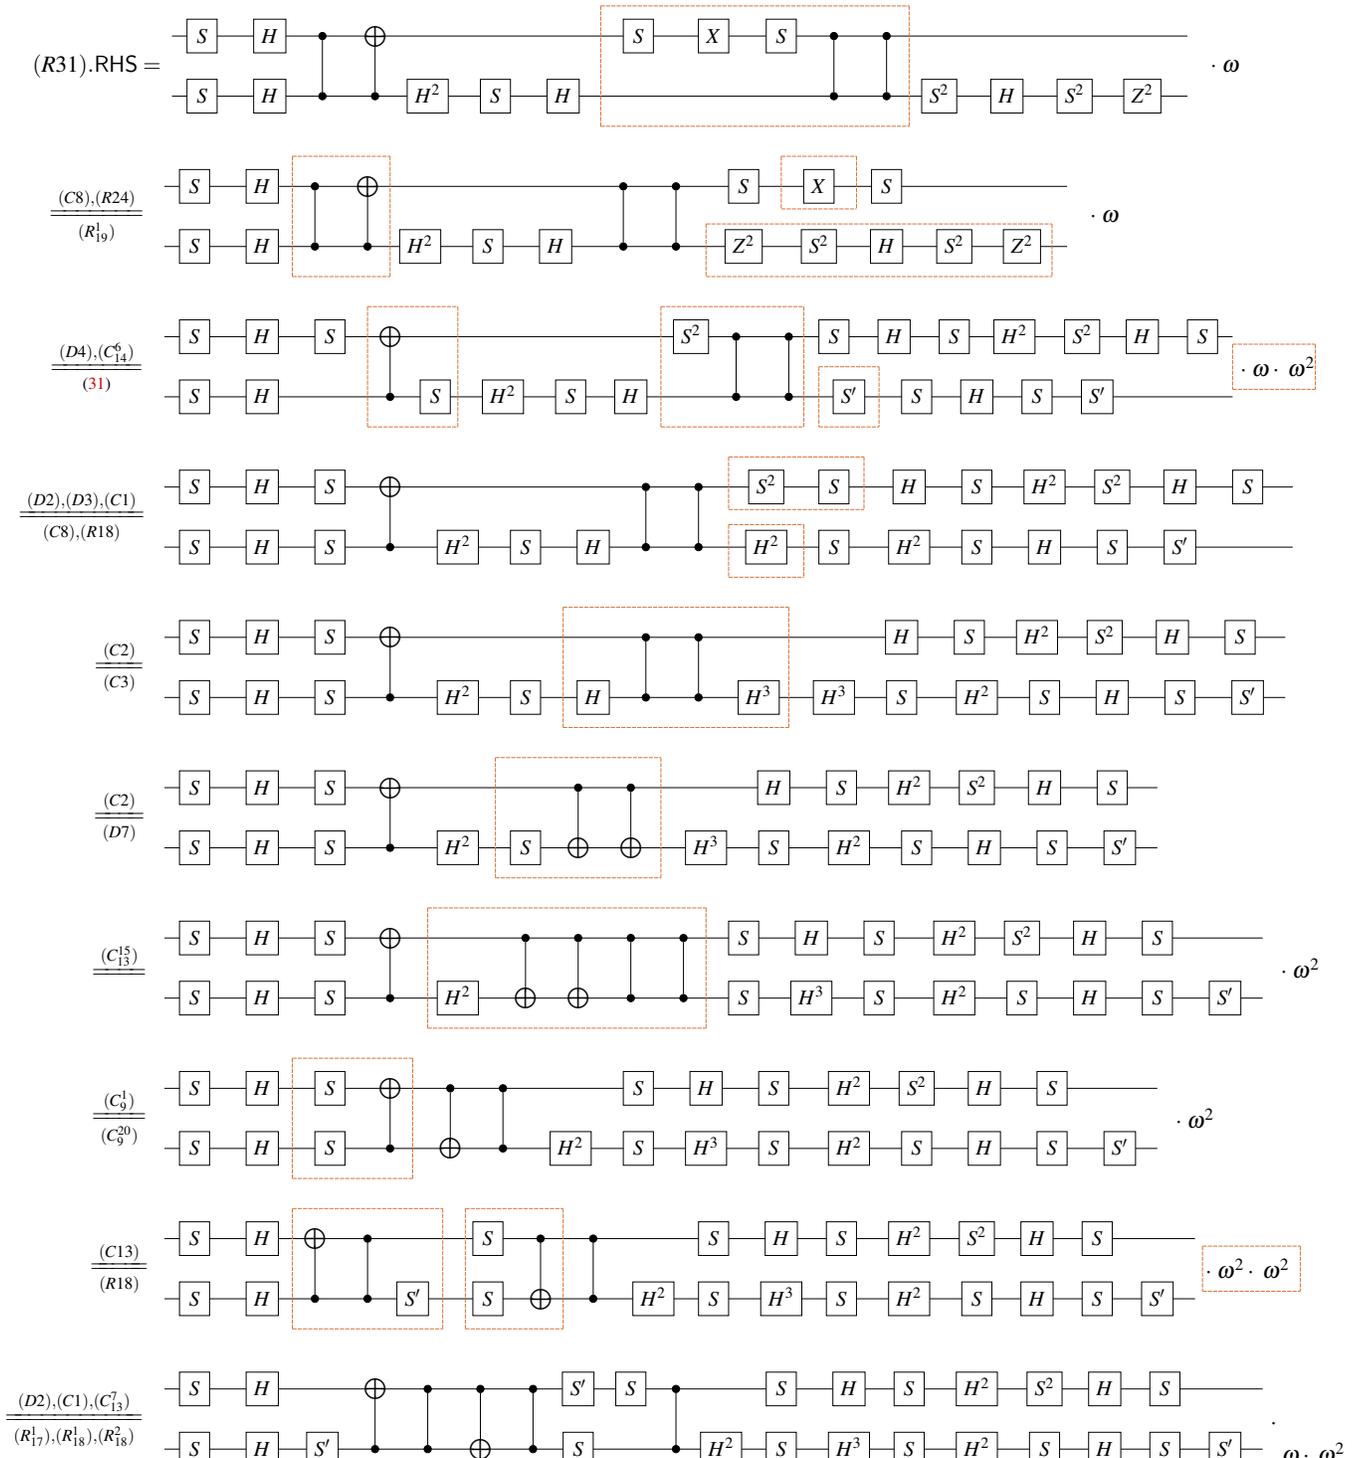

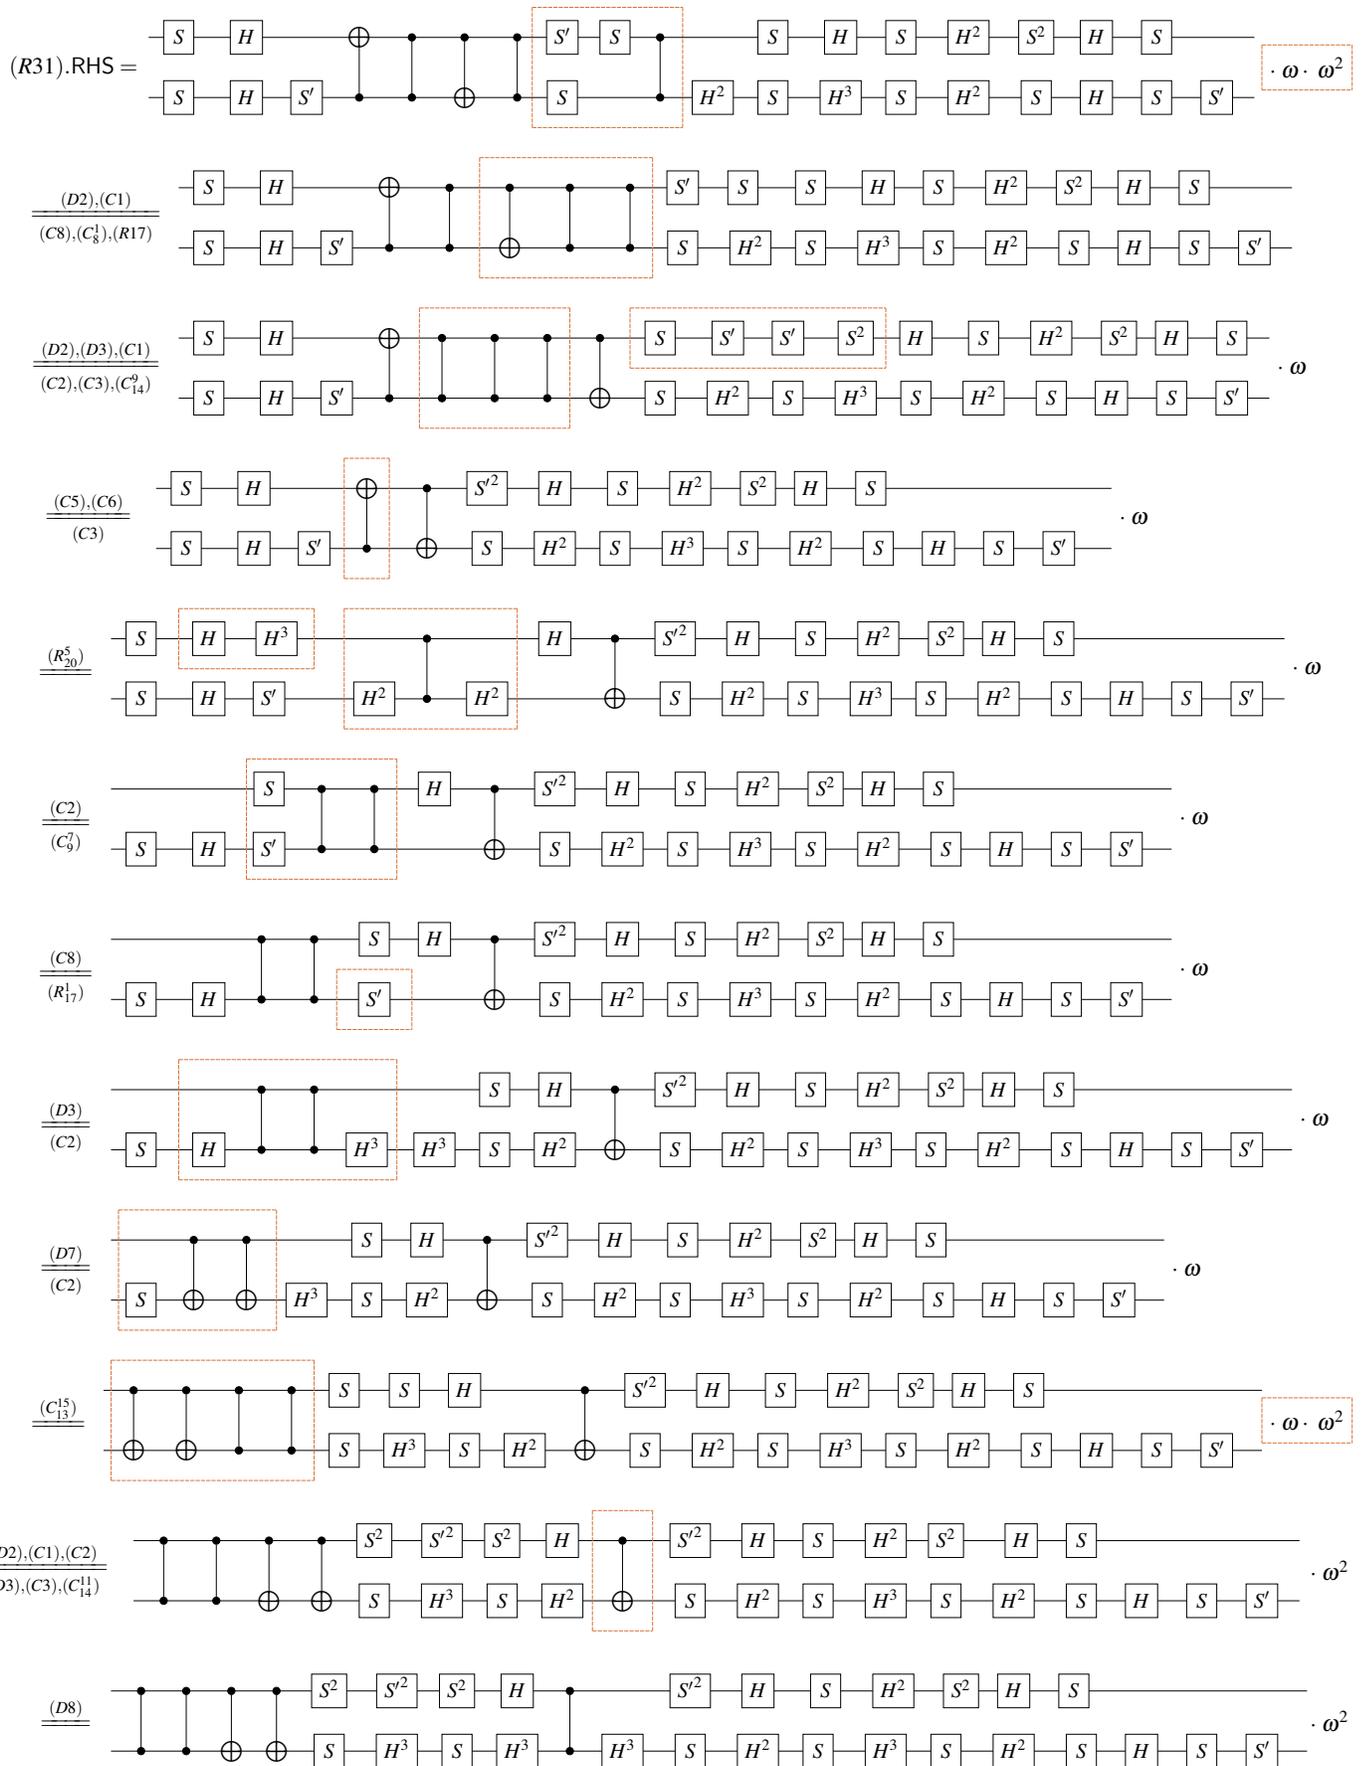

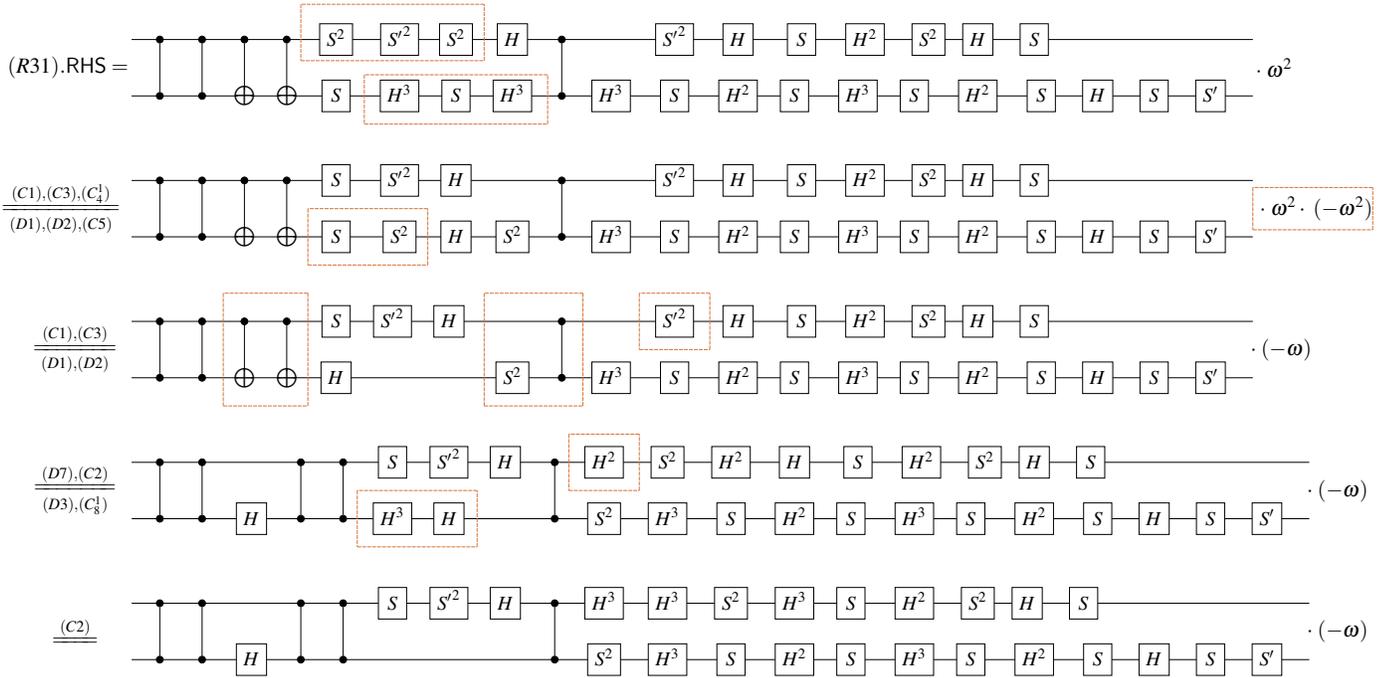

Hence, our problem is reduced to showing (32), both sides of which are simplified in (33) and (34). Therefore, it suffices to show that

$$HS^2H^2SH^3S^2H^3SH^2S^2HS \stackrel{\text{WTS}}{=} 1 \quad (\text{top})$$

$$SS'H^3SH^2SH^3SH^2SH \stackrel{\text{WTS}}{=} -1 \quad (\text{bottom})$$

Based on the derivations below, we complete the proof.

$$\begin{aligned}
(\text{top}).\text{LHS} &= HS^2H^2SH^3S^2H^3SH^2S^2HS \\
&\stackrel{(C2)}{=} HS^2H^2SH^3S^2H^3SH^2S^2(H^2H^3)S \\
&\stackrel{(D3)}{=} HS^2H^2SH^3S^2H^3SS^2H^3S \\
&\stackrel{(C2)}{=} HS^2H^2SH^3S^2H^3SS'^2(H^2HS^2H \cdot (-\omega^2)) \\
&\stackrel{(C5)}{=} HS^2H^2SH^3S^2H^3S'^2HS^2H \cdot (-\omega^2) \\
&\stackrel{(C3)}{=} HS^2H^2SH^3S^2H^3(H^2S^2H^2)HS^2H \cdot (-\omega^2) \\
&\stackrel{(D3)}{=} HS^2H^2SH^3S^2H^3(H^2S^2H^2)HS^2H \cdot (-\omega^2) \\
&\stackrel{(C2)}{=} HS^2H^2SH^3(S^2HS^2)H^3S^2H \cdot (-\omega^2) \\
&\stackrel{(C4)}{=} HS^2H^2SH^3(H^3SH^3)H^3S^2H \cdot (-\omega^2) \cdot (-\omega) \\
&\stackrel{(D1),(D2)}{=} HS^2(H^2SH^2)SH^2S^2H \stackrel{(D3)}{=} HS^2(S'S)H^2S^2H \\
&\stackrel{(C1),(C2)}{=} HS'H^2S^2H \stackrel{(D3)}{=} H(H^2SH^2)H^2S^2H \stackrel{(C2)}{=} H^3H \stackrel{(C2)}{=} 1. \\
&\stackrel{(C3)}{=}
\end{aligned}$$

$$\begin{aligned}
 \text{(bottom).LHS} &= SS'H^3SH^2S(H^3S)H^2SH \\
 &\stackrel{(C_4^1)}{=} SS'H^3SH^2S(S^2HS^2H)H^2SH \cdot (-\omega^2) \\
 &\stackrel{(C_3)}{=} SS'(H^3SH^3)S^2H^3SH \cdot (-\omega^2) \\
 &\stackrel{(C_4^1)}{\stackrel{(C_1)}{=}} SS'(S^2HS^2)S^2H^3SH \cdot (-\omega^2) \cdot (-\omega)^5 \\
 &\stackrel{(C_1),(C_3),(C_5)}{\stackrel{(D_1),(D_2)}{=}} S'HSH^3SH \cdot \omega \\
 &\stackrel{(D_3)}{=} H^2S(H^2HSH^3)SH \cdot \omega \\
 &\stackrel{(C_4^1)}{\stackrel{(C_1)}{=}} H^2S(S^2HS^2)SH \cdot \omega \cdot (-\omega)^5 \\
 &\stackrel{(C_1),(C_3)}{\stackrel{(D_1),(D_2)}{=}} H^2HH \cdot (-1) \stackrel{(C_2)}{=} -1.
 \end{aligned}$$

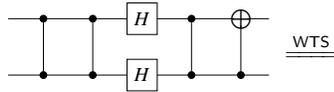

WTS

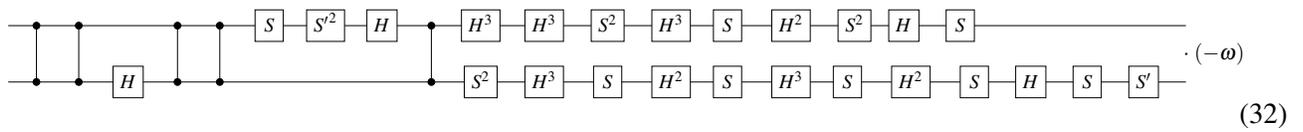

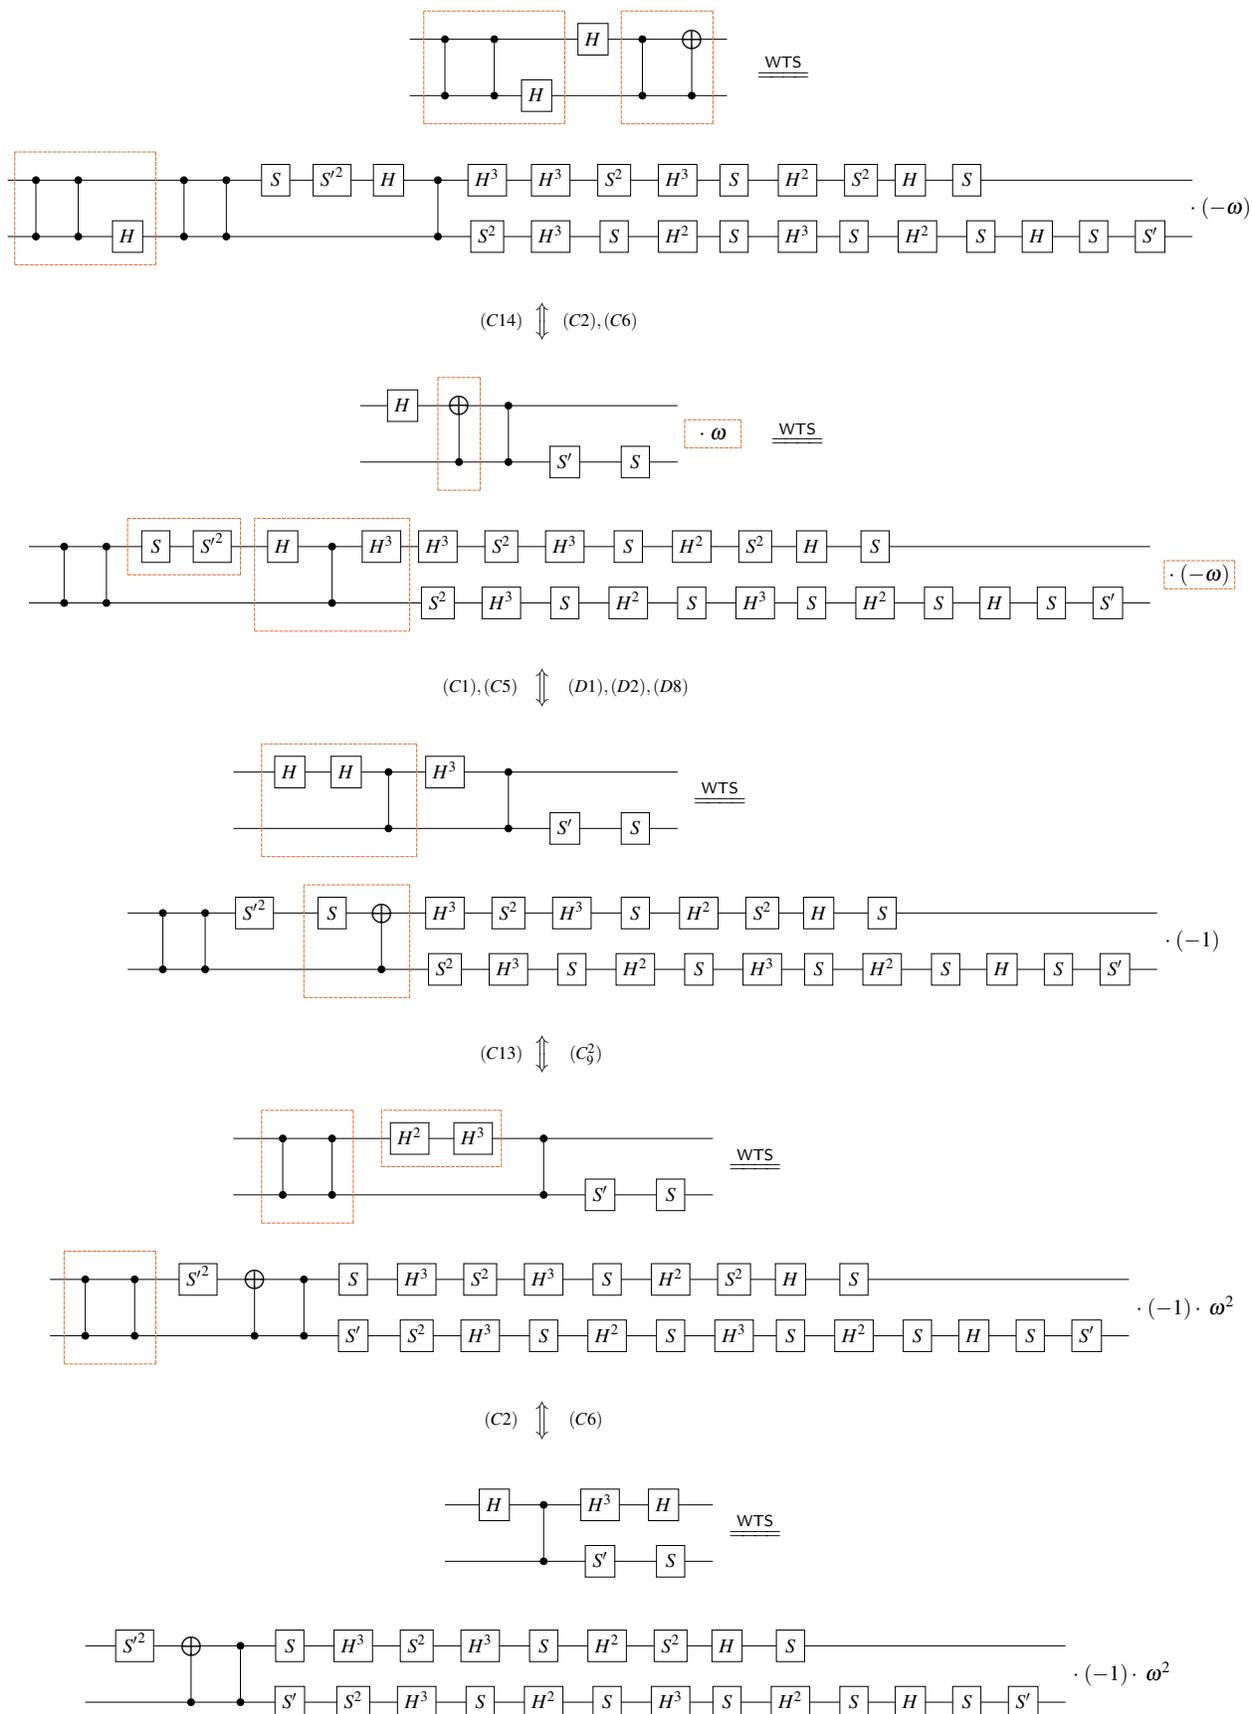

(34)

**Proposition 3.26.** *Up to the single-qutrit Clifford completeness, the equations in Figures 57 and 58 imply all equations in Section 1.2.*

*Proof.* By Lemmas 3.2 to 3.4, 3.6, 3.9 to 3.16, 3.18, 3.20, 3.22, 3.24 and 3.25 and corollaries 3.5, 3.8, 3.17, 3.19, 3.21 and 3.23, we complete the proof.  $\square$

### 3.2 Reduce the Two-Qutrit Box Relations

**Lemma 3.27.** *All the box relations in Appendix C.3 of [1] follow from the equations in Figures 54 and 58 as well as Sections 1.1 and 1.2, with the derived generators in Figures 53 and 57.*

*Proof.* Details are in the GitHub repository: QutritClifford/Two-Qutrit/Box2Derived<sup>2</sup>. □

**Theorem 3.1.** *Up to the single-qutrit Clifford completeness, any true equality between two-qutrit Clifford circuits is provable using the rules in Figure 58 with the derived generators in Figure 57.*

*Proof.* By Proposition 4.3 in [1], the box relations in Appendices C.1 to C.3 are complete for the two-qutrit Clifford group. By Lemma 3.27, the equations in Figures 54 and 58 as well as Sections 1.1 and 1.2 with the derived generators in Figures 53 and 57 suffice to prove all box relations in Appendix C.3. By Proposition 3.26, the equations in Section 1.2 follow from the equations in Figures 57 and 58. This implies that up to the single-qutrit Clifford completeness, we can prove any true equality between two-qutrit Clifford circuits using the rules in Figure 58 with the derived generators in Figure 57. □

## 4 Three-Qutrit Clifford Completeness

Finally, we show that by adding the equations from Figure 60 to Figures 54 and 58, we obtain a complete set of rewrite rules for all 3-qutrit Clifford Circuits. According to the arguments in [1], this establishes the completeness of multi-qutrit Clifford circuits in terms of the generators  $-\omega$ ,  $H$ ,  $S$ , and  $CZ$ , as well as the relations in Figure 1.

In Section 4.1, we show that the derived relations in Section 1.3 follow from the reduced relations in Figure 60, the derived generators in Figure 59, as well as the single- and two-qutrit Clifford completeness established in Sections 2 and 3. In Section 4.2, we show that the 171 three-qutrit box relations follow from the equations in Figures 2 and 60, as well as the derived relations in Section 1.

Together, we prove the three-qutrit Clifford completeness, as stated below. Its proof will be presented at the end of this section.

**Theorem 4.1.** *Up to the single- and two-qutrit Clifford completeness, any true equality between three-qutrit Clifford circuits is provable using the rules in Figure 60 with the derived generators in Figure 59.*

In Section 1.2, the entangling gates in each relation only act on adjacent qutrits. Next, we show how to generalize these relations to three-qutrit relations, where the entangling gates act on non-adjacent qutrits.

---

<sup>2</sup><https://github.com/SarahMMMLi/QutritClifford/tree/main/Two-Qutrit/Box2Derived>

(D9)

(D10)

(D11)

Figure 59: The three-qutrit derived generators from [Figure 2](#).

(C15)

(C16)

(C17)

(C18)

Figure 60: The three-qutrit reduced relations from [Figure 1](#).

**Definition 4.2.** Let  $U \in \mathcal{C}_2$ . Then  $U^* \in \mathcal{C}_3$  and

(35)

**Proposition 4.3.** Let  $U, V, W, T \in \mathcal{C}_2$ . Then the two-qutrit relation  $R$  implies the three-qutrit relation  $R^*$ .

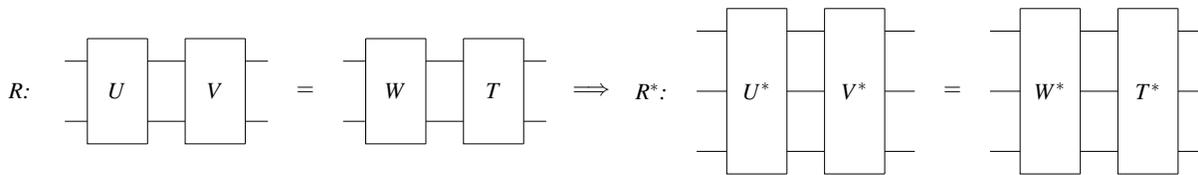

*Proof.*

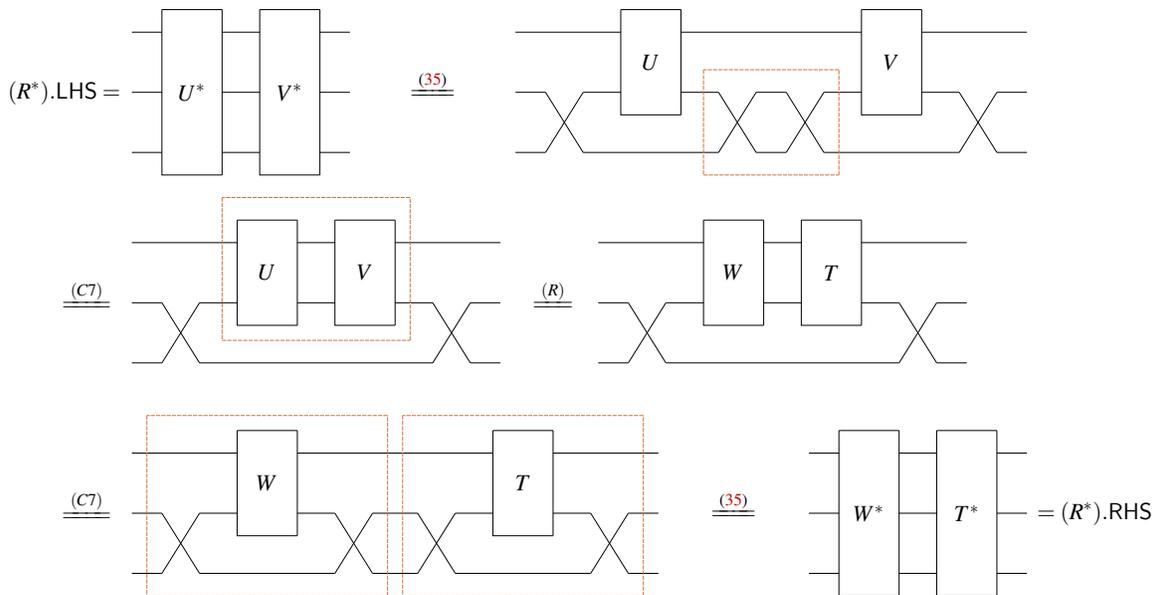

□

**Lemma 4.4.** The equations in [Figure 29](#) follow from the reduced relations.

*Proof.* By symmetry, it suffices to prove that (COMMUTE) follows from the equations in [Figures 1 and 2](#).

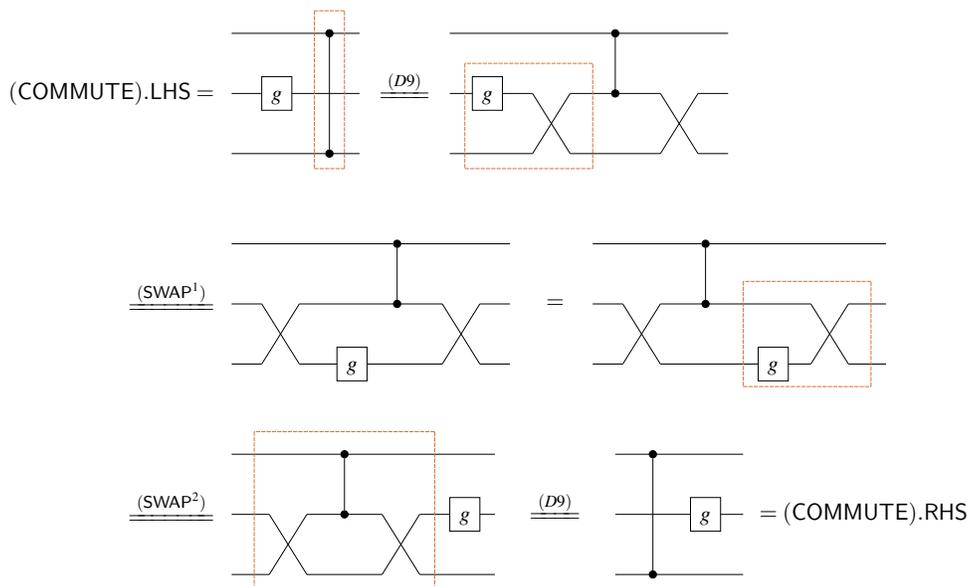

□

### 4.1 Reduce the Three-Qutrit Derived Relations

**Lemma 4.5.** *The equations in Figure 30 follow from the reduced relations.*

*Proof.* We derive all equations in Figure 30 in order.

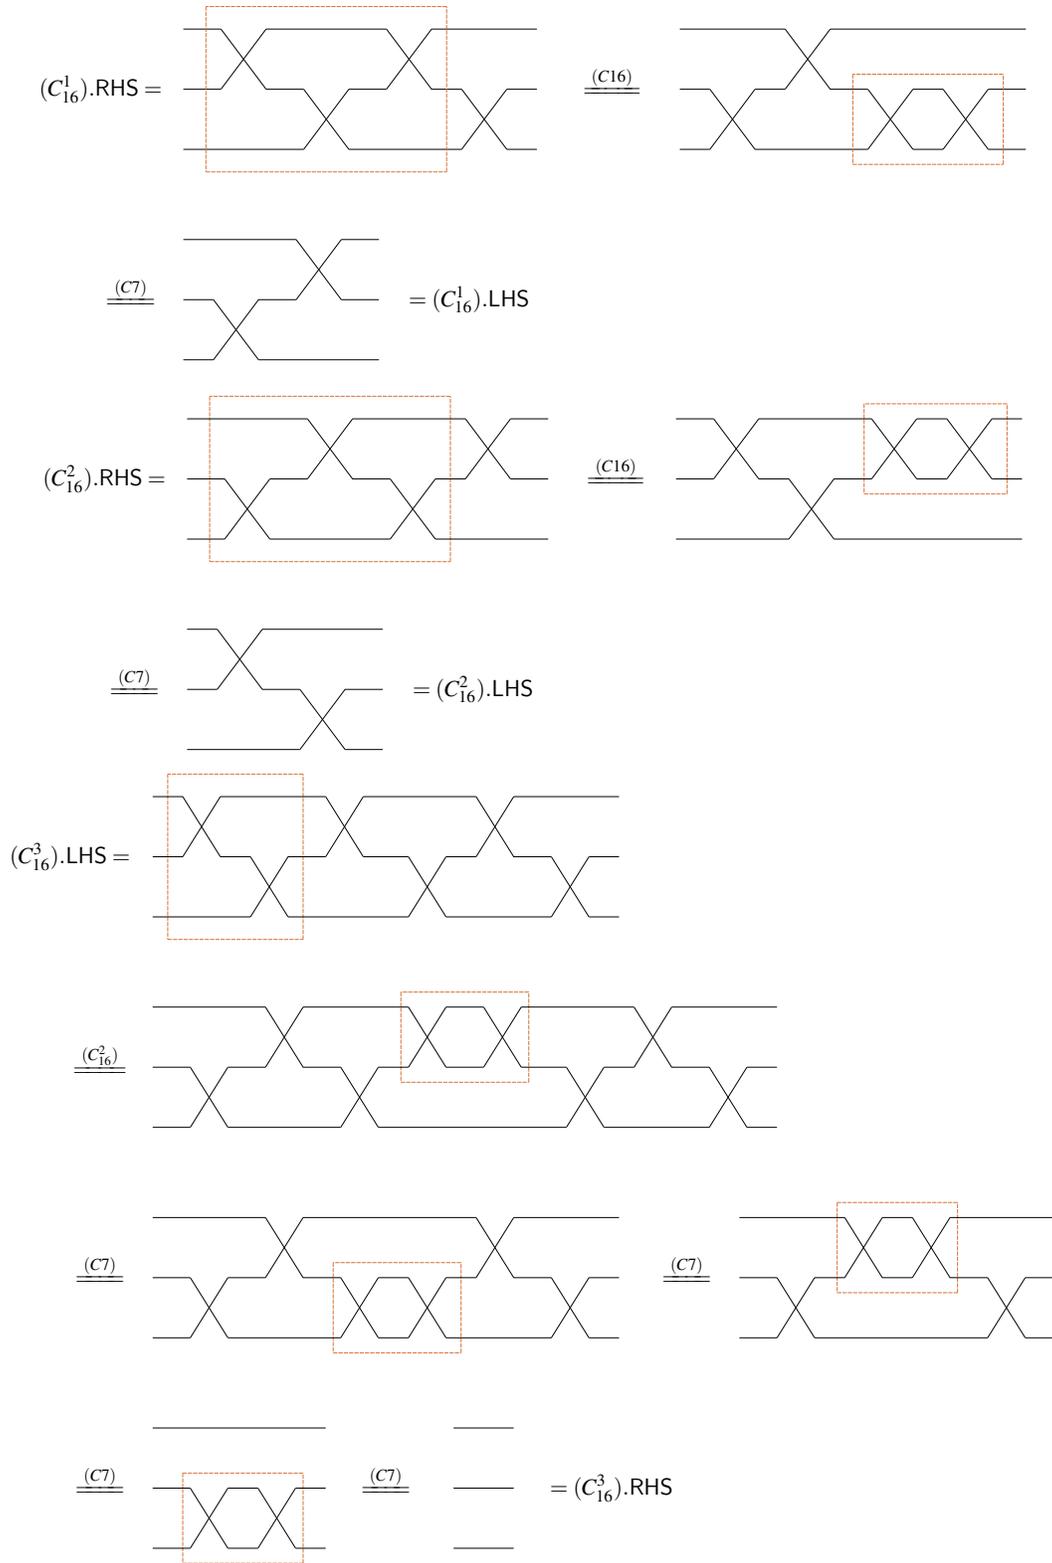

□

**Lemma 4.6.** *The equations in Figure 31 follow from the reduced relations.*

*Proof.* We derive all equations in Figure 31 in order.

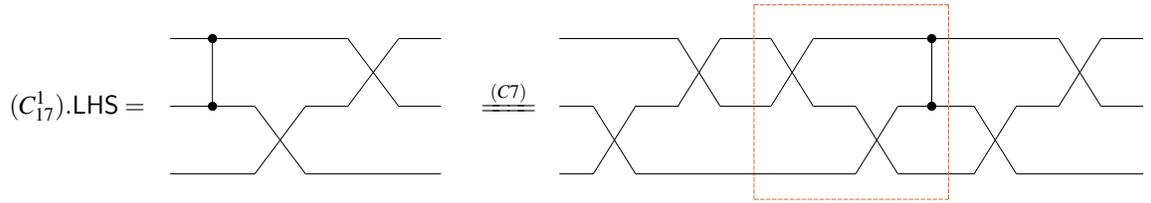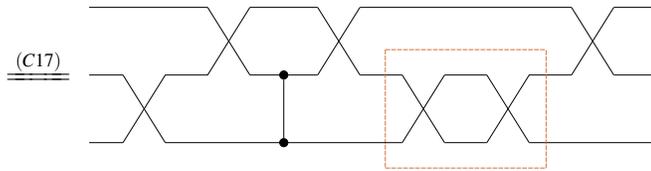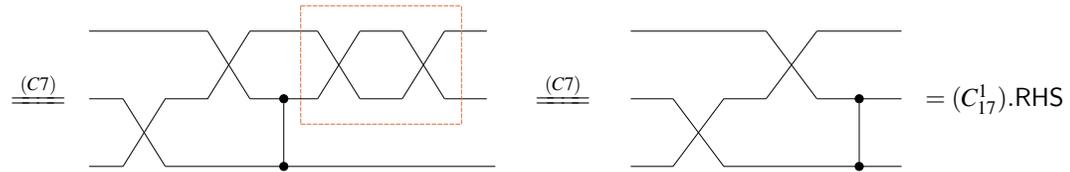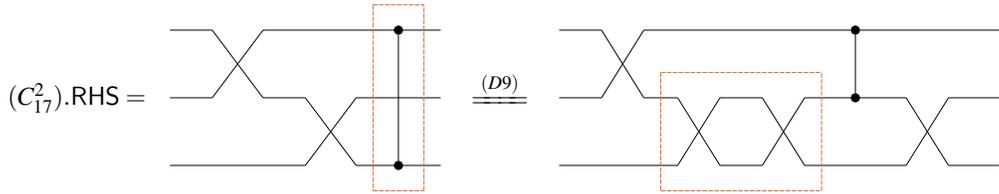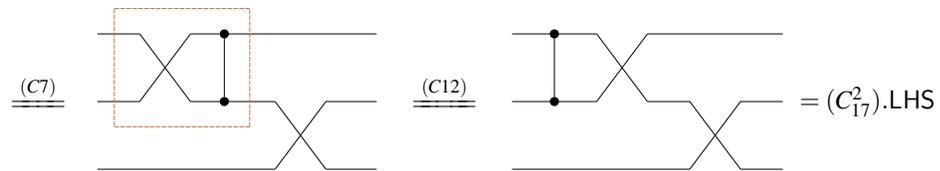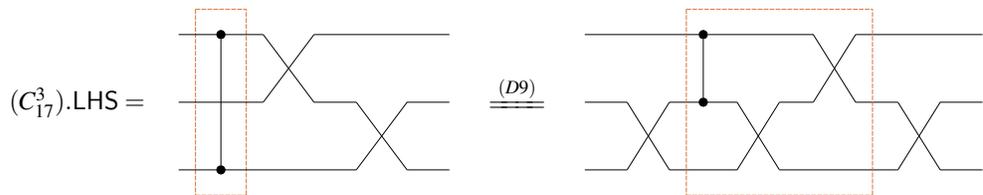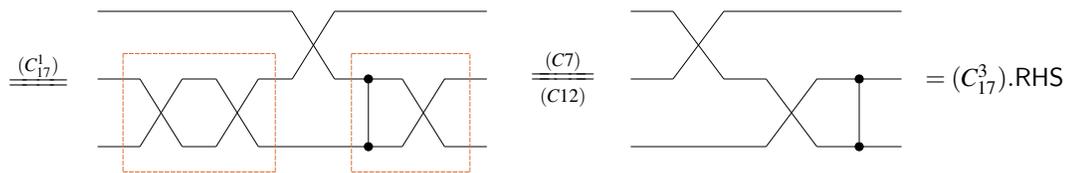

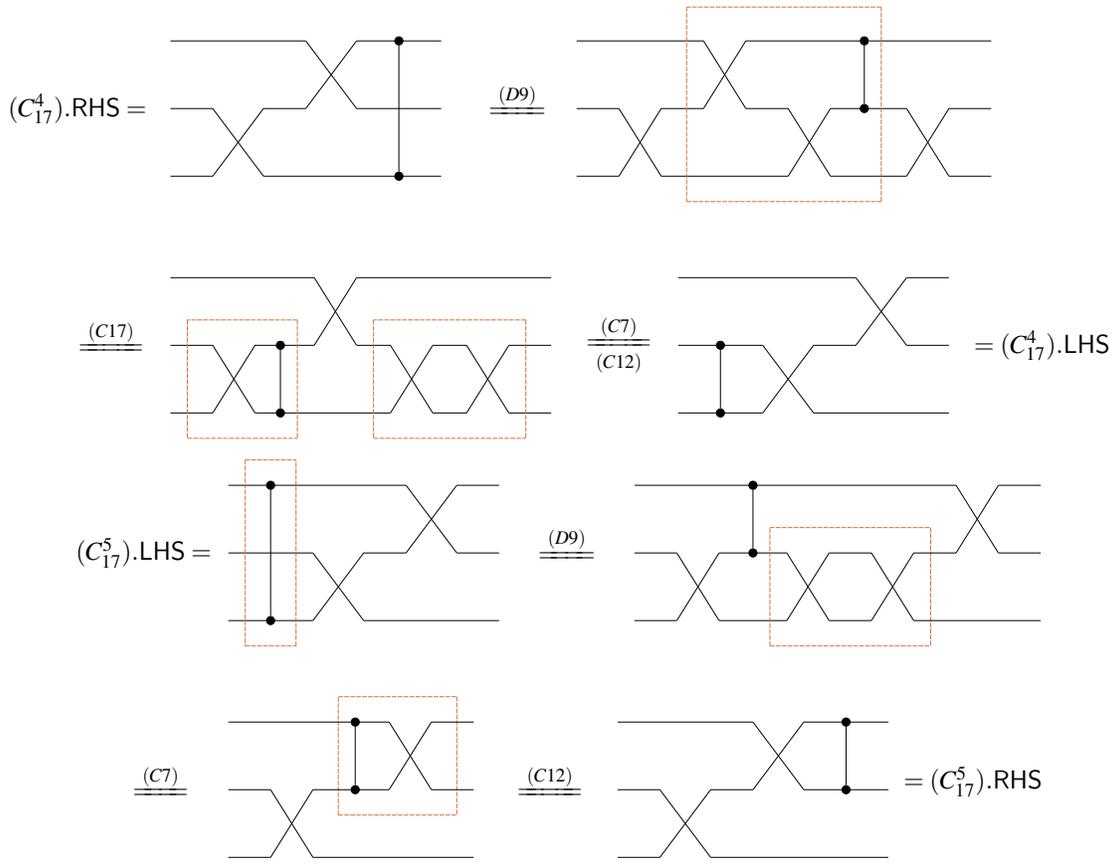

□

**Lemma 4.7.** *The equations in Figure 32 follow from the reduced relations.*

*Proof.* By symmetry, it suffices to prove that  $(C_{17}^6)$  and  $(C_{17}^8)$  follow from the equations in Figures 1 and 2.

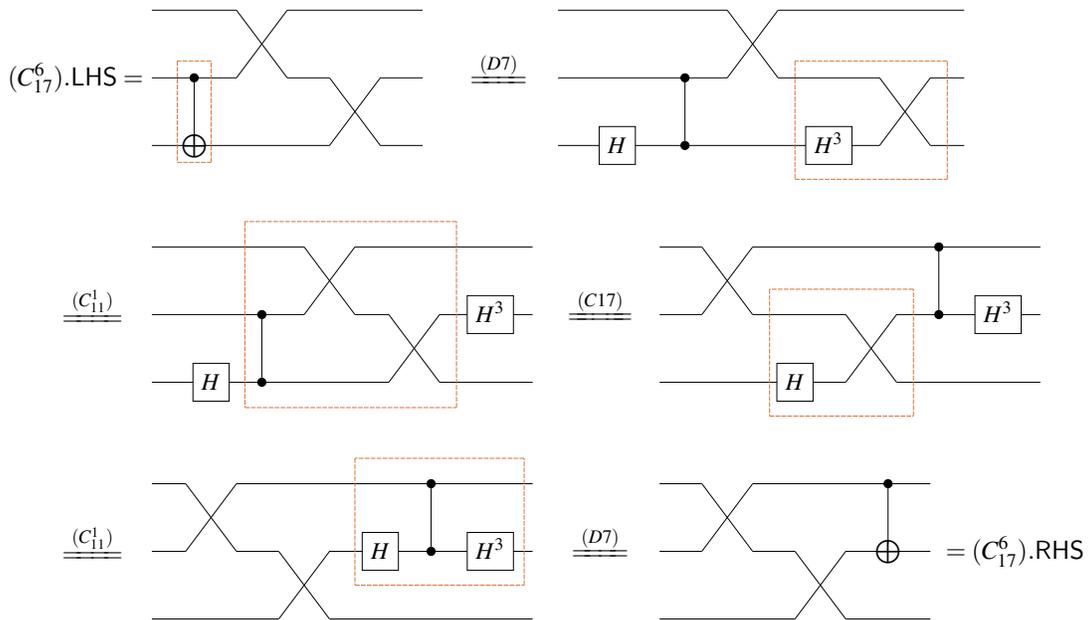

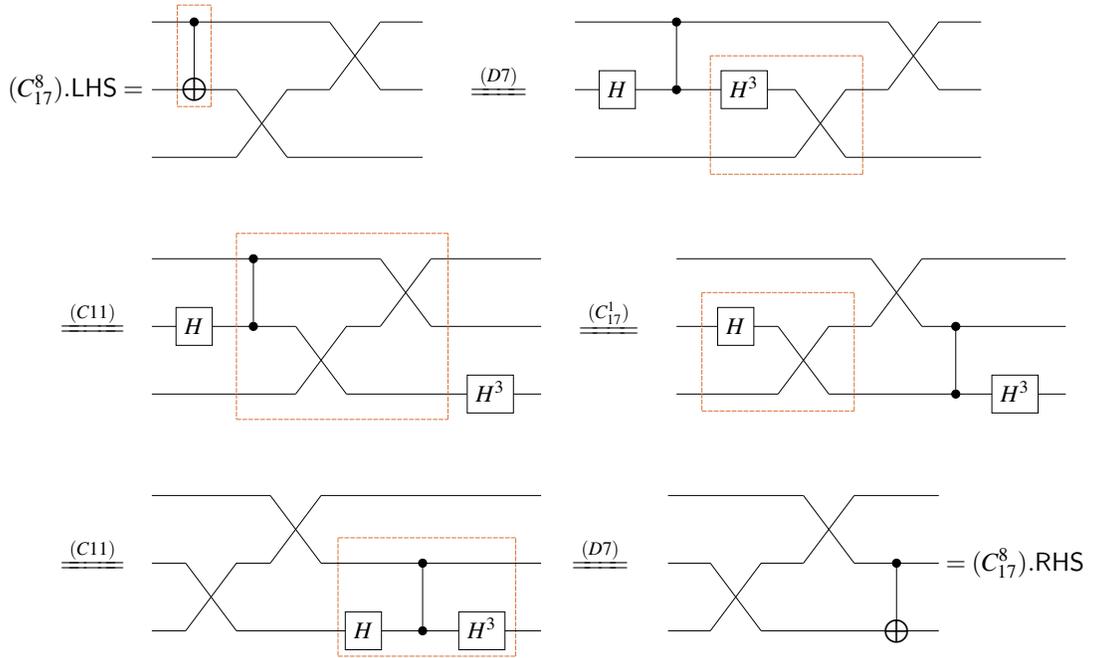

□

**Lemma 4.8.** *The equations in Figure 33 follow from the reduced relations.*

*Proof.*

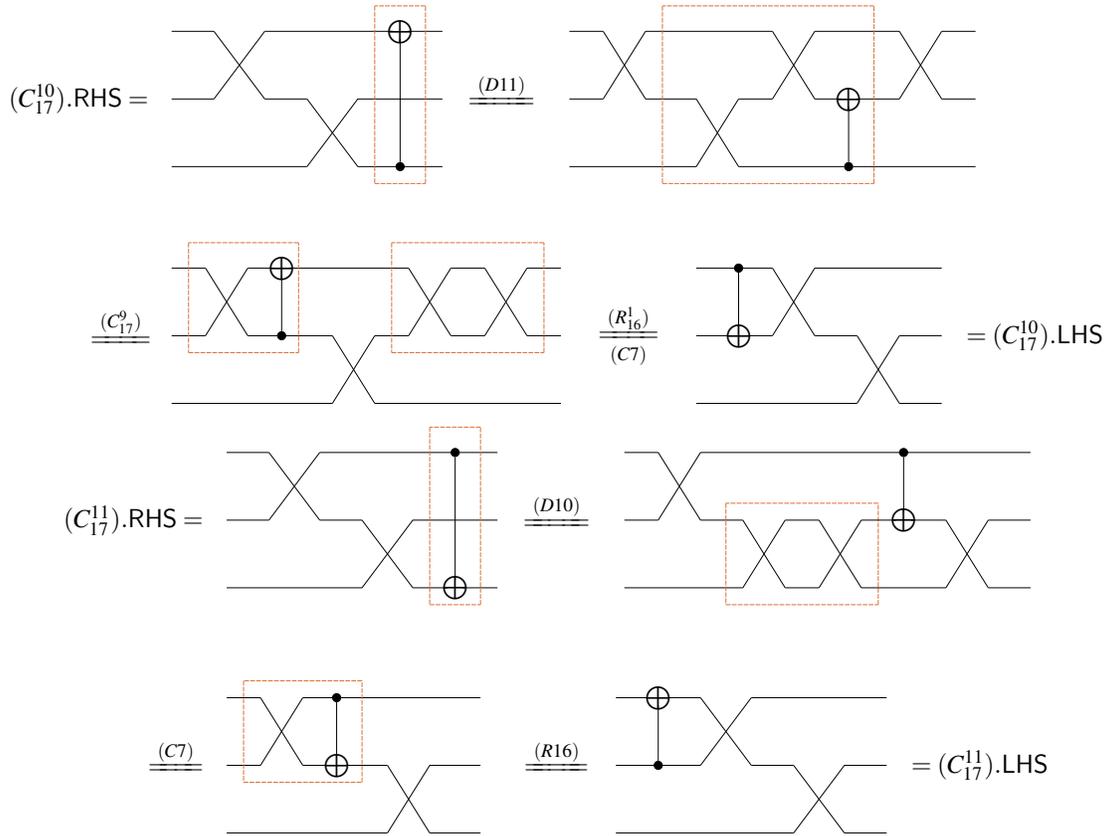

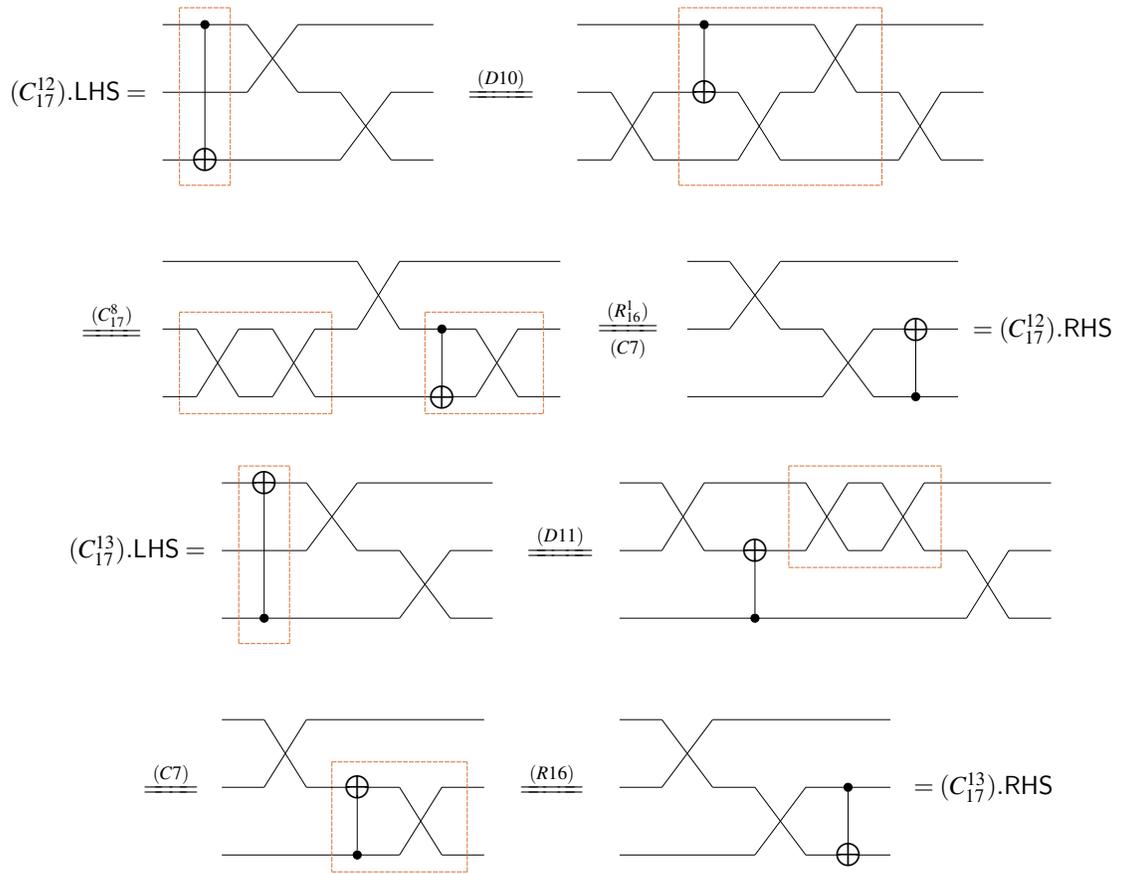

□

**Corollary 4.9.** *The equations in Figure 34 follow from the reduced relations.*

**Lemma 4.10.** *The equations in Figure 35 follow from the reduced relations.*

*Proof.* It suffices to derive  $(C_{17}^{18})$ ,  $(C_{17}^{19})$ ,  $(C_{17}^{20})$ , and  $(C_{17}^{21})$  from the reduced relations, as the derivation of the other equations in Figure 35 follows analogously.

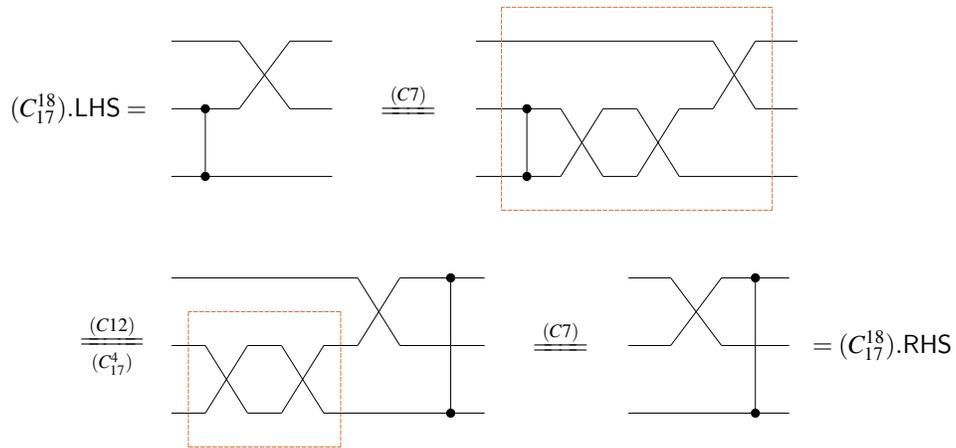

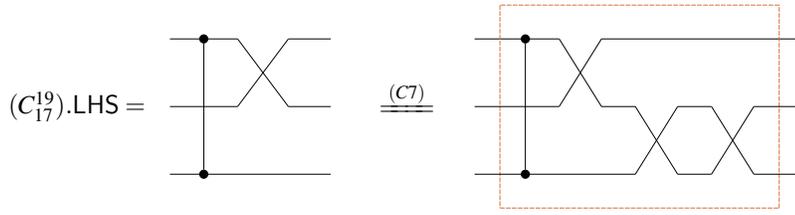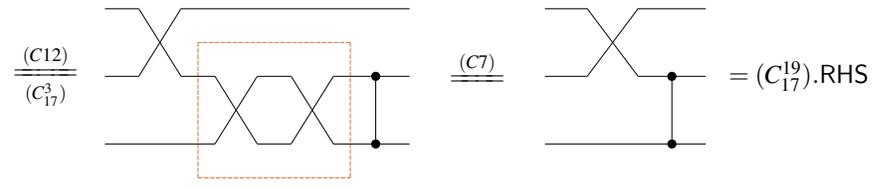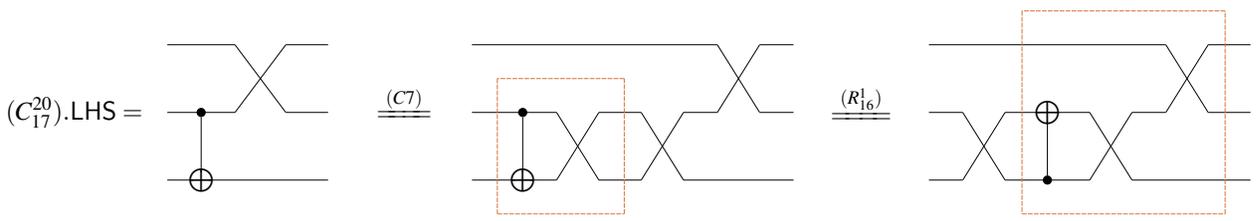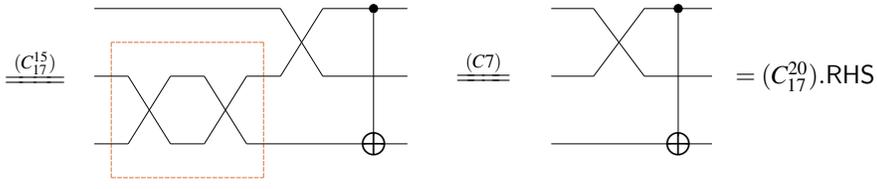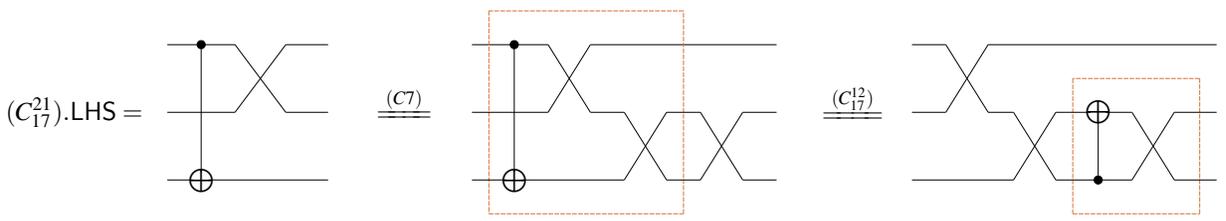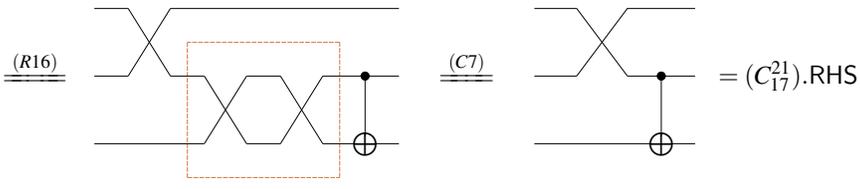

□

**Lemma 4.11.** *The equations in Figure 36 follow from the reduced relations.*

*Proof.* It suffices to derive (rCX) from (D10) and the other reduced relations, as the derivation of (rXC) follows analogously.

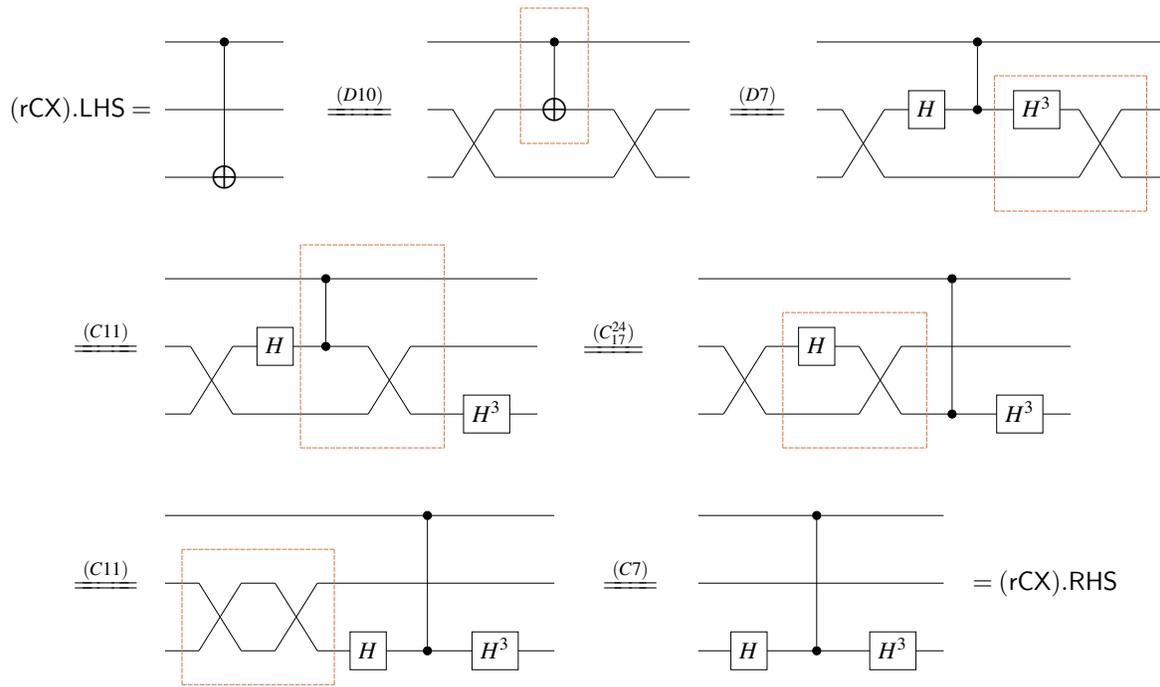

□

**Lemma 4.12.** *The equations in Figure 37 follow from the reduced relations.*

*Proof.* We derive (C<sub>15</sub><sup>1</sup>) and (C<sub>15</sub><sup>2</sup>) in order. By symmetry, it suffices to prove that (C<sub>15</sub><sup>3</sup>), (C<sub>15</sub><sup>5</sup>), (C<sub>15</sub><sup>7</sup>), (C<sub>15</sub><sup>9</sup>), and (C<sub>15</sub><sup>10</sup>) follow from the equations in Figures 1 and 2.

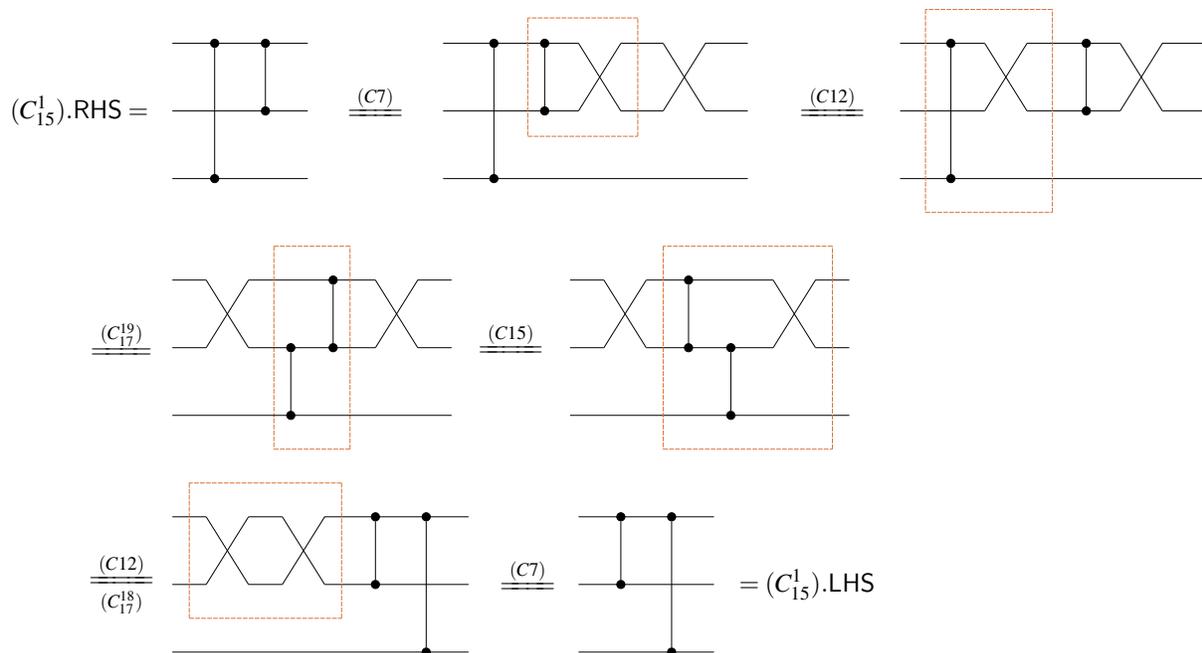

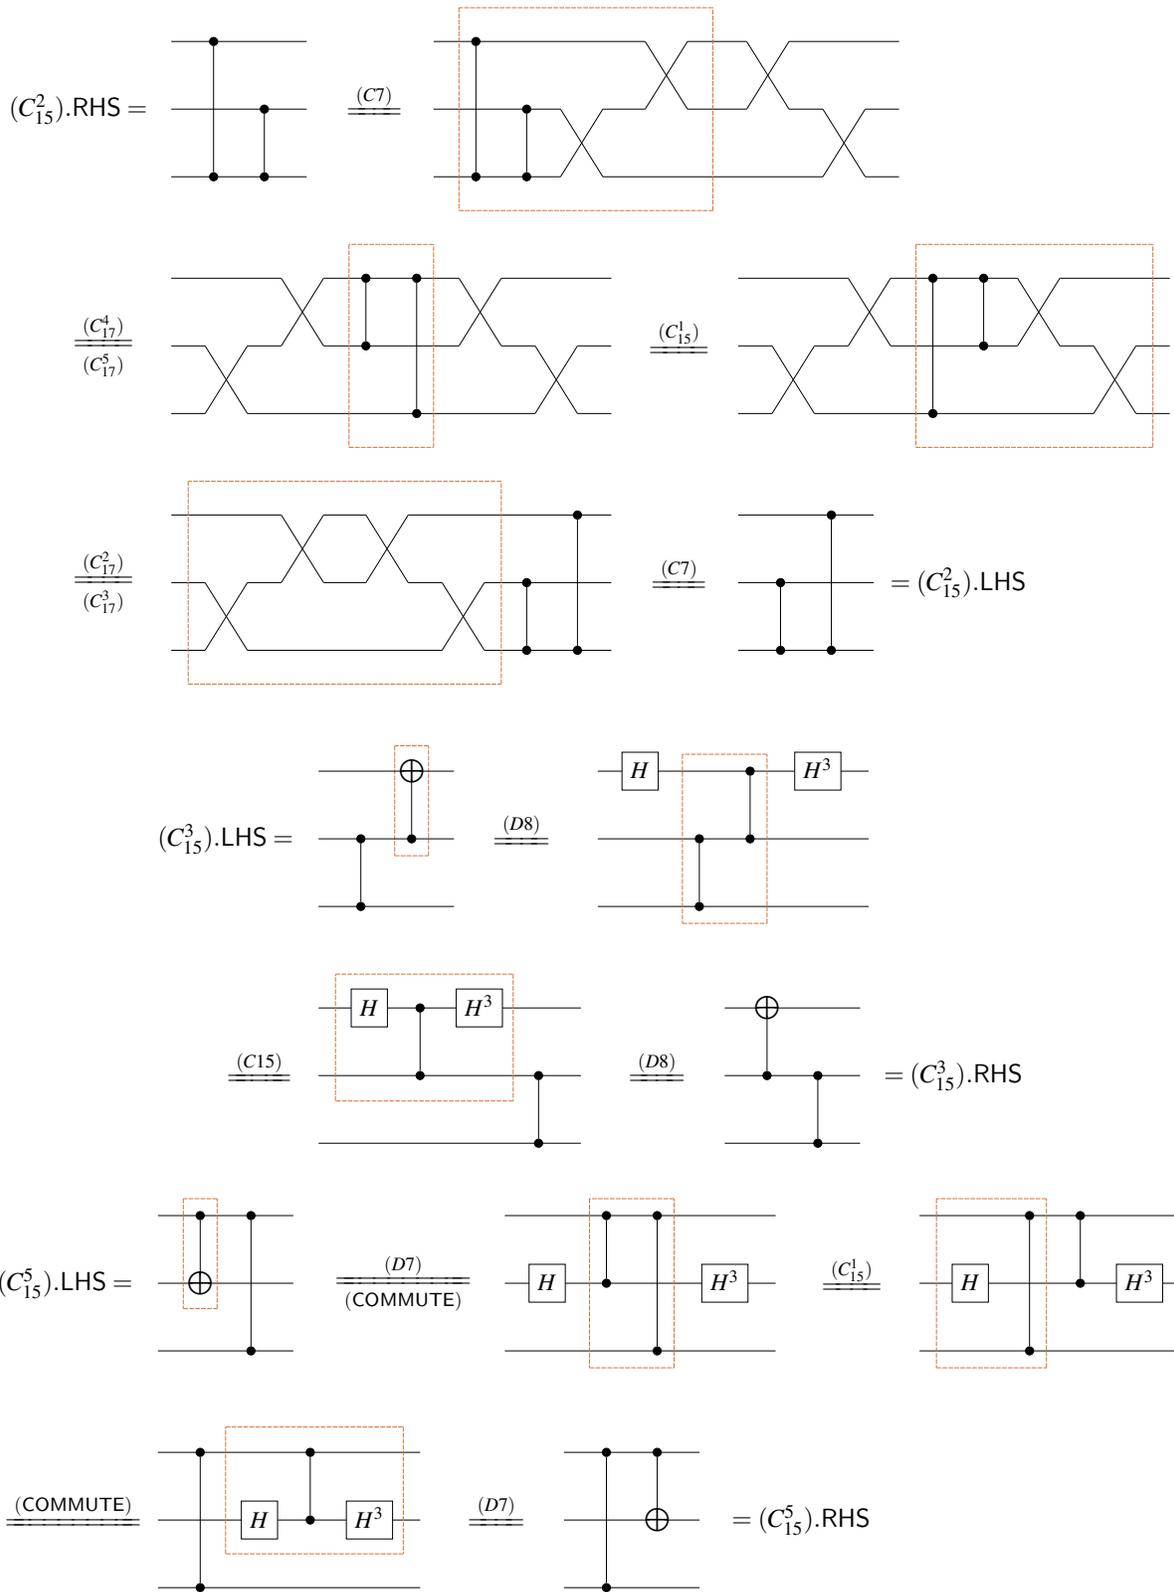

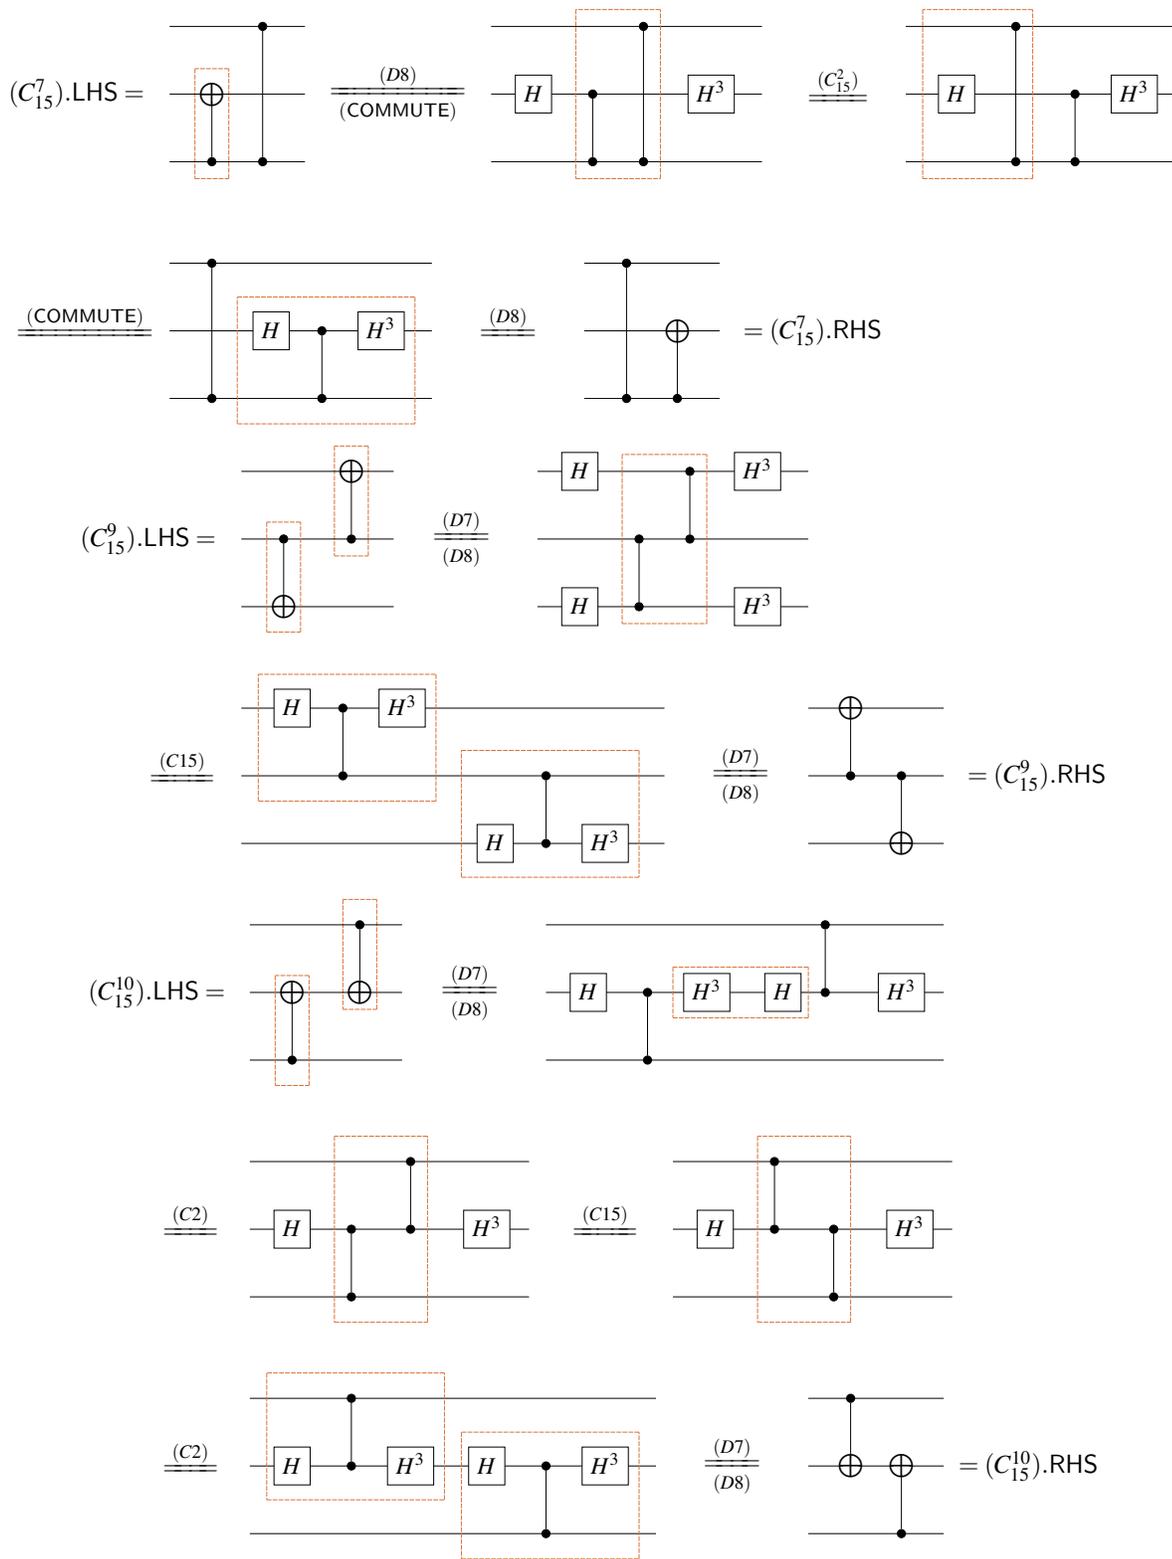

□

**Lemma 4.13.** *The equations in Figure 38 follow from the reduced relations.*

*Proof.* Firstly, let us derive  $(C_{18}^1)$ ,  $(C_{18}^2)$ ,  $(C_{18}^3)$ , and  $(C_{18}^4)$  in order.

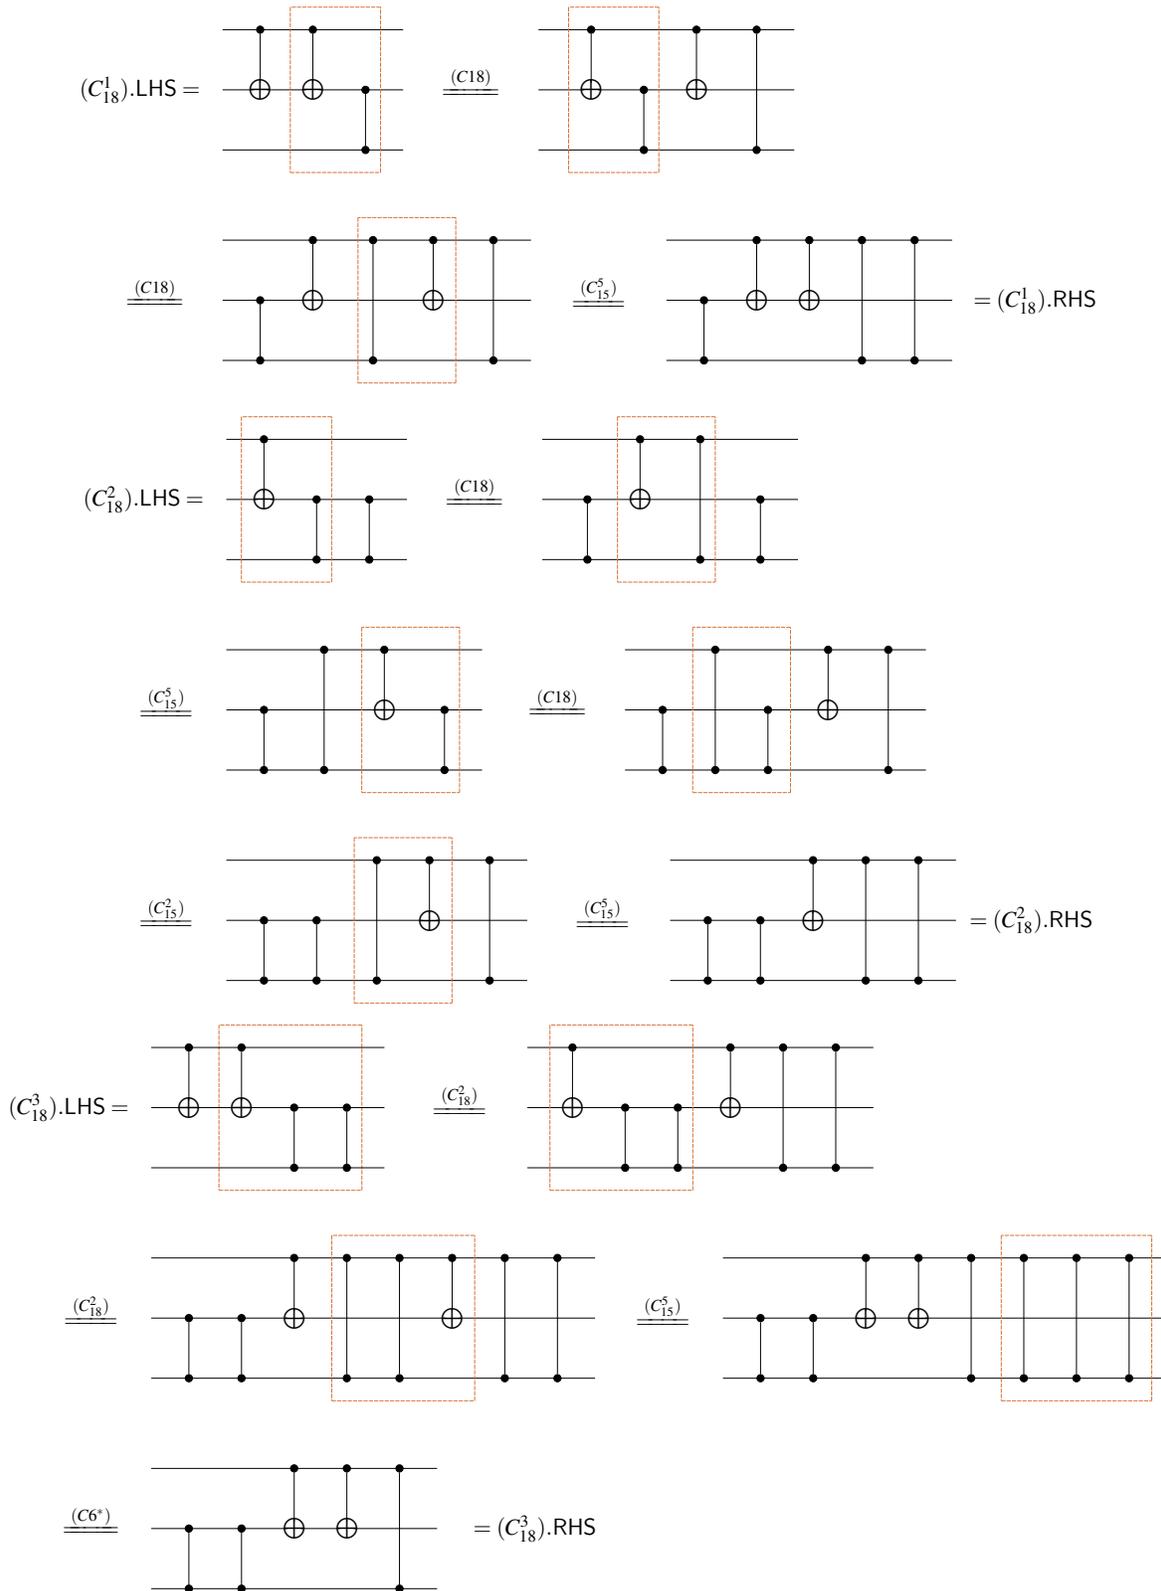

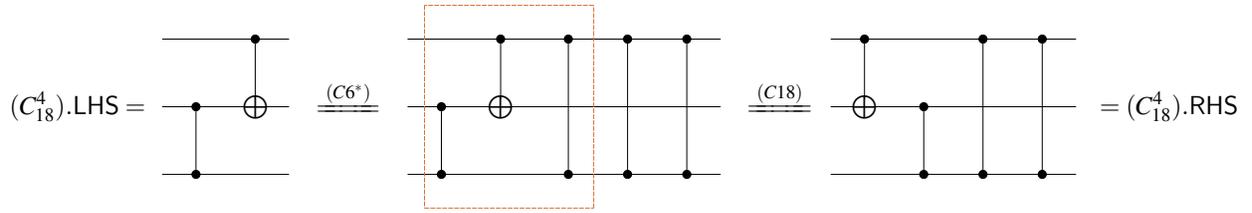

Reasoning analogously as above, we can derive  $(C_{18}^5)$ ,  $(C_{18}^6)$ , and  $(C_{18}^7)$ . Finally, let us derive  $(C_{18}^8)$ .

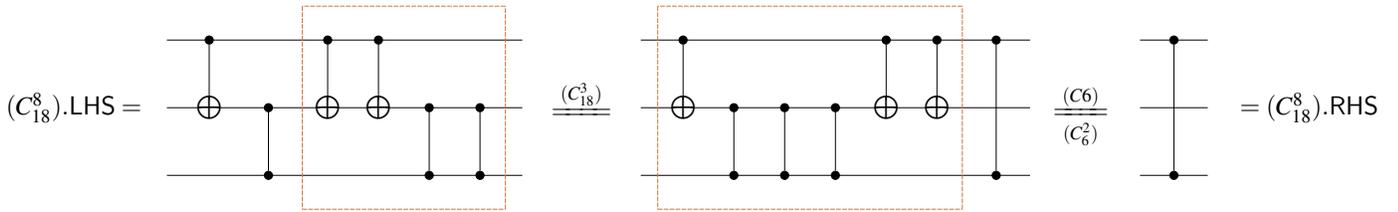

□

**Lemma 4.14.** *The equations in Figure 39 follow from the reduced relations.*

*Proof.* Firstly, let us derive  $(C_{18}^9)$ ,  $(C_{18}^{10})$ ,  $(C_{18}^{11})$ ,  $(C_{18}^{12})$ , and  $(C_{18}^{13})$  in order.

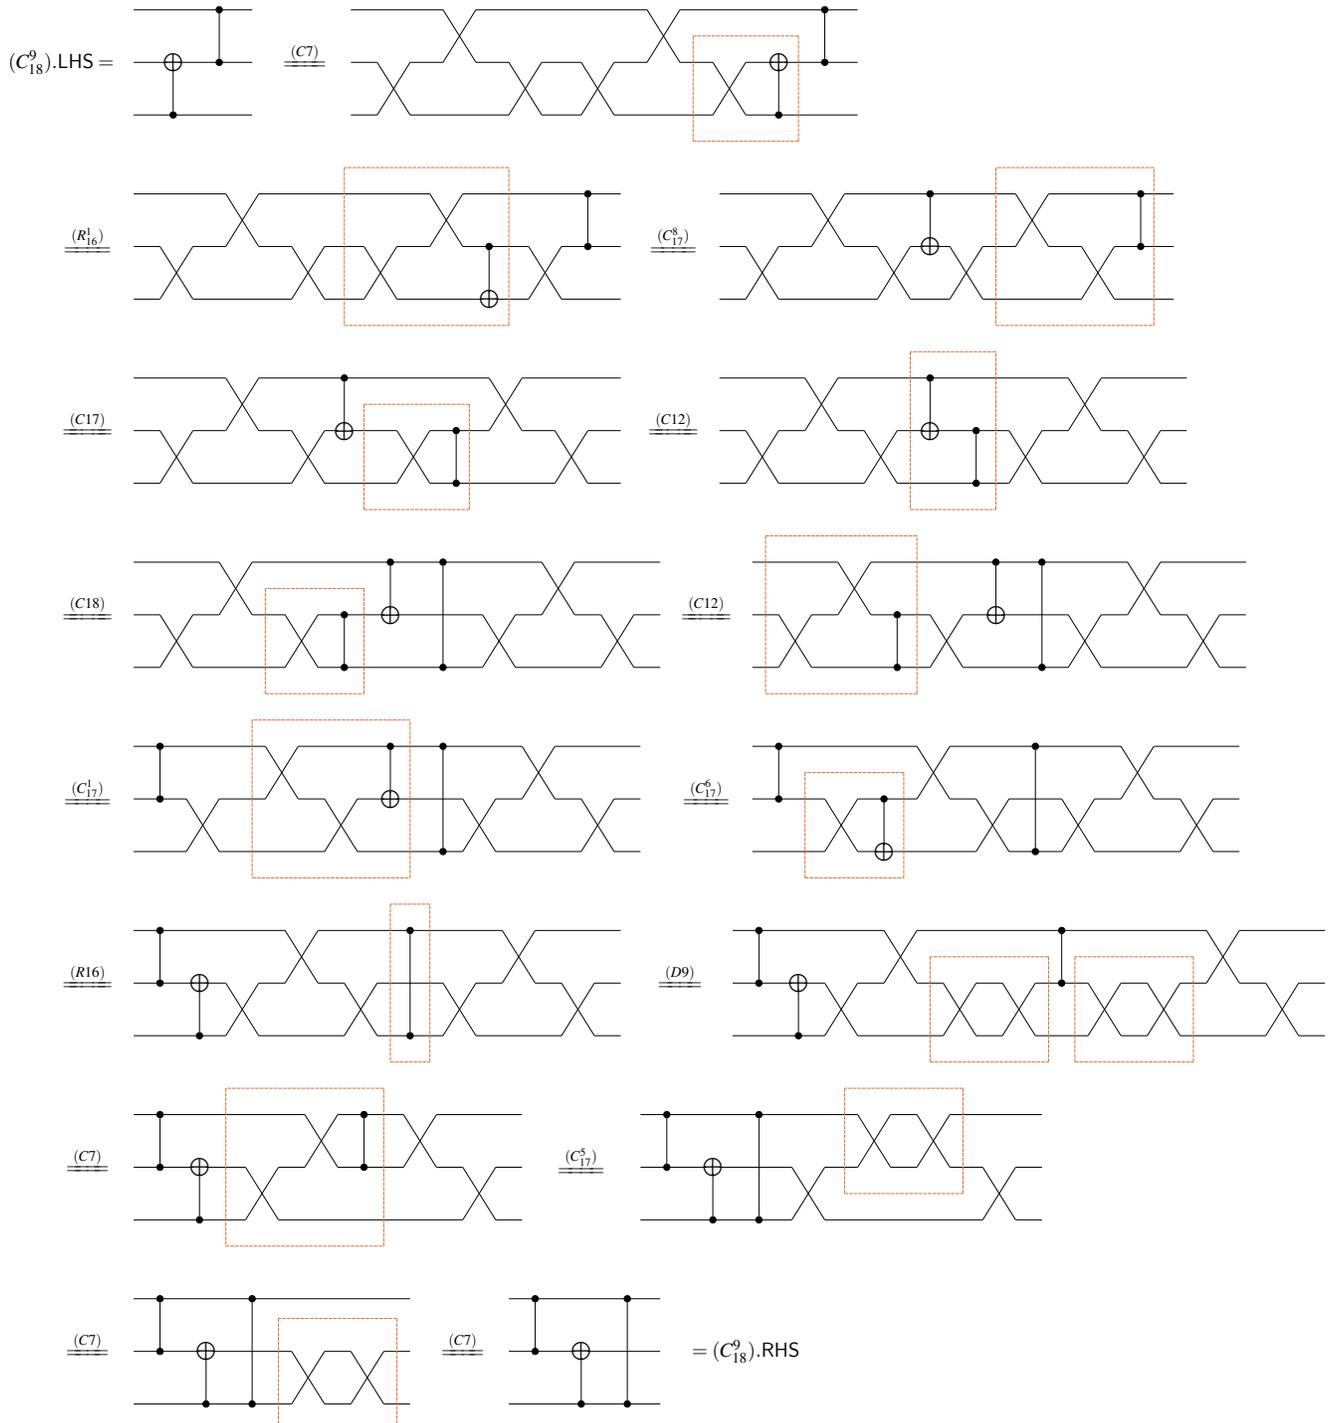



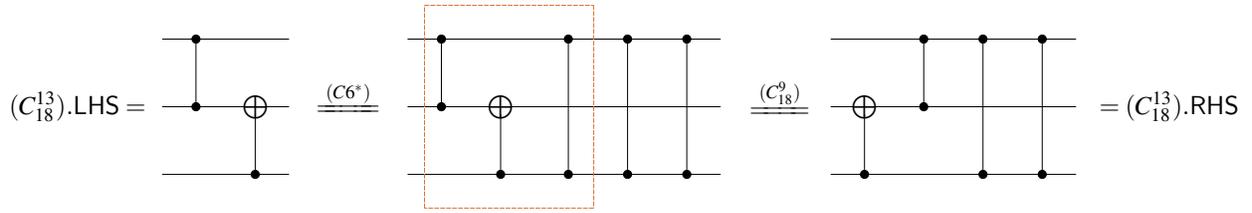

Reasoning analogously as above, we can derive  $(C_{18}^{14})$ ,  $(C_{18}^{15})$ , and  $(C_{18}^{16})$ . Finally, let us derive  $(C_{18}^{17})$ .

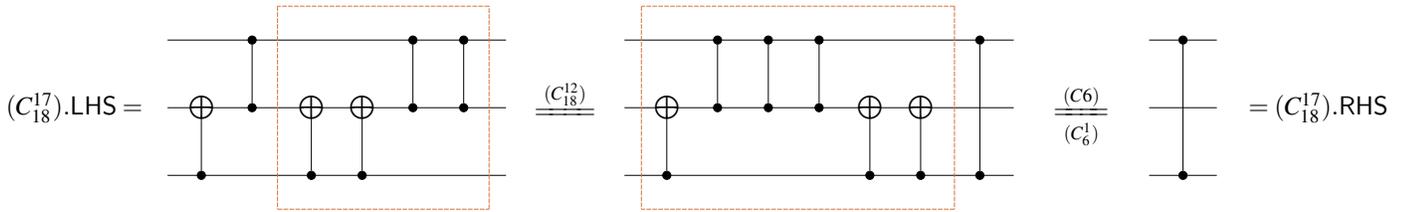

□

**Lemma 4.15.** *The equations in Figure 40 follow from the reduced relations.*

*Proof.* It suffices to derive  $(C_{18}^{18})$  from the equations in Figure 40 and other reduced relations, as other derivations follow analogously.

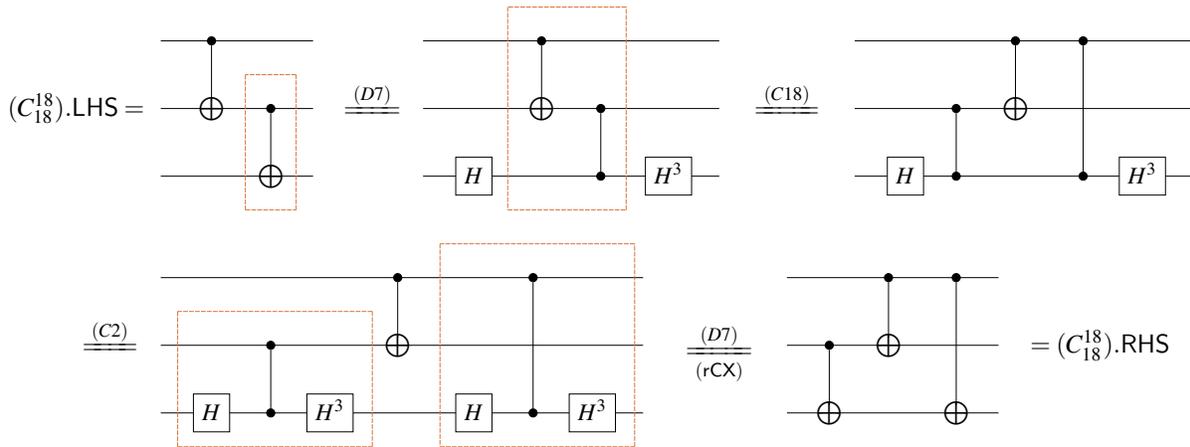

□

**Corollary 4.16.** *The equations in Figure 41 follow from the reduced relations.*

**Lemma 4.17.** *The equations in Figure 42 follow from the reduced relations.*

*Proof.*

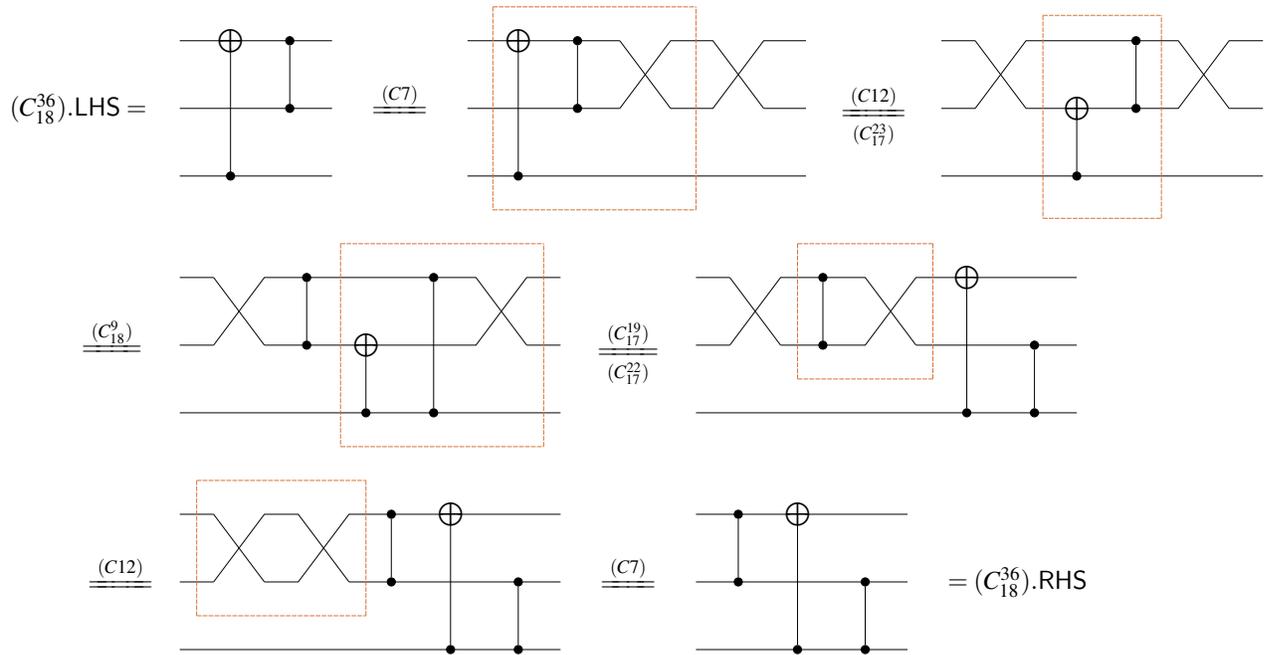

Reasoning analogously as before, we can derive the remaining equations in Figure 42. □

**Lemma 4.18.** *The equations in Figure 43 follow from the reduced relations.*

*Proof.*

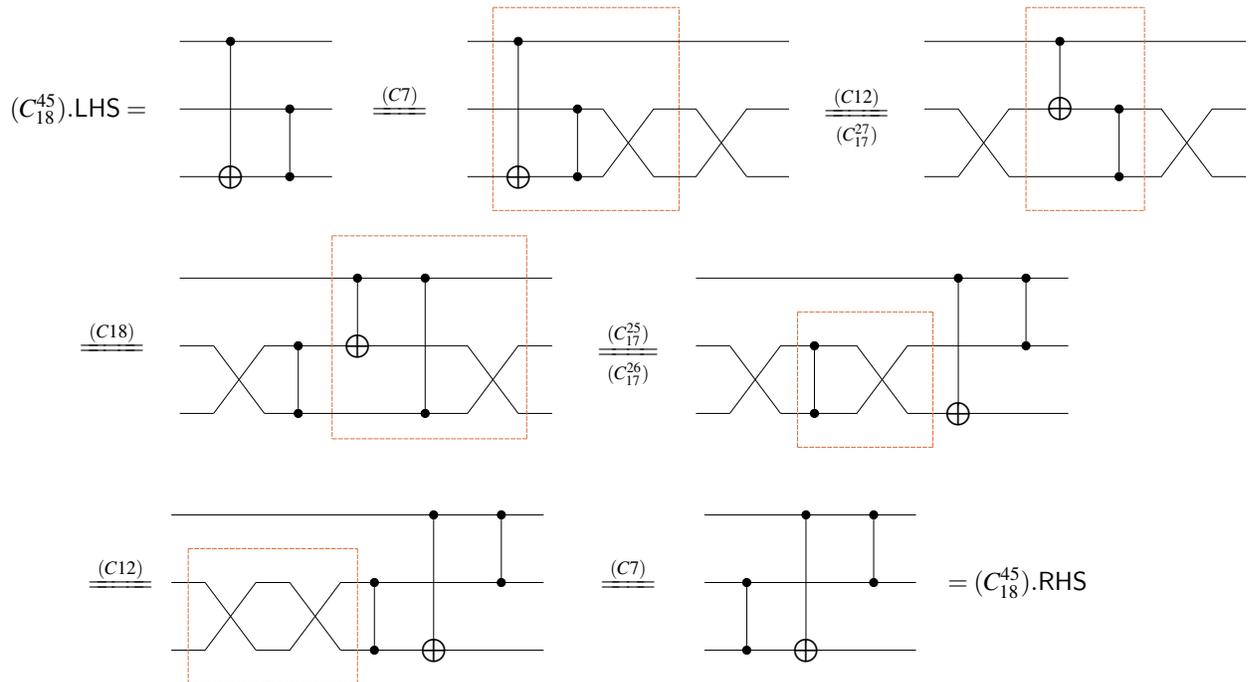

Reasoning analogously as before, we can derive the remaining equations in [Figure 43](#). □

**Corollary 4.19.** *The equations in [Figure 44](#) follow from the reduced relations.*

**Corollary 4.20.** *The equations in [Figure 45](#) follow from the reduced relations.*

**Lemma 4.21.** *The equations in [Figure 46](#) follow from the reduced relations.*

*Proof.*

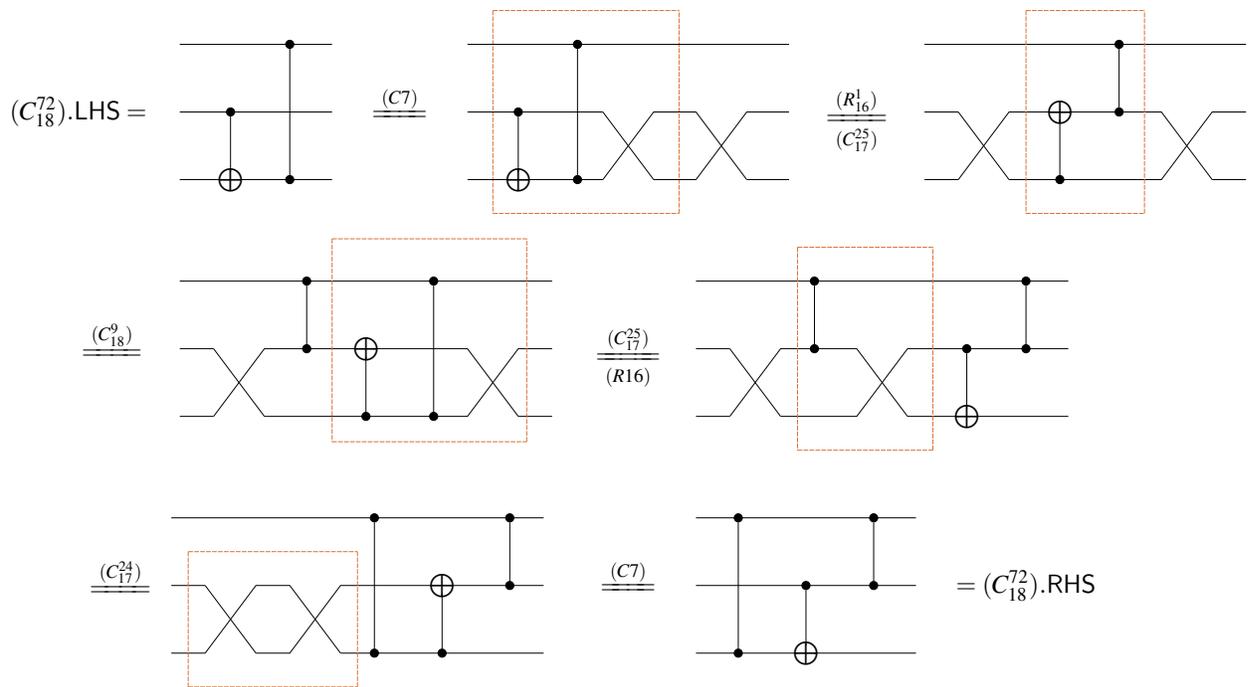

Reasoning analogously as before, we can derive the remaining equations in [Figure 46](#). □

**Lemma 4.22.** *The equations in [Figure 47](#) follow from the reduced relations.*

*Proof.*

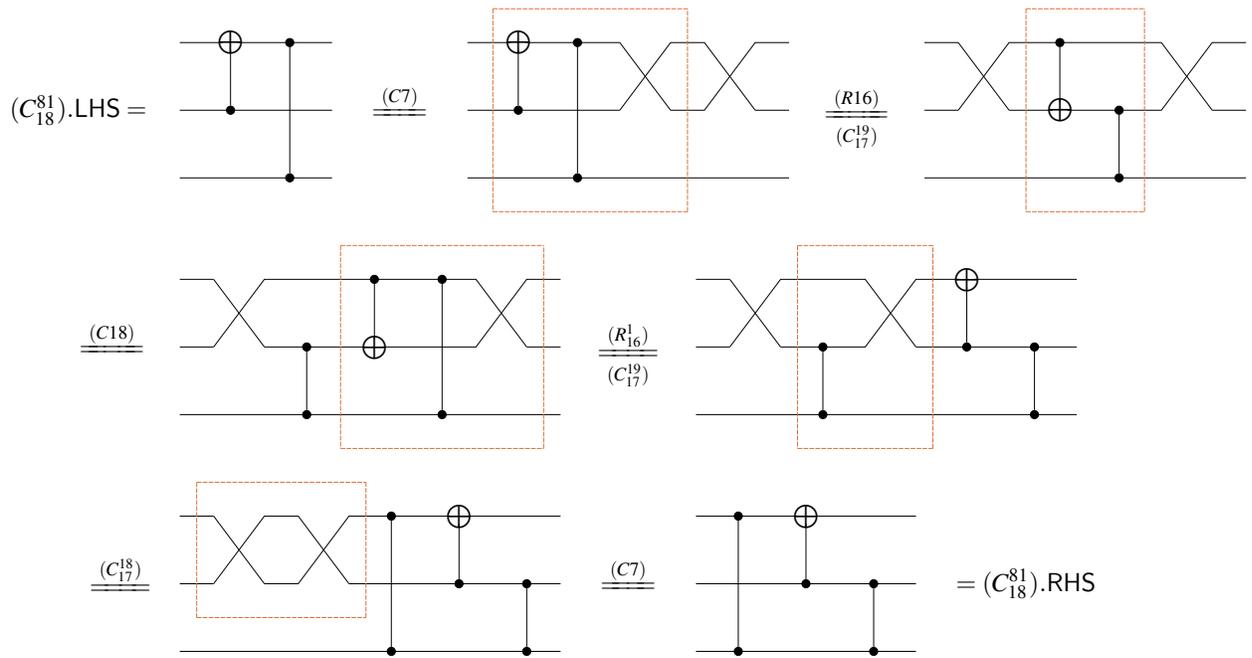

Reasoning analogously as before, we can derive the remaining equations in Figure 47. □

**Corollary 4.23.** *The equations in Figure 48 follow from the reduced relations.*

**Corollary 4.24.** *The equations in Figure 49 follow from the reduced relations.*

In Lemmas 4.25 to 4.36, we show that each equation in Figures 50 to 52 follows from the reduced relations presented in Figure 1 and the derived generators defined in Figure 2.

**Lemma 4.25.** *(R32) and (R33) follow from the reduced relations.*

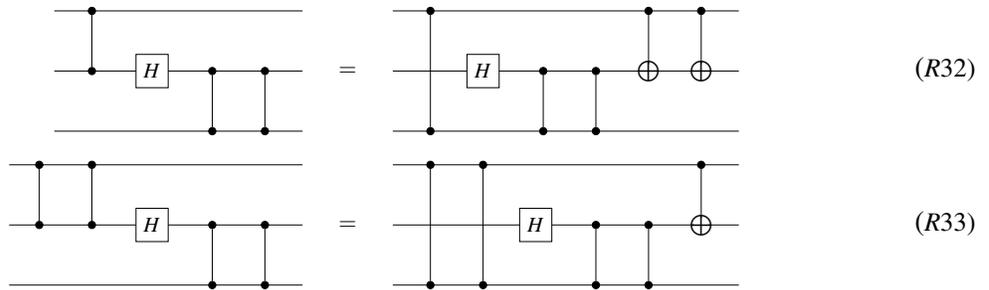

Proof.

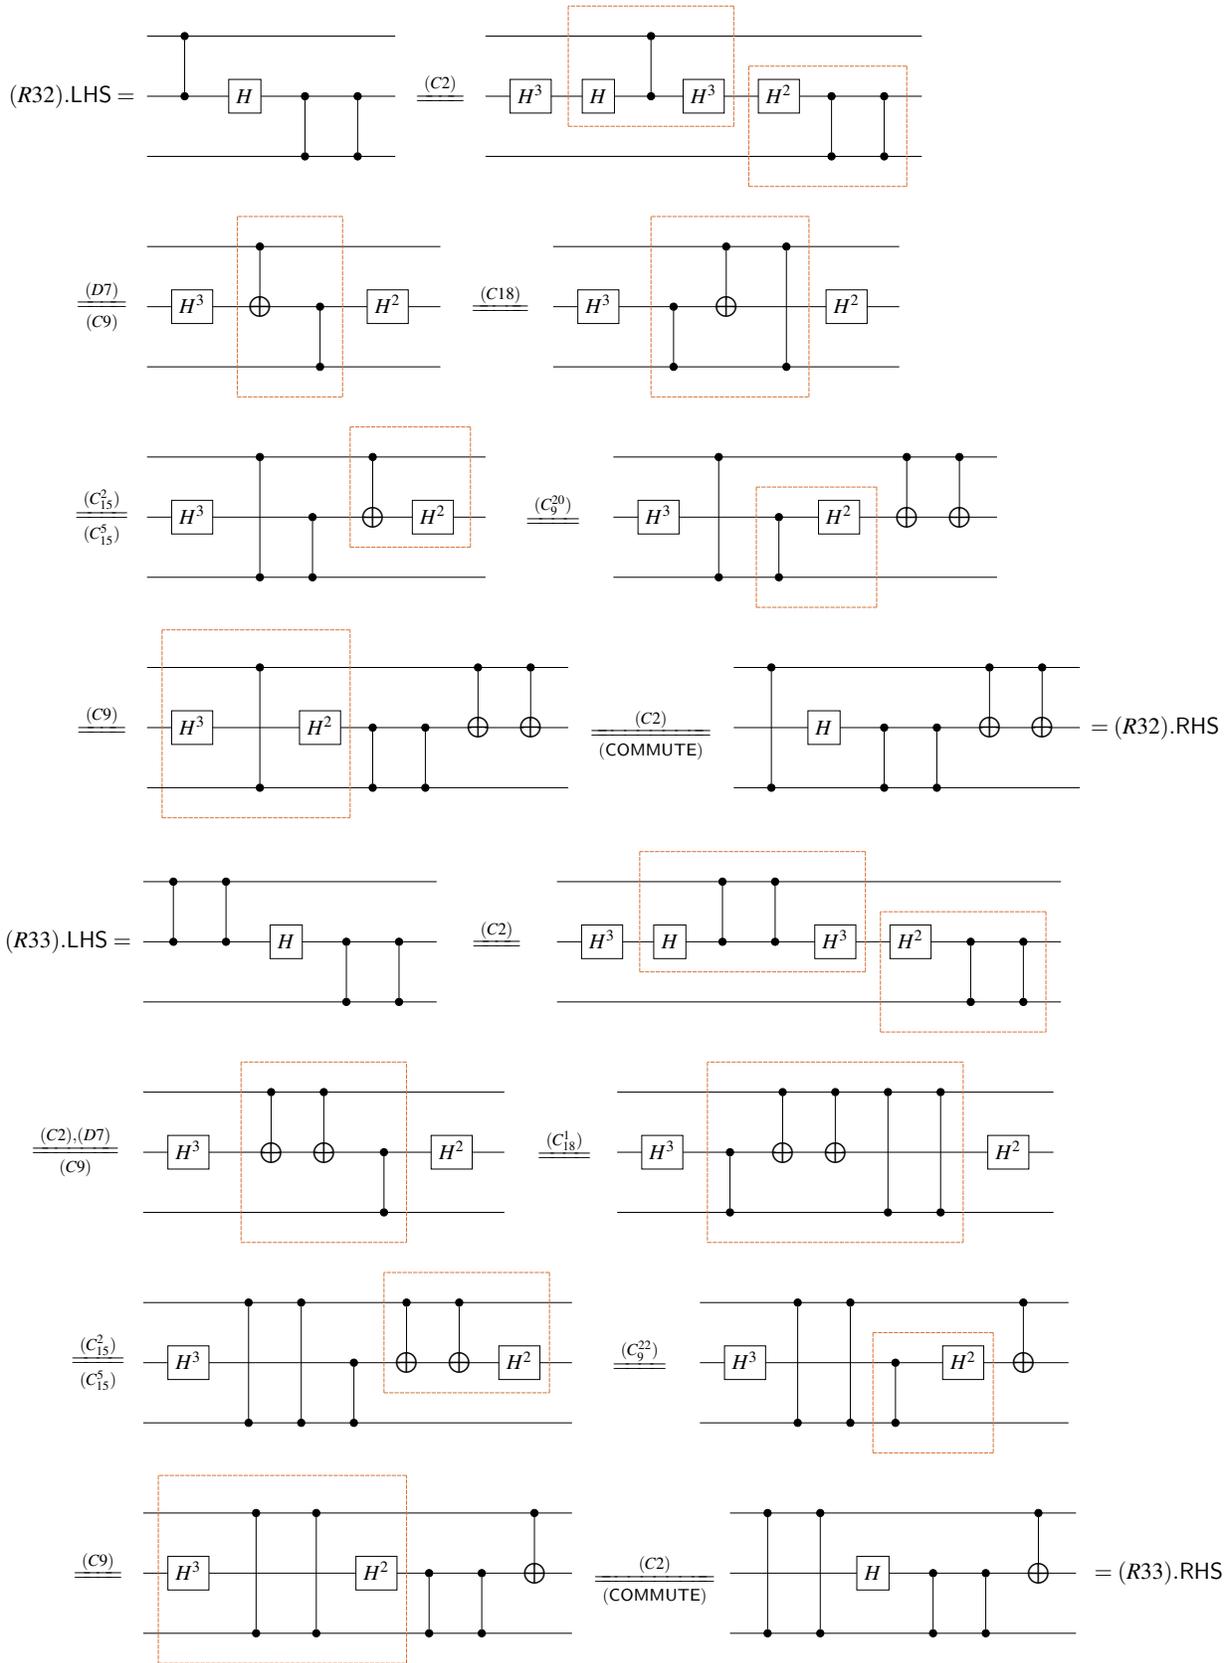

□

**Lemma 4.26.** (R34) and (R35) follow from the reduced relations.

(R34)

(R35)

*Proof.*

(R34).LHS =  $\xrightarrow{(C7)}$   $\xrightarrow{\substack{(C11),(C12) \\ (C17^{19})}}$   $\xrightarrow{(R32)}$   $\xrightarrow{\substack{(COMMUTE) \\ (C15^2)}}$   $\xrightarrow{\substack{(R16^1),(C11^1) \\ (C17^18),(C17^19)}}$   $\xrightarrow{(C7)}$  (R34).RHS

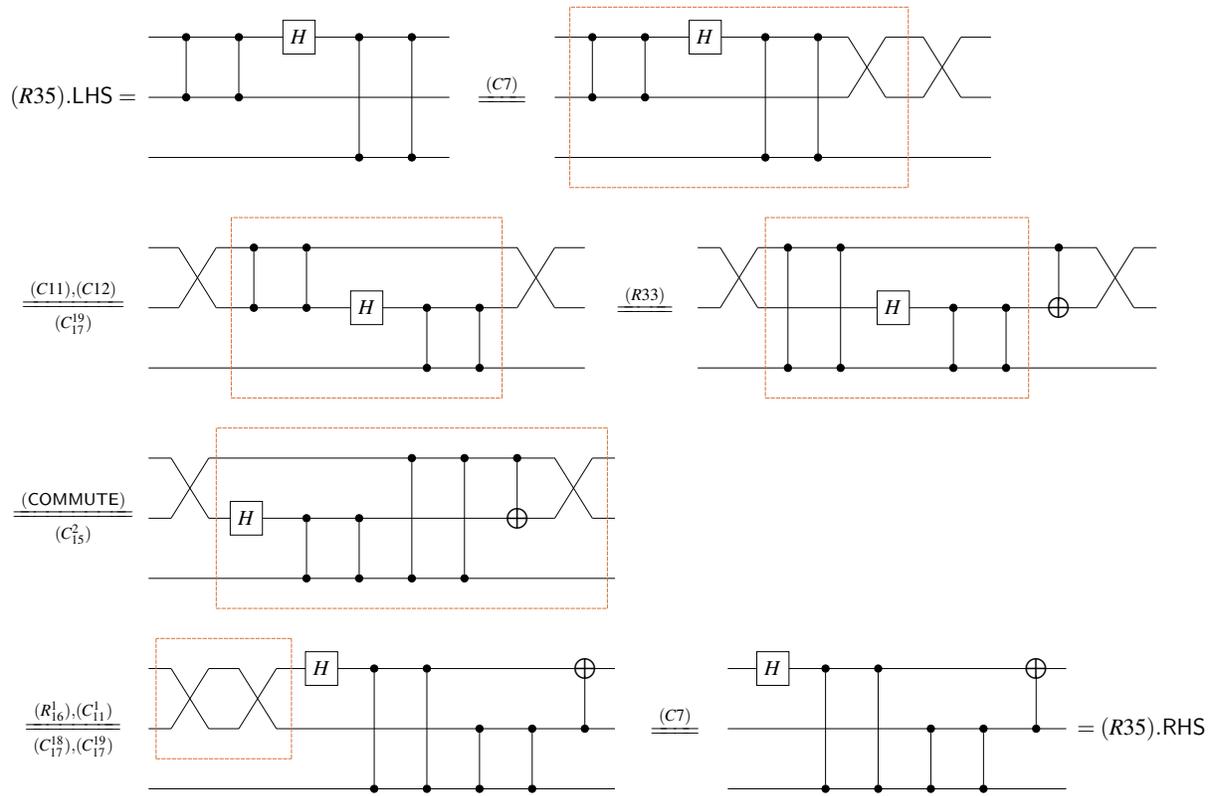

□

**Lemma 4.27.** (R36) and (R37) follow from the reduced relations.

(R36)

(R37)

*Proof.*

(R36).LHS =  $\xrightarrow{(C_{18}^1)}$   $\xrightarrow{\frac{(C_{15})}{(C_{18}^1)}}$   $\xrightarrow{(C_{14}^1)}$   $\cdot \omega^2 \xrightarrow{\frac{(C_{13}^1)}{(R_{17}^1)}}$   $\cdot \omega^2$   $\xrightarrow{\frac{(C_{15}^1), (C_{15}^2)}{(C_3), (C_{15}^1)}}$   $\cdot \omega$   $\xrightarrow{(C_{13}^{14+})}$   $\cdot \omega$   $\xrightarrow{\frac{(C_8), (C_8^1)}{(R_{18})}}$   $\cdot \omega$   $\xrightarrow{\frac{(C_3)}{(C_5)}}$   $\cdot \omega$   $\xrightarrow{(C_{13}^1)}$   $\xrightarrow{\frac{(\text{COMMUTE}^2)}{(C_5), (C_8^1)}}$  = (R36).RHS

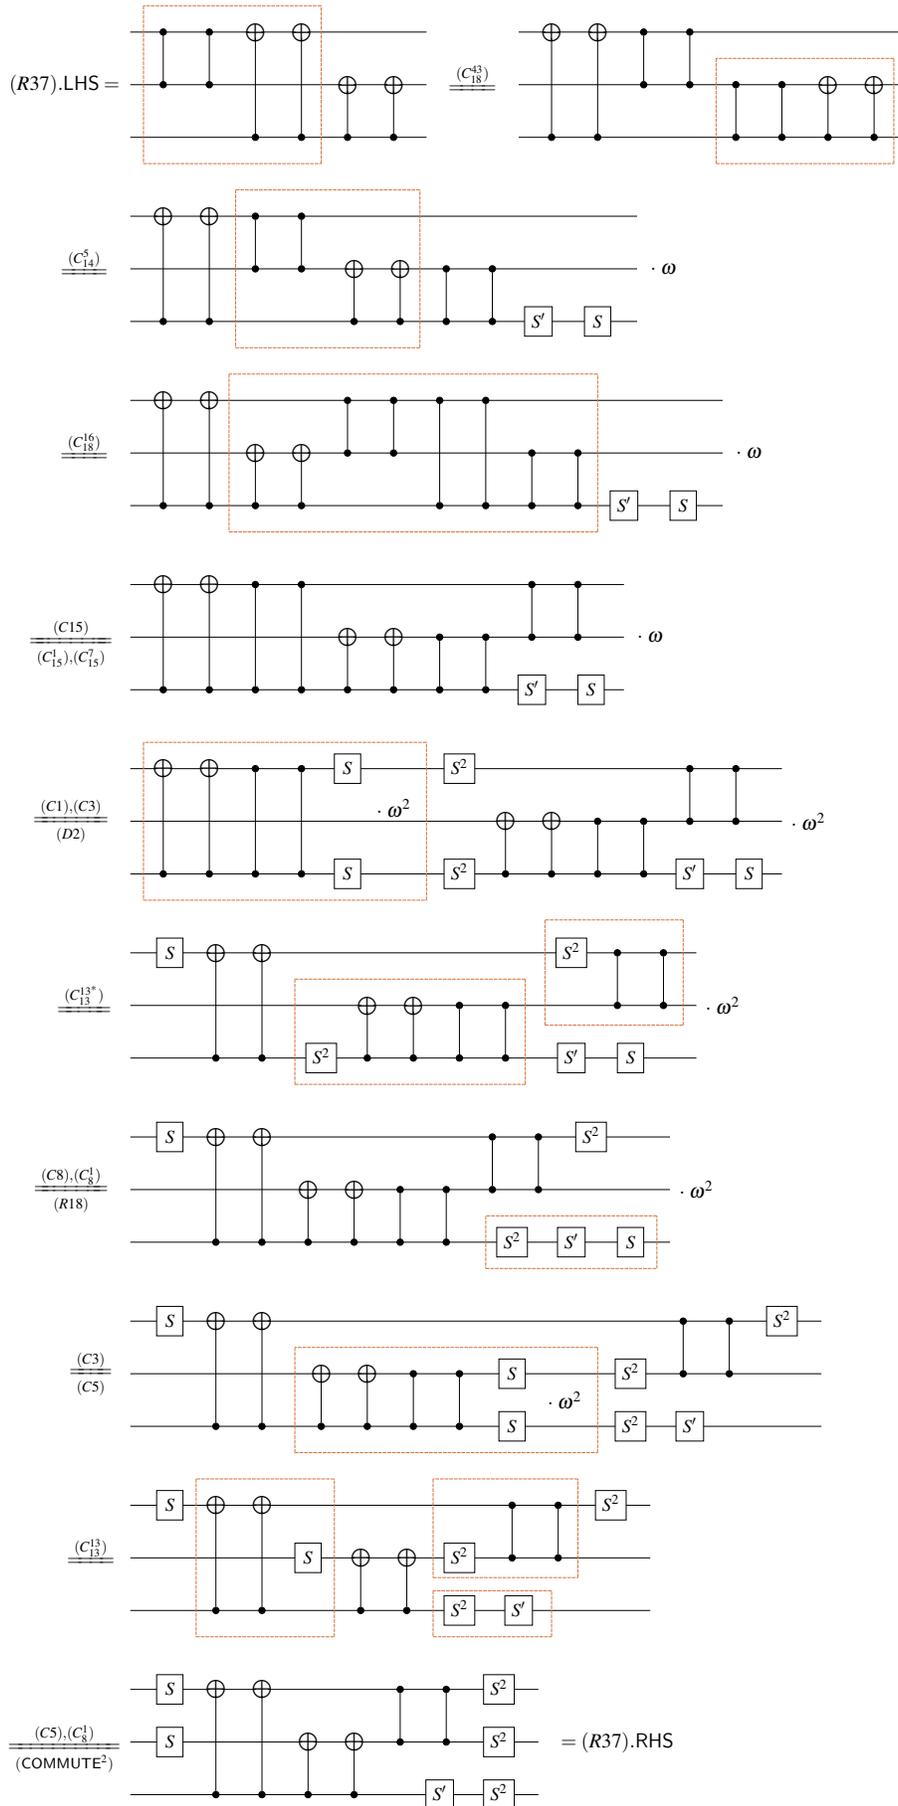

□

**Lemma 4.28.** (R38) and (R39) follow from the reduced relations.

(R38)

(R39)

*Proof.*

(R38).LHS =  $\stackrel{(C2)}{=} \stackrel{(COMMUTE)}{=}$

$\stackrel{(C_{18}^8)}{=} \stackrel{(C2)}{=}$

$\stackrel{(C_{19}^{22})}{=}$

$\stackrel{(C9)}{=}$

$\stackrel{(D7)}{=}$

$\stackrel{(C2)}{=} = (R38).RHS$

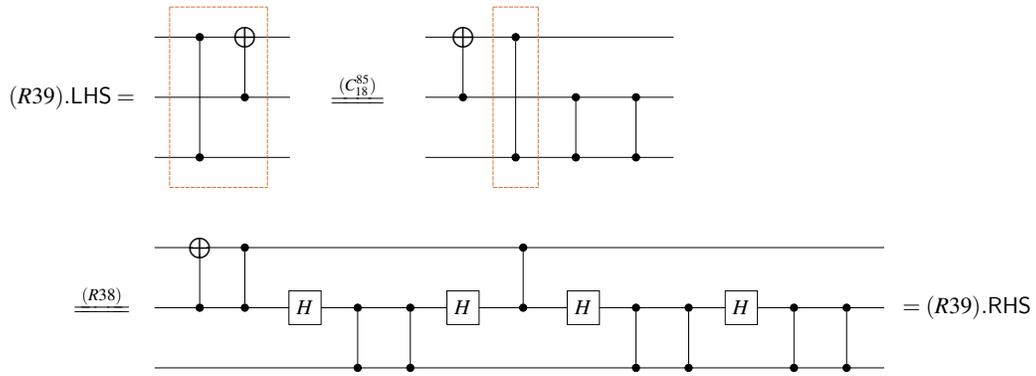

**Lemma 4.29.** (R40) and (R41) follow from the reduced relations.

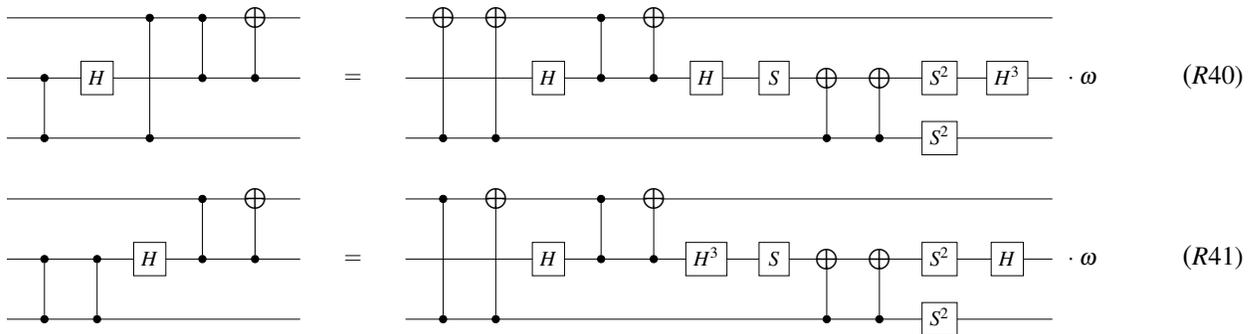

*Proof.* First, (37) simplifies the righthand side of (R40), so it suffices to derive (36) from the equations in Figure 1 and section 1.

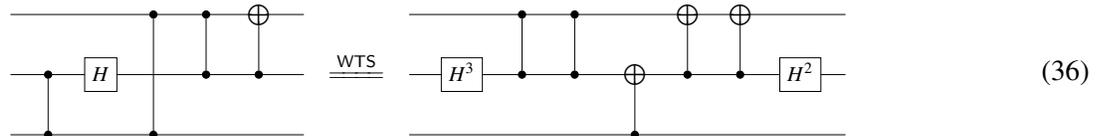

Left-appepending both sides of (36) by  $I \otimes H \otimes I$  yields

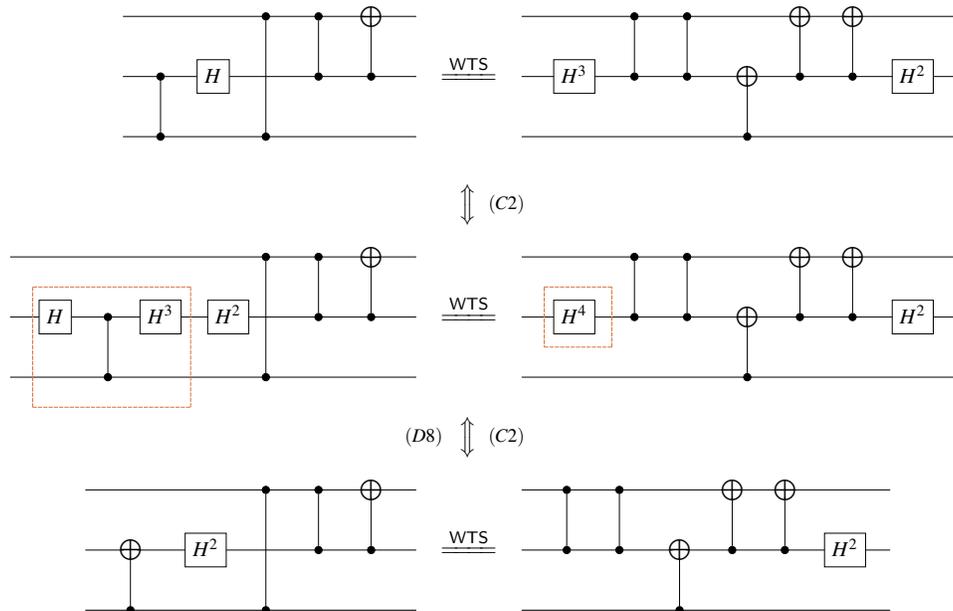

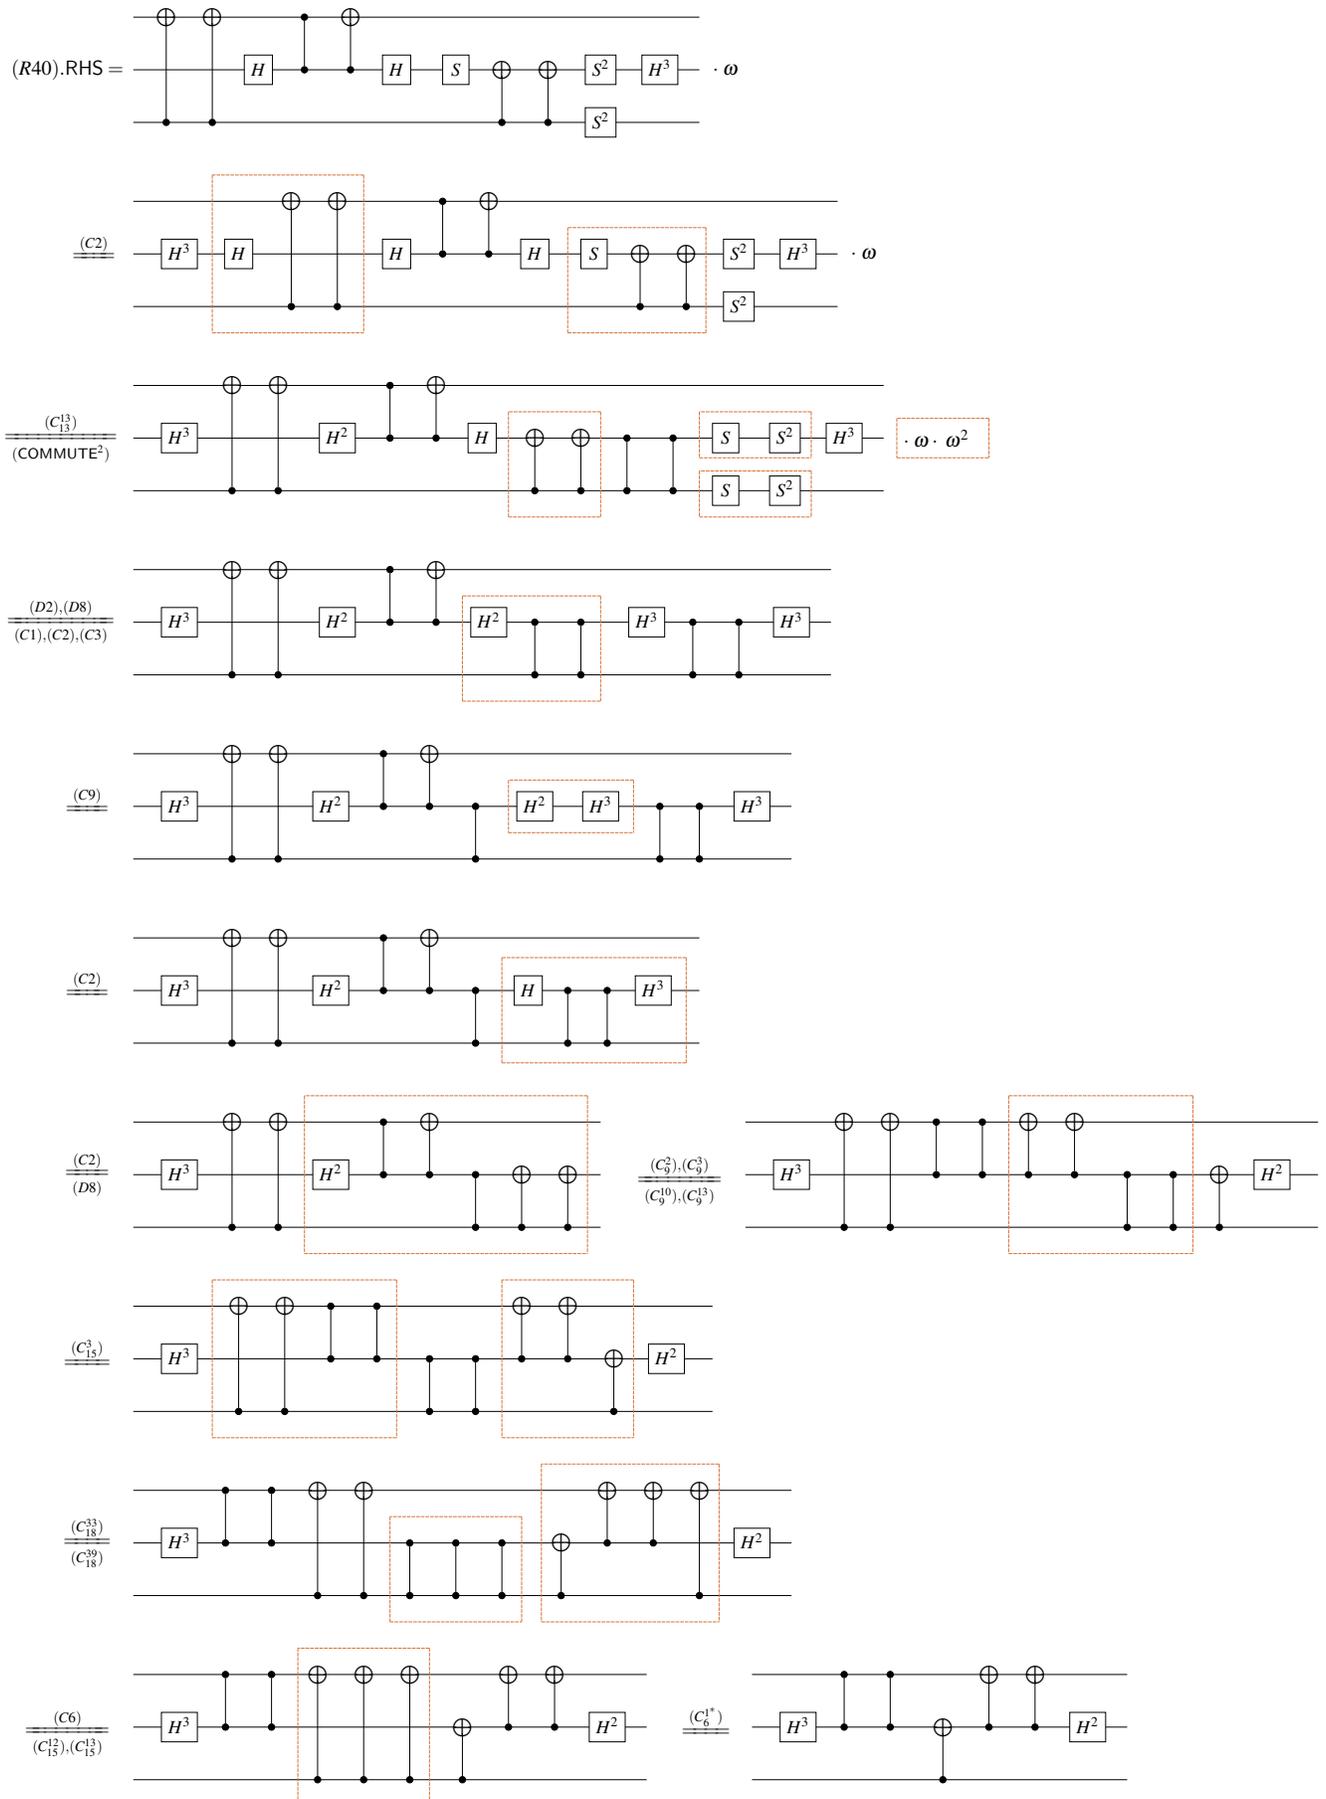

Thus, it suffices to derive (38).

(38)

We proceed as follows, which completes the proof.

(38).LHS =  $\xrightarrow{\text{(COMMUTE)}}$   $\xrightarrow{\frac{(C_9^3)}{(C_9^{13})}}$   $\xrightarrow{\frac{(C_{18}^{11})}{(C_6^*)}}$  = (38).RHS

To derive (R41) from the equations in Figure 1 and section 1, (40) first simplifies the righthand side of it. Hence, it suffices to show that (39) follows from the equations in Figure 1 and section 1.

(39)

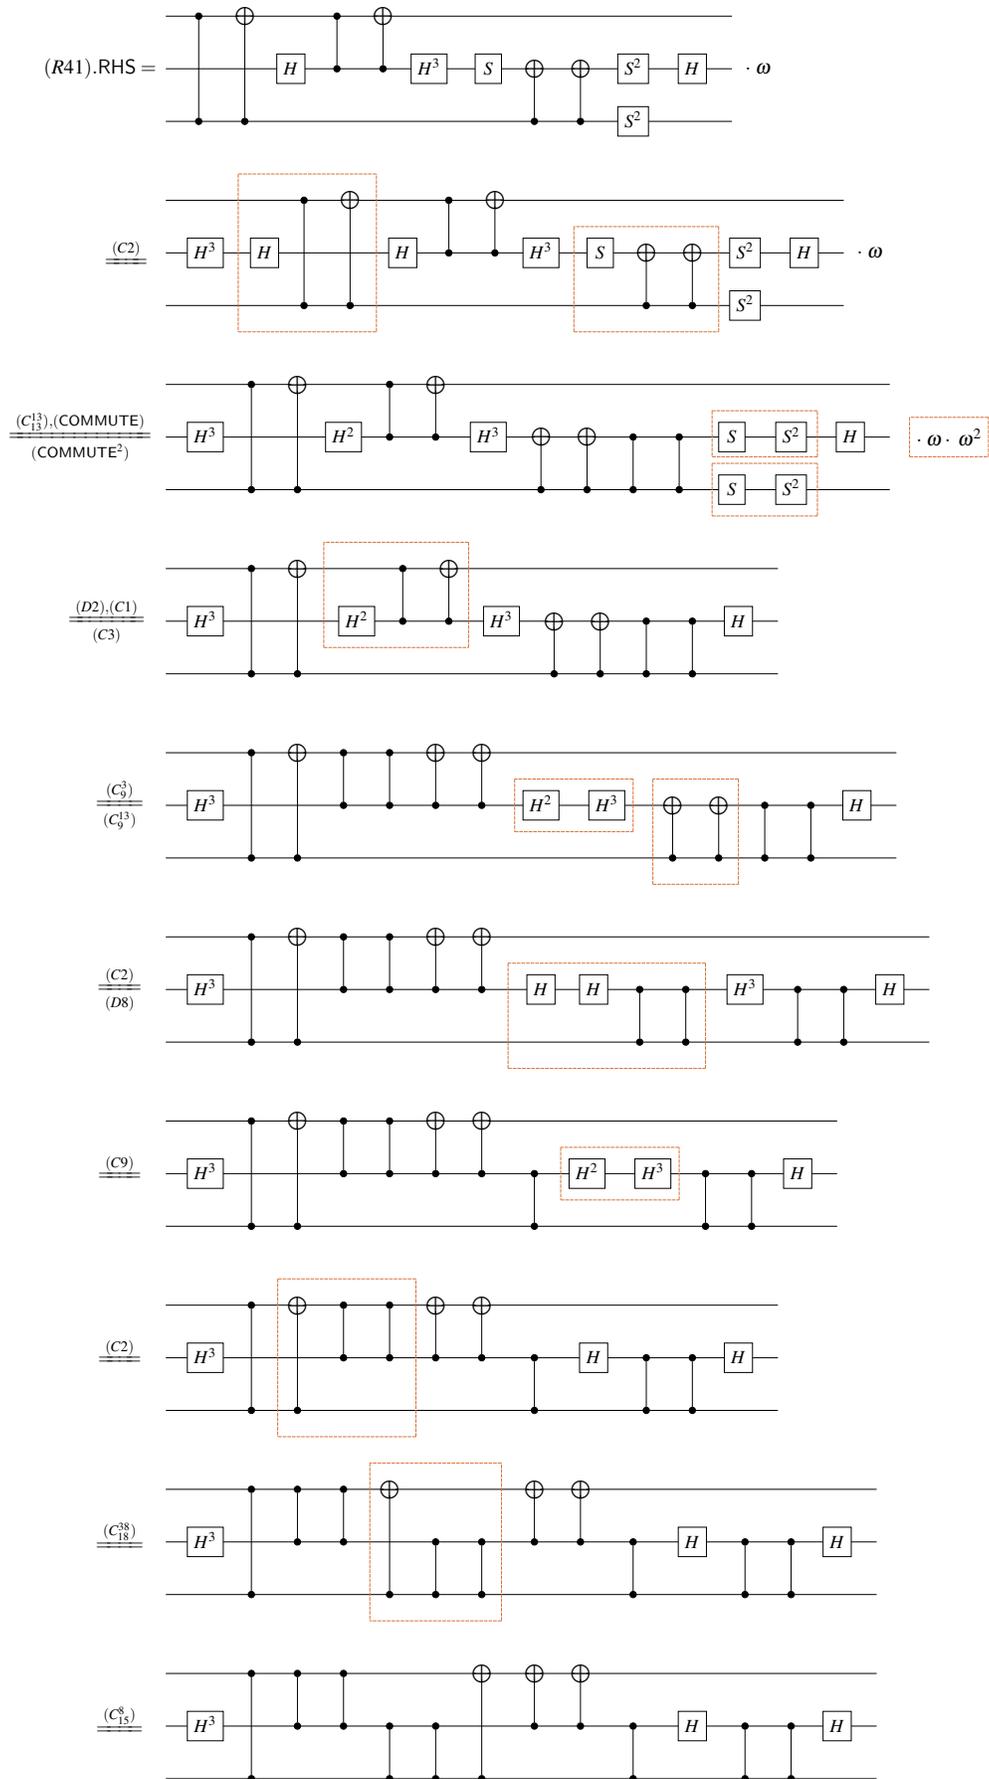

Left-appending both sides of (39) by  $I \otimes H \otimes I$  yields

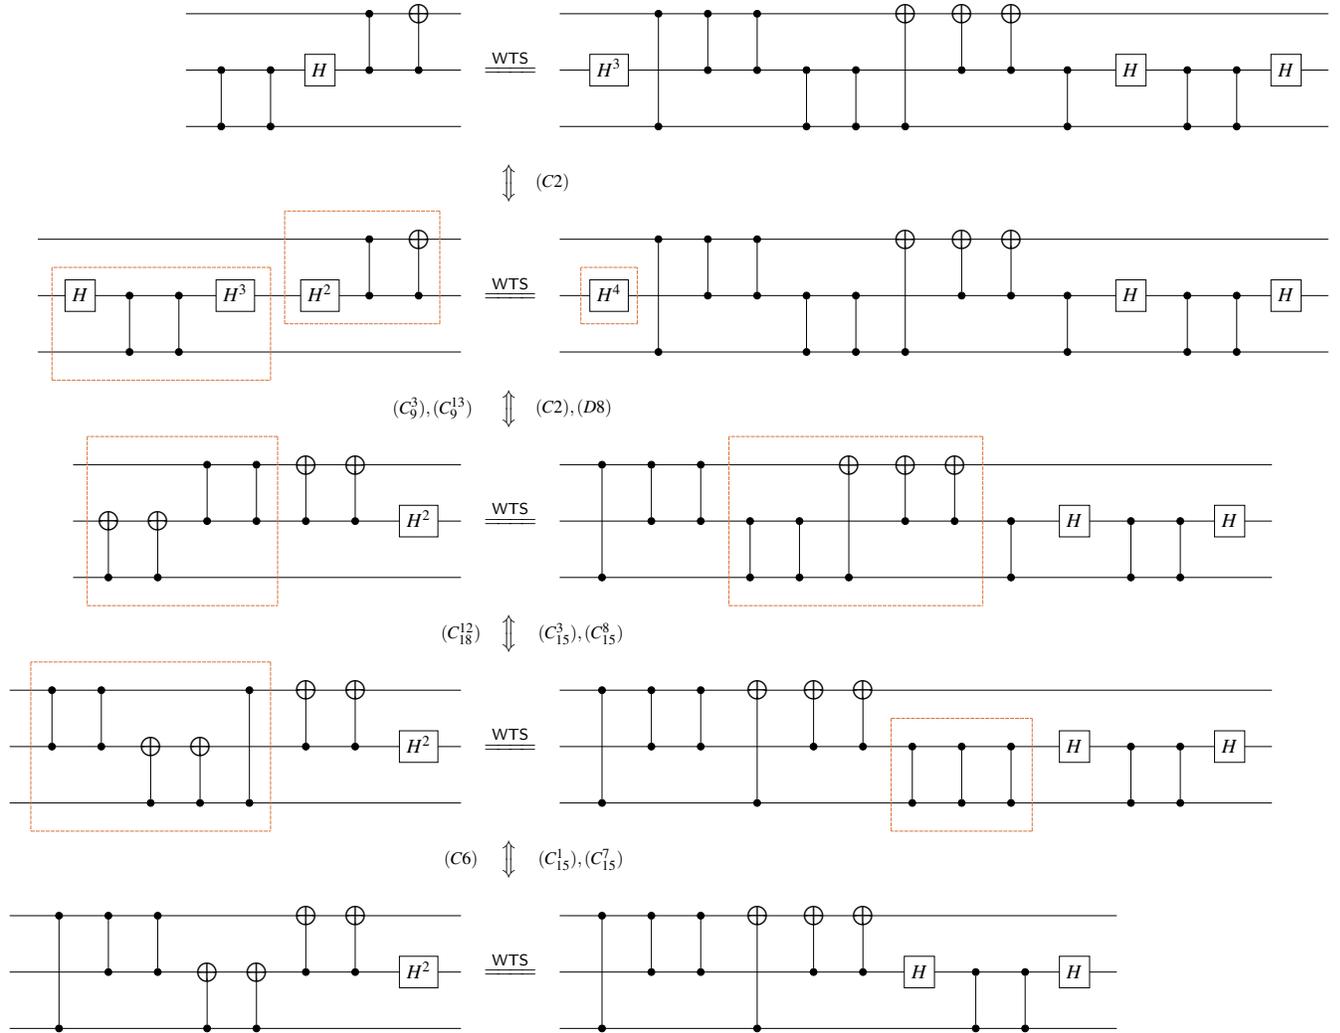

Thus, it suffices to derive (41).

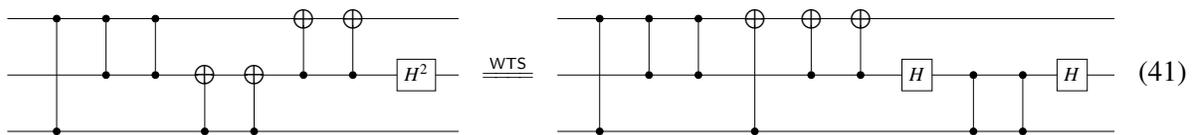

Right-appending both sides of (41) by  $I \otimes H^2 \otimes I$  yields

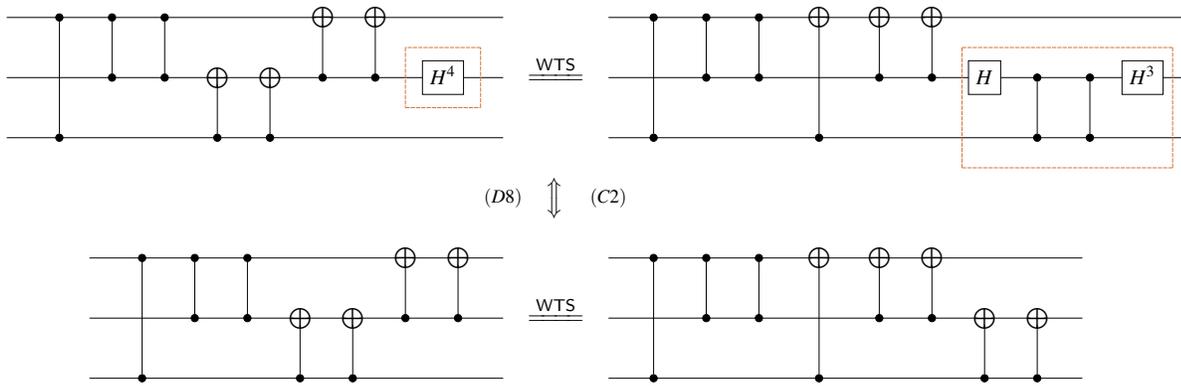

Therefore, our problem is reduced to deriving (42), which follow from  $(C_{18}^{30})$ ,  $(C_{15}^{12})$ , and  $(C_{15}^{13})$ .

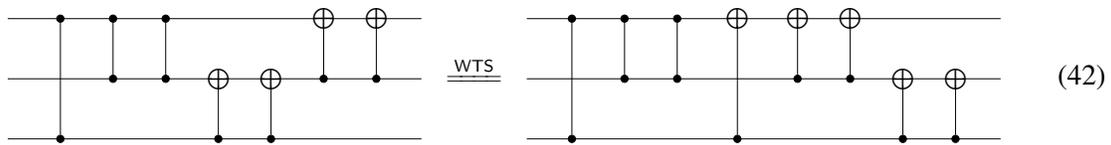

□

**Lemma 4.30.** (R42) and (R43) follow from the reduced relations.

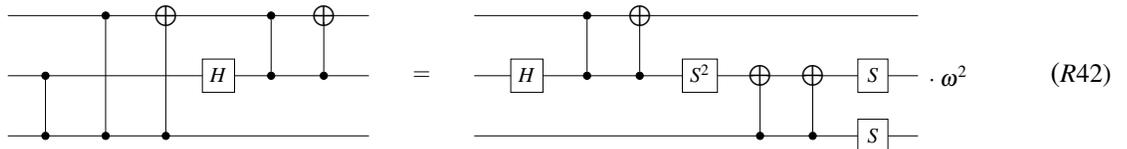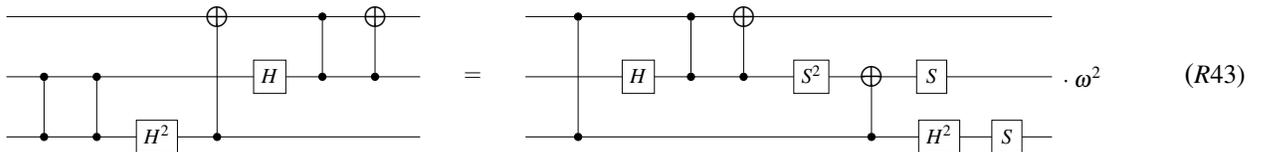

*Proof.* First, (44) simplifies the righthand side of (R42), so it suffices to derive (43) from the equations in Figure 1 and section 1.

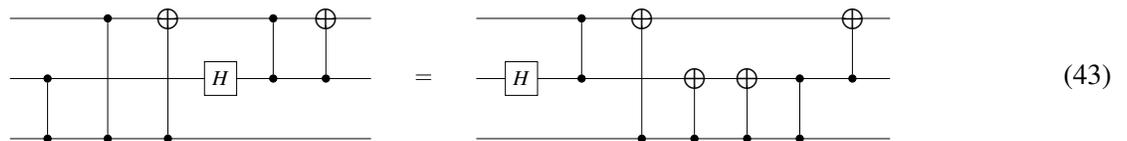

(R42).RHS = 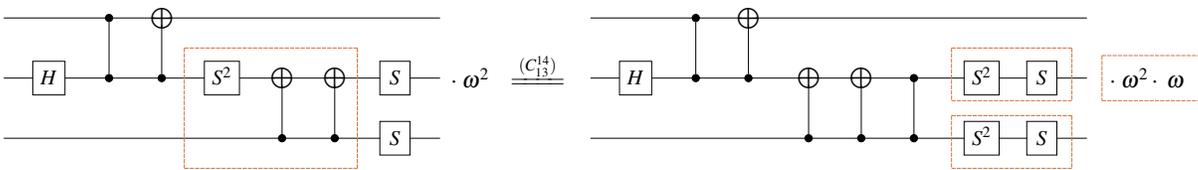

$\xrightarrow[\text{(C3)}]{\text{(D2),(C1)}} \xrightarrow[\text{(C18)}]{\text{(C32)}} \xrightarrow[\text{(C15)}]{\text{(C15)}^3}$

(44)

Left-appepending both sides of (43) by  $I \otimes H \otimes I$  yields

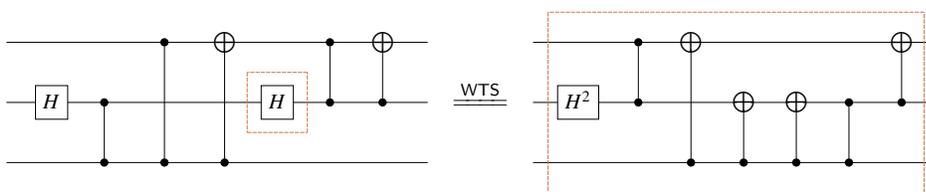

$\xrightarrow[\text{(C9)}]{\text{(C9)}^2, \text{(C9)}^3, \text{(C9)}^0, \text{(C9)}^{13}} \updownarrow \text{(C2), (COMMUTE}^2)$

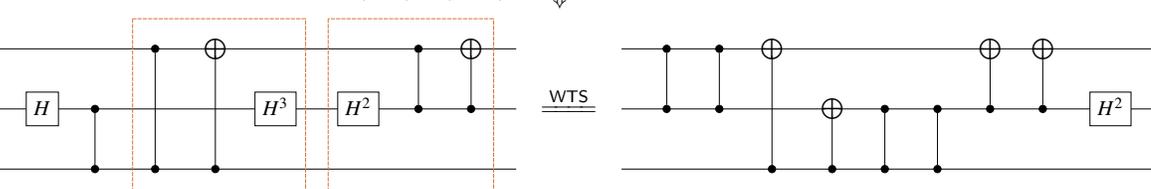

$\xrightarrow[\text{(C9)}]{\text{(C9)}^3, \text{(C9)}^{13}} \updownarrow \text{(COMMUTE), (COMMUTE}^2)$

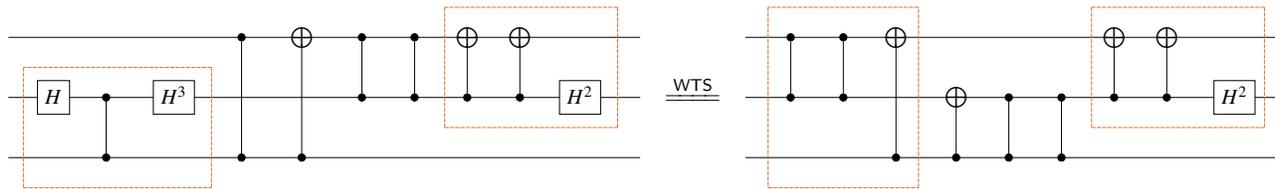

$\xrightarrow[\text{(D8), (C6)}]{\text{(C2), (C18)}^4}$

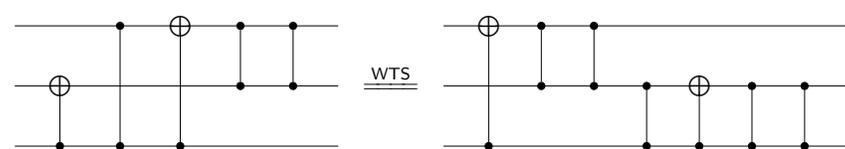

Therefore, our problem is reduced to deriving (45), which is shown below.

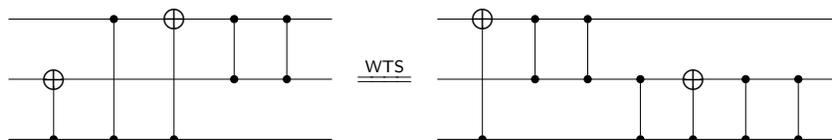

(45)

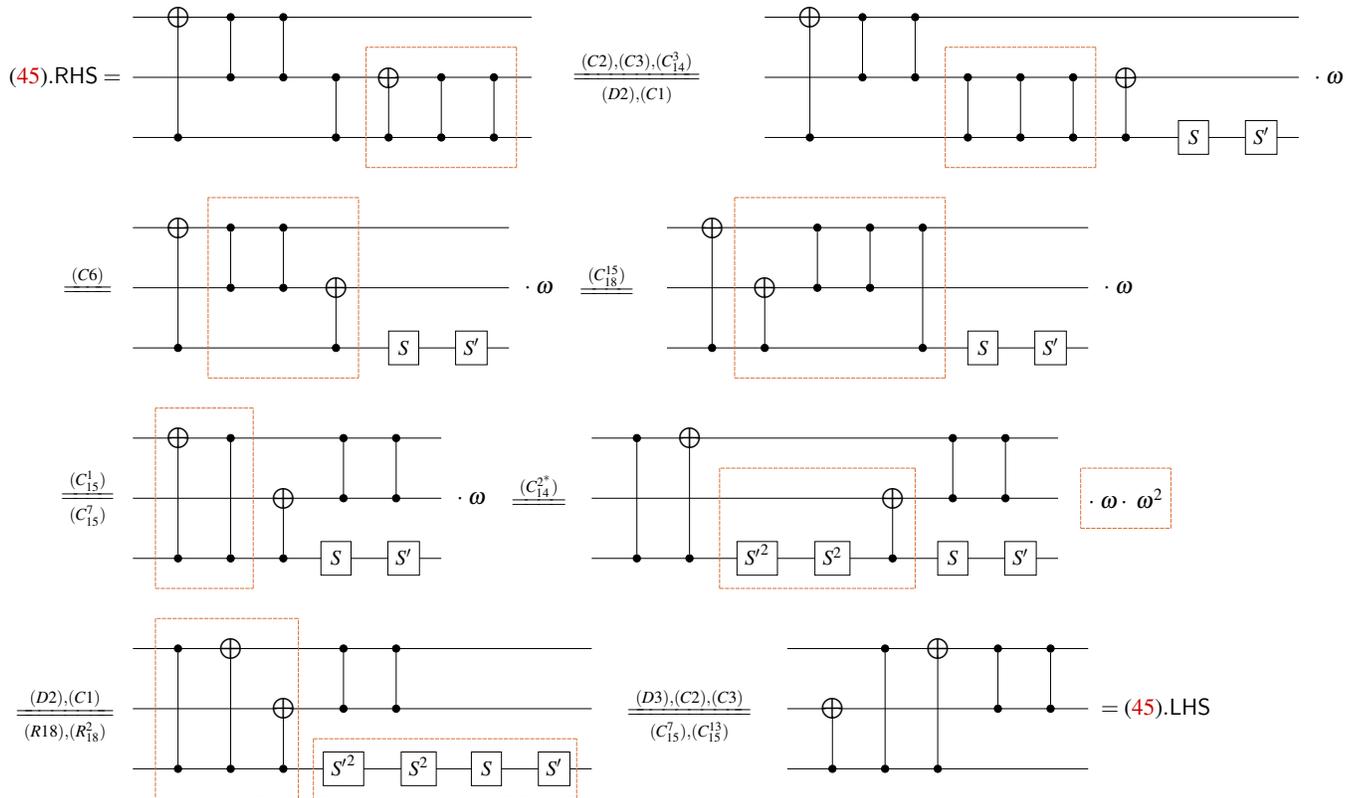

To derive (R43) from the equations in Figure 1 and section 1, (48) first simplifies the righthand side of it. Hence, it suffices to show that (46) follows from the equations in Figure 1 and section 1.

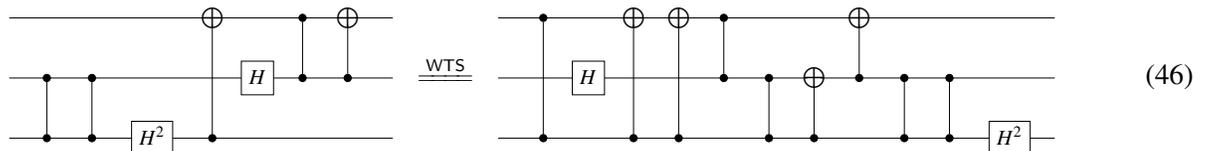

Right-appending both sides of (46) by  $I \otimes I \otimes H^2$  yields

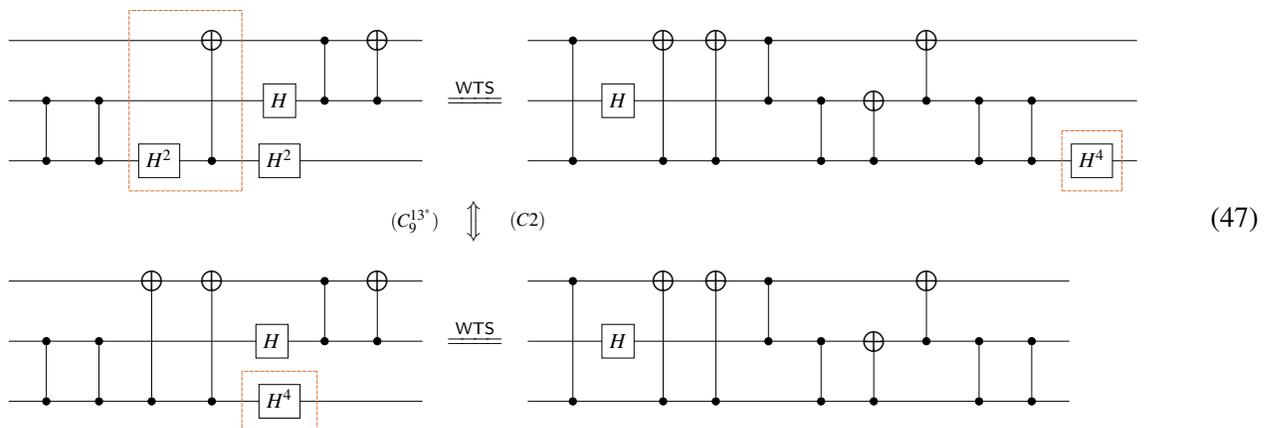

(R43).RHS = 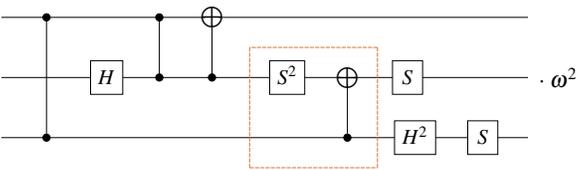

(C13) 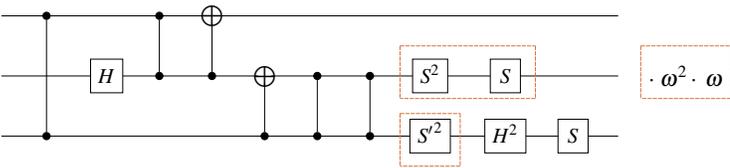

(D2),(D3)  
(C1),(C2),(C3) 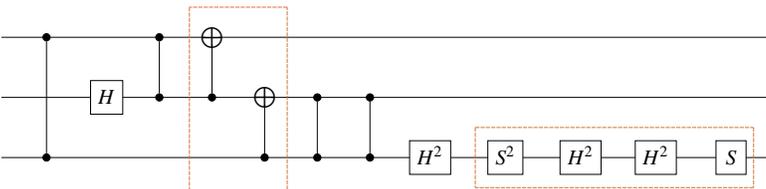

(C2),(C3)  
(C18) 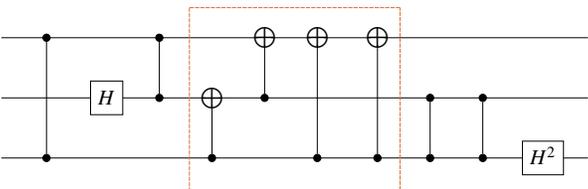

(C12)  
(C15) 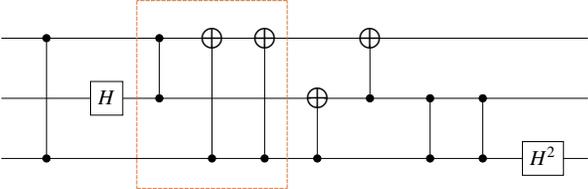

(C41)  
(C18) 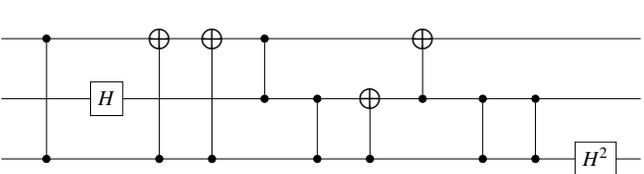

(48)

By (C2), it suffices to derive (49).

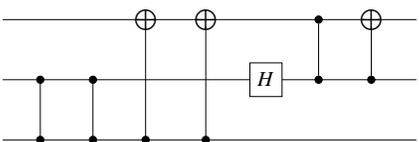  $\xrightarrow{\text{WTS}}$  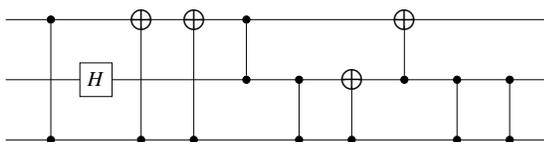

(49)

Left-appending both sides of (49) by  $I \otimes H \otimes I$  yields

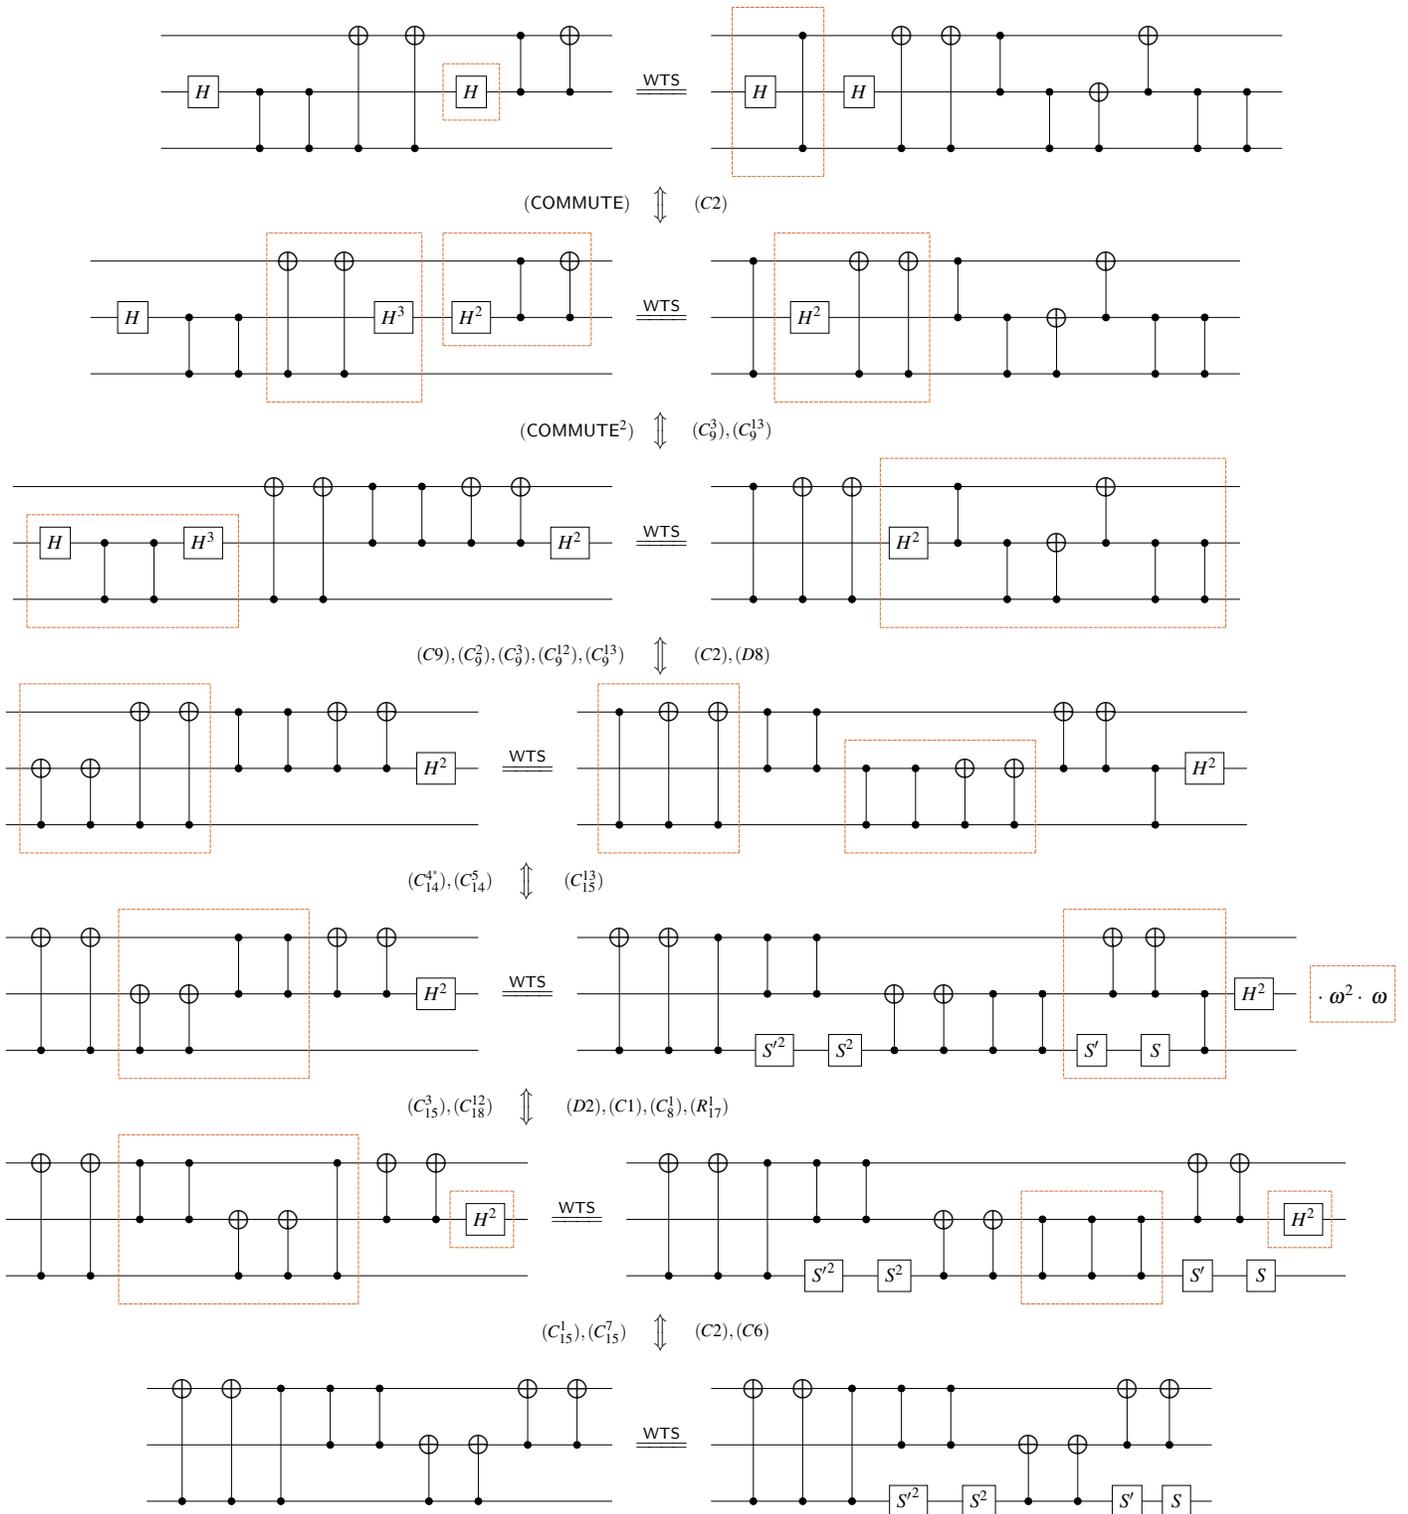

Thus, it suffices to derive (50).

(50)

We proceed as follows and this completes the proof.

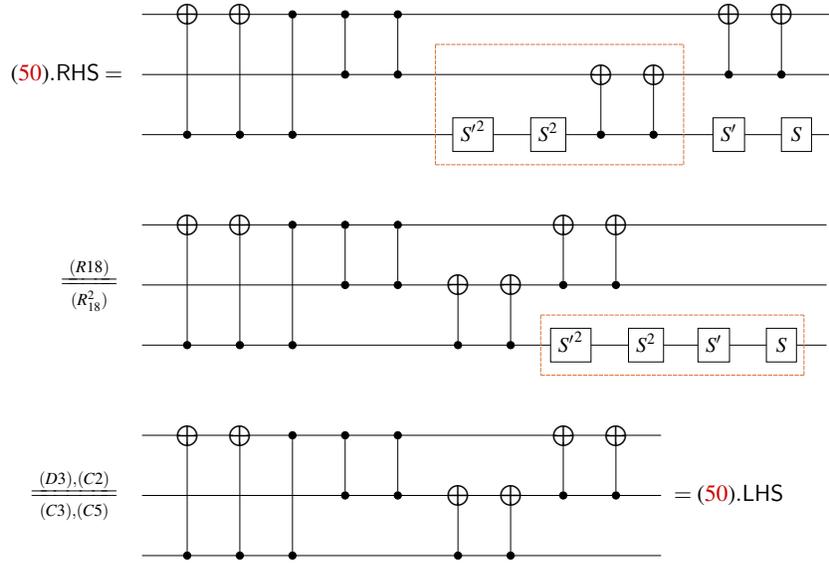

□

**Lemma 4.31.** (R44) and (R45) follow from the reduced relations.

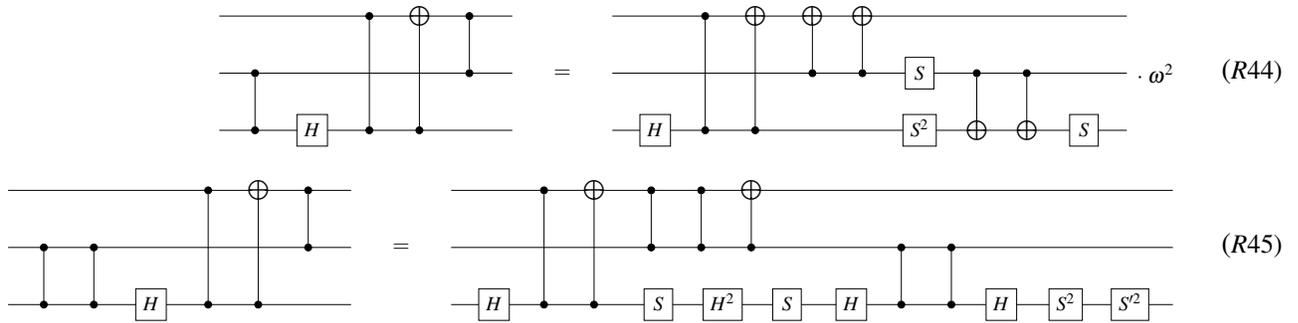

*Proof.* First, (52) simplifies the righthand side of (R44), so it suffices to derive (51) from the equations in Figure 1 and section 1.

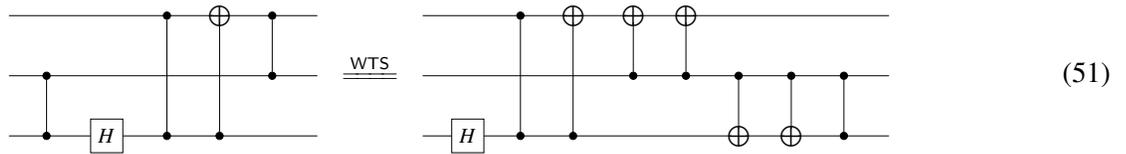

Combined with (C2), left-append both sides of (51) by  $I \otimes I \otimes H$ .

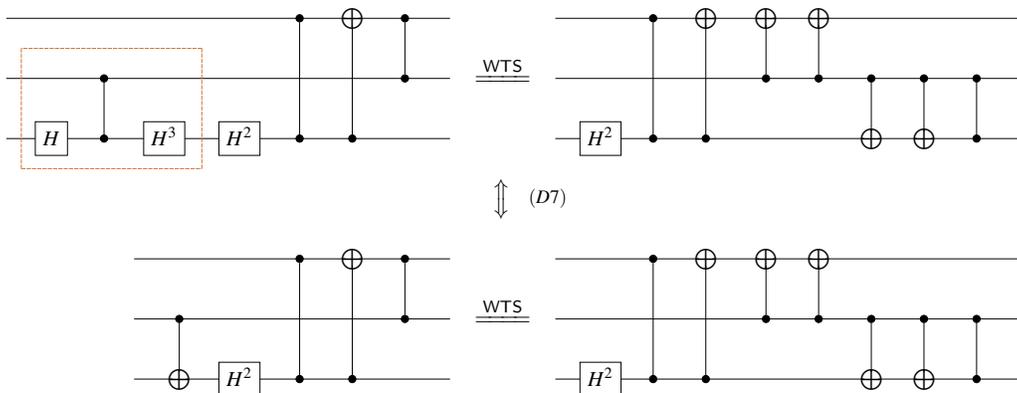

$$\begin{aligned}
 (R44).RHS = & \text{Quantum circuit with 3 qubits, gates } H, S, S^2, \text{ and } \omega^2. \\
 \frac{(C_{13}^{16})}{(R_{18}^{18})} & \text{Quantum circuit with 3 qubits, gates } H, S, S^2, \text{ and } \omega^2 \cdot \omega. \\
 \frac{(D2),(C1)}{(C3)} & \text{Quantum circuit with 3 qubits, gates } H, S, S^2.
 \end{aligned} \tag{52}$$

It follows that

$$\text{Quantum circuit with } H^2 \text{ gate} \xrightarrow{\text{WTS}} \text{Quantum circuit with } H^2 \text{ gate} \tag{53}$$

Then we simplify both sides of (53) using the rewrite rules listed in Figure 1 and section 1. Since the lefthand side is simplified to exactly match the righthand side, the proof is complete.

$$\begin{aligned}
 & \text{Quantum circuit with } H^2 \text{ gate} \xrightarrow{\text{WTS}} \text{Quantum circuit with } H^2 \text{ gate} \\
 & \quad \quad \quad \updownarrow (C_9^{3^*}), (C_9^{13^*}) \quad \quad \quad \updownarrow (C_9^3), (C_9^{20}) \\
 & \text{Quantum circuit with } H^2 \text{ gate} \xrightarrow{\text{WTS}} \text{Quantum circuit with } H^2 \text{ gate} \\
 & \quad \quad \quad \updownarrow (C_{18}^{74}) \\
 & \text{Quantum circuit with } H^2 \text{ gate} \xrightarrow{\text{WTS}} \text{Quantum circuit with } H^2 \text{ gate}
 \end{aligned}$$

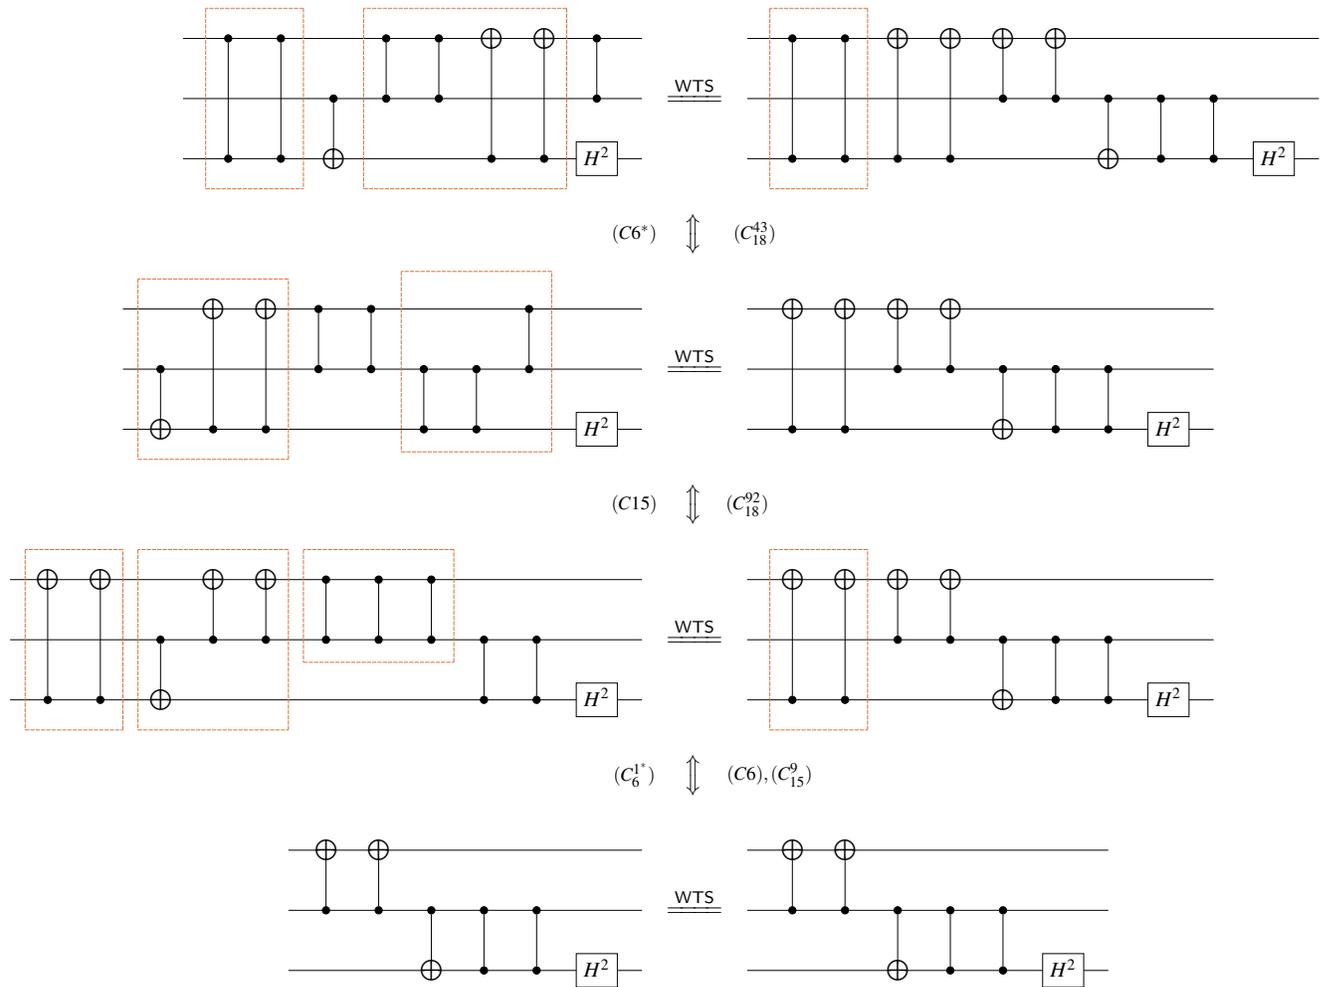

To derive (R45) from the equations in Figure 1 and section 1, (55) first simplifies the righthand side of it. Hence, it suffices to show that (54) follows from the equations in Figure 1 and section 1.

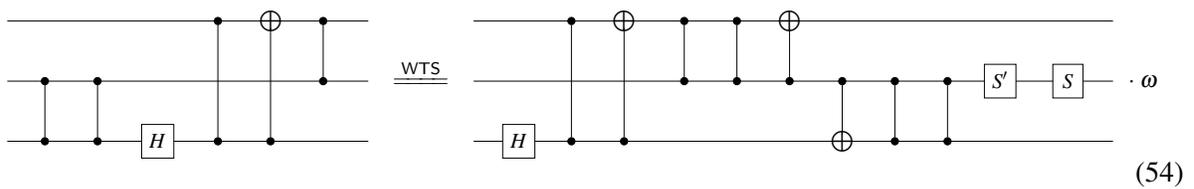

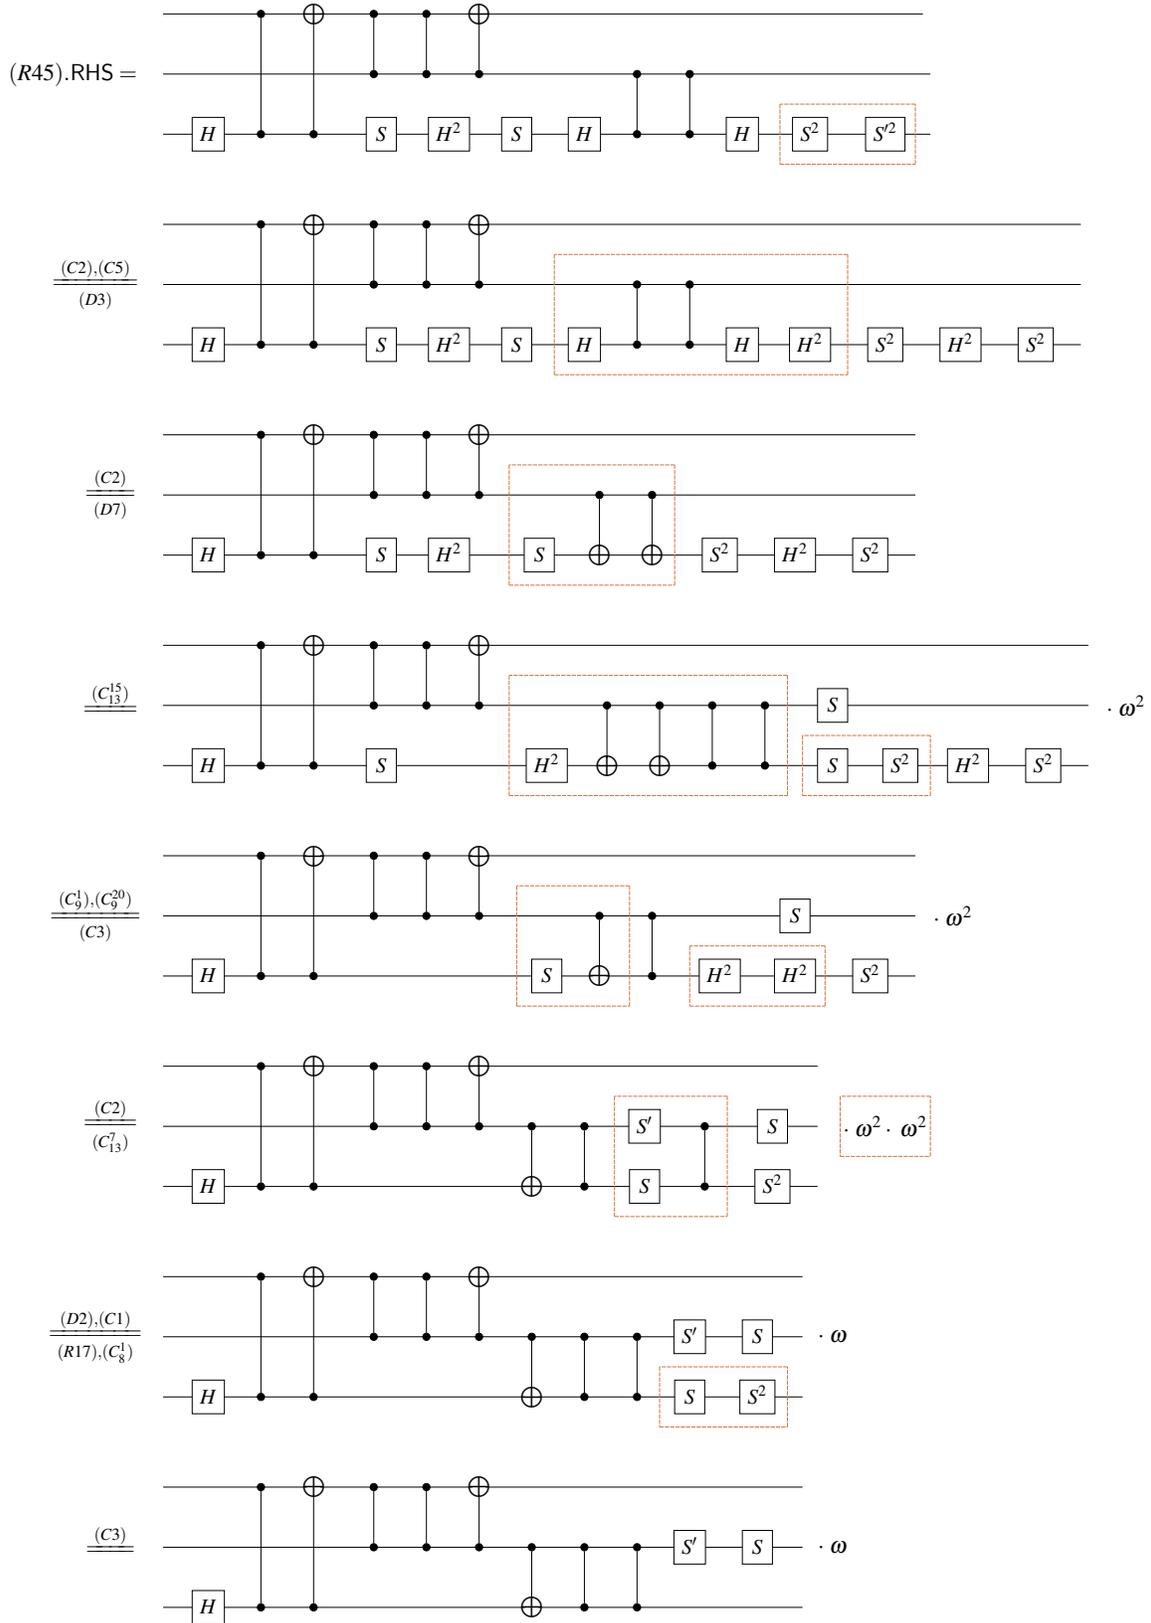

Left-appepending both sides of (54) by  $I \otimes I \otimes H$  yields

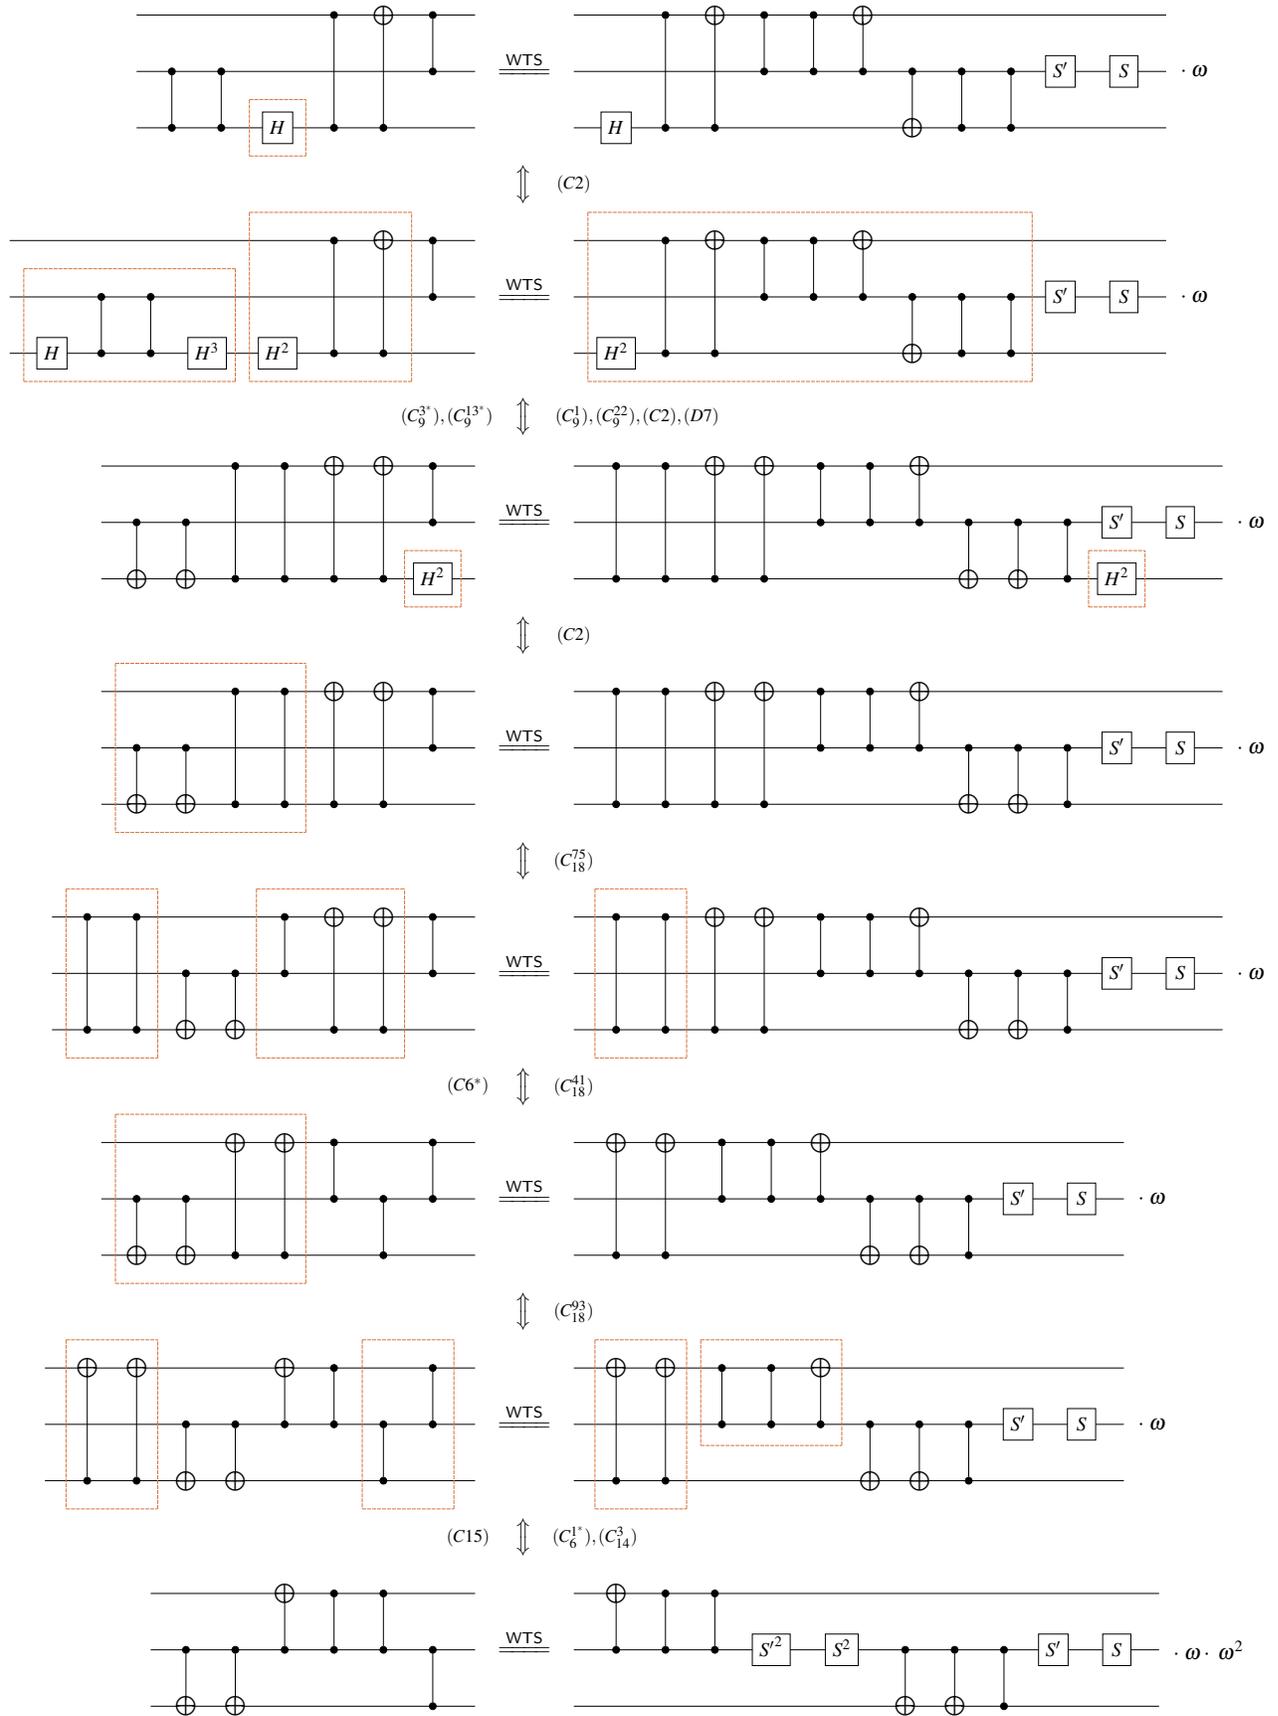

By (D2) and (C1), it suffices to derive (56).

(56)

We proceed as follows, and this completes the proof.

□

**Lemma 4.32.** (R46) and (R47) follow from the reduced relations.

(R46)

(R47)

*Proof.* First, (58) simplifies the righthand side of (R46), so it suffices to derive (57) from the equations in Figure 1 and section 1.

(57)

$$\begin{aligned}
 (R46).RHS = & \text{Circuit diagram with 3 qubits. Top qubit has a control dot and target line with a circle containing a plus sign. Middle qubit has a control dot and target line with a circle containing a plus sign. Bottom qubit has a control dot and target line with a circle containing a plus sign. A dashed box encloses  $S'$  and  $S^2$  on the middle qubit, and  $S^2$  on the bottom qubit. A  $H$  gate is on the bottom qubit. A  $S$  gate is on the bottom qubit. (58) \\
 \frac{(R_{18}^1), (R_{18}^3)}{(C_{13}^6)} & \text{Circuit diagram similar to the first, but with a dashed box around  $S^2$  and  $S'$  on the middle qubit, and  $S^2$  and  $S$  on the bottom qubit. A  $\cdot \omega$  symbol is on the right. \\
 \frac{(C3)}{(C5)} & \text{Circuit diagram similar to the second, but with a dashed box around  $S$  and  $S'$  on the middle qubit. A  $\cdot \omega$  symbol is on the right.
 \end{aligned}$$

Left-appending both sides of (57) by  $I \otimes I \otimes H$  yields

$$\begin{aligned}
 & \text{Circuit diagram with 3 qubits. Top qubit has a control dot and target line with a circle containing a plus sign. Middle qubit has a control dot and target line with a circle containing a plus sign. Bottom qubit has a control dot and target line with a circle containing a plus sign. A dashed box encloses an  $H$  gate on the bottom qubit. \\
 & \xrightarrow{\text{WTS}} \text{Circuit diagram with 3 qubits. Top qubit has a control dot and target line with a circle containing a plus sign. Middle qubit has a control dot and target line with a circle containing a plus sign. Bottom qubit has a control dot and target line with a circle containing a plus sign. A dashed box encloses  $S$  and  $S'$  on the middle qubit, and  $S$  and  $S'$  on the bottom qubit. A  $\cdot \omega$  symbol is on the right. \\
 & \updownarrow (C2) \\
 & \text{Circuit diagram with 3 qubits. Top qubit has a control dot and target line with a circle containing a plus sign. Middle qubit has a control dot and target line with a circle containing a plus sign. Bottom qubit has a control dot and target line with a circle containing a plus sign. A dashed box encloses  $H$  and  $H^3$  on the bottom qubit, and  $H^2$  on the middle qubit. \\
 & \xrightarrow{\text{WTS}} \text{Circuit diagram with 3 qubits. Top qubit has a control dot and target line with a circle containing a plus sign. Middle qubit has a control dot and target line with a circle containing a plus sign. Bottom qubit has a control dot and target line with a circle containing a plus sign. A dashed box encloses  $H^2$  on the middle qubit, and  $S$  and  $S'$  on the bottom qubit. A  $\cdot \omega$  symbol is on the right. \\
 & \updownarrow (D7), (C_9^{3*}), (C_9^{13*}) \quad \updownarrow (C_9^3), (C_9^{20}) \\
 & \text{Circuit diagram with 3 qubits. Top qubit has a control dot and target line with a circle containing a plus sign. Middle qubit has a control dot and target line with a circle containing a plus sign. Bottom qubit has a control dot and target line with a circle containing a plus sign. A dashed box encloses  $H^2$  on the bottom qubit. \\
 & \xrightarrow{\text{WTS}} \text{Circuit diagram with 3 qubits. Top qubit has a control dot and target line with a circle containing a plus sign. Middle qubit has a control dot and target line with a circle containing a plus sign. Bottom qubit has a control dot and target line with a circle containing a plus sign. A dashed box encloses  $S$  and  $S'$  on the middle qubit, and  $H^2$  on the bottom qubit. A  $\cdot \omega$  symbol is on the right. \\
 & \updownarrow (C_{18}^{74}) \\
 & \text{Circuit diagram with 3 qubits. Top qubit has a control dot and target line with a circle containing a plus sign. Middle qubit has a control dot and target line with a circle containing a plus sign. Bottom qubit has a control dot and target line with a circle containing a plus sign. A dashed box encloses  $H^2$  on the bottom qubit. \\
 & \xrightarrow{\text{WTS}} \text{Circuit diagram with 3 qubits. Top qubit has a control dot and target line with a circle containing a plus sign. Middle qubit has a control dot and target line with a circle containing a plus sign. Bottom qubit has a control dot and target line with a circle containing a plus sign. A dashed box encloses  $S$  and  $S'$  on the middle qubit, and  $H^2$  on the bottom qubit. A  $\cdot \omega$  symbol is on the right. \\
 & \updownarrow (C6^*) \quad \updownarrow (C_{18}^{43}) \\
 & \text{Circuit diagram with 3 qubits. Top qubit has a control dot and target line with a circle containing a plus sign. Middle qubit has a control dot and target line with a circle containing a plus sign. Bottom qubit has a control dot and target line with a circle containing a plus sign. A dashed box encloses  $H^2$  on the bottom qubit. \\
 & \xrightarrow{\text{WTS}} \text{Circuit diagram with 3 qubits. Top qubit has a control dot and target line with a circle containing a plus sign. Middle qubit has a control dot and target line with a circle containing a plus sign. Bottom qubit has a control dot and target line with a circle containing a plus sign. A dashed box encloses  $S$  and  $S'$  on the middle qubit, and  $H^2$  on the bottom qubit. A  $\cdot \omega$  symbol is on the right.
 \end{aligned}$$

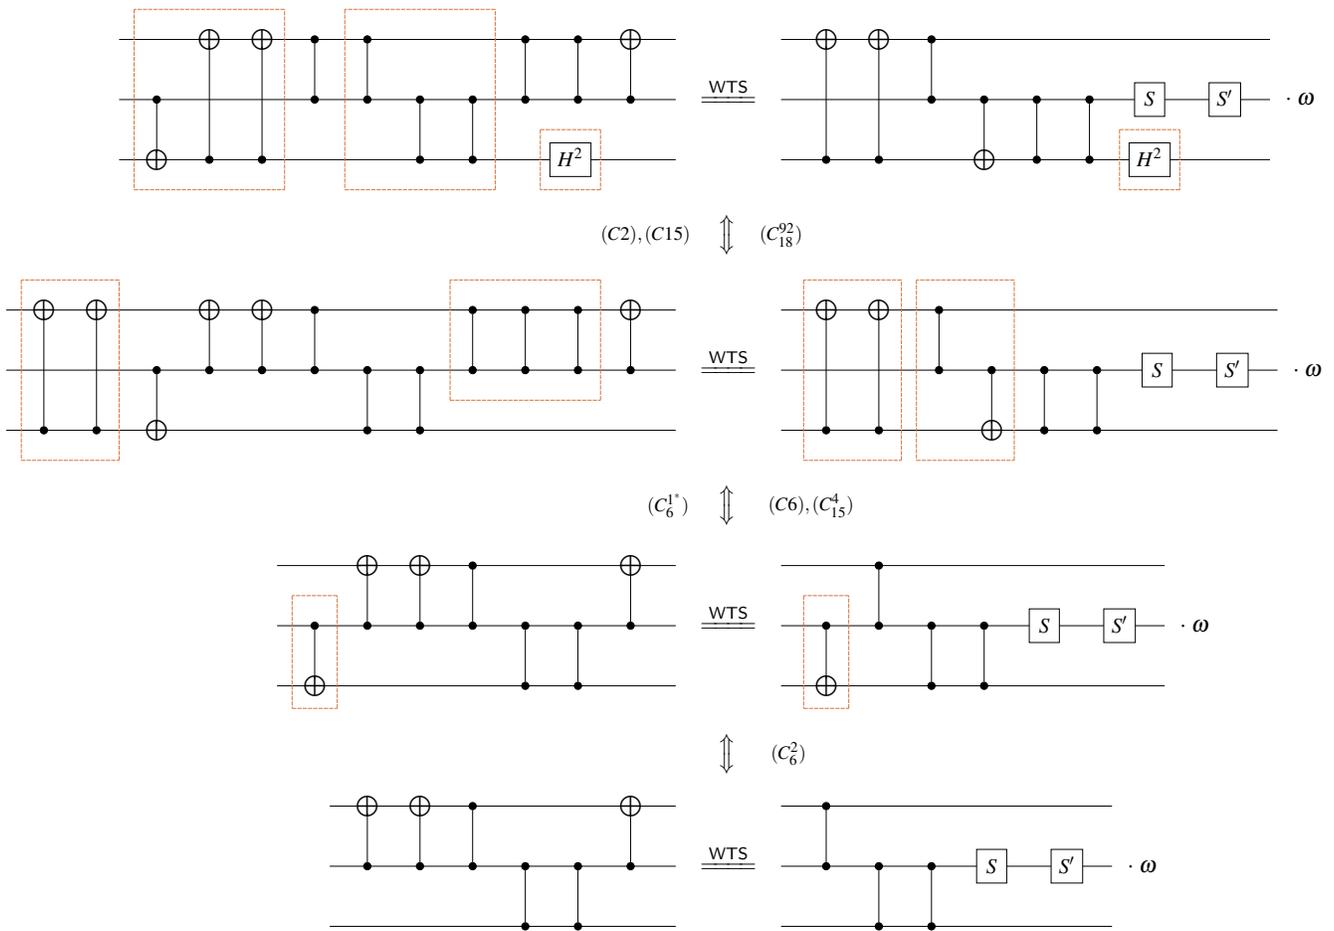

Thus, it suffices to derive (59).

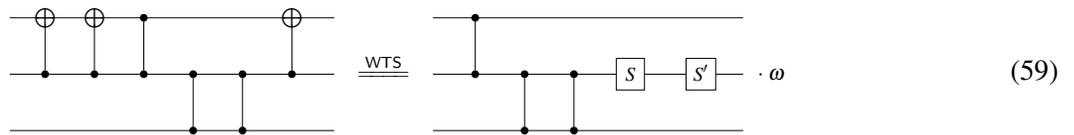

We proceed as follows, and this completes the proof.

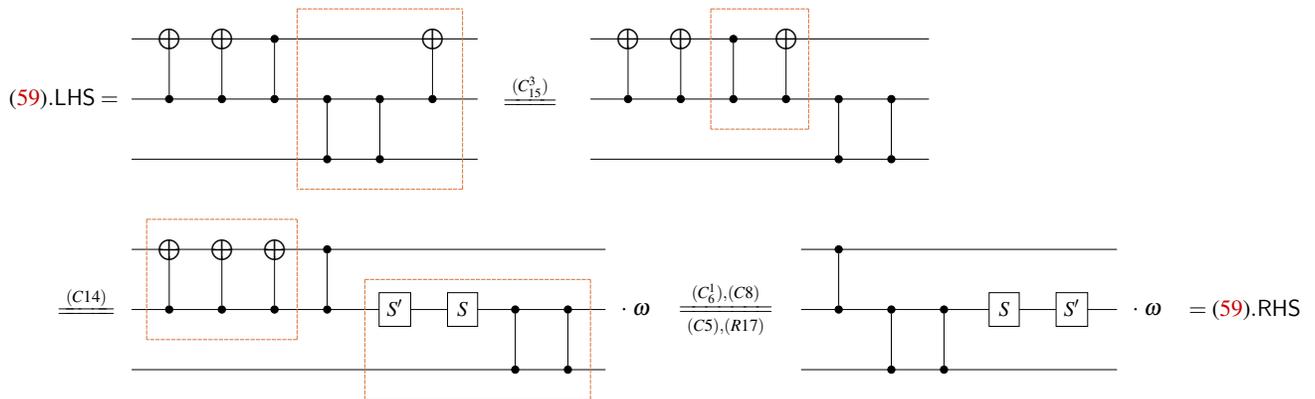

□

To derive (R47) from the equations in Figure 1 and section 1, (61) first simplifies the righthand side of it. Hence, it suffices to show that (60) follows from the equations in Figure 1 and section 1.

(60)

(R47).RHS =  $\cdot \omega^2$

$\xrightarrow{(D3)}$   $\cdot \omega^2$

$\xrightarrow[(D7)]{(C2)}$   $\cdot \omega^2$

$\xrightarrow[(R_{18}^1)]{(C_{13}^{16})}$   $\cdot \omega^2 \cdot \omega$

$\xrightarrow[(C3)]{(D2),(C1)}$   $\cdot \omega^2 \cdot \omega$

$\xrightarrow[(C_9^{20}),(C_9^3)]{(COMMUTE),(COMMUTE^2)}$   $\cdot \omega^2 \cdot \omega$

$\xrightarrow[(C_9^{17})]{(C2)}$

(61)

By (C2), left-appeiding both sides of (60) by  $I \otimes I \otimes H$  yields (62). The detailed derivation is shown below.

(62)

Therefore, we can apply the equations in [Figure 37](#) to show that (62) holds, and this completes the proof.

$(C_9^{3*}), (C_9^{13*}) \iff (C_9^1), (C_9^{22}), (C2), (D7)$   
 $(C2) \iff (C_{18}^{75})$   
 $(C6^*) \iff (C_{18}^{41})$   
 $(C15) \iff (C_{18}^{93})$   
 $(C6) \iff (C_6^1)$

**Lemma 4.33.** (R48) and (R49) follow from the reduced relations.

(R48)

(R49)

*Proof.* First, (67) simplifies the righthand side of (R48), so it suffices to derive (63) from the equations in Figure 1 and section 1.

(63)

Next, (68) simplifies the lefthand side of (63), so it suffices to derive (64) from the equations in Figure 1 and section 1.

(64)

By (C2), right-appending both sides of (64) by  $I \otimes H^2 \otimes I$  yields (65).

(65)

By (D7), left-appending both sides of (65) by  $I \otimes I \otimes H$  yields (66).

(66)

Finally, (69) simplifies both sides of (66) using the rewrite rules listed in Figure 1 and section 1. Since the lefthand side is simplified to exactly match the righthand side, the proof is complete.

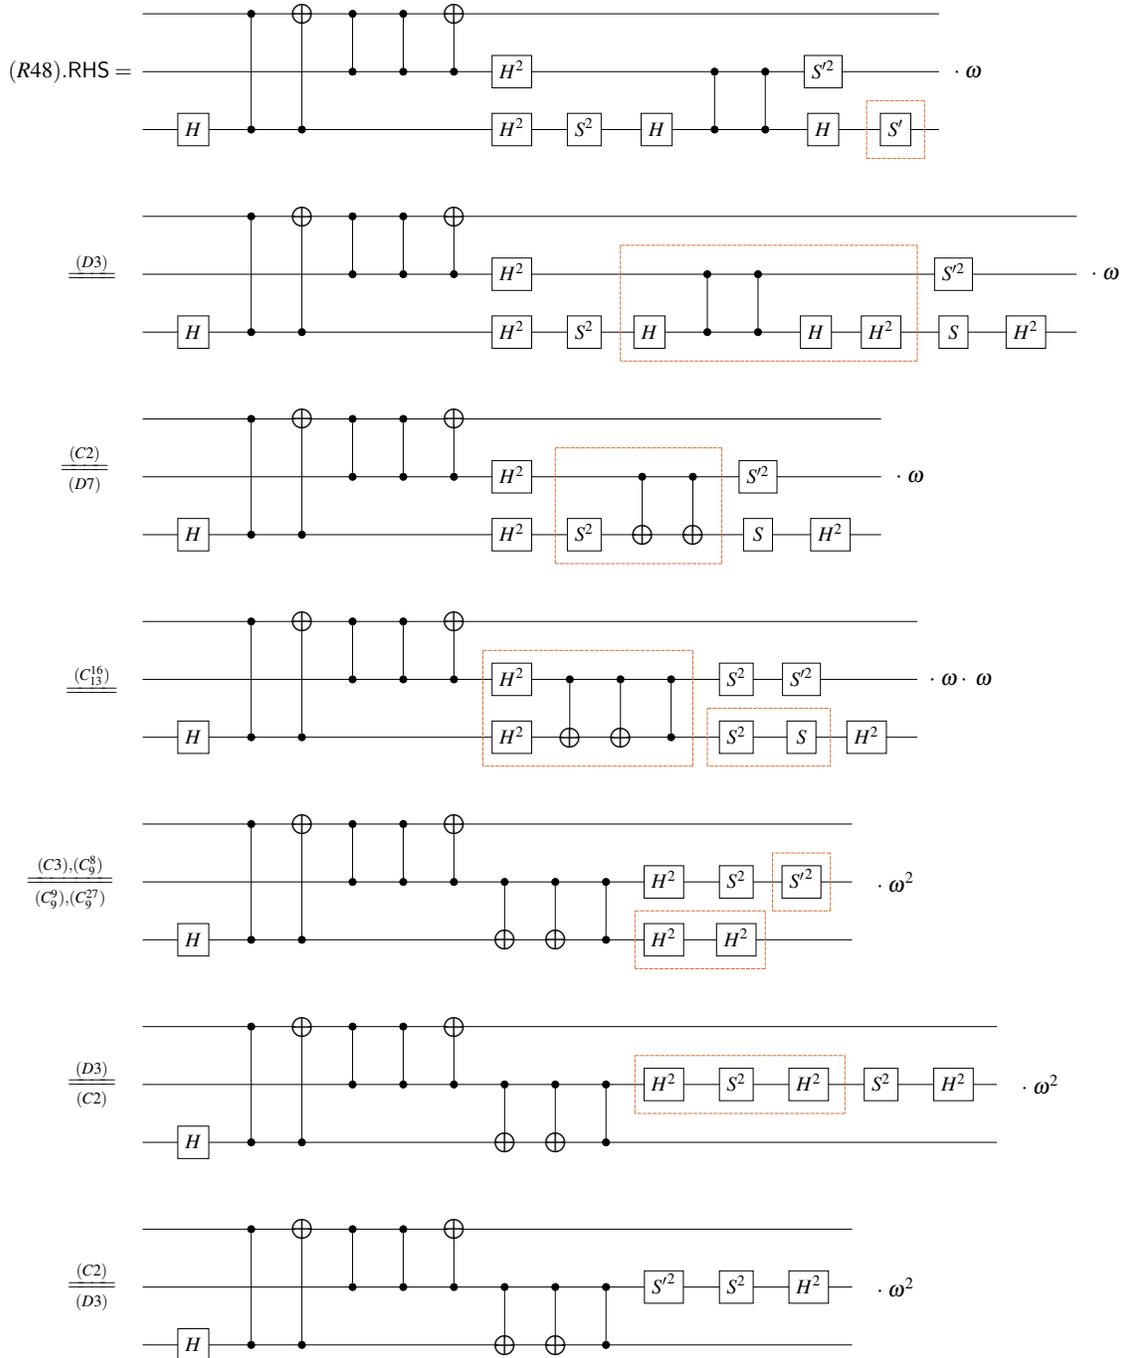

(67)

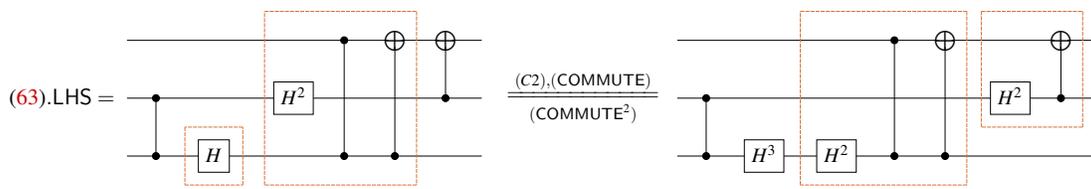

(68)

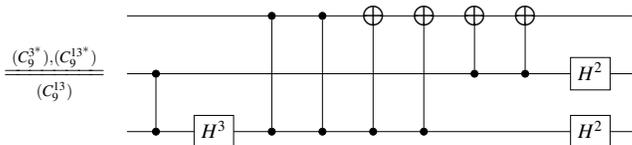

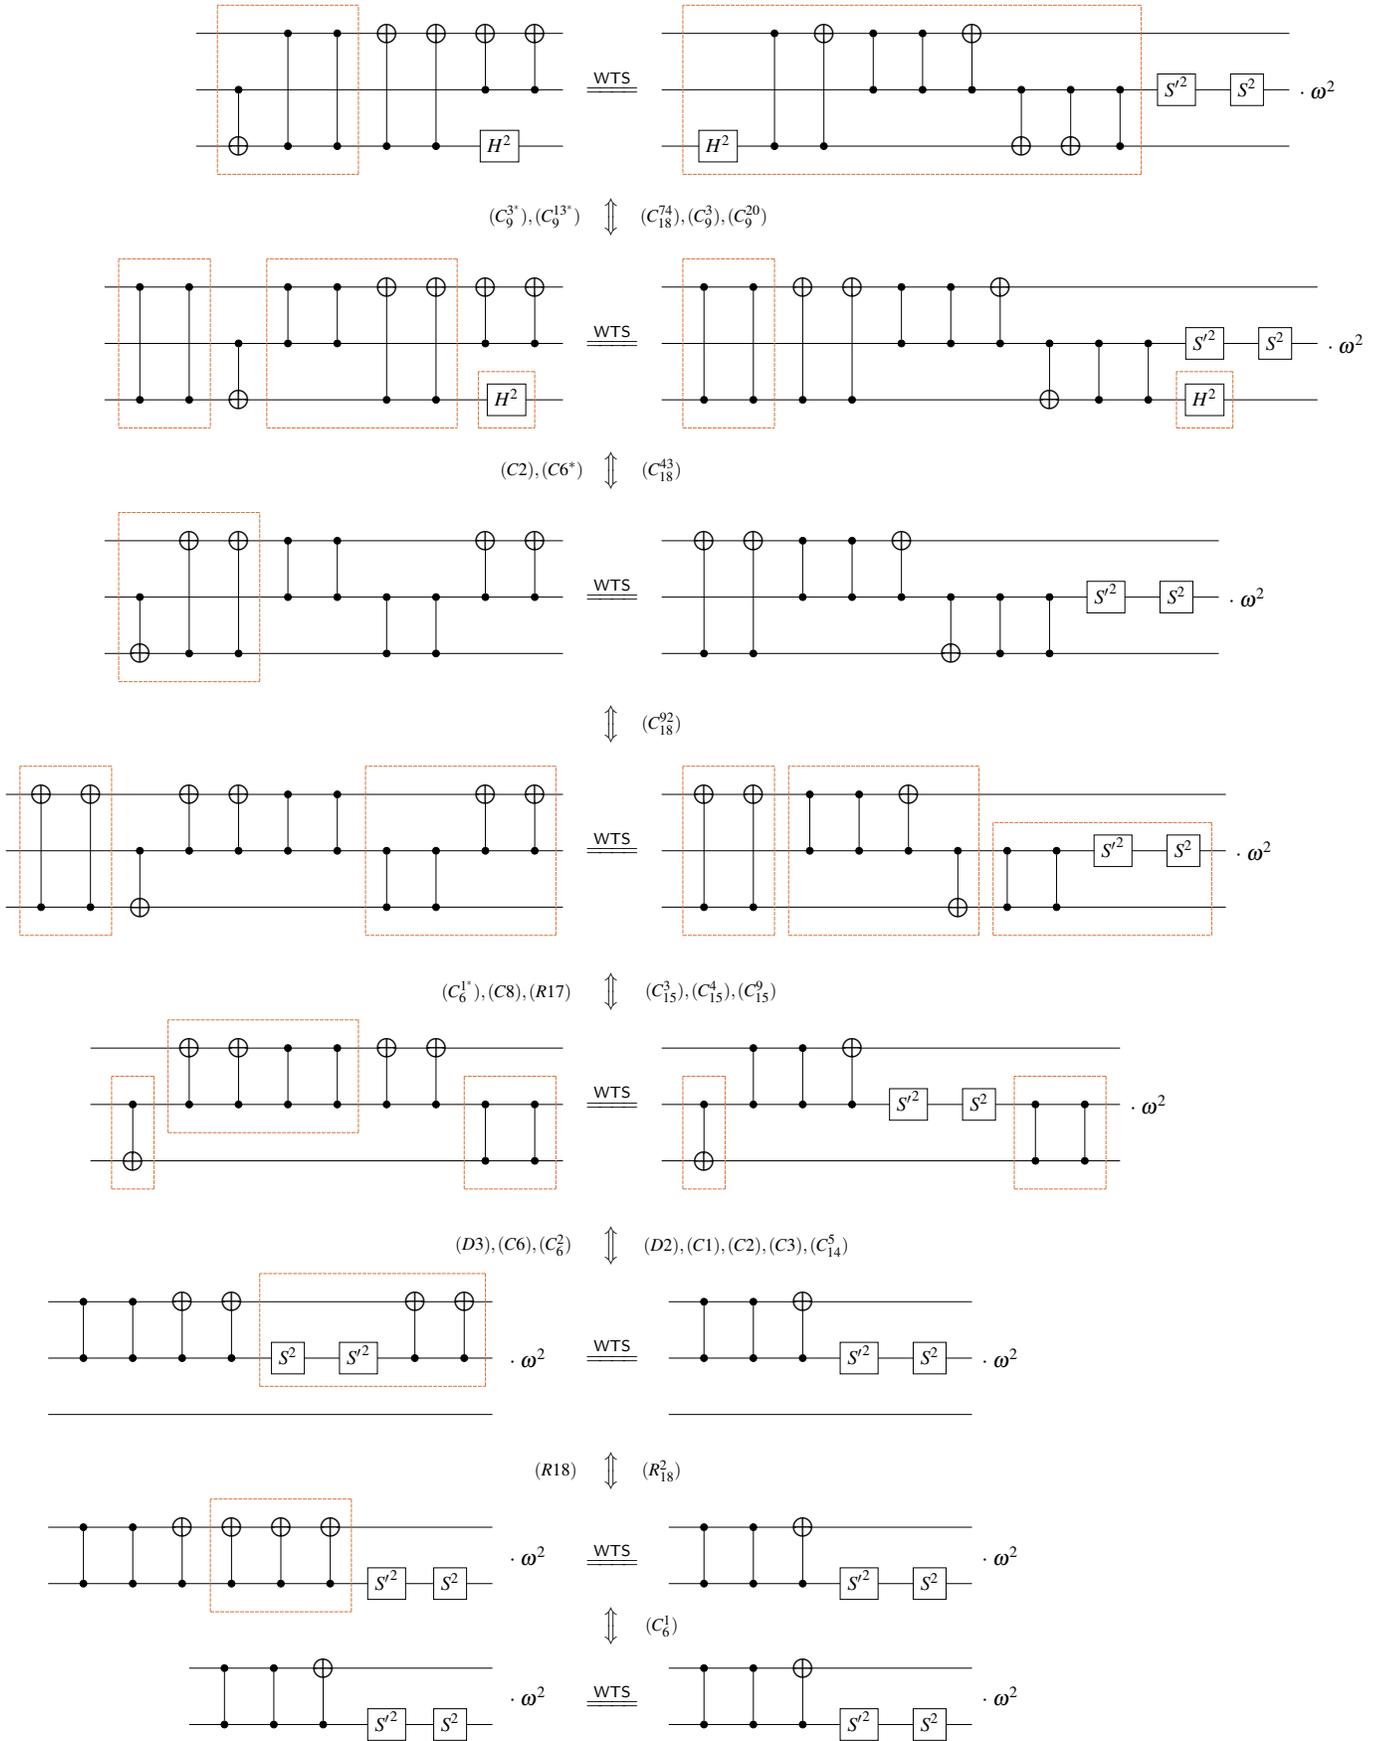

To derive (R49) from the equations in Figure 1 and section 1, (71) first simplifies the righthand side of it. Hence, it suffices to show that (70) follows from the equations in Figure 1 and section 1.

(70)

(R49).RHS =

(71)

By (C2), left-appending both sides of (70) by  $I \otimes I \otimes H$  yields (72). It simplifies both sides of (70) using the rewrite rules listed in Figure 1 and section 1. Since the lefthand side is simplified to exactly match the righthand side, the proof is complete.

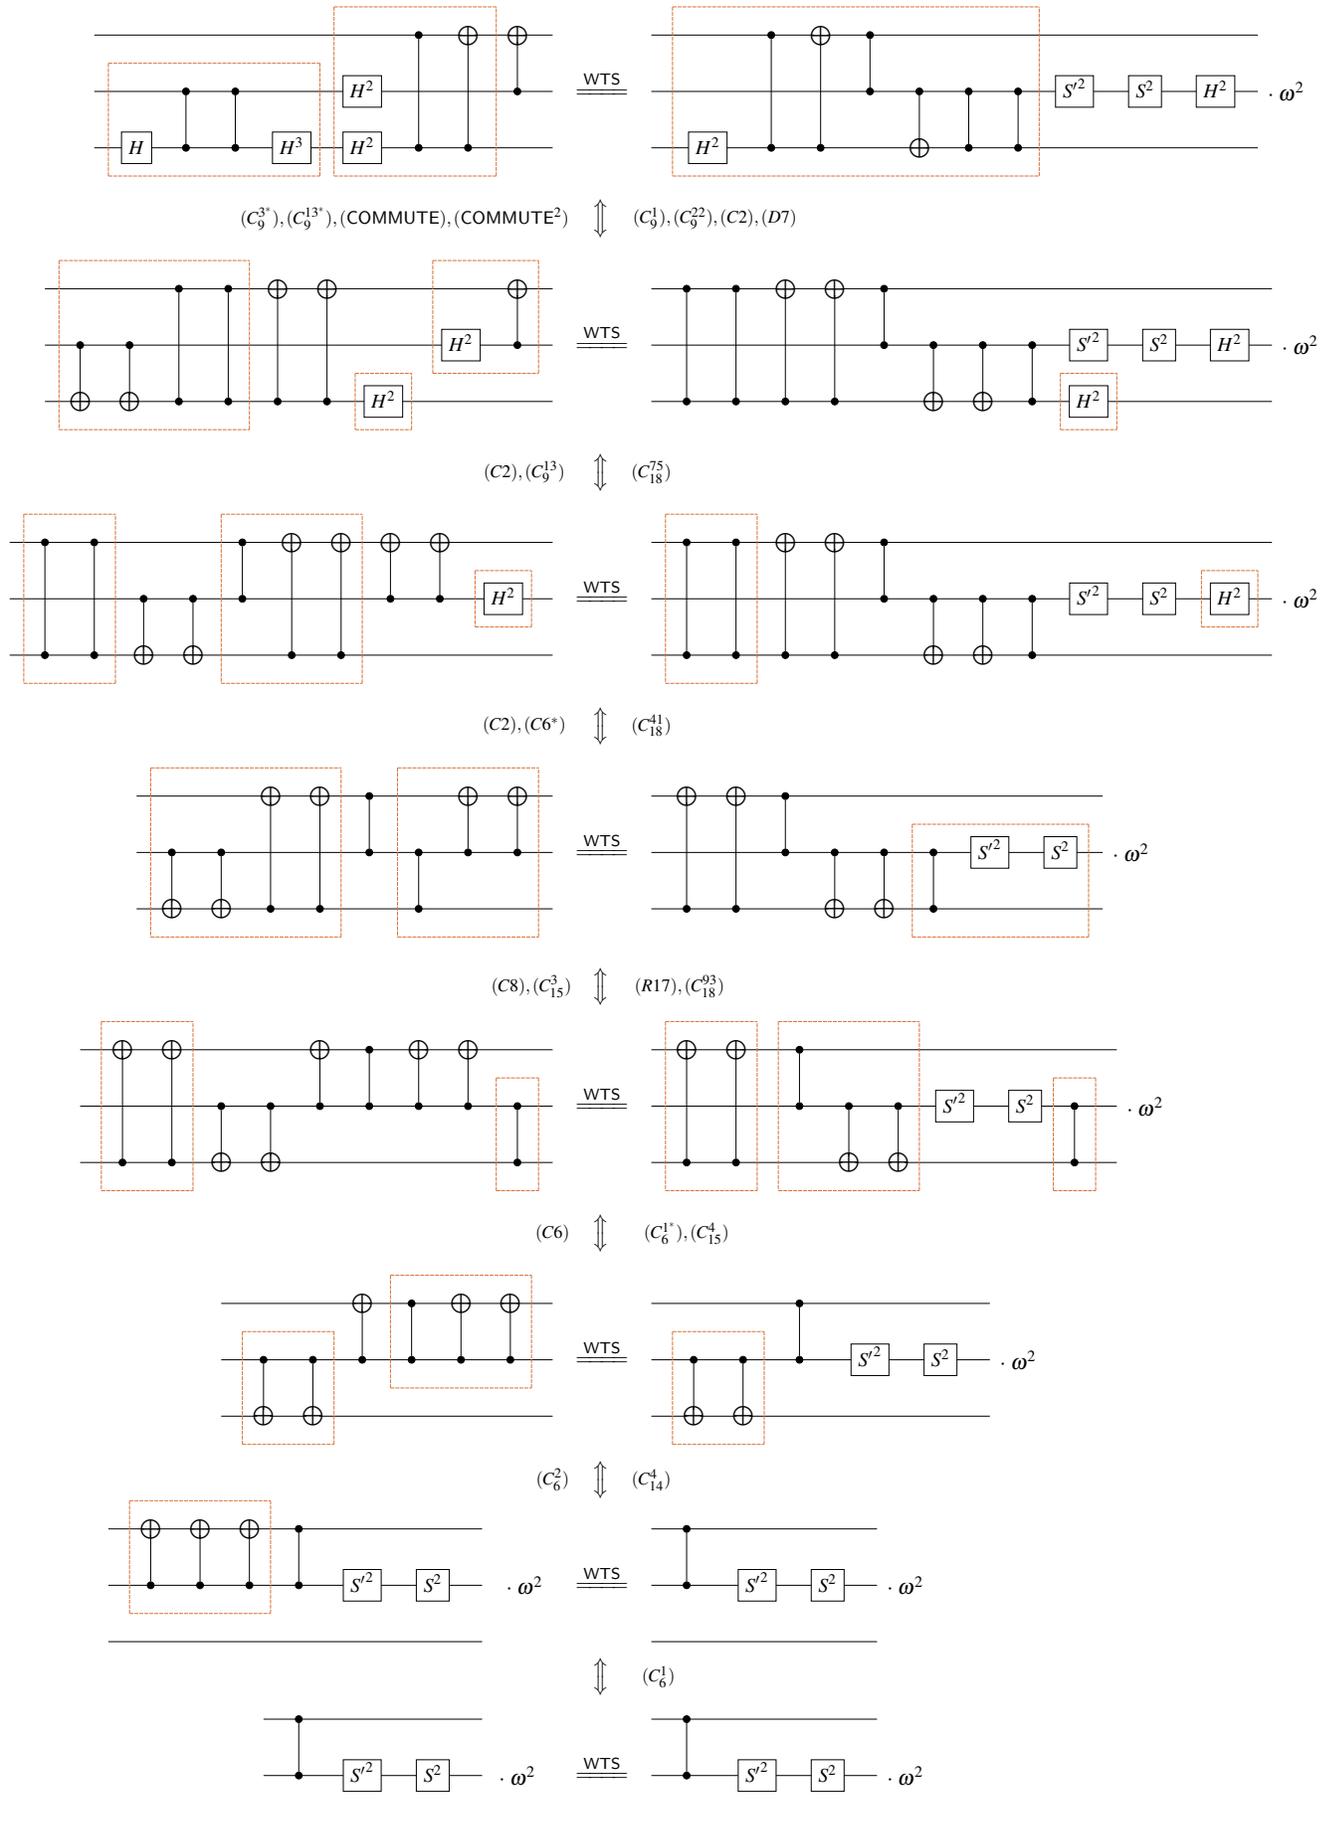

**Lemma 4.34.** (R50) and (R51) follow from the reduced relations.

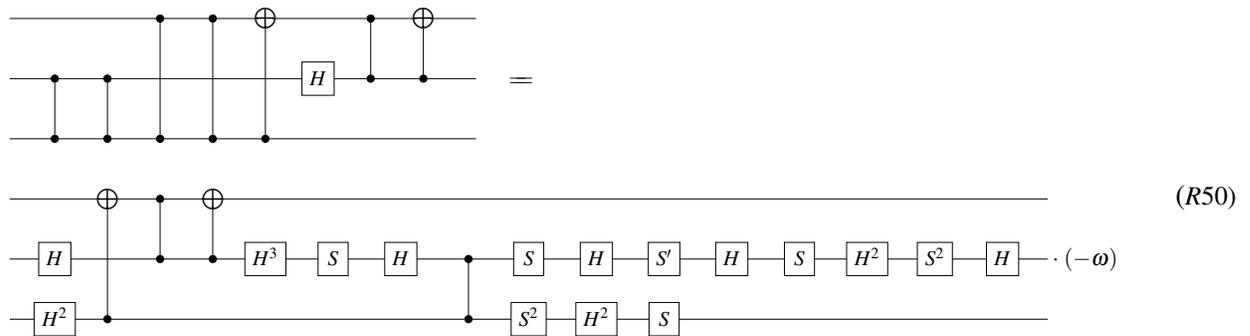

(R50)

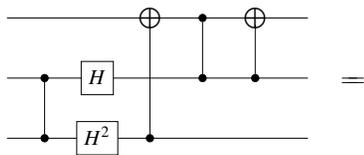

(R51)

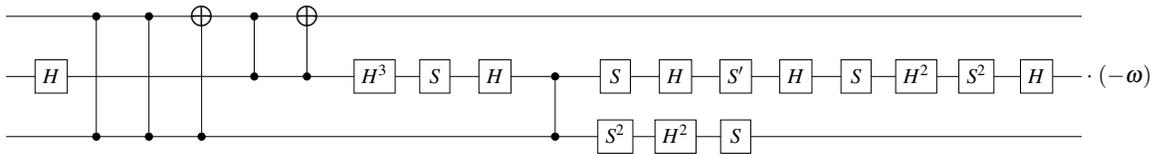

*Proof.* First note that

$$SHS'SHS \stackrel{(D3)}{=} SH(H^2SH^2)HS \stackrel{(C_4)}{=} (HS^2H)H^3S \cdot (-\omega^2) \stackrel{(C2)}{=} HS^2S \cdot (-\omega^2) \stackrel{(C3)}{=} H \cdot (-\omega^2). \quad (73)$$

Then, (77) simplifies the righthand side of (R50), so it suffices to derive (74) from the equations in Figure 1 and section 1.

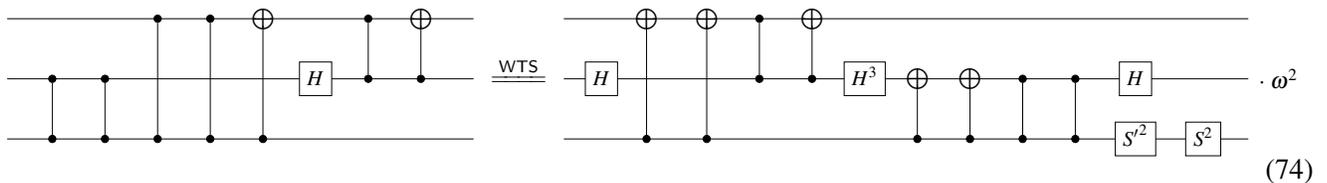

(74)

By (C2), left-appepending both sides of (74) by  $I \otimes H \otimes I$  yields (76). Hence, it suffices to derive (75).

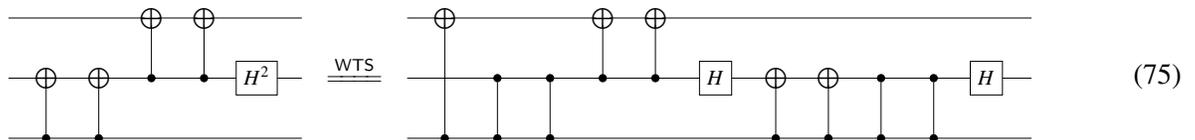

(75)

Finally, (78) shows how to reduce the righthand side of (75) to its lefthand side using the rewrite rules listed in Figure 1 and section 1. This completes the proof.

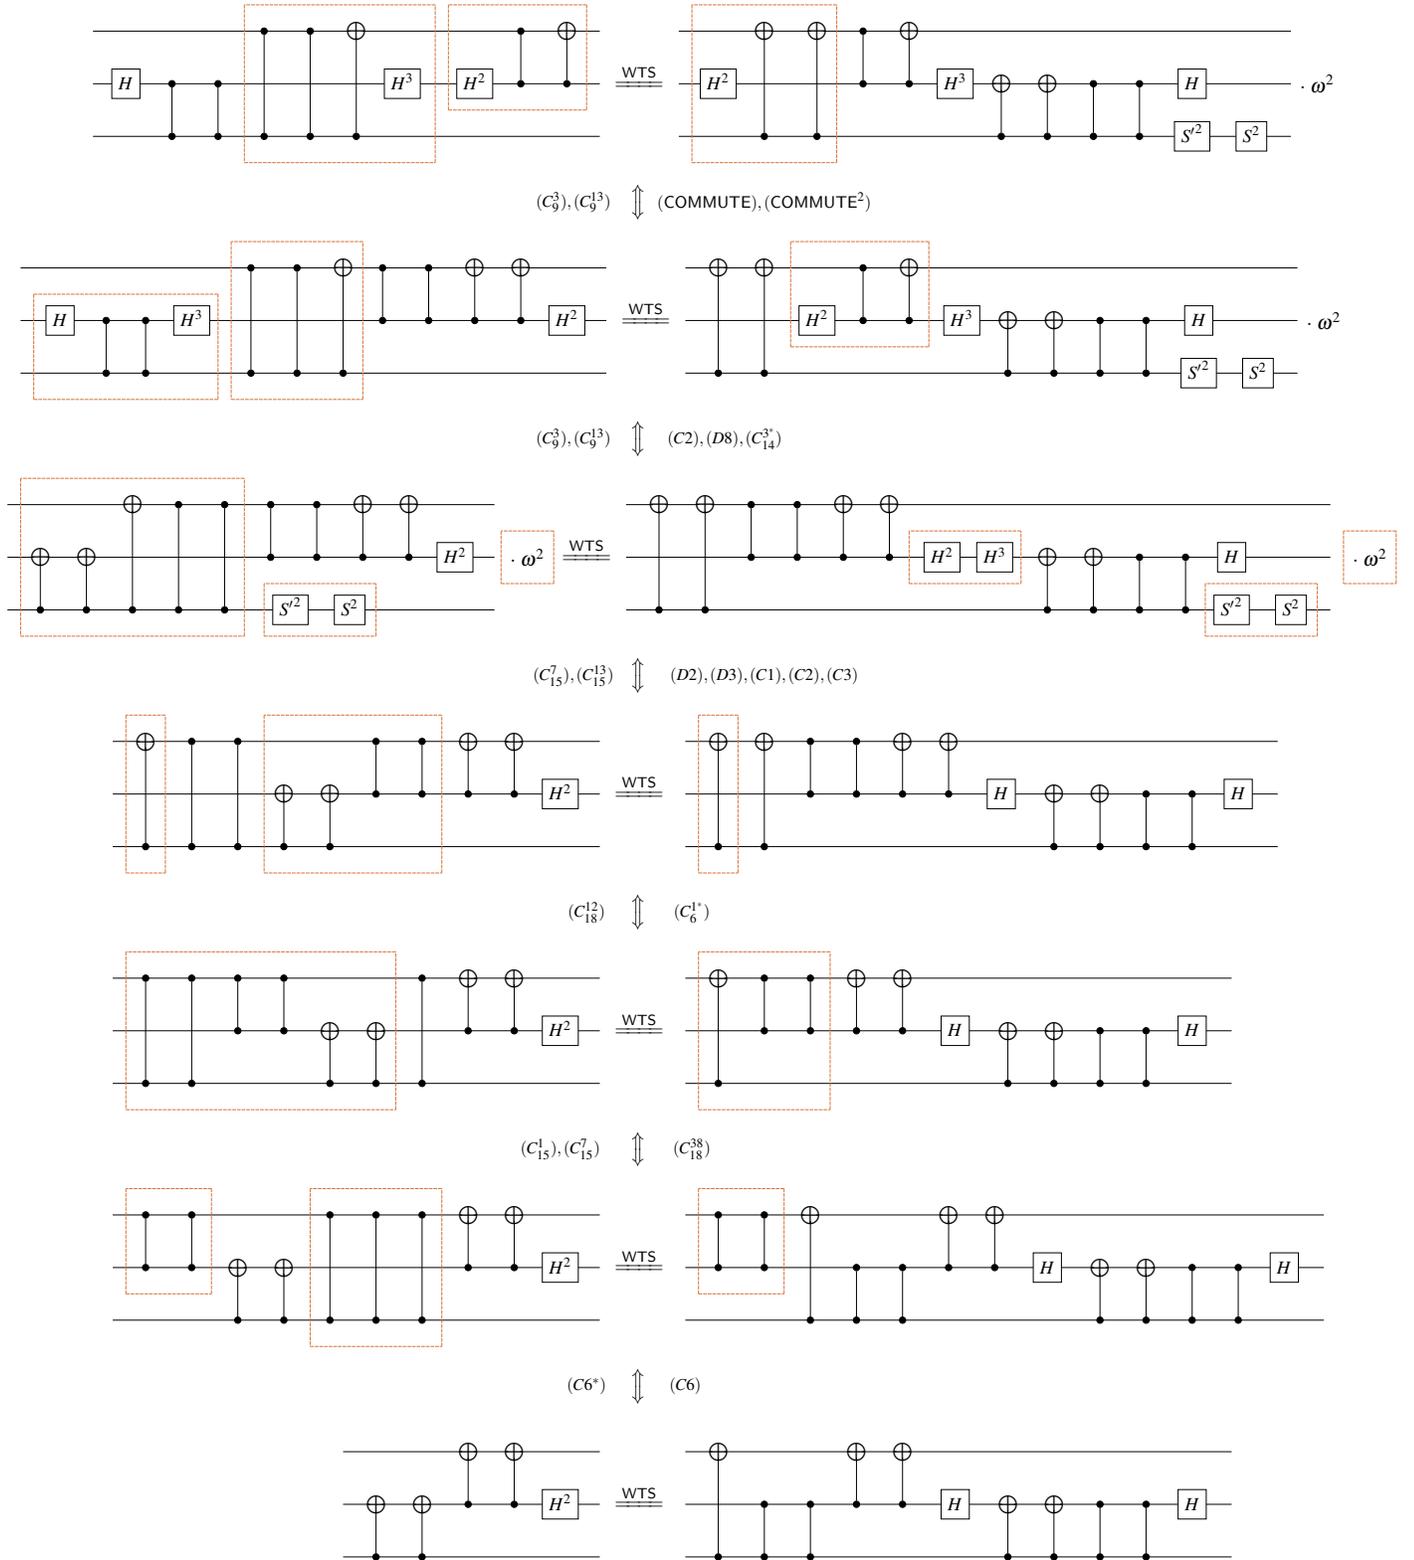

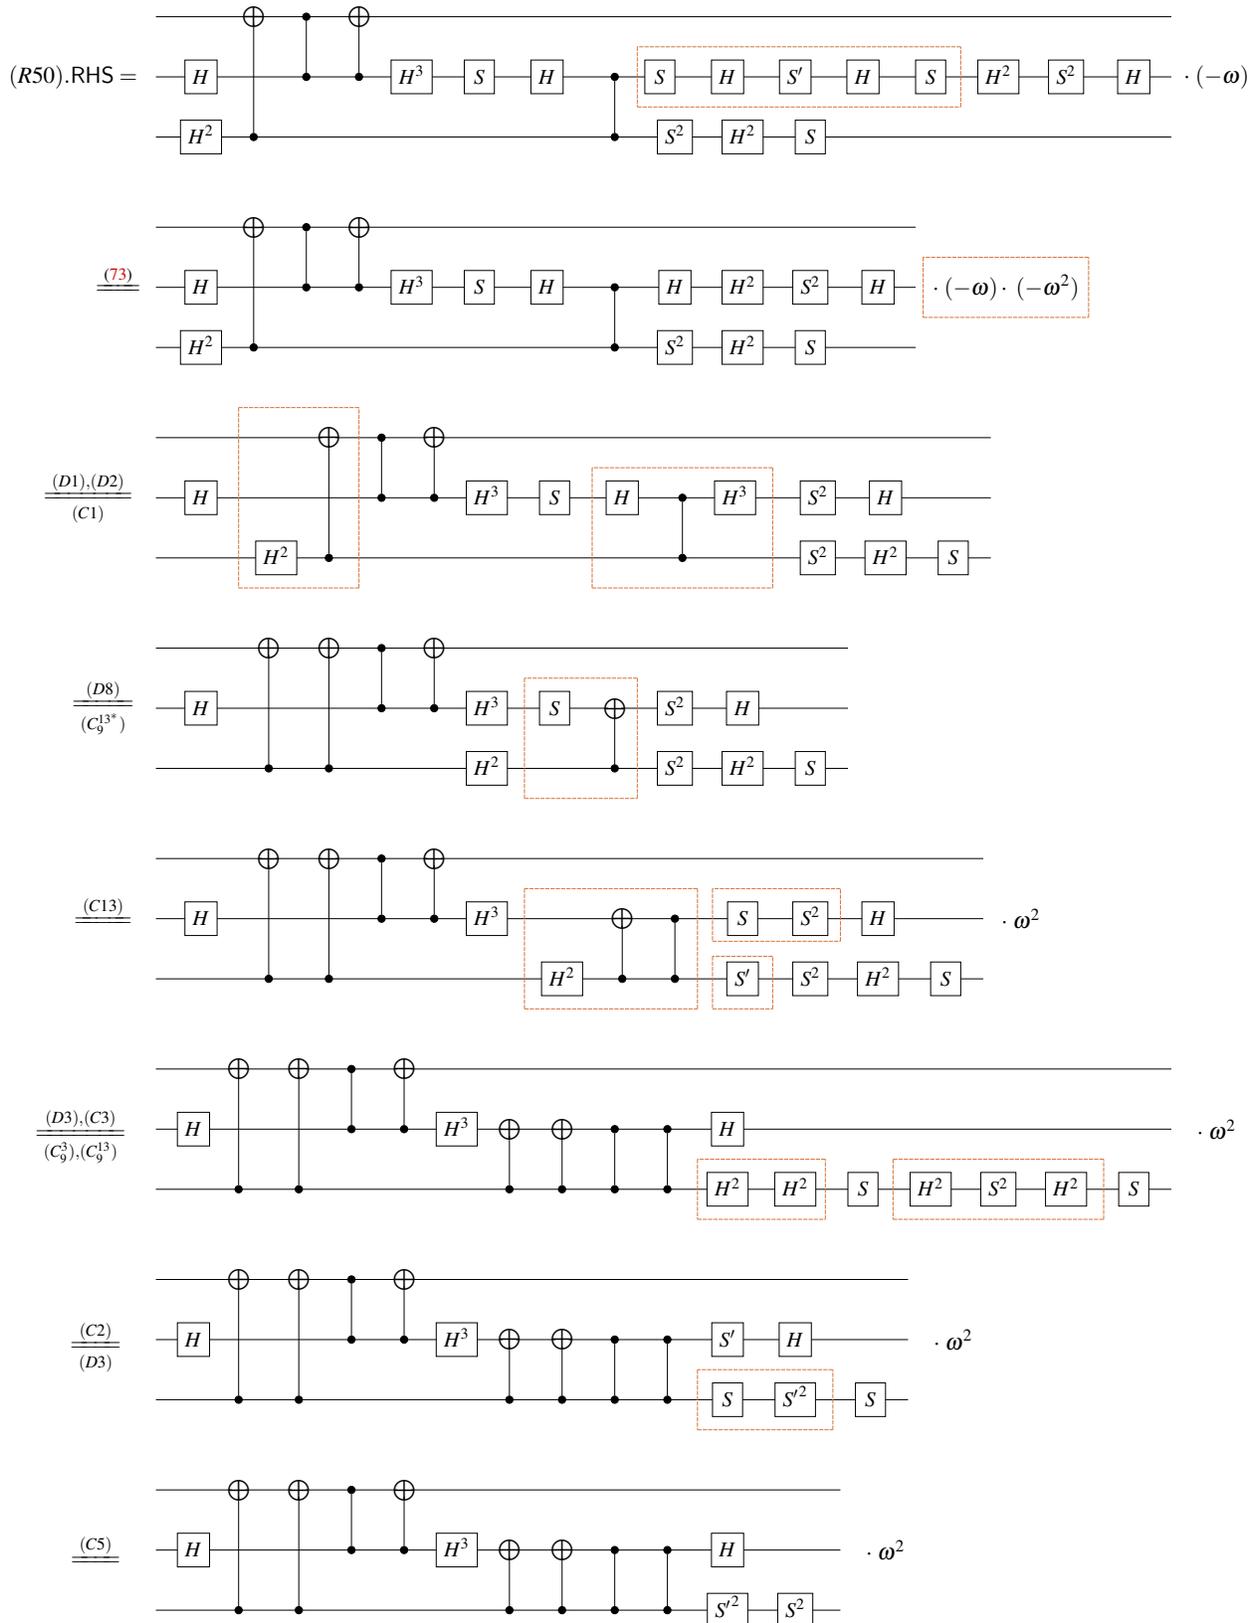

(75).RHS =

$\frac{(C2)}{(D8)}$

$\frac{(C9)}{(C2)}$

$\frac{(C_{15}^3)}{(C2)}$

$\frac{(C6),(D8)}{(C2)}$   $\frac{(C_{13}^{13}), (C_{15}^{13})}{(C_{18}^{30})}$  = (75).LHS

(78)

To derive (R51) from the equations in Figure 1 and section 1, (81) first simplifies the righthand side of it. Hence, it suffices to show that (79) follows from the equations in Figure 1 and section 1.

$\stackrel{WTS}{=} \cdot \omega^2$  (79)

By (C2), left-appending both sides of (79) by  $I \otimes H \otimes I$  yields (82). Hence, it suffices to derive (80).

(80)

Finally, (83) shows how to reduce the lefthand side of (80) to its righthand side using the rewrite rules listed in

Figure 1 and section 1. This completes the proof.

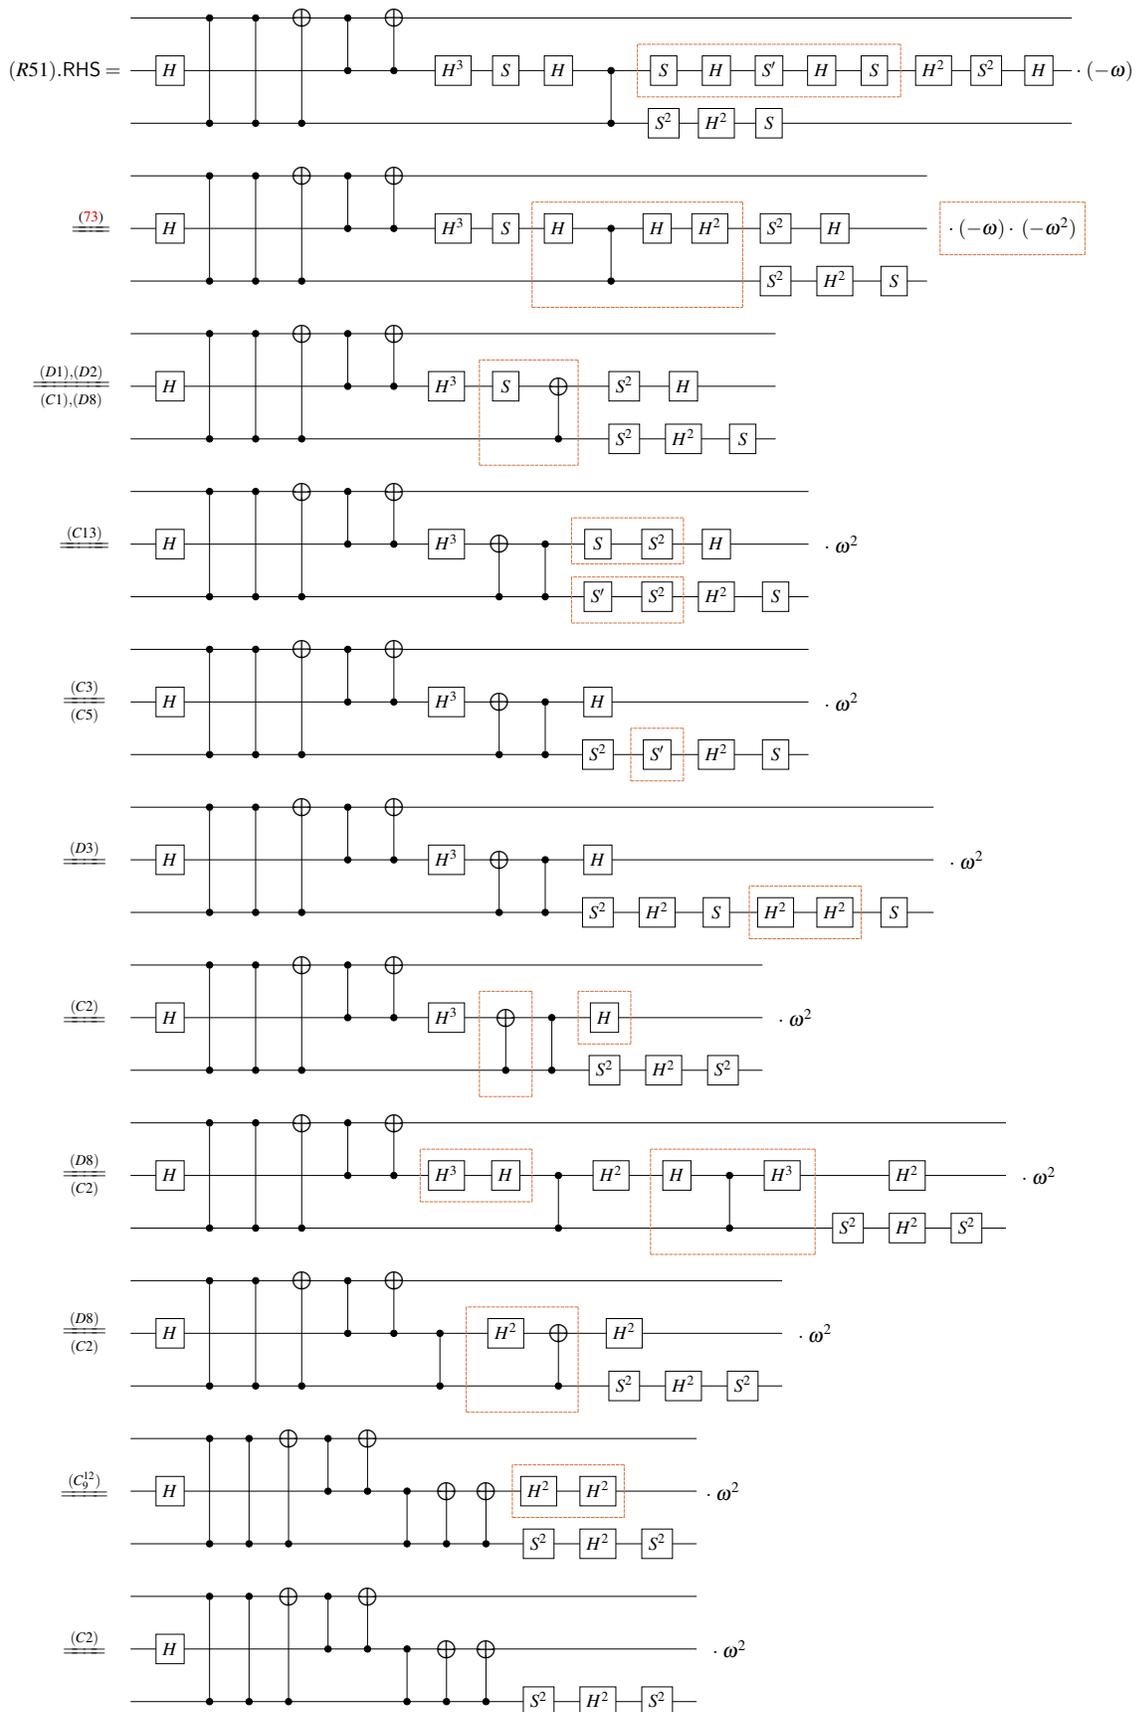

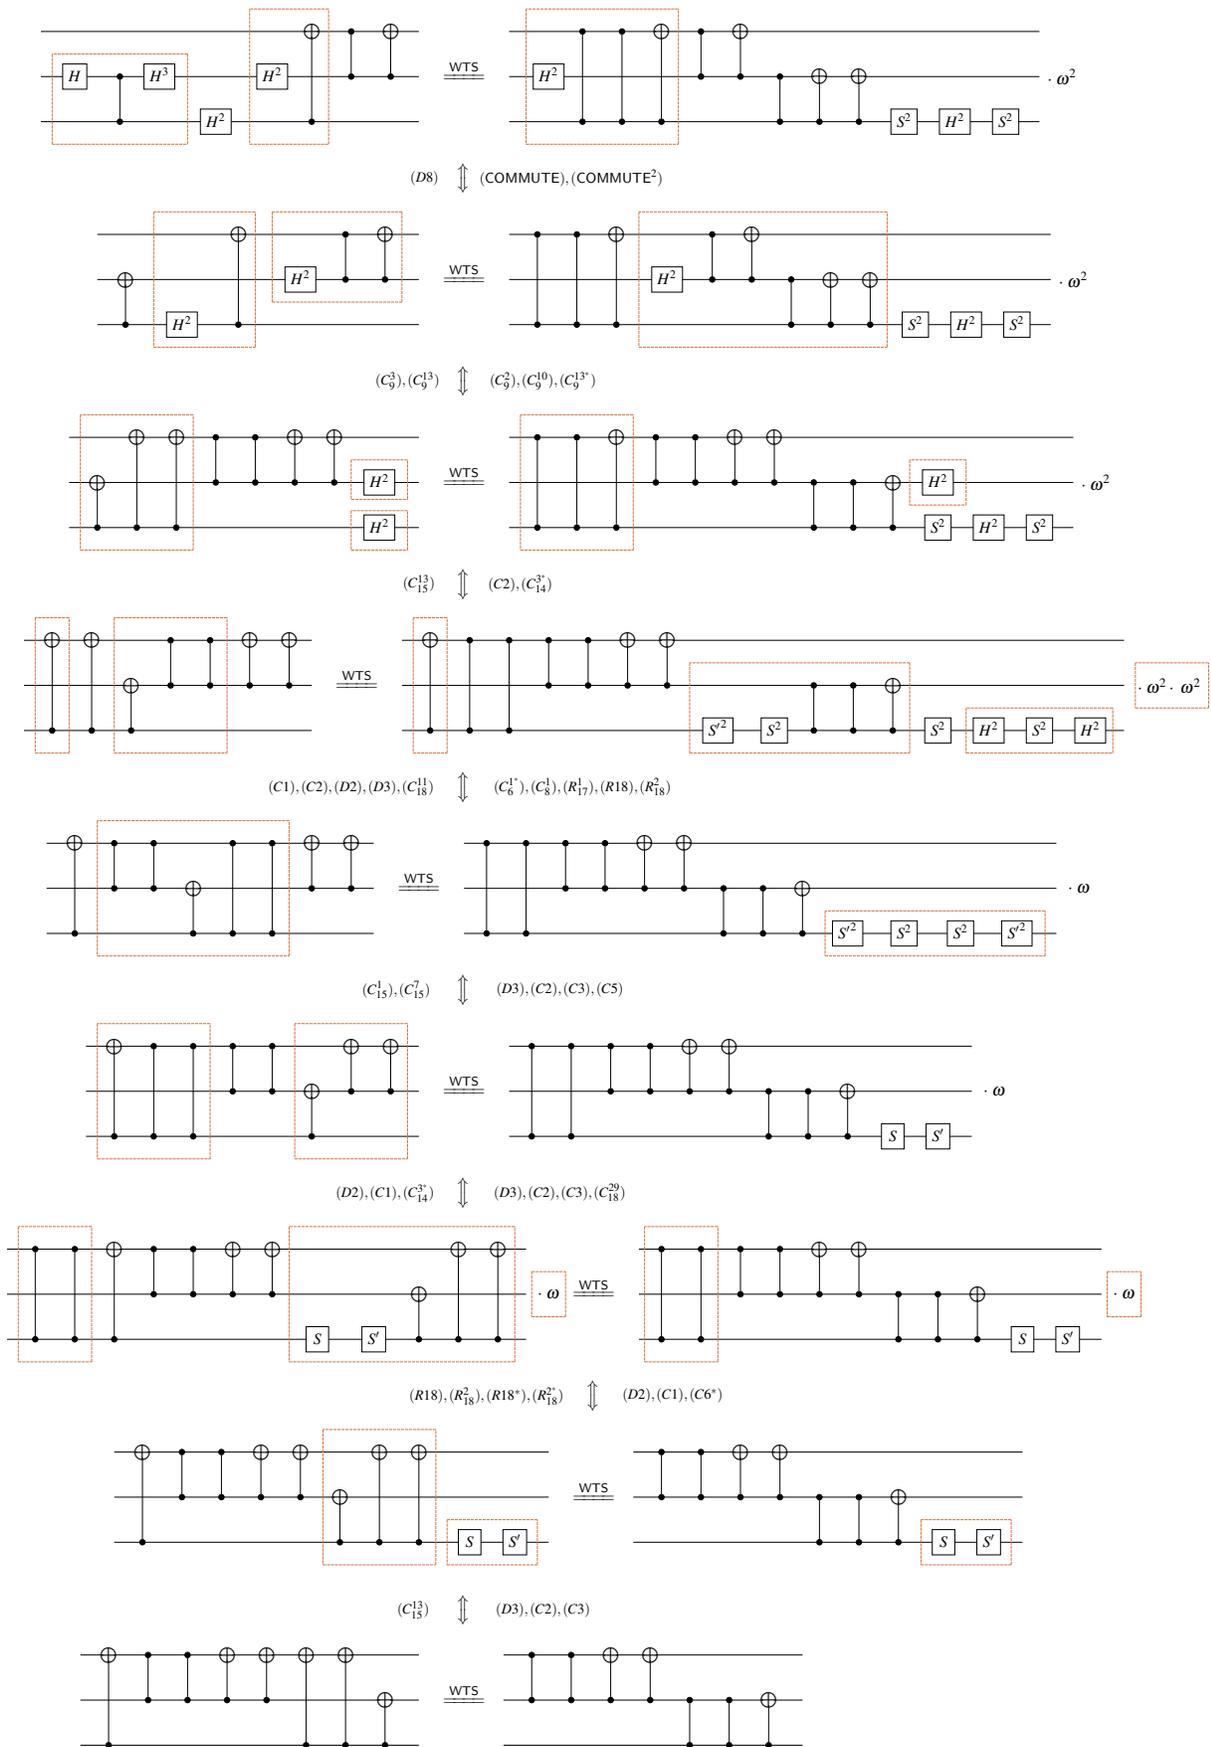

(82)

(80).LHS = 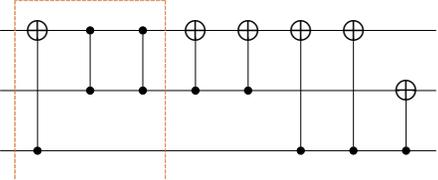  $\xrightarrow{(C_{18}^{38})}$  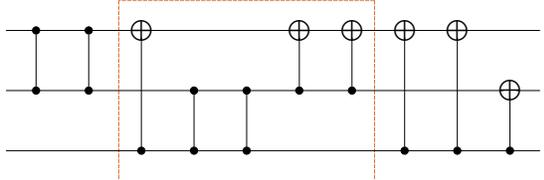  $\xrightarrow[\substack{(C_{15}^8), (C_{15}^{12}) \\ (C_{15}^3)}]{(C_6^{1*})}$  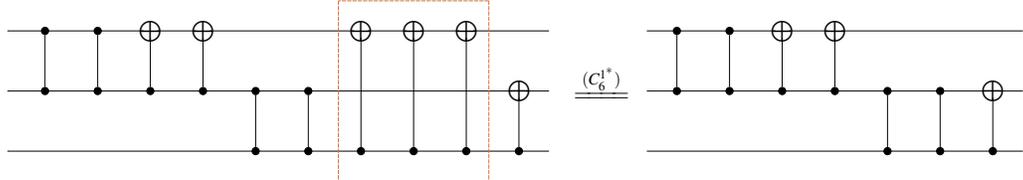 = (80).RHS

(83) □

**Lemma 4.35.** (R52) follows from the reduced relations.

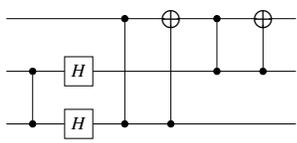 = 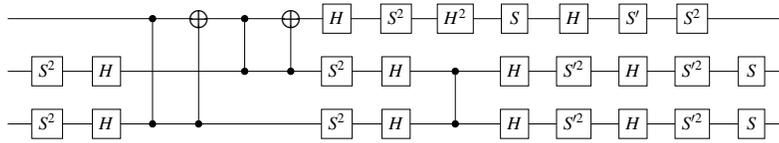  $\cdot \omega$  (R52)

*Proof.* First note that

$$HS^2H^2SHS'S^2 \xrightarrow{(R5)} (HS^2H^2SH)Z^2 \xrightarrow{(R2)} X^2Z^2. \tag{84}$$

Then, (88) simplifies the righthand side of (R52), so it suffices to derive (85) from the equations in Figure 1 and section 1.

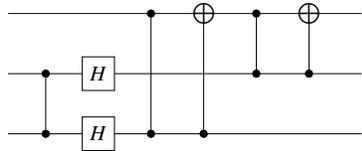  $\xrightarrow{WTS}$  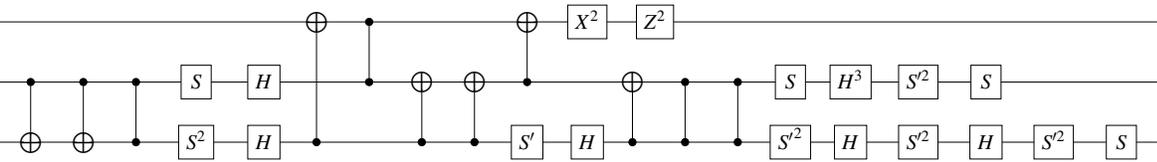  $\cdot \omega$  (85)

Note also that

$$S'^2 (HS'^2H) S'^2 S \xrightarrow[\substack{(D1), (D2)}]{(C1), (C_4^3)} (S'^2 S') H^3 (S' S'^2) S \cdot (-\omega) \xrightarrow[\substack{(D3), (C2)}]{(C3)} H^3 S \cdot (-\omega). \tag{86}$$

By (D1), (D2), and (C1), (89) simplifies the righthand side of (85). Hence, it suffices to derive (87).

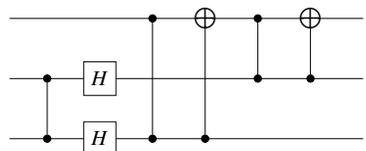  $\xrightarrow{WTS}$  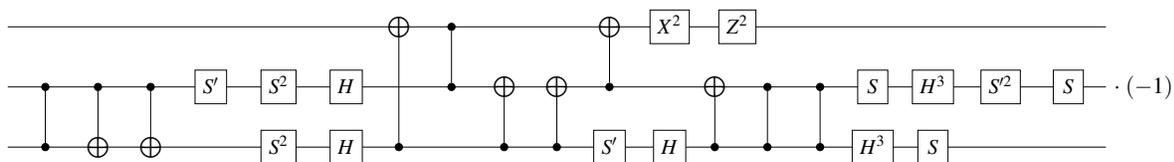  $\cdot (-1)$  (87)

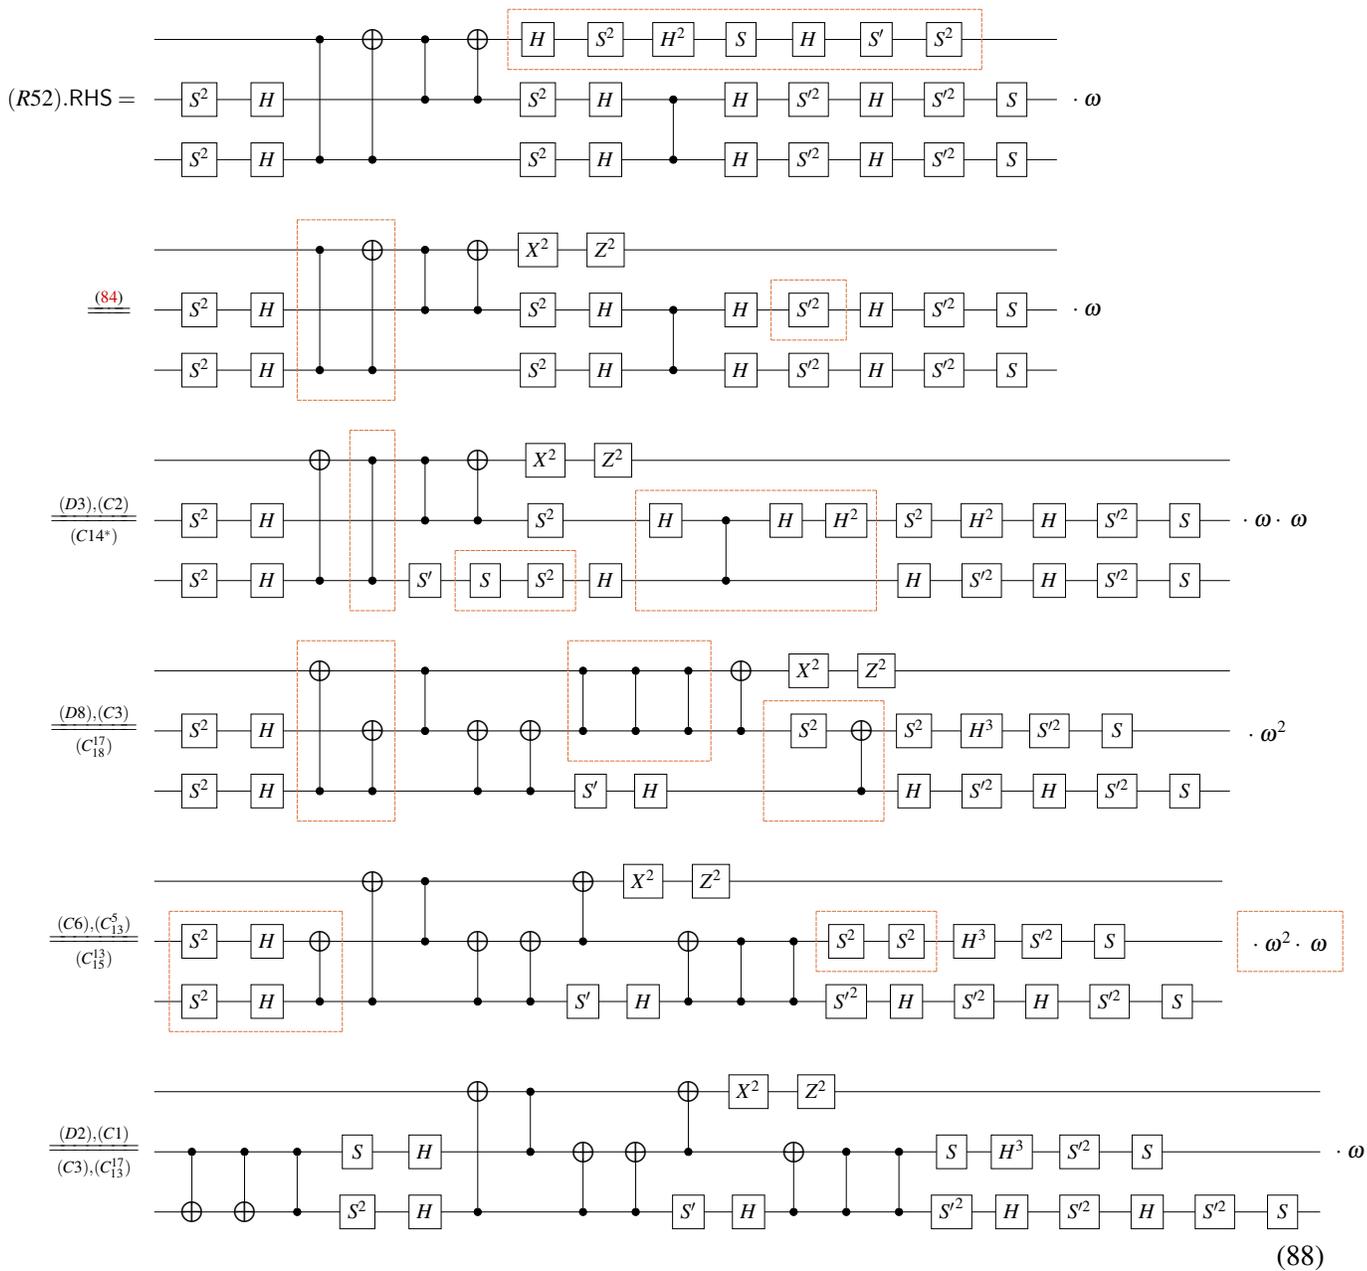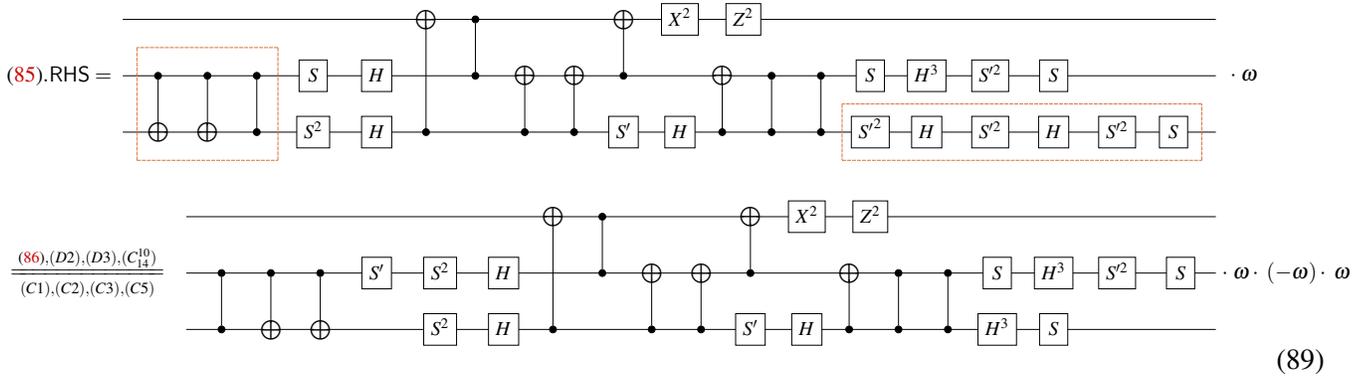

By (C6), left-appepending both sides of (87) by  $I \otimes CZ^2$  yields (90).

Then, (96), (97), and (98) simplify the righthand side of (90). Therefore, it suffices to derive (91) from the equations in Figure 1 and section 1.

By (C2), left-appepending both sides of (91) by  $I \otimes H^3 \otimes H^3$  yields (92).

Based on this, (99) simplifies both sides of (92), so our problem is reduced to showing (93).

Then, (100) and (101) simplify the righthand side of (93), bringing it one step closer to its lefthand side. Note that

$$(S'^2 S) X^2 Z^2 \stackrel{(R4)}{=} (Z X^2) Z^2 \stackrel{(R12)}{=} X^2 (Z Z^2) \cdot (\omega^2)^2 \stackrel{(D2),(C1)}{\stackrel{(R6)}{=} } X^2 \cdot \omega. \tag{94}$$

By (D1), (D2), and (C1), it suffices to show that

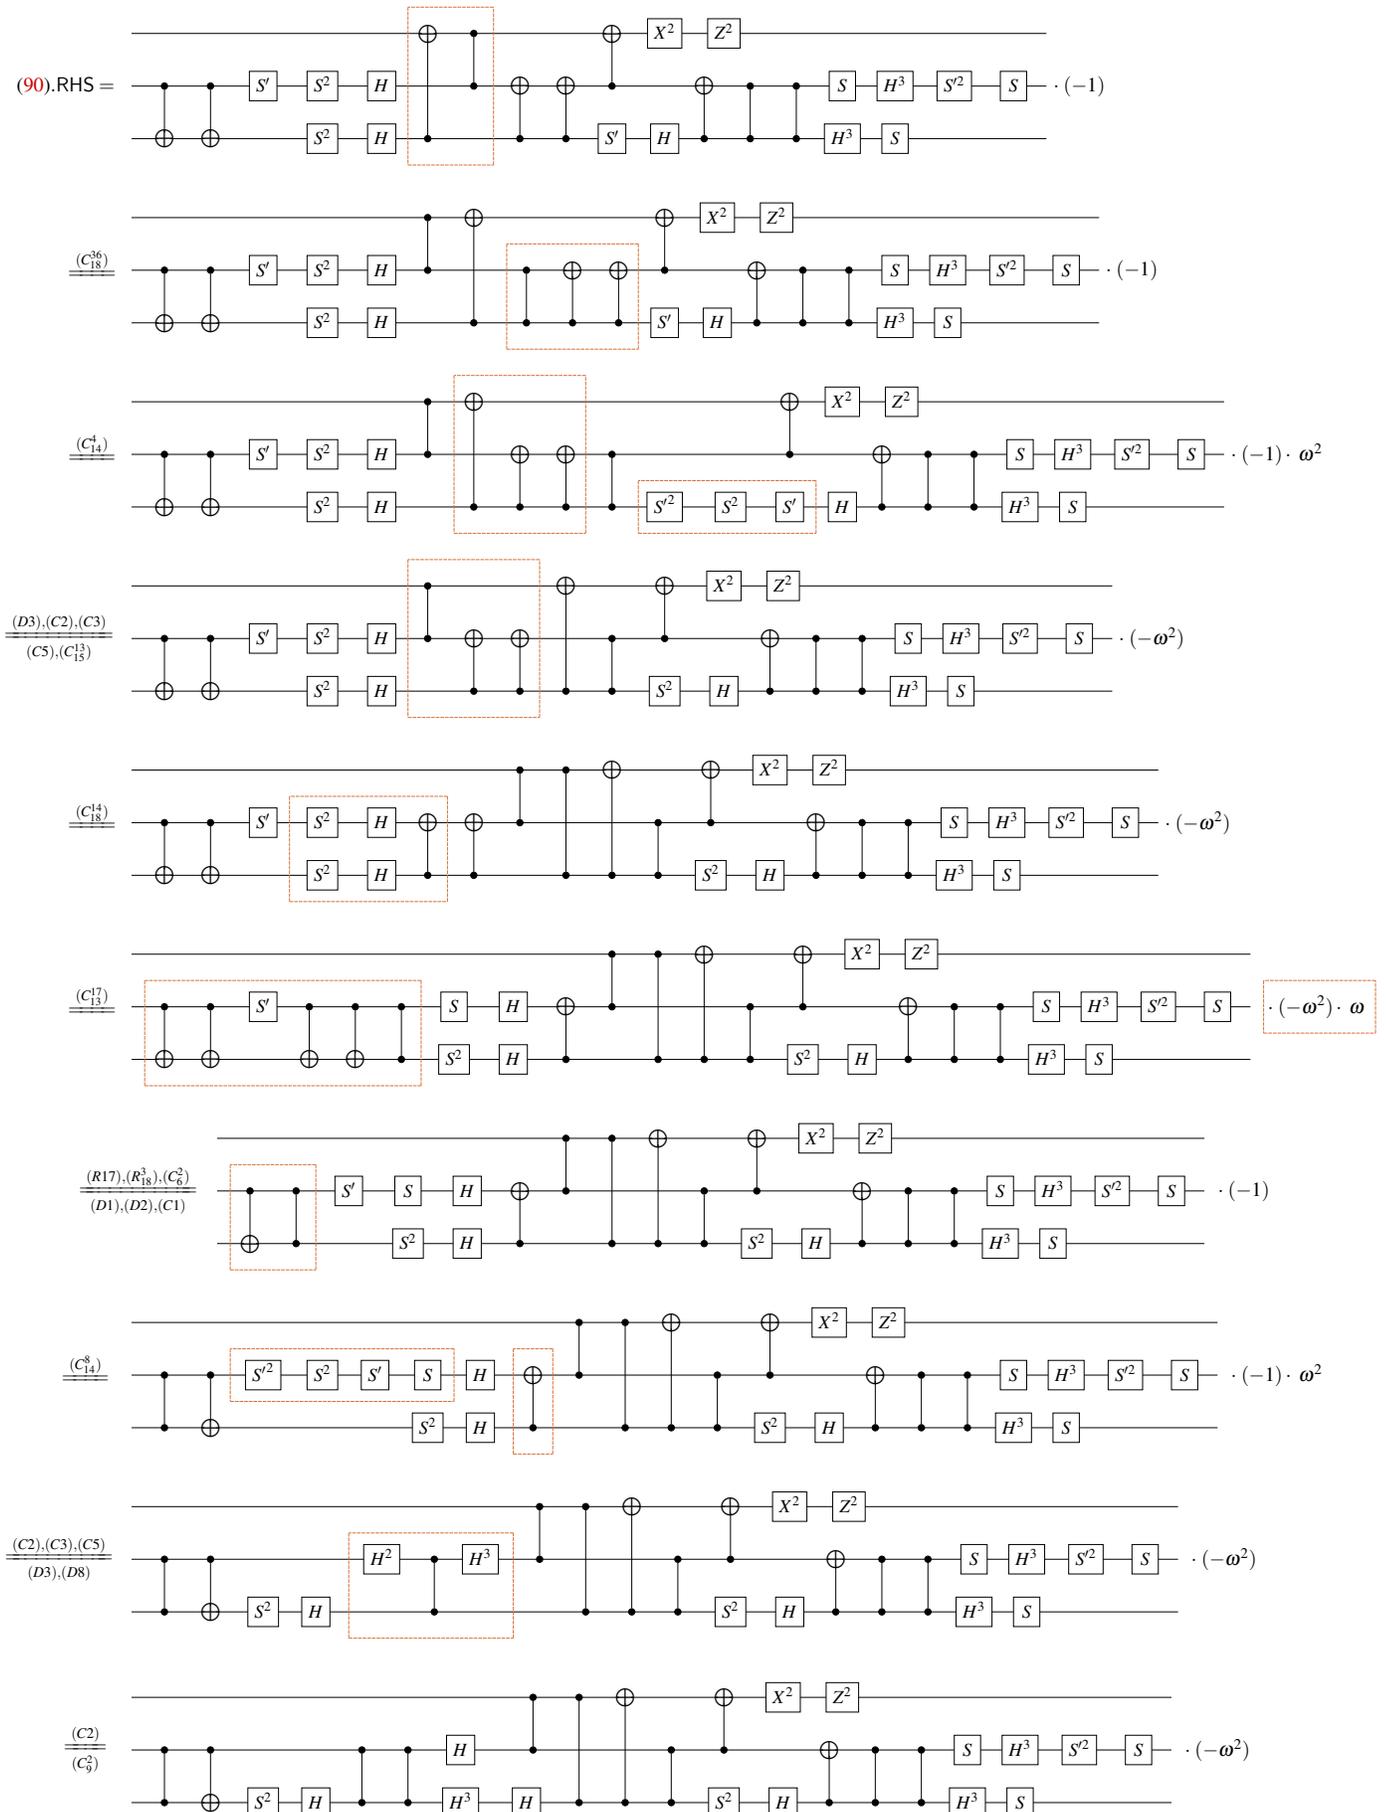

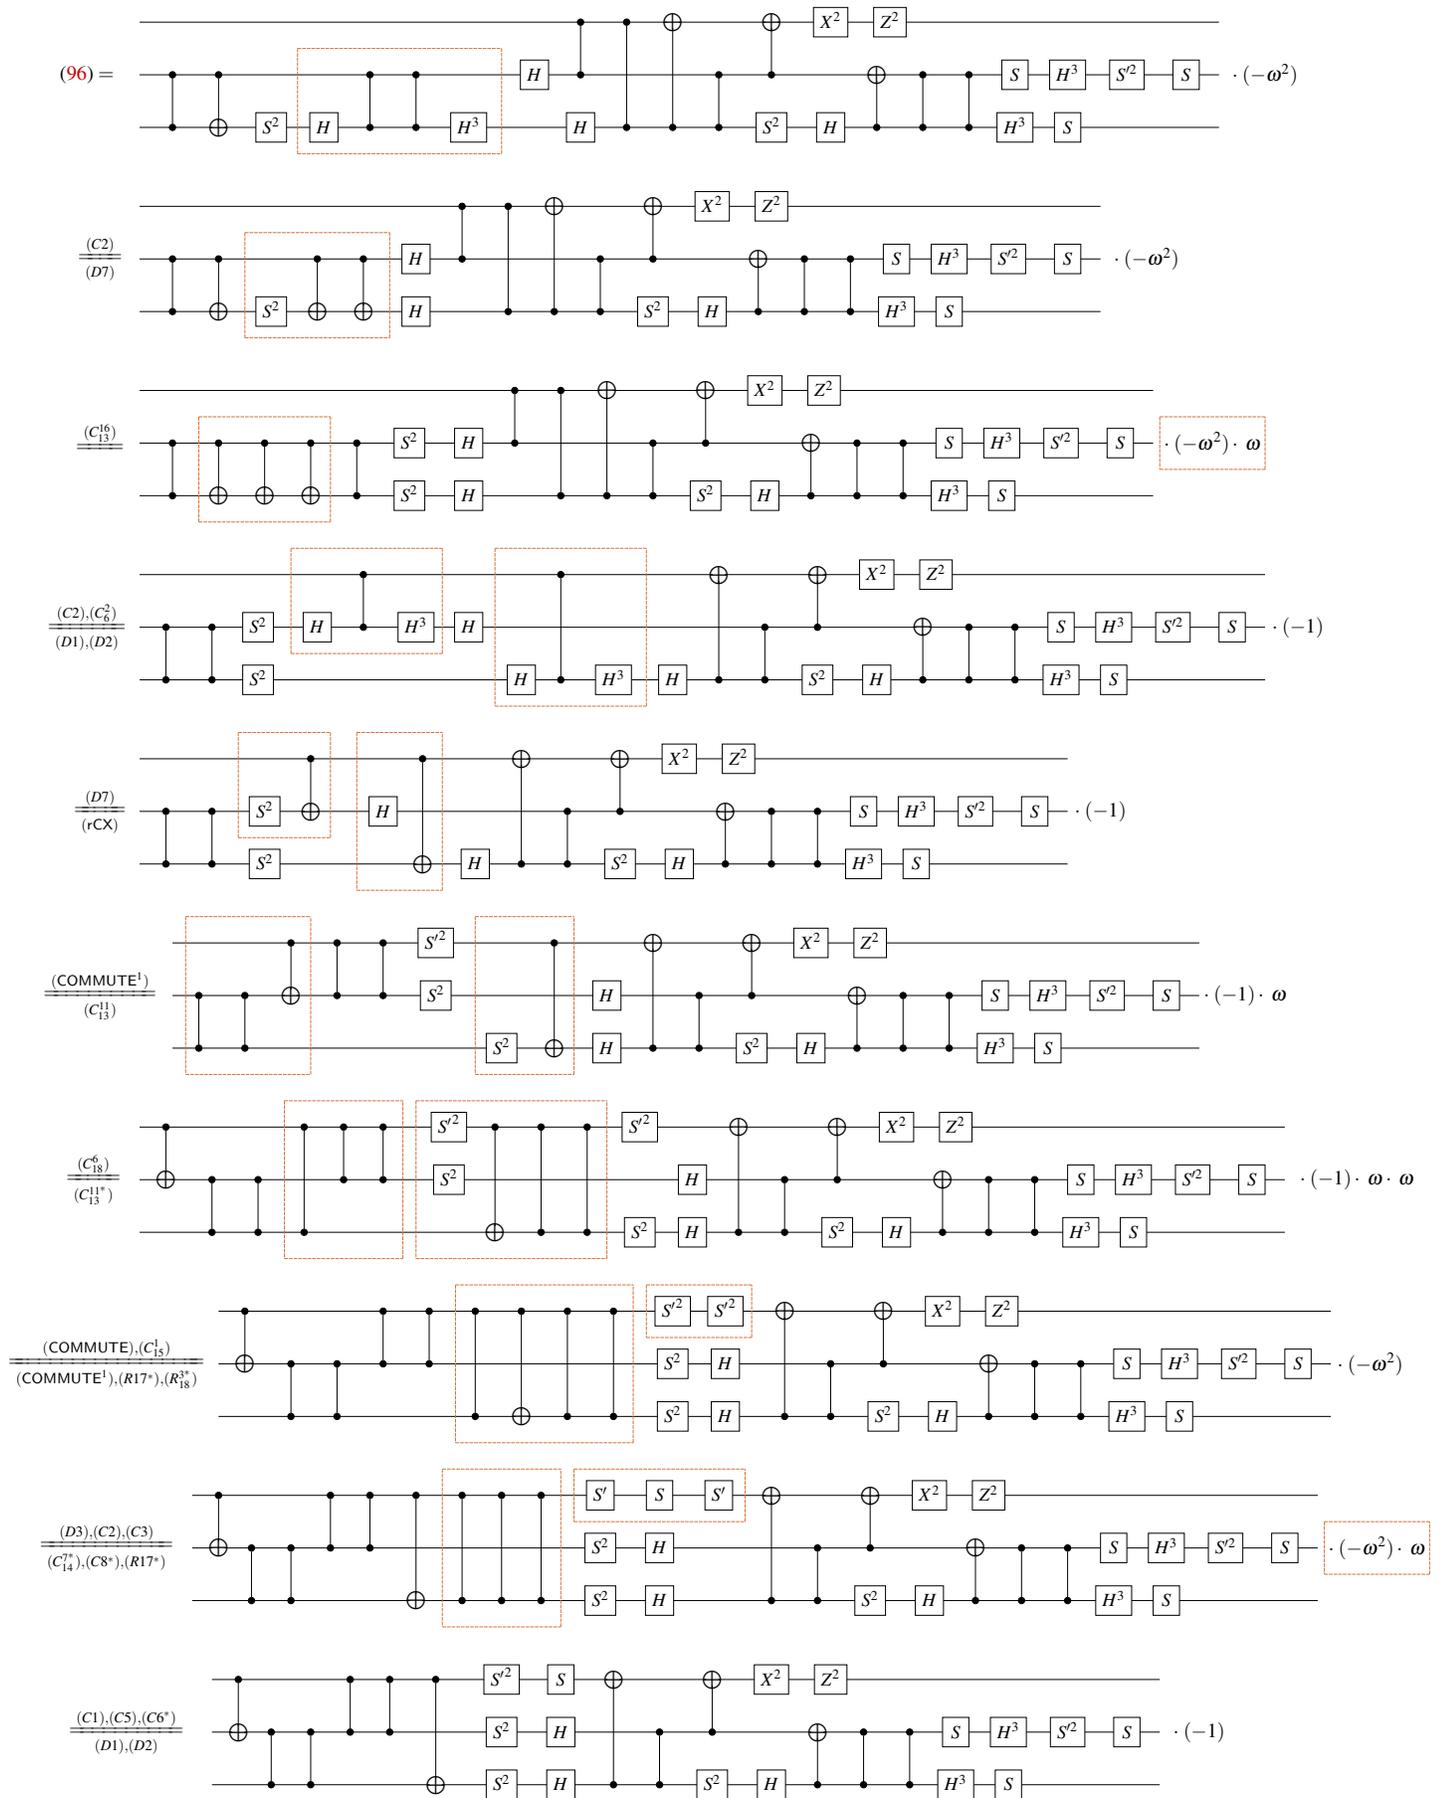

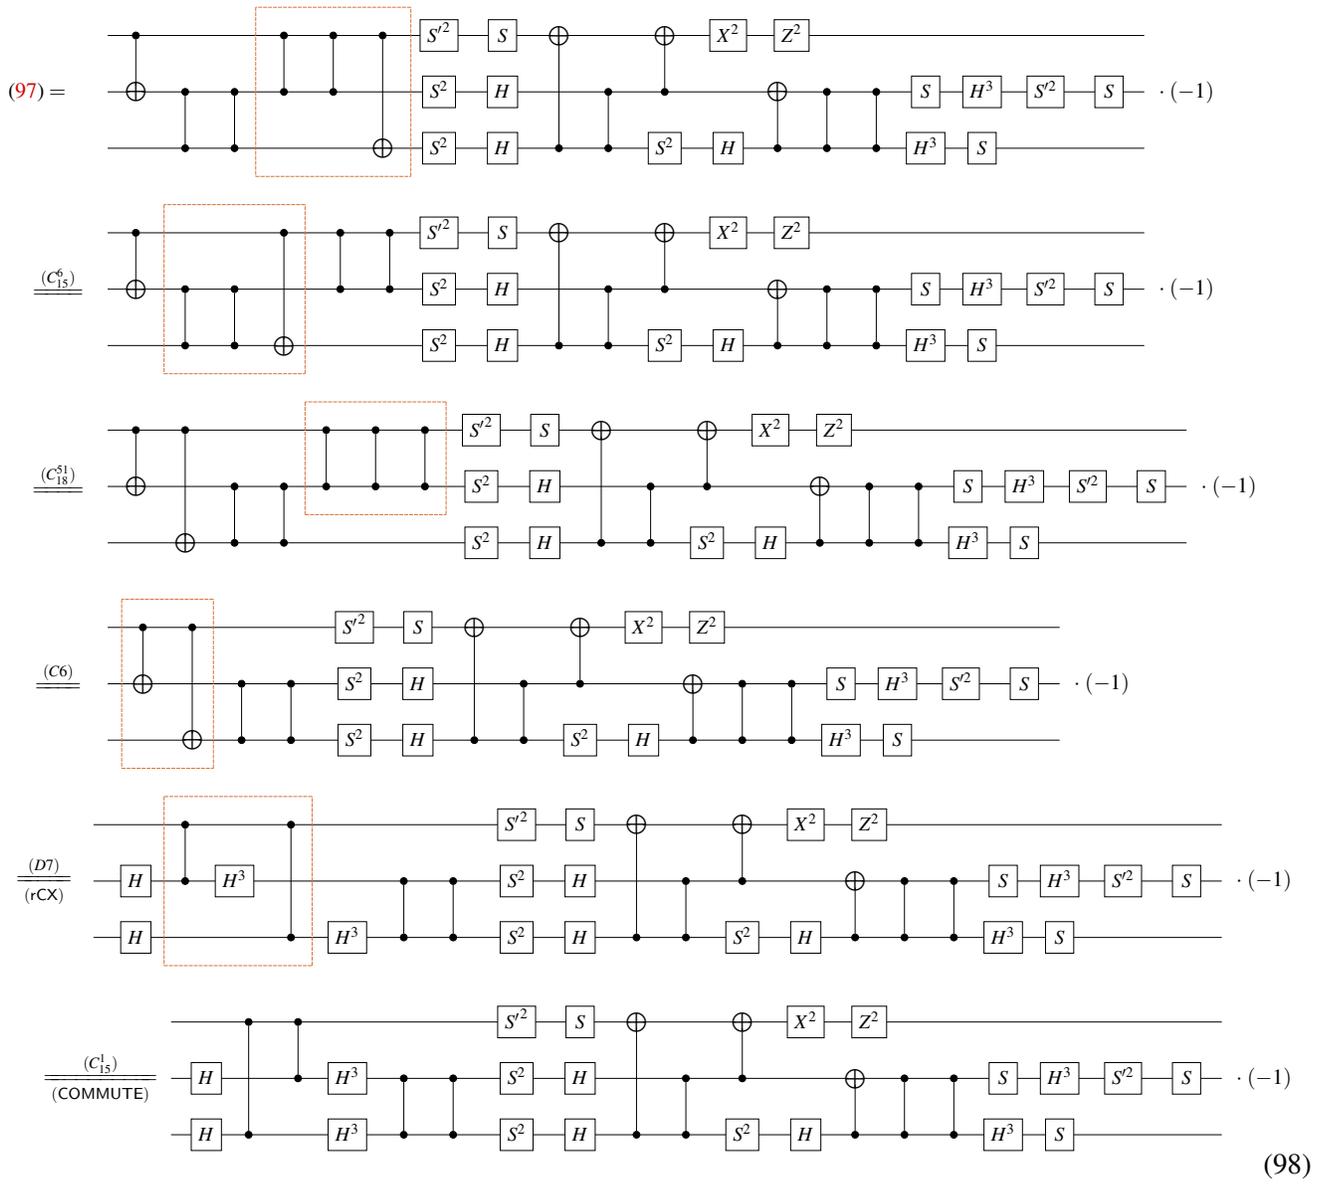

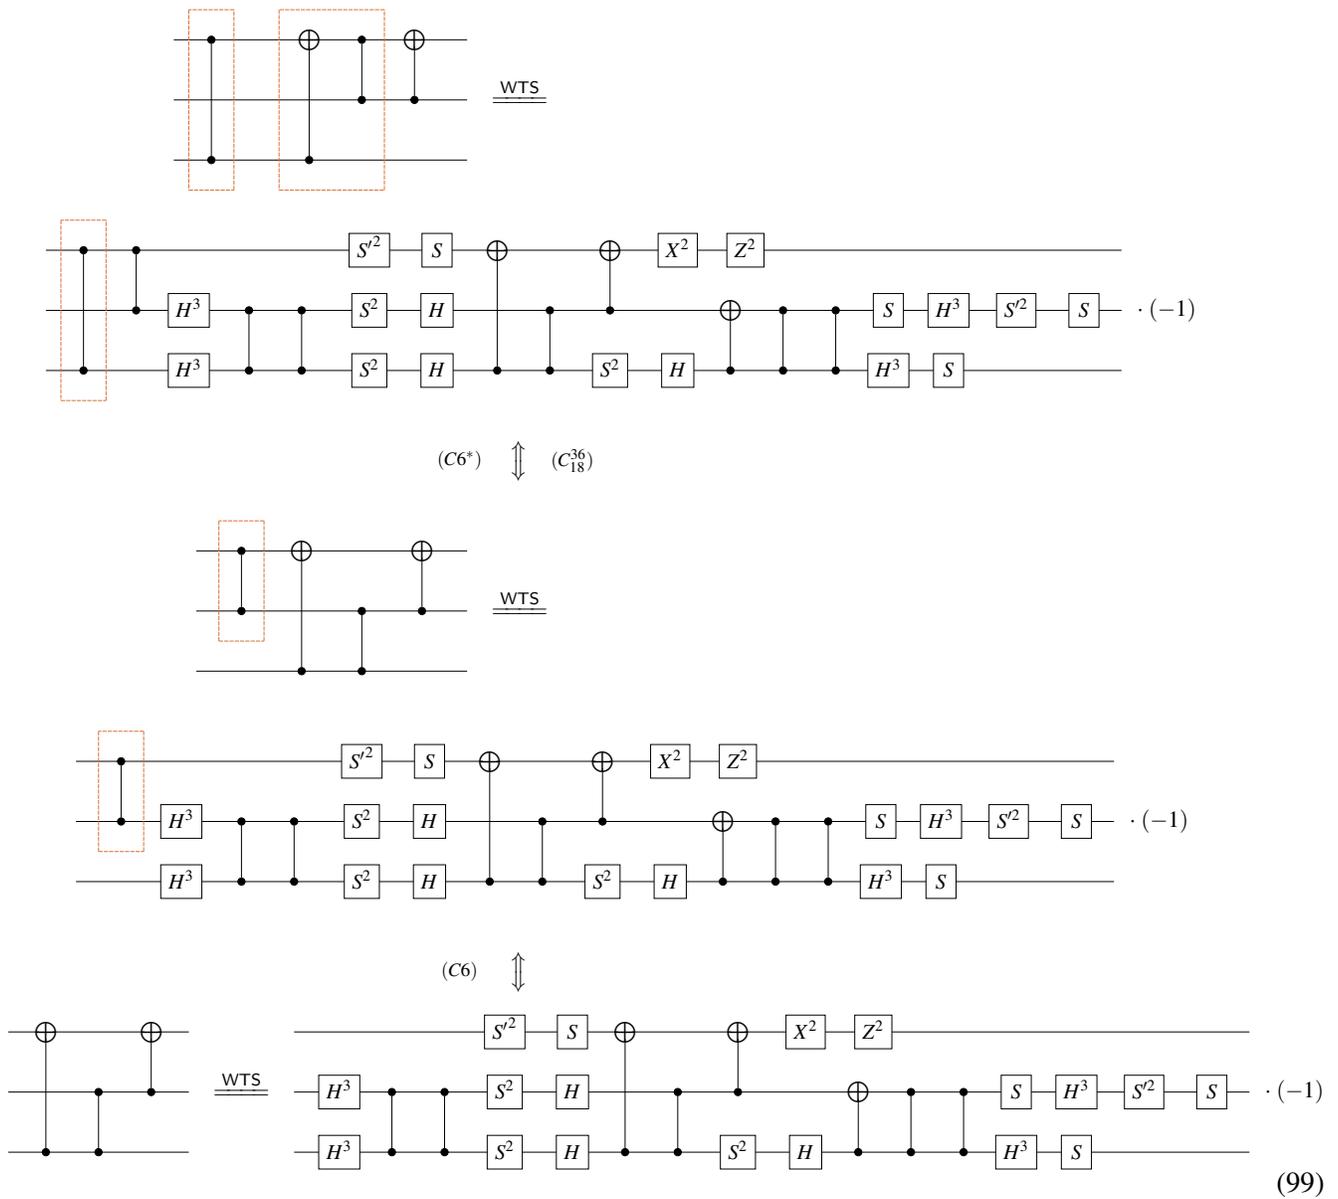

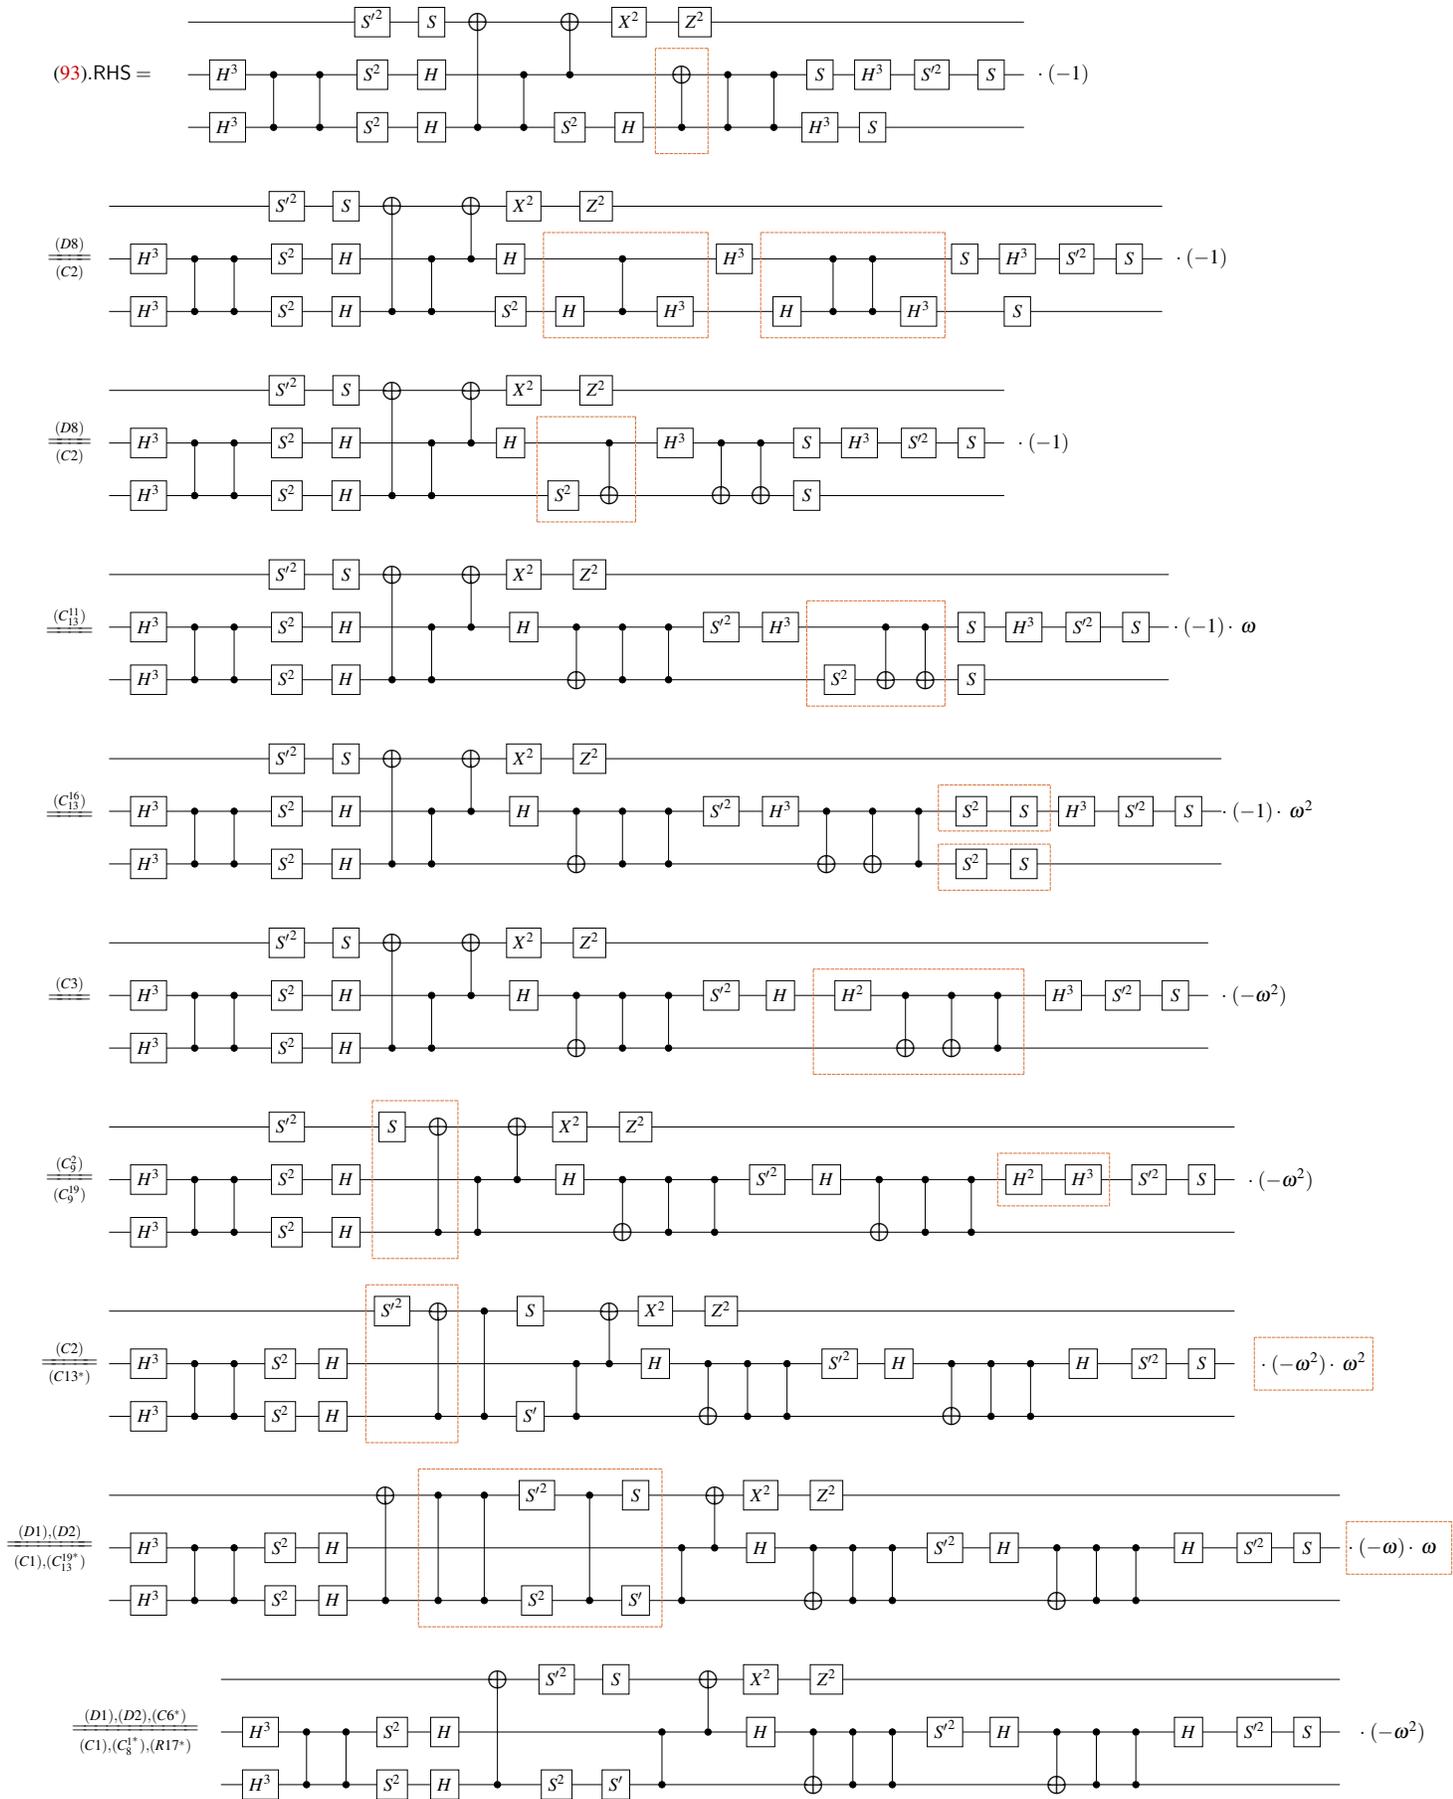

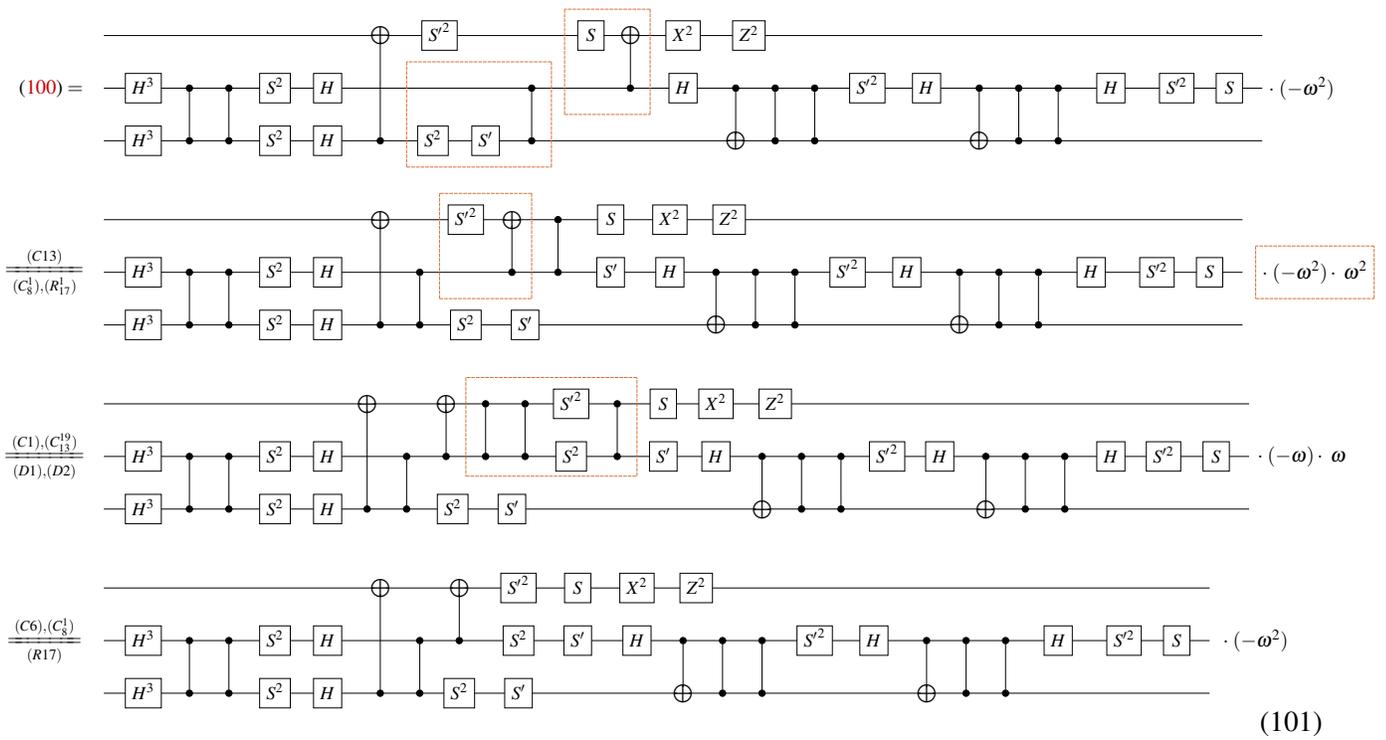

Then, (102) and (103) simplify the righthand side of (95), bringing it another step closer to its lefthand side.

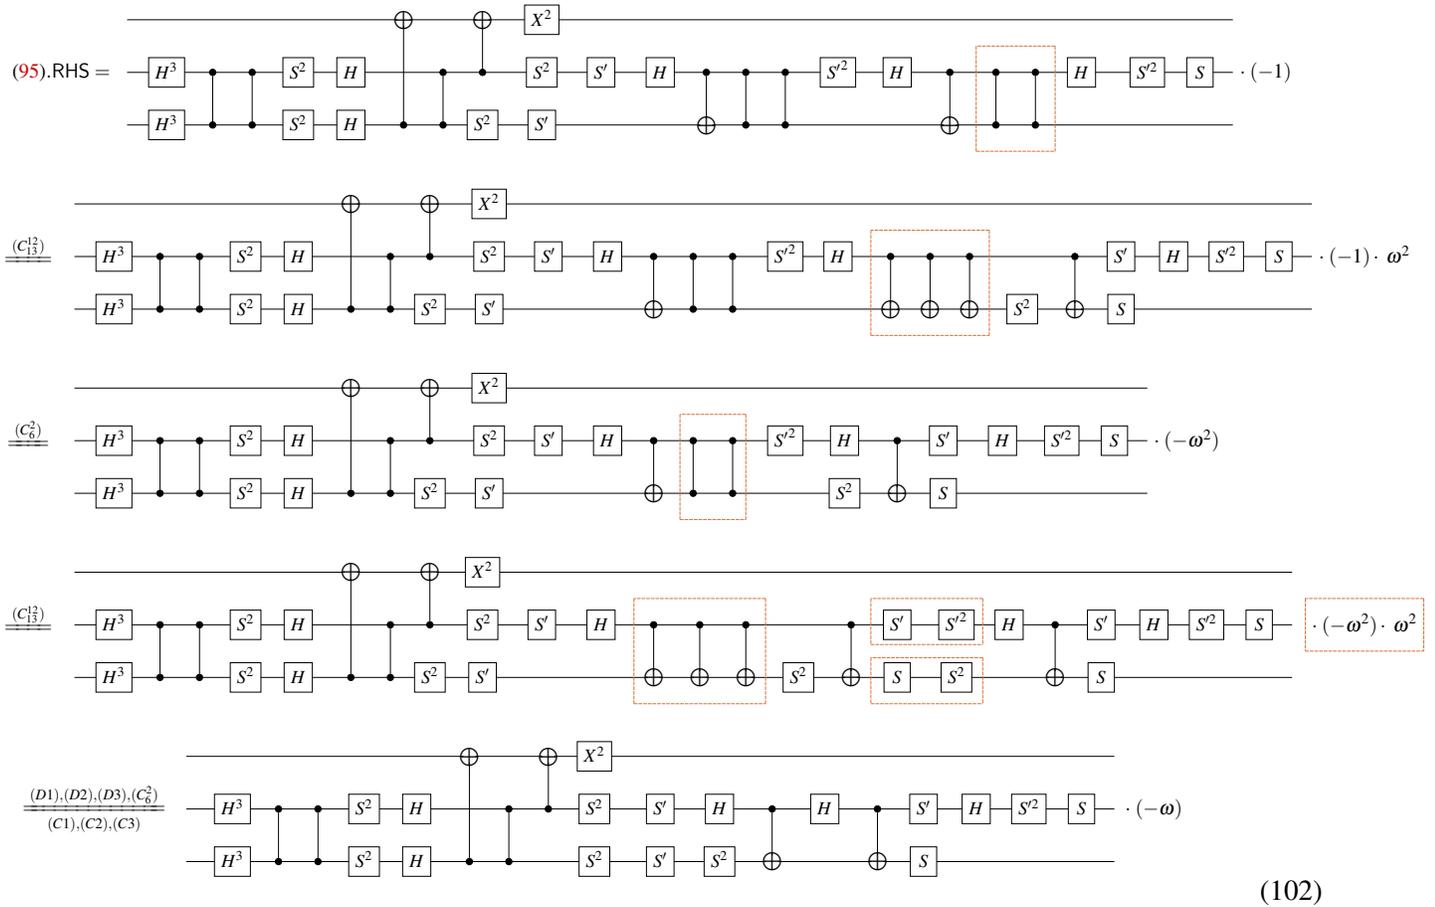

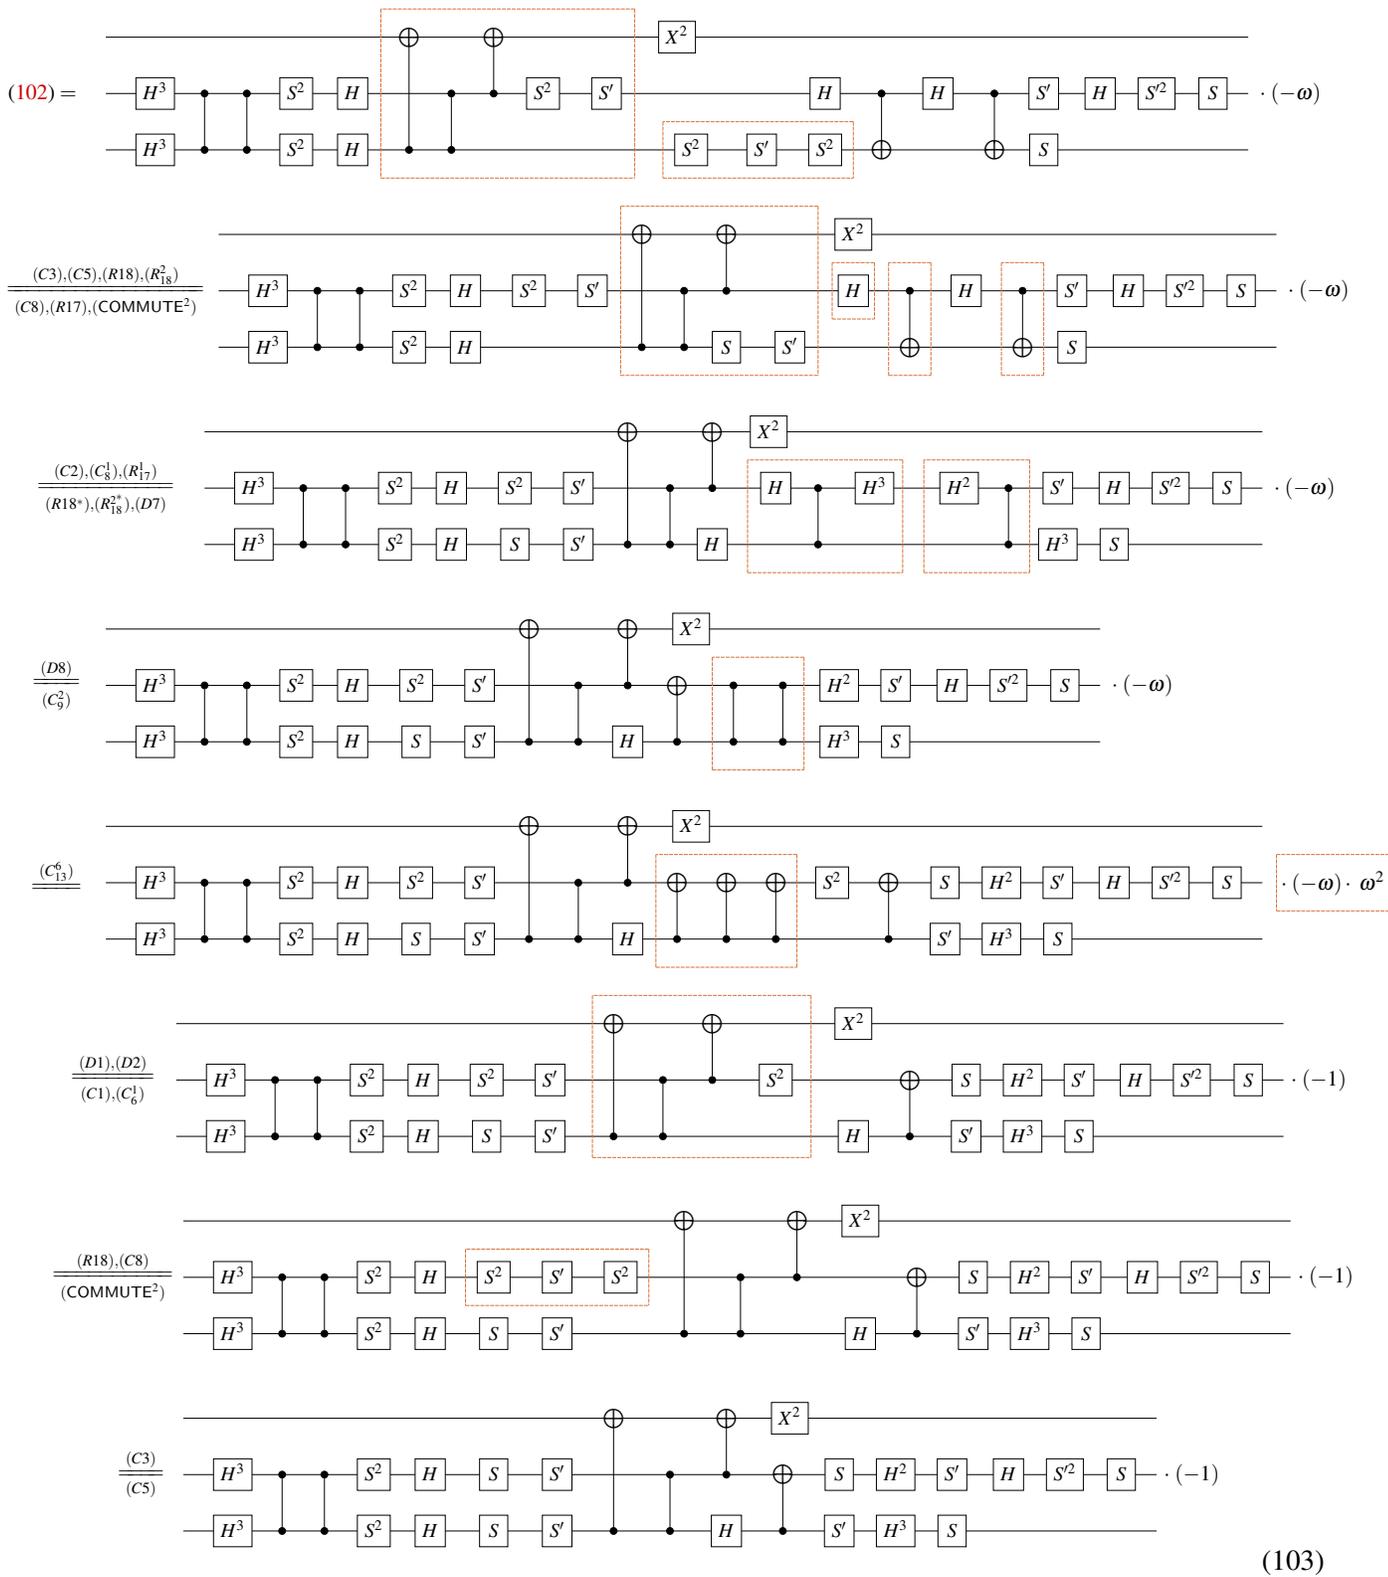

Note that

$$SH^2S'HS'^2S \xrightarrow[(C2)]{(D3)} S(H^2H^2)S(H^2HH^2)S^2H^2S \xrightarrow{(C2)} (S^2HS^2)H^2S$$

$$\stackrel{(C_4^1)}{=} (H^3SH^3)H^2S \cdot (-\omega) \stackrel{(C_2)}{=} H^3SHS \cdot (-\omega) \quad (104)$$

Based on this, as well as (D1), (D2), and (C2), (105) simplifies (103) as follows.

(103) = (105)

$\stackrel{(C_3)}{=} \stackrel{(C_3)}{=} \dots$

Therefore, it suffices to derive (106), where

$$A \stackrel{WTS}{=} BAC \iff AC^{-1} \stackrel{WTS}{=} BA.$$

(106)

By (D2), (D3), (C1), (C2), (C3), (R3), and (C<sub>6</sub><sup>1</sup>), we can rewrite (106) to (107).

(107)

By direct computation, one can check that (108) holds. According to the single-qutrit Clifford completeness established by Theorem 2.1, there exists a sequence of rewrite rules in Figure 1 such that the lefthand side of (108) can be transformed to its righthand side.

$$H^2S^2HSS' = H^3SHXZ^2 \cdot (-\omega). \quad (108)$$

This allows us to further simplify the righthand side of (107), as shown in (109).

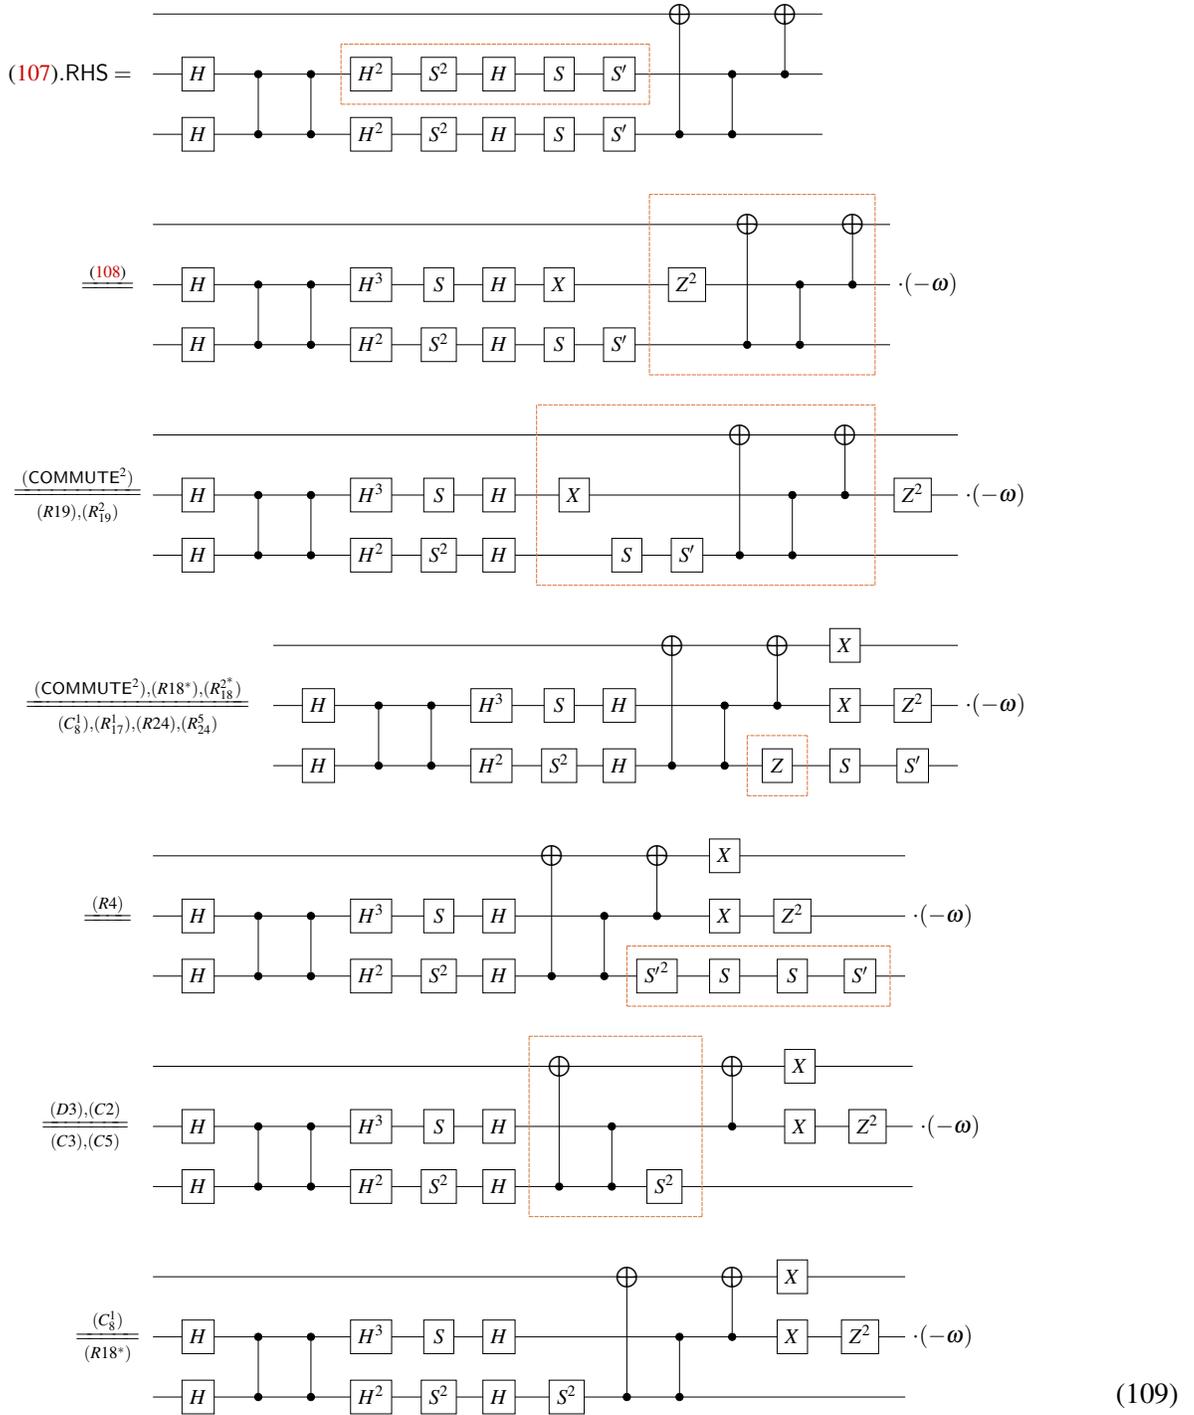

Combining (110), (D1), (D2), and (C1), (109) is simplified to (111).

$$H^2 (S^2 H S^2) \stackrel{(C_4^1)}{=} H^2 (H^3 S H^3) \cdot (-\omega) \stackrel{(C2)}{=} H S H^3 \cdot (-\omega). \tag{110}$$

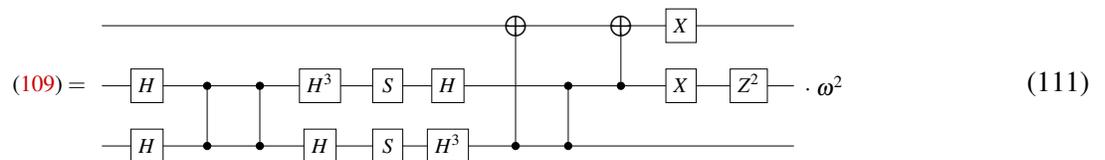

Putting (107) and (111) together, our problem is reduced to showing (112).

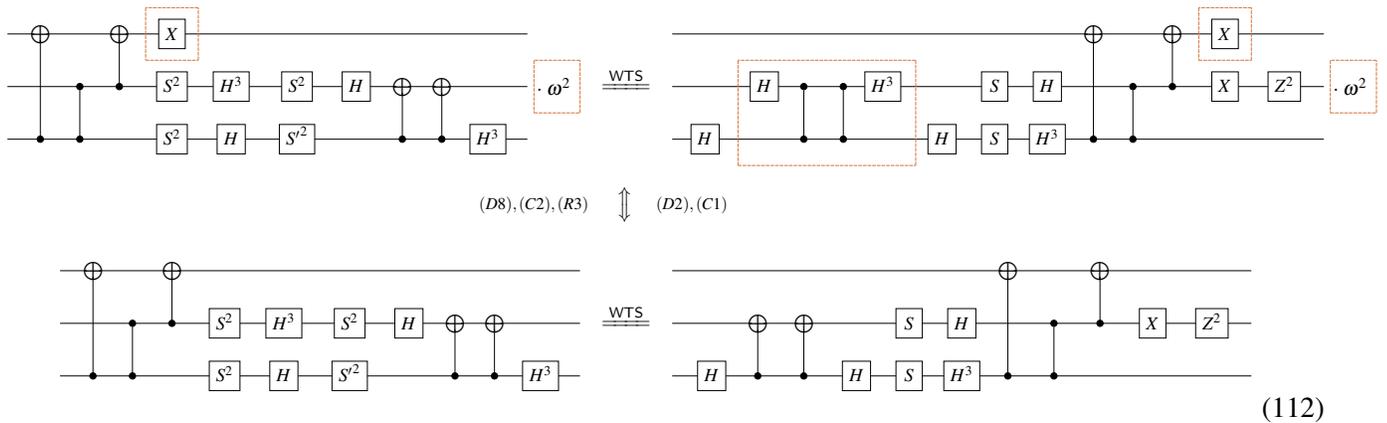

By direct computation, one can check that (113) holds. According to the single-qutrit Clifford completeness established by **Theorem 2.1**, there exists a sequence of rewrite rules in **Figure 1** such that the lefthand side of (113) can be transformed to its righthand side.

$$S^2 H^3 S^2 H = H S X Z^2 \cdot (-\omega^2). \tag{113}$$

Then, (115) simplifies the lefthand side of (112), taking it one step closer to its righthand side. By (D1), (D2), (C1), (R3), and (R6), our problem is reduced to showing (114).

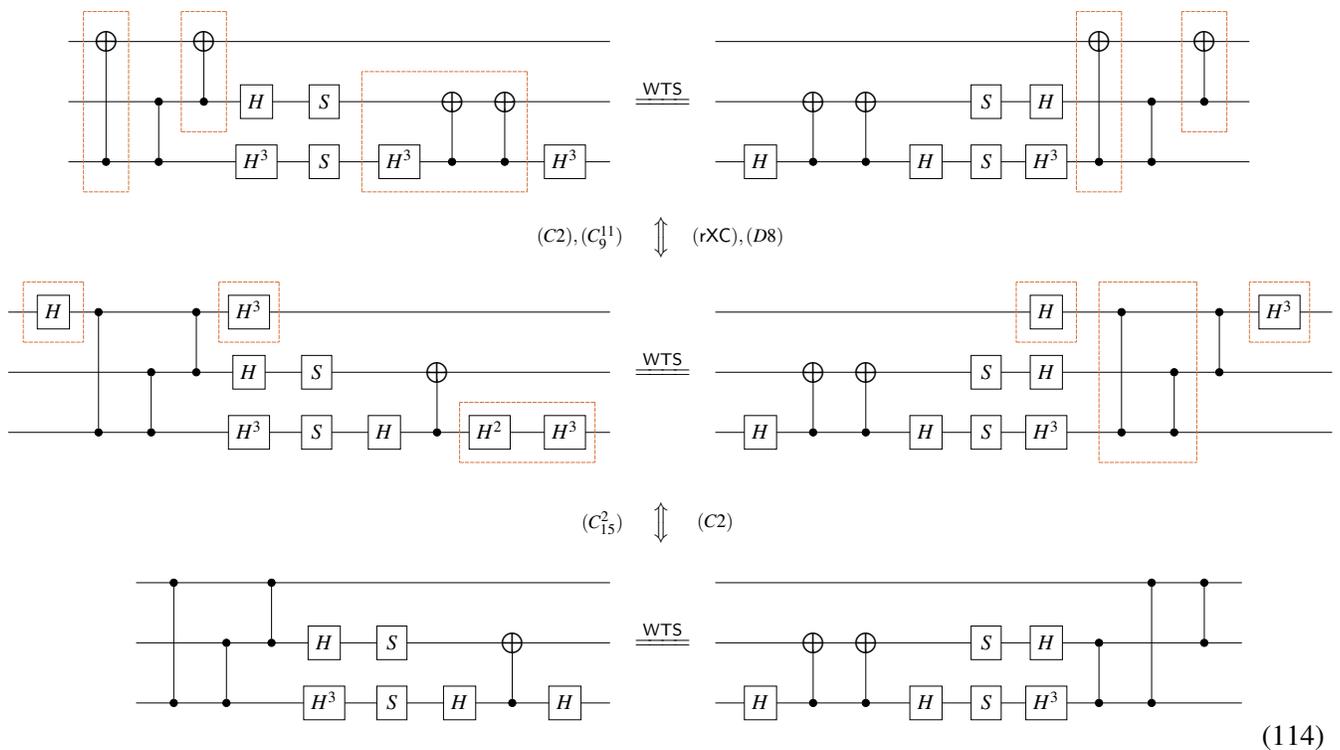

(112).LHS = 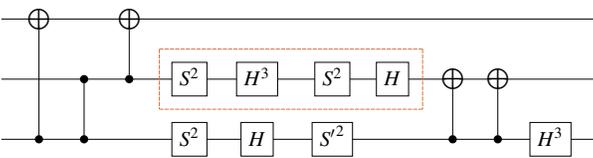

(113) 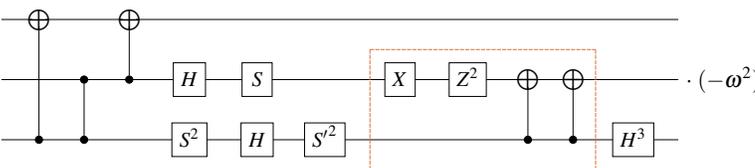  $\cdot (-\omega^2)$

$\frac{(R6),(R_{24}^9)}{(R_{19}^2),(R_{19}^4)}$  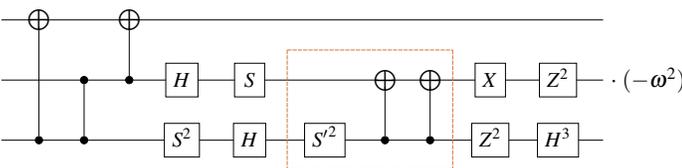  $\cdot (-\omega^2)$

(R\_{18}^2) 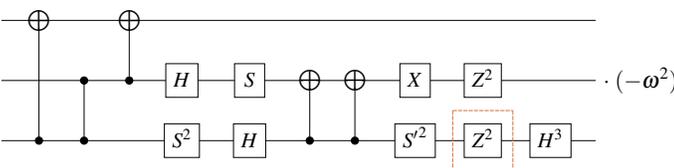  $\cdot (-\omega^2)$

(R5) 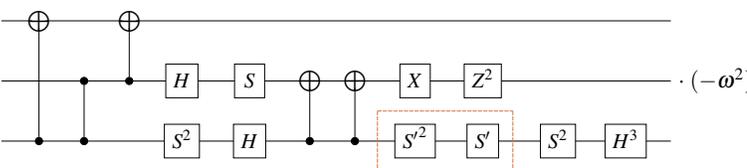  $\cdot (-\omega^2)$

$\frac{(D3),(C2)}{(C3)}$  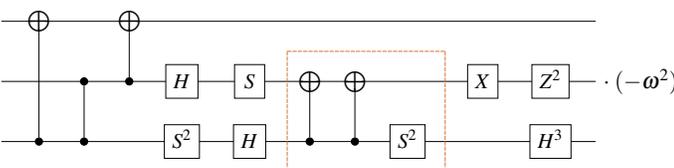  $\cdot (-\omega^2)$

(R18) 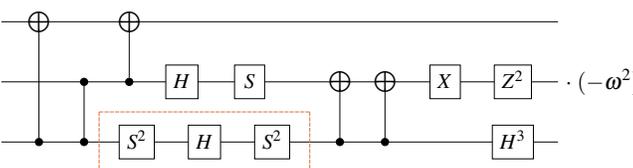  $\cdot (-\omega^2)$

(C\_4^1) 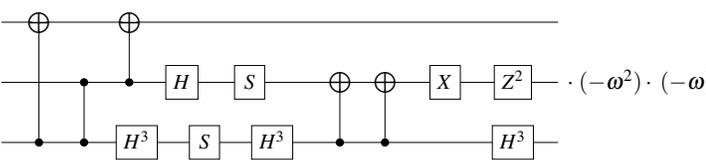  $\cdot (-\omega^2) \cdot (-\omega)$

(115)

Next, (116) simplifies the righthand side of (114), taking it one step closer to its lefthand side.

(114).RHS =

$\frac{(C2), (C_{15}^1)}{(COMMUTE)}$

$\frac{(D7)}{(D8)}$

$\frac{(C13)}{(C2)}$

$\frac{(C_9^{11}), (C_{13}^7)}{(R_{17}^{1*})}$

$\frac{(C_{18}^4), (R17^*), (D2)}{(C1), (COMMUTE)}$

$\frac{(C6^*), (C_{15}^1)}{(C_3^3), (C_9^{13})}$

(116)

Locally, (118) simplifies the two-qutrit circuit  $Q$  in (117).

$Q$

(117)

$$\begin{aligned}
 Q = & \text{Circuit with two qutrits, gates } H^3, S, H, \text{ and } \oplus. \\
 \frac{(C2)}{(D8)} & \text{Circuit with gates } H, H^3, S, H, H^3, H. \\
 \frac{(C2)}{(D7)} & \text{Circuit with gates } H, H^3, S, \oplus, \oplus, H, H^3. \\
 \frac{(C13)}{(C13)} & \text{Circuit with gates } H, H^3, \oplus, \oplus, S, H^3, S, H, \cdot \omega^2. \\
 \frac{(C2)}{(D7)} & \text{Circuit with gates } H, H^3, H, H^3, S, H^3, S, H, \cdot \omega^2. \\
 \frac{(C2)}{(C6)} & \text{Circuit with gates } H, H^3, S, H^3, S, H, \cdot \omega^2.
 \end{aligned} \tag{118}$$

Combing (117) and (118), (120) and (121) further simplify (116). Based on (114), our problem is reduced to showing (119).

$$\begin{aligned}
 & \text{Circuit 1} \xrightarrow{\text{WTS}} \text{Circuit 2} \\
 & \text{Circuit 1} \xleftrightarrow{(C6^*)} \text{Circuit 3} \xleftrightarrow{\text{WTS}} \text{Circuit 4} \\
 & \text{Circuit 3} \xleftrightarrow{(C6)} \text{Circuit 5} \\
 & \text{Circuit 1} \xrightarrow{\text{WTS}} \text{Circuit 6}
 \end{aligned} \tag{119}$$

By direct computation, one can check that (119) holds. According to the two-qutrit Clifford completeness established by Theorem 3.1, there exists a sequence of rewrite rules in Figure 1 such that the lefthand side of (119) can be transformed to its righthand side. This completes the proof.

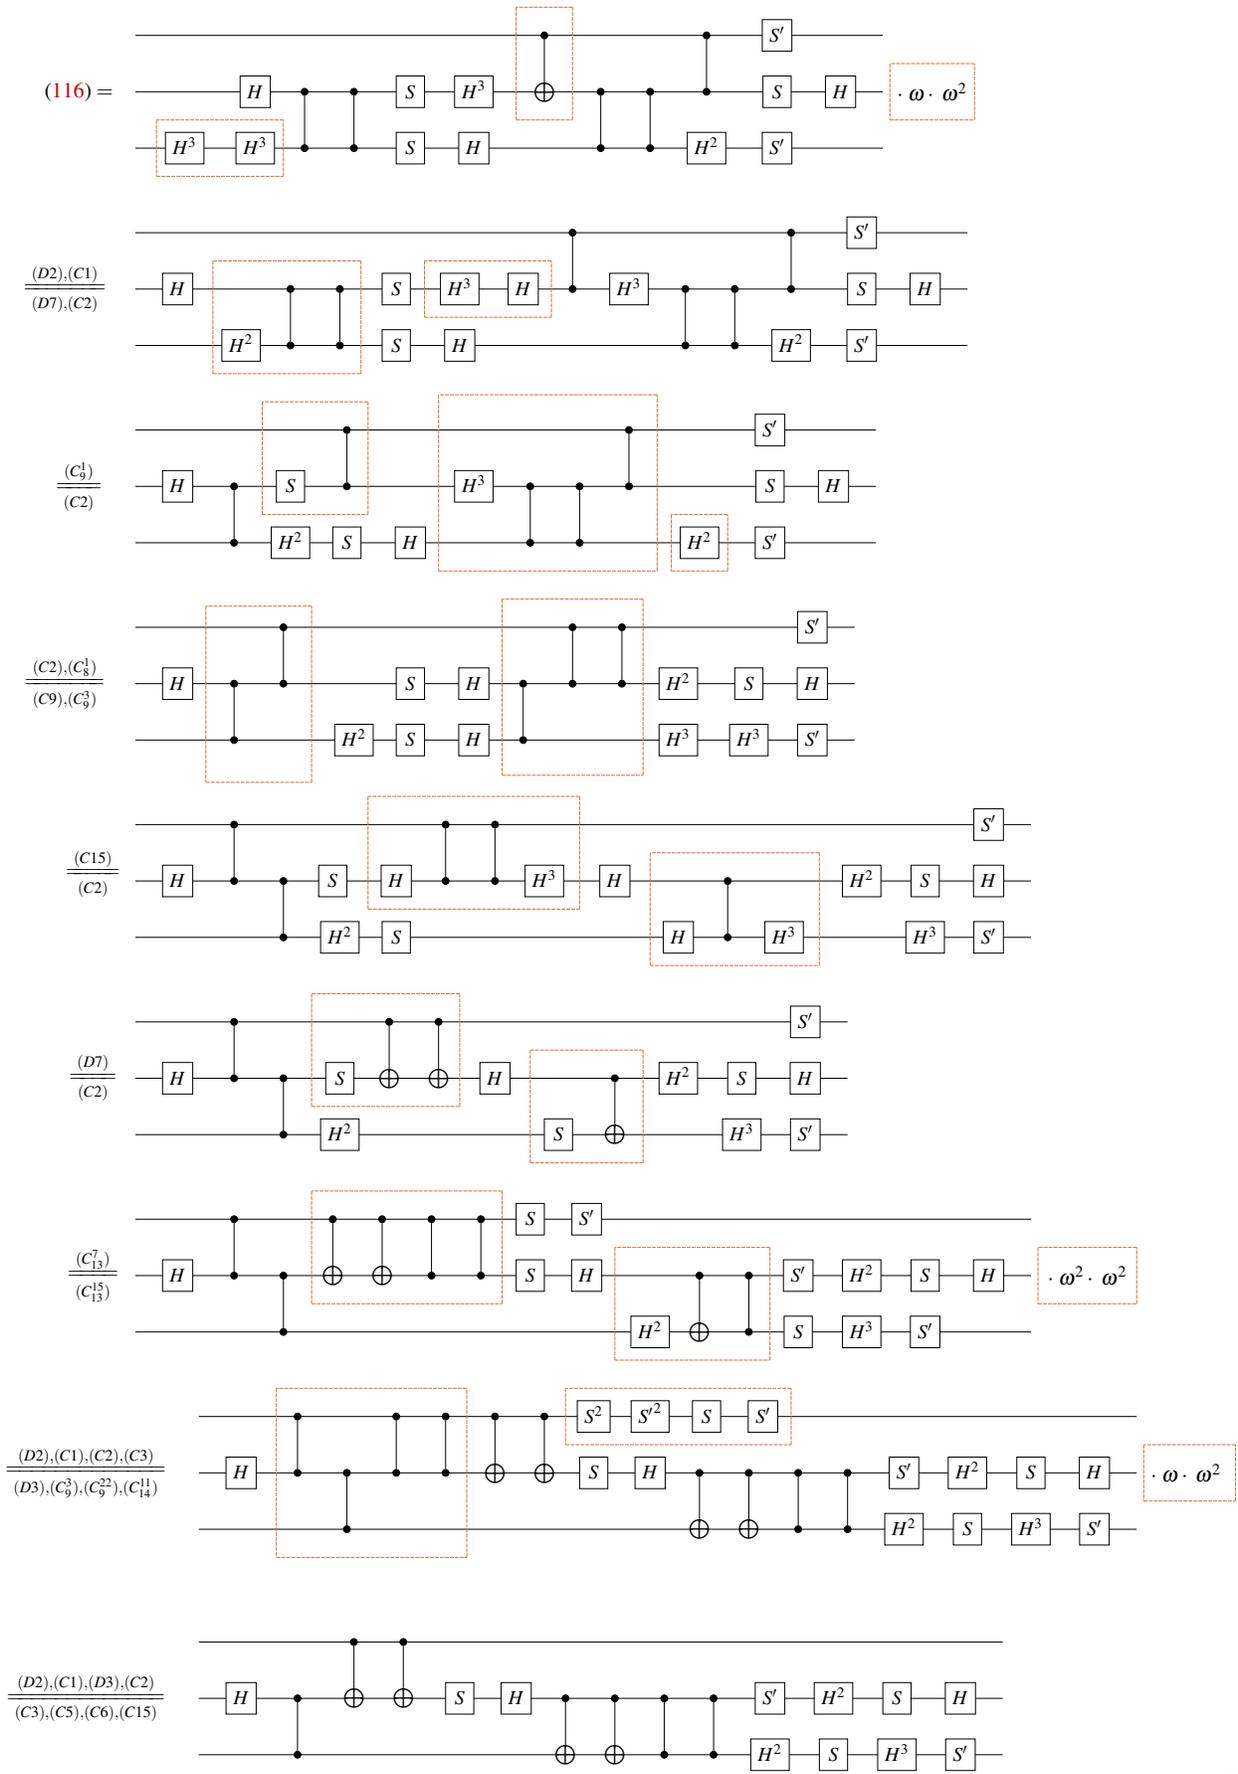

(121)

□

**Lemma 4.36.** (R53) follows from the reduced relations.

(R53)

*Proof.* First note that

$$X^2 (Z^2 X^2) Z^2 \stackrel{(R12)}{=} X^2 X^2 Z^2 Z^2 \cdot (\omega^2)^4 \stackrel{(R3),(R6)}{(D2),(C1)} XZ \cdot \omega^2. \tag{122}$$

Then, (123) leverages (R52) and rewrites the lefthand side of (R53), bringing it one step closer to its righthand side.

(R53).LHS =

(R52)

(84)  
(C8), (C8')

(R52)

(84)  
(C3)

(122)  
(C3)

(D2)  
(C1)

(123)

Note also that

$$XZ \stackrel{(D4)}{\stackrel{(R4)}{=}} HSH^2S^2HS'^2S. \tag{124}$$

Hence, it suffices to derive (125) from the equations in Figure 1 and section 1.

(125)

By (C2), (C3), (C6), (C6<sup>1</sup>), (C6<sup>1</sup>)<sup>\*</sup>, (C6<sup>1</sup>)<sup>\*</sup>, (R3), and (R6), our problem is reduced to showing (126).

(126)

By direct computation, one can check that (126) holds. According to the two-qutrit Clifford completeness established by [Theorem 3.1](#), there exists a sequence of rewrite rules in [Figure 1](#) such that the lefthand side of (126) can be transformed to its righthand side. This completes the proof. □

**Proposition 4.37.** *Up to the single- and two-qutrit Clifford completeness, the equations in [Figures 59 and 60](#) imply all equations in [Section 1.3](#).*

*Proof.* By [Proposition 4.3](#), [lemmas 4.4 to 4.8](#), [4.10 to 4.15](#), [4.17](#), [4.18](#), [4.21](#), [4.22](#) and [4.25 to 4.36](#), and [corollaries 4.9](#), [4.16](#), [4.19](#), [4.20](#), [4.23](#) and [4.24](#), we complete the proof. □

## 4.2 Reduce the Three-Qutrit Box Relations

**Lemma 4.38.** *The equations in [Figures 1 and 2](#) as well as [Section 1](#) suffice to prove all box relations in [Appendix C.4](#) of [\[1\]](#).*

*Proof.* Details are in the GitHub repository: [QutritClifford/Three-Qutrit/Box2Derived](https://github.com/SarahMMMLi/QutritClifford/tree/main/Three-Qutrit/Box2Derived)<sup>3</sup>. □

**Theorem 4.1.** *Up to the single- and two-qutrit Clifford completeness, any true equality between three-qutrit Clifford circuits is provable using the rules in [Figure 60](#) with the derived generators in [Figure 59](#).*

*Proof.* By [Proposition 4.3](#) in [\[1\]](#), the box relations in [Appendices C.1 to C.4](#) are complete for the three-qutrit Clifford group. By [Lemma 4.38](#), the equations in [Figures 1 and 2](#) as well as [Section 1](#) suffice to prove all box relations in [Appendix C.4](#). By [Proposition 4.37](#), the equations in [Section 1.3](#) follow from the equations in [Figures 1 and 2](#). This implies that up to the single- and two-qutrit Clifford completeness, we can prove any true equality between three-qutrit Clifford circuits using the rules in [Figure 1](#) with the derived generators in [Figure 2](#). □

<sup>3</sup><https://github.com/SarahMMMLi/QutritClifford/tree/main/Three-Qutrit/Box2Derived>

## References

- [1] Sarah Meng Li, Michele Mosca, Neil J. Ross, John van de Wetering & Yuming Zhao (2025): *A Complete and Natural Rule Set for Multi-Qutrit Clifford Circuits*. *Electronic Proceedings in Theoretical Computer Science* 343, p. 210–264, doi:<https://doi.org/10.4204/eptcs.343.11>. Available at <http://dx.doi.org/10.4204/EPTCS.343.11>.
